# Supplementary material for: Possible high-temperature superconductors predicted from electronic structure and data-filtering algorithms
Source: arXiv:1109.6935 source file (2011-09-30)
Supplement: Supplementary file 1 [file supplementary.pdf]

## Supplementary information

The table below shows compound name, space group, space group number, bravais lattice and ICSD reference number. Using the ICSD web-site [1], and the ICSD reference number, allows the reader to generate pictures of the crystal structure.

In the fat-band representation the thickness of the band corresponds to the amount of *s*-, *p*- or *d*-character of the band. This is calculated as follows. Let  $n(\mathbf{k})$  be the occupation at  $\mathbf{k}$  given by

$$n(\mathbf{k}) = Tr(O(\mathbf{k})\rho(\mathbf{k}))$$

where  $O(\mathbf{k})$  and  $\rho(\mathbf{k})$  is the overlap and density, respectively. The fatness  $f_l$  for eigenvalue  $\nu$  can then be calculated using

$$f_l = \frac{Tr(O(\mathbf{k})\rho^{\nu_l}(\mathbf{k}))}{Tr(O(\mathbf{k})\rho(\mathbf{k}))}$$

where element  $ij$  of the density matrix is given in terms of weights ( $w$ ) and eigenvectors ( $Z$ ) by:

$$\rho_{ij}(\mathbf{k}) = \sum_{\nu} w_{\nu,\mathbf{k}} Z_i(\mathbf{k}, \nu) Z_j^{\dagger}(\mathbf{k}, \nu)$$

$$\rho_{ij}^{\nu_l}(\mathbf{k}) = w_{\nu_l,\mathbf{k}} Z_i(\mathbf{k}, \nu_l) Z_j^{\dagger}(\mathbf{k}, \nu_l)$$

$\sum_l f_l$  sums up to one electron and  $l$  runs over the complete basis. Note that in the figures below the Fermi level is at zero. Also, in the band plots we make a projection on atomic and l-resolved fat bands.

- 
- [1] G. Bergerhoff and I. D. Brown, in Crystallographic Databases, F. H. Allen et al. (Hrsg.) Chester, International Union of Crystallography, (1987). The figures were generated using ICSD Web (<http://icsd.fiz-karlsruhe.de/icsd>) using version 2.1.0.

| Material                                                          | Space group | (#)   | Bravais lattice     | ICSD # |
|-------------------------------------------------------------------|-------------|-------|---------------------|--------|
| AuCuZn <sub>2</sub>                                               | F m -3 m    | (225) | cubic face-centred  | 150571 |
| AgAuZn <sub>2</sub>                                               | F m -3 m    | (225) | cubic face-centred  | 604792 |
| CuNi <sub>2</sub> Sb                                              | F m -3 m    | (225) | cubic face-centred  | 53320  |
| CuNi <sub>2</sub> Sn                                              | F m -3 m    | (225) | cubic face-centred  | 103068 |
| ErPt <sub>2</sub>                                                 | F d -3 m S  | (227) | cubic face-centred  | 103287 |
| EuPt <sub>2</sub>                                                 | F d -3 m S  | (227) | cubic face-centred  | 103430 |
| HoPt <sub>2</sub>                                                 | F d -3 m S  | (227) | cubic face-centred  | 104441 |
| NaPt <sub>2</sub>                                                 | F d -3 m S  | (227) | cubic face-centred  | 644945 |
| BaPt <sub>2</sub>                                                 | F d -3 m S  | (227) | cubic face-centred  | 616039 |
| CuSe                                                              | P 63/m m c  | (194) | hexagonal primitive | 240    |
| KAuTe                                                             | P 63/m m c  | (194) | hexagonal primitive | 40165  |
| RbAuTe                                                            | P 63/m m c  | (194) | hexagonal primitive | 75026  |
| CdInGaS <sub>4</sub>                                              | P -3 m 1    | (164) | hexagonal primitive | 20785  |
| ZrNCl                                                             | P -3 m 1    | (164) | hexagonal primitive | 25506  |
| KCuSe                                                             | P 63/m m c  | (194) | hexagonal primitive | 12157  |
| KCuTe                                                             | P 63/m m c  | (194) | hexagonal primitive | 12158  |
| Li <sub>2</sub> ZnGe                                              | P -3 m 1    | (164) | hexagonal primitive | 53678  |
| Li <sub>2</sub> ZnSi                                              | P -3 m 1    | (164) | hexagonal primitive | 16221  |
| AuYO <sub>2</sub>                                                 | P 63/m m c  | (194) | hexagonal primitive | 95675  |
| AgAlO <sub>2</sub>                                                | P 63/m m c  | (194) | hexagonal primitive | 300020 |
| CuBr                                                              | P 63 m c    | (186) | hexagonal primitive | 30092  |
| Ca <sub>2</sub> CuZn <sub>2</sub> P <sub>3</sub>                  | P 63/m m c  | (194) | hexagonal primitive | 89517  |
| Al <sub>5</sub> C <sub>3</sub> N                                  | P 63 m c    | (186) | hexagonal primitive | 26859  |
| Ca <sub>3</sub> Cu <sub>2</sub> Zn <sub>2</sub> P <sub>4</sub>    | P -3 m 1    | (164) | hexagonal primitive | 89515  |
| Eu <sub>3</sub> Cu <sub>2</sub> Zn <sub>2</sub> P <sub>4</sub>    | P -3 m 1    | (164) | hexagonal primitive | 89516  |
| Cu <sub>4</sub> (S <sub>2</sub> ) <sub>2</sub> (CuS) <sub>2</sub> | P 63/m m c  | (194) | hexagonal primitive | 26968  |

| Material                                                             | Space group  | (#)   | Bravais lattice           | ICSD # |
|----------------------------------------------------------------------|--------------|-------|---------------------------|--------|
| LaKPtO <sub>3</sub>                                                  | C 1 2/m 1    | (12)  | monoclinic base-centred   | 417108 |
| BaY <sub>2</sub> F <sub>8</sub>                                      | C 1 2/m 1    | (12)  | monoclinic base-centred   | 74359  |
| AgCuS                                                                | C m c m      | (63)  | orthorhombic base-centred | 30233  |
| LaSeTe <sub>2</sub>                                                  | C m c m      | (63)  | orthorhombic base-centred | 413171 |
| NbS <sub>2</sub>                                                     | C m 2 m      | (38)  | orthorhombic base-centred | 67443  |
| BaNiY <sub>2</sub> O <sub>5</sub>                                    | I m m m      | (71)  | orthorhombic body-centred | 68795  |
| RuOCl <sub>2</sub>                                                   | I m m m      | (71)  | orthorhombic body-centred | 83883  |
| Bi <sub>2</sub> (CO <sub>3</sub> )O <sub>2</sub>                     | I m m 2      | (44)  | orthorhombic body-centred | 94740  |
| Al <sub>2</sub> Ba <sub>3</sub> Ge <sub>2</sub>                      | I m m m      | (71)  | orthorhombic body-centred | 52612  |
| Ba <sub>3</sub> Al <sub>2</sub> Si <sub>2</sub>                      | I m m m      | (71)  | orthorhombic body-centred | 100128 |
| Ba <sub>3</sub> Al <sub>2</sub> Sn <sub>2</sub>                      | I m m m      | (71)  | orthorhombic body-centred | 9565   |
| NbSe <sub>2</sub>                                                    | F m 2 m      | (42)  | orthorhombic face-centred | 71339  |
| TaS <sub>2</sub>                                                     | F m 2 m      | (42)  | orthorhombic face-centred | 280988 |
| TaSe <sub>2</sub>                                                    | F 2 m m      | (42)  | orthorhombic face-centred | 67651  |
| TaSe <sub>2</sub>                                                    | F m 2 m      | (42)  | orthorhombic face-centred | 72198  |
| Tl <sub>2</sub> Ba <sub>2</sub> CuO <sub>6</sub>                     | F m m m      | (69)  | orthorhombic face-centred | 41569  |
| TiNCl                                                                | P m m n S    | (59)  | orthorhombic primitive    | 27396  |
| Pb <sub>2</sub> Ba <sub>2</sub> YCuCu <sub>2</sub> O <sub>8</sub>    | P 2 21 2     | (17)  | orthorhombic primitive    | 66088  |
| Pb <sub>2</sub> Sr <sub>2</sub> YCu <sub>3</sub> O <sub>8</sub>      | P 2 21 2     | (17)  | orthorhombic primitive    | 66587  |
| YBa <sub>2</sub> Cu <sub>3</sub> O <sub>6.5</sub>                    | P m m m      | (47)  | orthorhombic primitive    | 75697  |
| YBa <sub>2</sub> Cu <sub>3</sub> O <sub>6.5</sub>                    | P m m m      | (47)  | orthorhombic primitive    | 96016  |
| EuBa <sub>2</sub> Cu <sub>3</sub> O <sub>7</sub>                     | P m m m      | (47)  | orthorhombic primitive    | 81171  |
| Ba <sub>2</sub> GdCu <sub>3</sub> O <sub>7</sub>                     | P m m m      | (47)  | orthorhombic primitive    | 56514  |
| HoBa <sub>2</sub> Cu <sub>3</sub> O <sub>7</sub>                     | P m m m      | (47)  | orthorhombic primitive    | 68044  |
| LaBa <sub>2</sub> Cu <sub>3</sub> O <sub>7</sub>                     | P m m m      | (47)  | orthorhombic primitive    | 81167  |
| NdBa <sub>2</sub> Cu <sub>3</sub> O <sub>7</sub>                     | P m m m      | (47)  | orthorhombic primitive    | 81169  |
| PrBa <sub>2</sub> Cu <sub>3</sub> O <sub>7</sub>                     | P m m m      | (47)  | orthorhombic primitive    | 81168  |
| SmBa <sub>2</sub> Cu <sub>3</sub> O <sub>7</sub>                     | P m m m      | (47)  | orthorhombic primitive    | 71705  |
| Ba <sub>2</sub> YCu <sub>3</sub> O <sub>7</sub>                      | P m m m      | (47)  | orthorhombic primitive    | 202770 |
| Ba <sub>2</sub> YCu <sub>3</sub> O <sub>7</sub>                      | P m m m      | (47)  | orthorhombic primitive    | 77737  |
| LaBa <sub>2</sub> Cu <sub>3</sub> O <sub>8</sub>                     | P m m m      | (47)  | orthorhombic primitive    | 85291  |
| Na <sub>3</sub> Cu <sub>4</sub> S <sub>4</sub>                       | P b a m      | (55)  | orthorhombic primitive    | 10004  |
| Sr <sub>4</sub> V <sub>3</sub> O <sub>10</sub>                       | I 4/m m m    | (139) | tetragonal body-centred   | 73698  |
| MoB                                                                  | I 41/a m d S | (141) | tetragonal body-centred   | 24280  |
| WB                                                                   | I 41/a m d S | (141) | tetragonal body-centred   | 24281  |
| Yb(AgS <sub>2</sub> )                                                | I 41 m d     | (109) | tetragonal body-centred   | 27091  |
| LaI <sub>2</sub>                                                     | I 4/m m m    | (139) | tetragonal body-centred   | 202452 |
| SmCu <sub>2</sub> Si <sub>2</sub>                                    | I 4/m m m    | (139) | tetragonal body-centred   | 106843 |
| TbCu <sub>2</sub> Si <sub>2</sub>                                    | I 4/m m m    | (139) | tetragonal body-centred   | 106844 |
| Cu <sub>2</sub> TmSi <sub>2</sub>                                    | I 4/m m m    | (139) | tetragonal body-centred   | 53349  |
| Cu <sub>2</sub> YSi <sub>2</sub>                                     | I 4/m m m    | (139) | tetragonal body-centred   | 23551  |
| Li <sub>2</sub> PdH <sub>2</sub>                                     | I 4/m m m    | (139) | tetragonal body-centred   | 108534 |
| Na <sub>2</sub> PdH <sub>2</sub>                                     | I 4/m m m    | (139) | tetragonal body-centred   | 68071  |
| (Cu <sub>2</sub> S <sub>2</sub> )(Sr <sub>2</sub> NiO <sub>2</sub> ) | I 4/m m m    | (139) | tetragonal body-centred   | 88424  |
| Ca <sub>2</sub> (CuBr <sub>2</sub> O <sub>2</sub> )                  | I 4/m m m    | (139) | tetragonal body-centred   | 1028   |
| Sr <sub>2</sub> CoO <sub>2</sub> Br <sub>2</sub>                     | I 4/m m m    | (139) | tetragonal body-centred   | 151789 |
| CuSr <sub>2</sub> Br <sub>2</sub> O <sub>2</sub>                     | I 4/m m m    | (139) | tetragonal body-centred   | 1178   |
| Ca <sub>2</sub> (CuCl <sub>2</sub> O <sub>2</sub> )                  | I 4/m m m    | (139) | tetragonal body-centred   | 1027   |
| Ca <sub>2</sub> CuO <sub>2</sub> Cl <sub>2</sub>                     | I 4/m m m    | (139) | tetragonal body-centred   | 83117  |
| Sr <sub>2</sub> CuO <sub>2</sub> Cl <sub>2</sub>                     | I 4/m m m    | (139) | tetragonal body-centred   | 4087   |
| Tl <sub>2</sub> Ba <sub>2</sub> CaCu <sub>2</sub> O <sub>8</sub>     | I 4/m m m    | (139) | tetragonal body-centred   | 78592  |
| Bi <sub>2</sub> Sr <sub>2</sub> CaCu <sub>2</sub> O <sub>8</sub>     | I 4/m m m    | (139) | tetragonal body-centred   | 68188  |
| Ce <sub>2</sub> BiO <sub>2</sub>                                     | I 4/m m m    | (139) | tetragonal body-centred   | 9099   |
| Ce <sub>2</sub> SbO <sub>2</sub>                                     | I 4/m m m    | (139) | tetragonal body-centred   | 9100   |
| CePd <sub>2</sub> Si <sub>2</sub>                                    | I 4/m m m    | (139) | tetragonal body-centred   | 621852 |
| CePt <sub>2</sub> Si <sub>2</sub>                                    | I 4/m m m    | (139) | tetragonal body-centred   | 52895  |
| Cu <sub>2</sub> ErGe <sub>2</sub>                                    | I 4/m m m    | (139) | tetragonal body-centred   | 53251  |
| ErCu <sub>2</sub> Si <sub>2</sub>                                    | I 4/m m m    | (139) | tetragonal body-centred   | 106845 |
| Cu <sub>2</sub> GdSi <sub>2</sub>                                    | I 4/m m m    | (139) | tetragonal body-centred   | 64825  |

| Material                                                             | Space group | (#)   | Bravais lattice         | ICSD # |
|----------------------------------------------------------------------|-------------|-------|-------------------------|--------|
| Cu <sub>2</sub> HoGe <sub>2</sub>                                    | I 4/m m m   | (139) | tetragonal body-centred | 53270  |
| YCu <sub>2</sub> Ge <sub>2</sub>                                     | I 4/m m m   | (139) | tetragonal body-centred | 52764  |
| Cu <sub>2</sub> HoSi <sub>2</sub>                                    | I 4/m m m   | (139) | tetragonal body-centred | 53289  |
| NdCu <sub>2</sub> Si <sub>2</sub>                                    | I 4/m m m   | (139) | tetragonal body-centred | 106842 |
| Eu <sub>2</sub> (VO <sub>4</sub> )                                   | I 4/m m m   | (139) | tetragonal body-centred | 89000  |
| K <sub>2</sub> (NiF <sub>4</sub> )                                   | I 4/m m m   | (139) | tetragonal body-centred | 15576  |
| K <sub>2</sub> (NiF <sub>4</sub> )                                   | I 4/m m m   | (139) | tetragonal body-centred | 631720 |
| Rb <sub>2</sub> (NiF <sub>4</sub> )                                  | I 4/m m m   | (139) | tetragonal body-centred | 69682  |
| La <sub>2</sub> (NiO <sub>4</sub> )                                  | I 4/m m m   | (139) | tetragonal body-centred | 1179   |
| La <sub>2</sub> (NiO <sub>4</sub> )                                  | I 4/m m m   | (139) | tetragonal body-centred | 33536  |
| La <sub>2</sub> PdO <sub>4</sub>                                     | I 4/m m m   | (139) | tetragonal body-centred | 40262  |
| Sr <sub>2</sub> (MoO <sub>4</sub> )                                  | I 4/m m m   | (139) | tetragonal body-centred | 152123 |
| Sr <sub>2</sub> (RuO <sub>4</sub> )                                  | I 4/m m m   | (139) | tetragonal body-centred | 157401 |
| Sr <sub>2</sub> VO <sub>4</sub>                                      | I 4/m m m   | (139) | tetragonal body-centred | 72219  |
| Cs <sub>2</sub> AgF <sub>4</sub>                                     | I 4/m m m   | (139) | tetragonal body-centred | 16254  |
| K <sub>2</sub> CoF <sub>4</sub>                                      | I 4/m m m   | (139) | tetragonal body-centred | 33522  |
| Rb <sub>2</sub> CoF <sub>4</sub>                                     | I 4/m m m   | (139) | tetragonal body-centred | 69683  |
| Gd <sub>2</sub> (CuO <sub>4</sub> )                                  | I 4/m m m   | (139) | tetragonal body-centred | 41844  |
| In <sub>2</sub> CuO <sub>4</sub>                                     | I 4/m m m   | (139) | tetragonal body-centred | 39475  |
| La <sub>2</sub> (CuO <sub>4</sub> )                                  | I 4/m m m   | (139) | tetragonal body-centred | 41643  |
| Ba <sub>2</sub> CoF <sub>6</sub>                                     | I 4/m m m   | (139) | tetragonal body-centred | 21057  |
| Ba <sub>2</sub> NiF <sub>6</sub>                                     | I 4/m m m   | (139) | tetragonal body-centred | 21056  |
| Ba <sub>2</sub> (ZnF <sub>6</sub> )                                  | I 4/m m m   | (139) | tetragonal body-centred | 21054  |
| (Cu <sub>2</sub> S <sub>2</sub> )(Sr <sub>2</sub> CuO <sub>2</sub> ) | I 4/m m m   | (139) | tetragonal body-centred | 88423  |
| Ba <sub>2</sub> Cu <sub>3</sub> O <sub>4</sub> Br <sub>2</sub>       | I 4/m m m   | (139) | tetragonal body-centred | 36128  |
| Ba <sub>2</sub> Cu <sub>3</sub> O <sub>4</sub> Cl <sub>2</sub>       | I 4/m m m   | (139) | tetragonal body-centred | 355    |
| Ca <sub>3</sub> Cu <sub>2</sub> O <sub>4</sub> Br <sub>2</sub>       | I 4/m m m   | (139) | tetragonal body-centred | 69182  |
| Ca <sub>3</sub> Cu <sub>2</sub> O <sub>4</sub> Cl <sub>2</sub>       | I 4/m m m   | (139) | tetragonal body-centred | 69181  |
| La <sub>3</sub> Ni <sub>2</sub> O <sub>6</sub>                       | I 4/m m m   | (139) | tetragonal body-centred | 249209 |
| K <sub>3</sub> Ni <sub>2</sub> F <sub>7</sub>                        | I 4/m m m   | (139) | tetragonal body-centred | 33523  |
| Sr <sub>3</sub> V <sub>2</sub> O <sub>7</sub>                        | I 4/m m m   | (139) | tetragonal body-centred | 71320  |
| Sr <sub>3</sub> (V <sub>2</sub> O <sub>7</sub> )                     | I 4/m m m   | (139) | tetragonal body-centred | 71451  |
| K <sub>3</sub> Co <sub>2</sub> F <sub>7</sub>                        | I 4/m m m   | (139) | tetragonal body-centred | 33524  |
| K <sub>3</sub> Cu <sub>2</sub> F <sub>7</sub>                        | I 4/m m m   | (139) | tetragonal body-centred | 15373  |
| La <sub>4</sub> Ni <sub>3</sub> O <sub>8</sub>                       | I 4/m m m   | (139) | tetragonal body-centred | 173372 |
| K <sub>5</sub> Te <sub>3</sub>                                       | I 4/m       | (87)  | tetragonal body-centred | 96743  |
| CaSmCuO <sub>3</sub> Cl                                              | P 4/n m m Z | (129) | tetragonal primitive    | 86428  |
| HgBa <sub>2</sub> CaCu <sub>2</sub> O <sub>6</sub>                   | P 4/m m m   | (123) | tetragonal primitive    | 75725  |
| HgBa <sub>2</sub> CaCu <sub>2</sub> O <sub>6</sub>                   | P 4/m m m   | (123) | tetragonal primitive    | 83087  |
| TlYBa <sub>2</sub> Cu <sub>2</sub> O <sub>7</sub>                    | P 4/m m m   | (123) | tetragonal primitive    | 74163  |
| TlCaSr <sub>2</sub> Cu <sub>2</sub> O <sub>7</sub>                   | P 4/m m m   | (123) | tetragonal primitive    | 74165  |
| NdBa <sub>2</sub> Cu <sub>2</sub> NbO <sub>8</sub>                   | P 4/m m m   | (123) | tetragonal primitive    | 44255  |
| Sr <sub>2</sub> CoO <sub>3</sub> Cl                                  | P 4/n m m Z | (129) | tetragonal primitive    | 91750  |
| HgBa <sub>2</sub> CuO <sub>4</sub>                                   | P 4/m m m   | (123) | tetragonal primitive    | 75720  |
| Sr <sub>2</sub> CuO <sub>2</sub> (CO <sub>3</sub> )                  | P 4 21 2    | (90)  | tetragonal primitive    | 83096  |
| KCeSe <sub>4</sub>                                                   | P 4/n b m Z | (125) | tetragonal primitive    | 67656  |
| NdLi <sub>2</sub> Sb <sub>2</sub>                                    | P 4/n m m Z | (129) | tetragonal primitive    | 36020  |
| HgBa <sub>2</sub> Ca <sub>2</sub> Cu <sub>3</sub> O <sub>8</sub>     | P 4/m m m   | (123) | tetragonal primitive    | 75730  |
| HoBa <sub>2</sub> Cu <sub>3</sub> O <sub>6</sub>                     | P 4/m m m   | (123) | tetragonal primitive    | 68047  |
| LuBa <sub>2</sub> Cu <sub>3</sub> O <sub>6</sub>                     | P 4/m m m   | (123) | tetragonal primitive    | 98113  |
| NdBa <sub>2</sub> Cu <sub>3</sub> O <sub>6</sub>                     | P 4/m m m   | (123) | tetragonal primitive    | 83074  |
| Cs(Cu <sub>4</sub> Se <sub>3</sub> )                                 | P 4/m m m   | (123) | tetragonal primitive    | 75196  |
| KCu <sub>4</sub> S <sub>3</sub>                                      | P 4/m m m   | (123) | tetragonal primitive    | 23336  |
| KCu <sub>4</sub> Se <sub>3</sub>                                     | P 4/m m m   | (123) | tetragonal primitive    | 280072 |

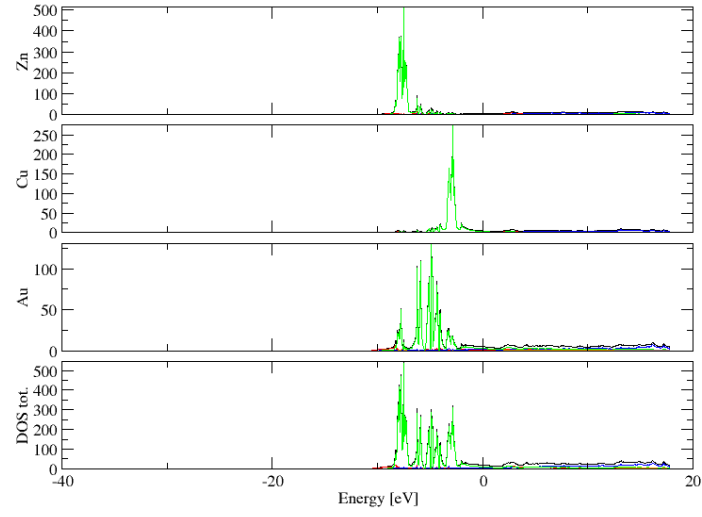

FIG. 1: (Color online) PDOS of AuCuZn<sub>2</sub> (ICSD #150571). The *s*-, *p*- and *d*-projected states are in red, blue and green, respectively. AuCuZn<sub>2</sub> crystallizes in space group *Fm*  $\bar{3}$  *m* (#225), in a cubic face-centred structure.

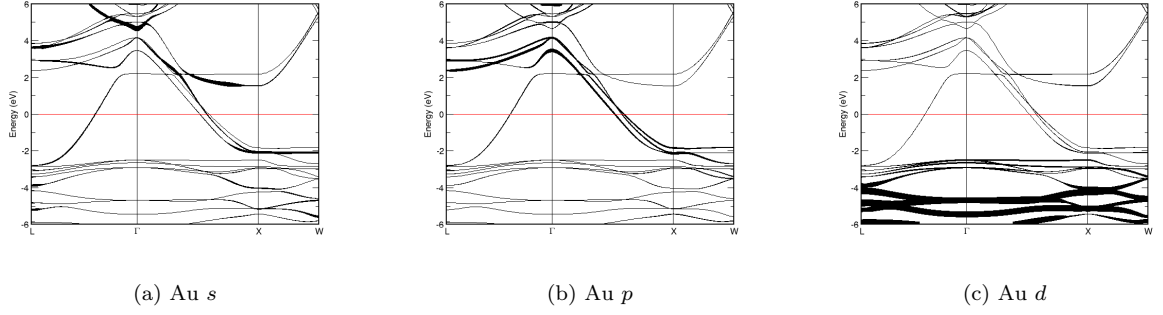

FIG. 2: Fat band representation of Au in AuCuZn<sub>2</sub>

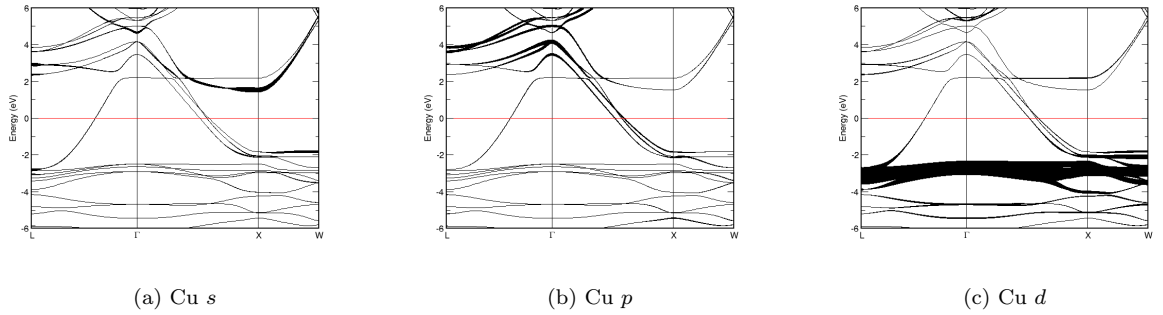

FIG. 3: Fat band representation of Cu in AuCuZn<sub>2</sub>



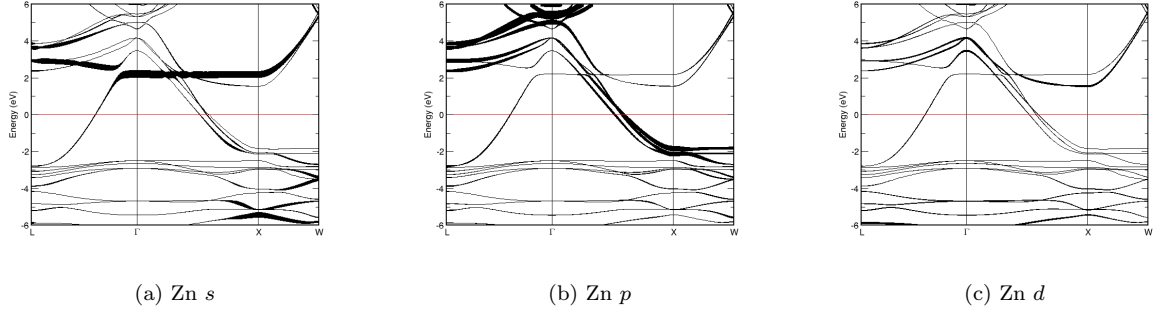

FIG. 4: Fat band representation of Zn in AuCuZn<sub>2</sub>

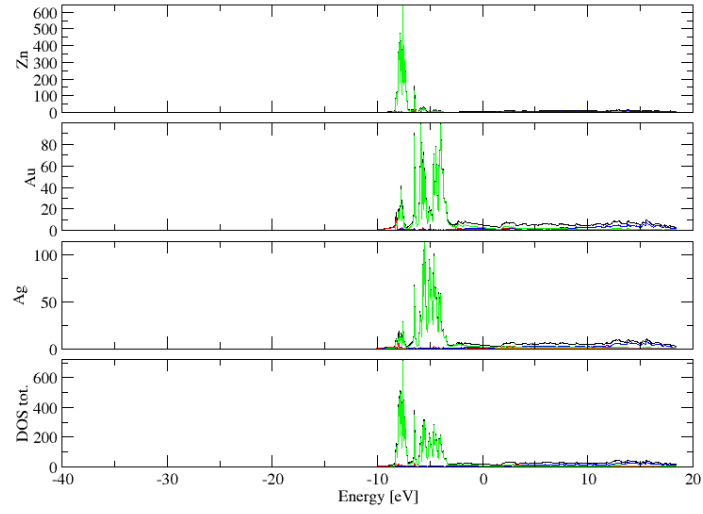

FIG. 5: (Color online) PDOS of AgAuZn<sub>2</sub> (ICSD #604792). The *s*-, *p*- and *d*-projected states are in red, blue and green, respectively. AgAuZn<sub>2</sub> crystallizes in space group Fm-3m (#225), in a cubic face-centred structure.

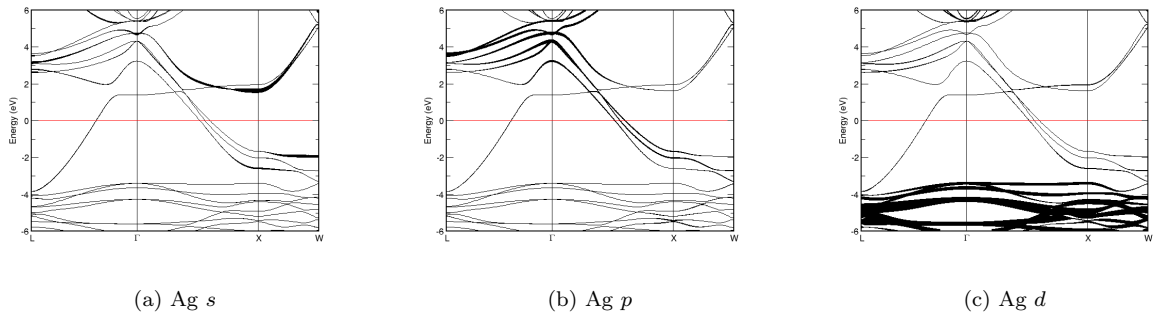

FIG. 6: Fat band representation of Ag in AgAuZn<sub>2</sub>

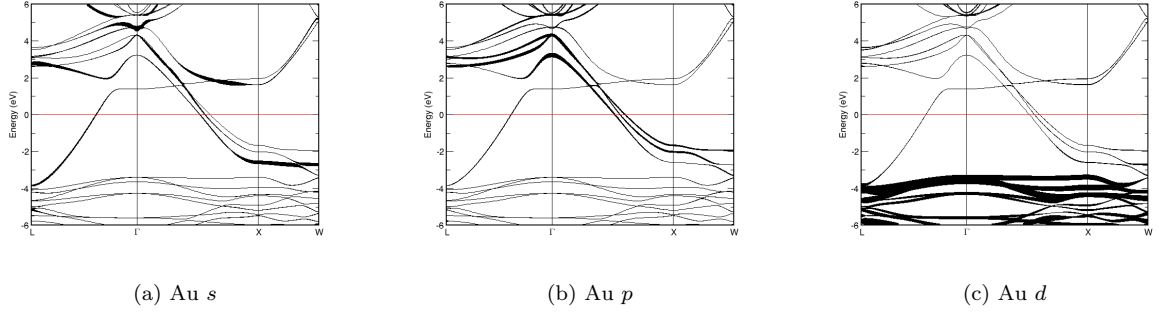

FIG. 7: Fat band representation of Au in AgAuZn<sub>2</sub>

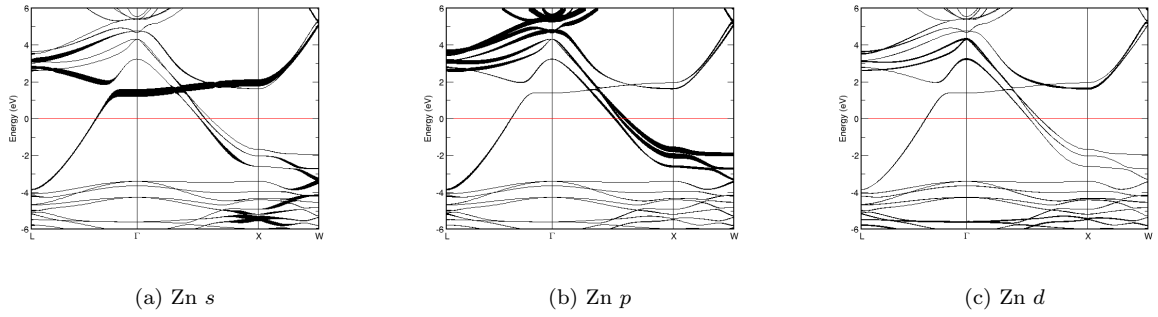

FIG. 8: Fat band representation of Zn in AgAuZn<sub>2</sub>

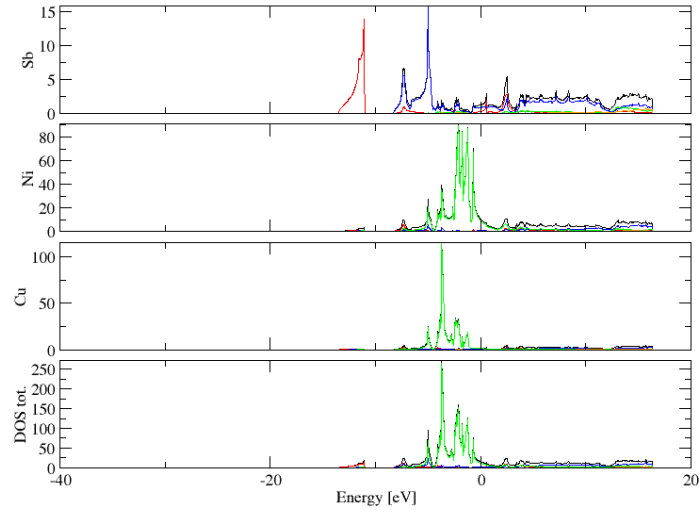

FIG. 9: (Color online) PDOS of CuNi<sub>2</sub>Sb (ICSD #53320). The *s*-, *p*- and *d*-projected states are in red, blue and green, respectively. CuNi<sub>2</sub>Sb crystallizes in space group *Fm*  $\bar{3}$  *m* (#225), in a cubic face-centred structure.

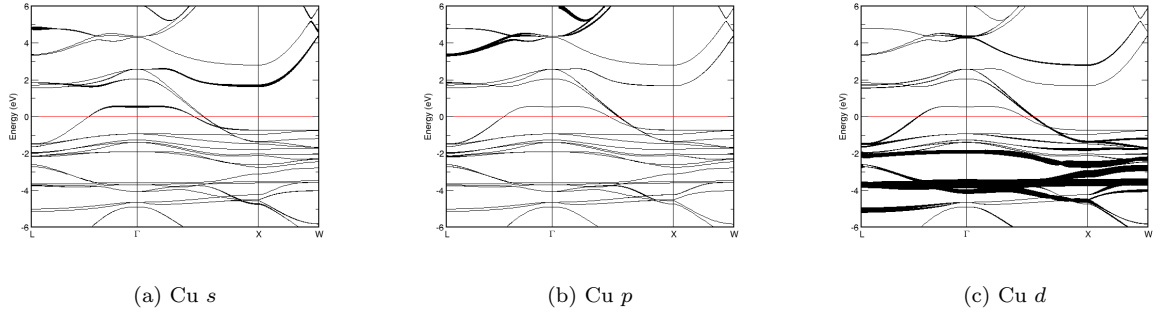

FIG. 10: Fat band representation of Cu in CuNi<sub>2</sub>Sb

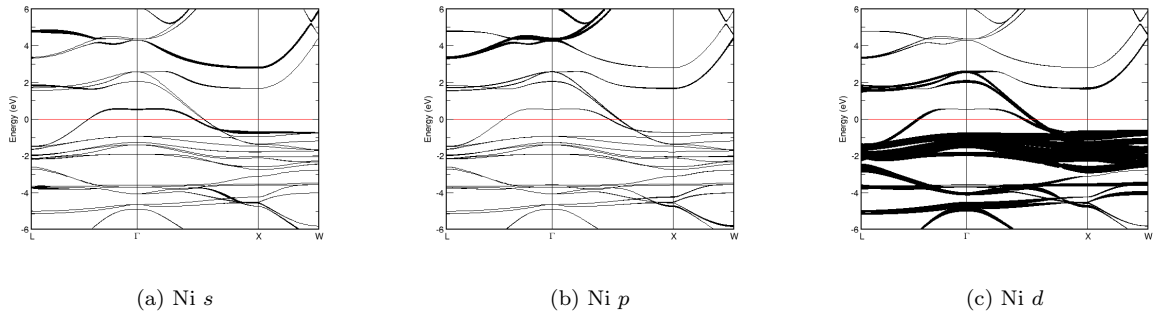

FIG. 11: Fat band representation of Ni in CuNi<sub>2</sub>Sb

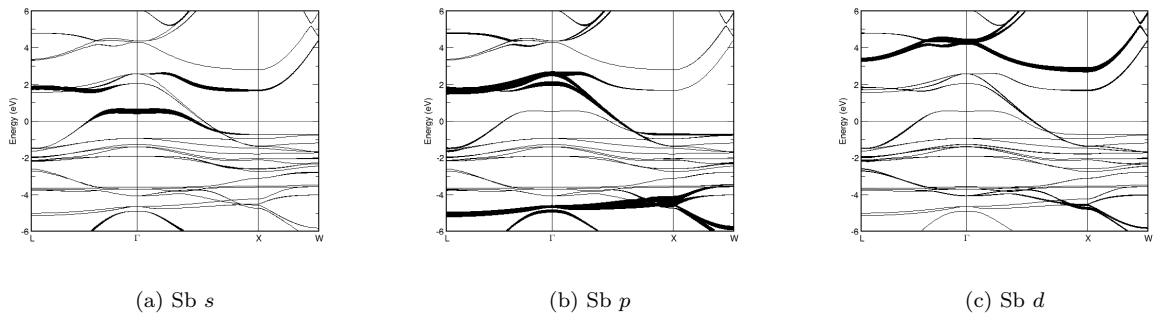

FIG. 12: Fat band representation of Sb in CuNi<sub>2</sub>Sb

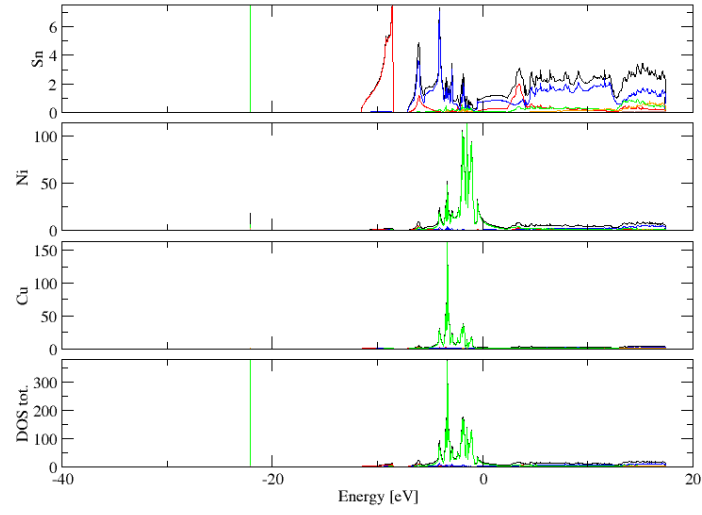

FIG. 13: (Color online) PDOS of  $\text{CuNi}_2\text{Sn}$  (ICSD #103068). The  $s$ -,  $p$ - and  $d$ -projected states are in red, blue and green, respectively.  $\text{CuNi}_2\text{Sn}$  crystallizes in space group  $Fm\bar{3}m$  (#225), in a cubic face-centred structure.

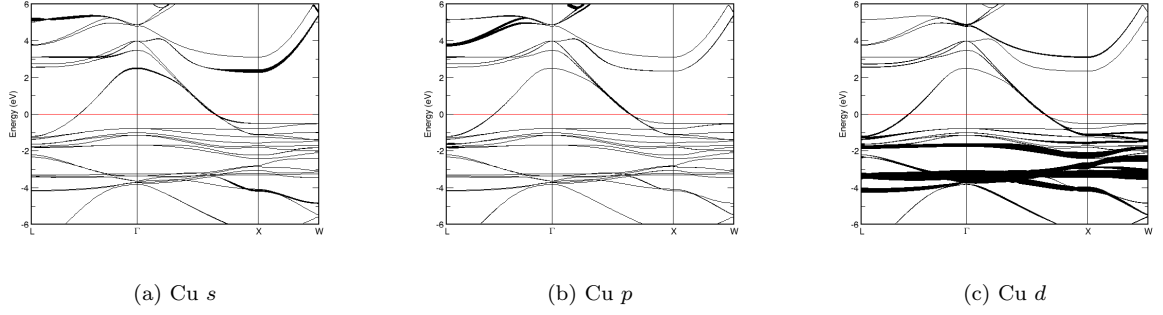

FIG. 14: Fat band representation of Cu in  $\text{CuNi}_2\text{Sn}$

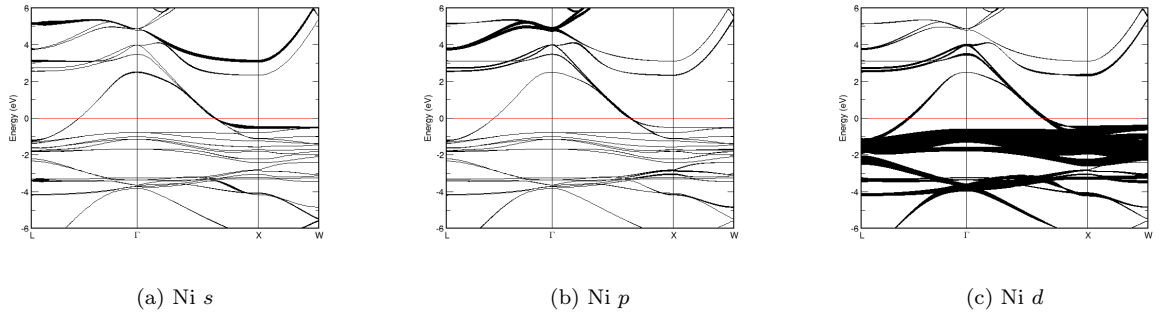

FIG. 15: Fat band representation of Ni in  $\text{CuNi}_2\text{Sn}$

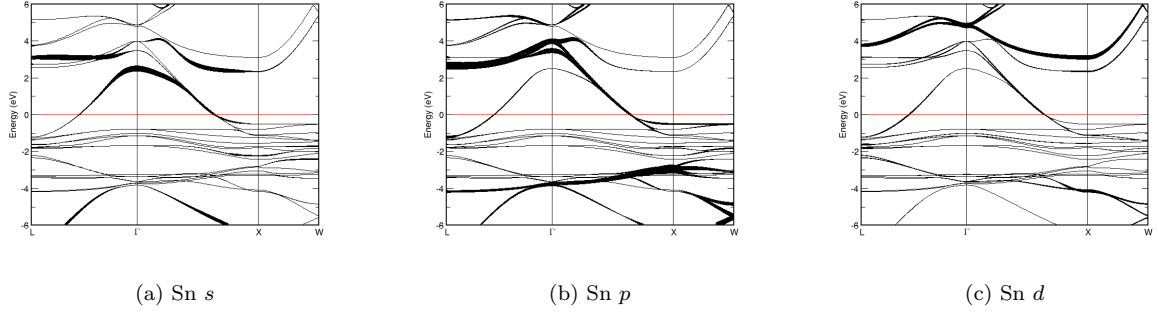

FIG. 16: Fat band representation of Sn in  $\text{CuNi}_2\text{Sn}$

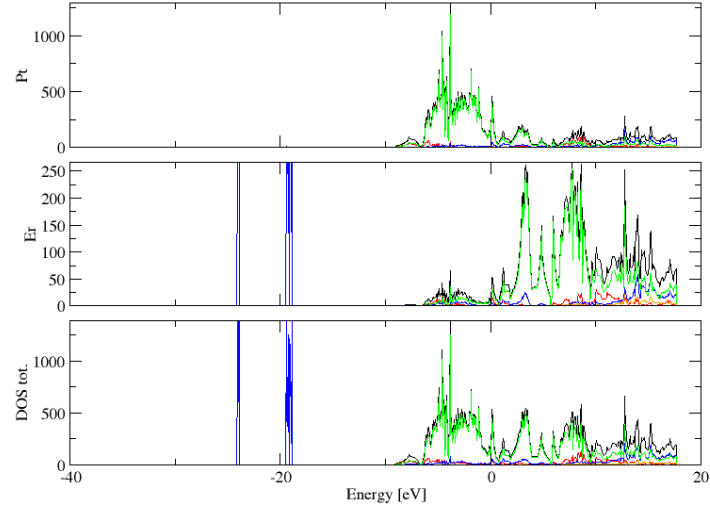

FIG. 17: (Color online) PDOS of  $\text{ErPt}_2$  (ICSD #103287). The *s*-, *p*- and *d*-projected states are in red, blue and green, respectively.  $\text{ErPt}_2$  crystallizes in space group  $Fm\bar{3}m$  (#227), in a cubic face-centred structure.

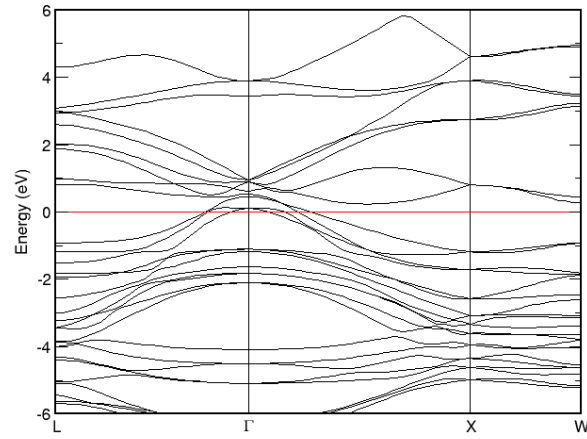

(a) *E vs. k*

FIG. 18: Band structure of  $\text{ErPt}_2$

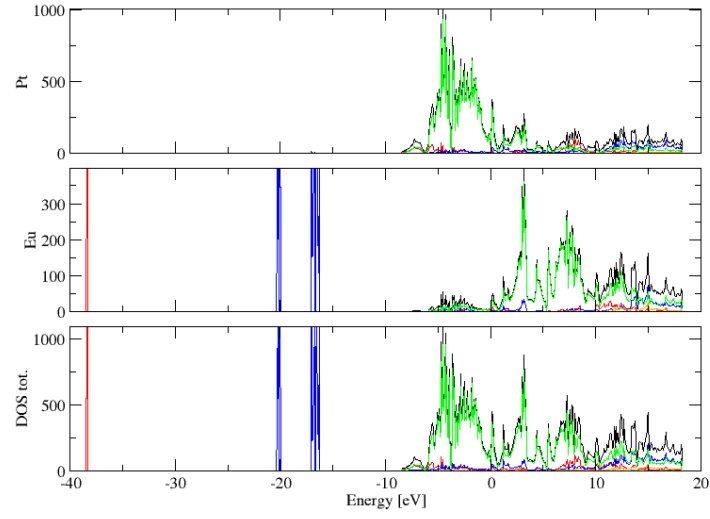

FIG. 19: (Color online) PDOS of  $\text{EuPt}_2$  (ICSD #103430). The  $s$ -,  $p$ - and  $d$ -projected states are in red, blue and green, respectively.  $\text{EuPt}_2$  crystallizes in space group  $F d -3 m S$  (#227), in a cubic face-centred structure.

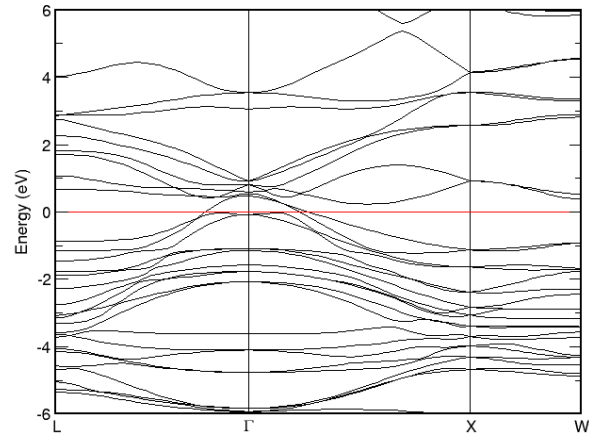

(a)  $E$  vs.  $k$

FIG. 20: Band structure of  $\text{EuPt}_2$

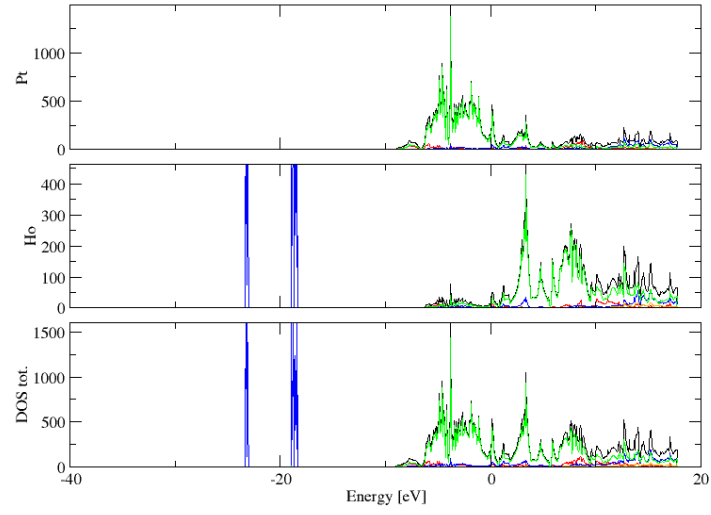

FIG. 21: (Color online) PDOS of  $\text{HoPt}_2$  (ICSD #104441). The  $s$ -,  $p$ - and  $d$ -projected states are in red, blue and green, respectively.  $\text{HoPt}_2$  crystallizes in space group  $F d -3 m S$  (#227), in a cubic face-centred structure.

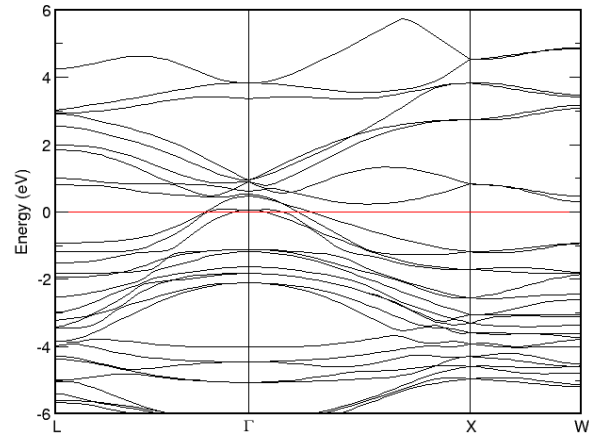

(a)  $E$  vs.  $k$

FIG. 22: Band structure of  $\text{HoPt}_2$

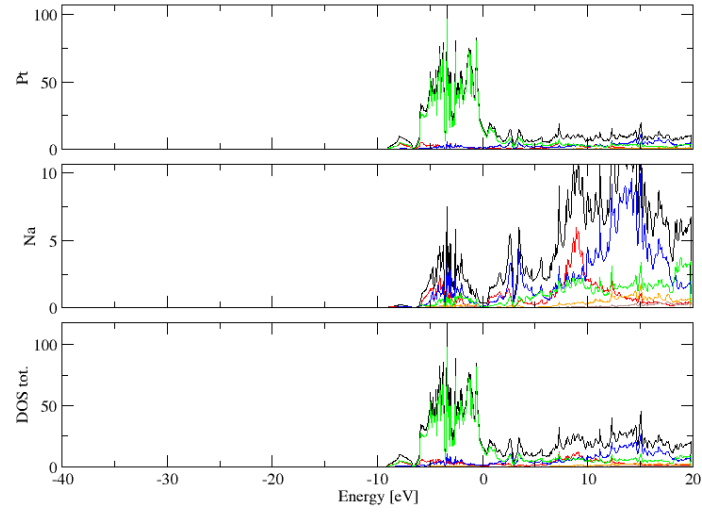

FIG. 23: (Color online) PDOS of  $\text{NaPt}_2$  (ICSD #644945). The  $s$ -,  $p$ - and  $d$ -projected states are in red, blue and green, respectively.  $\text{NaPt}_2$  crystallizes in space group  $F\bar{3}mS$  (#227), in a cubic face-centred structure.

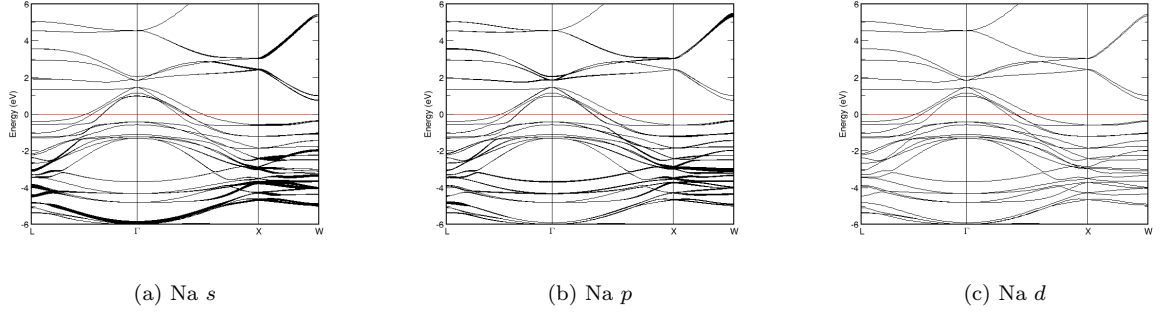

FIG. 24: Fat band representation of Na in  $\text{NaPt}_2$

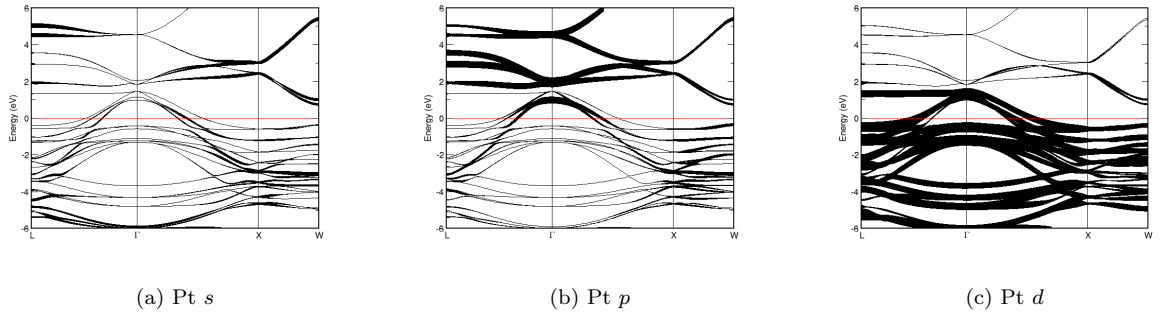

FIG. 25: Fat band representation of Pt in  $\text{NaPt}_2$



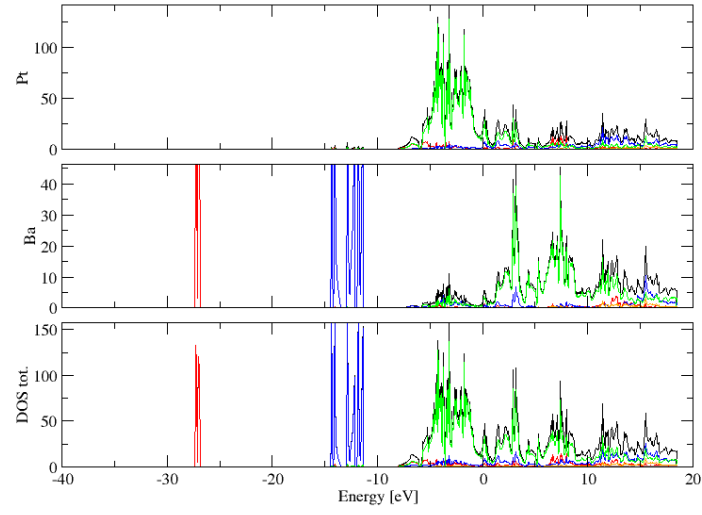

FIG. 26: (Color online) PDOS of BaPt<sub>2</sub> (ICSD #616039). The *s*-, *p*- and *d*-projected states are in red, blue and green, respectively. BaPt<sub>2</sub> crystallizes in space group  $Fm\bar{3}m$  (#227), in a cubic face-centred structure.

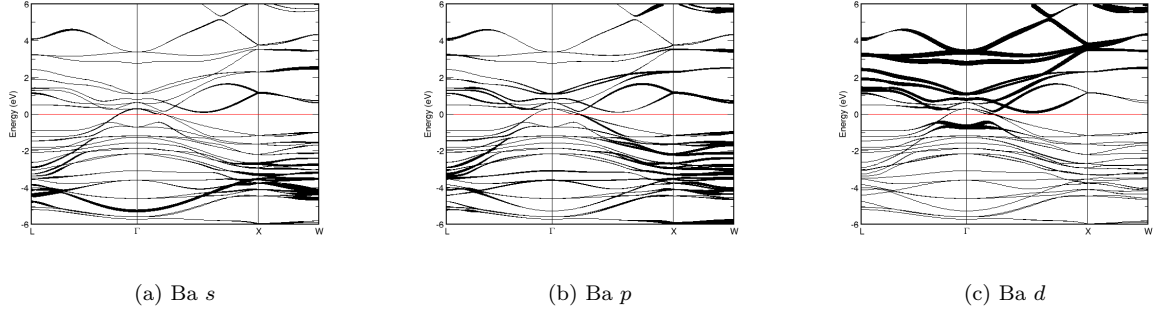

FIG. 27: Fat band representation of Ba in BaPt<sub>2</sub>

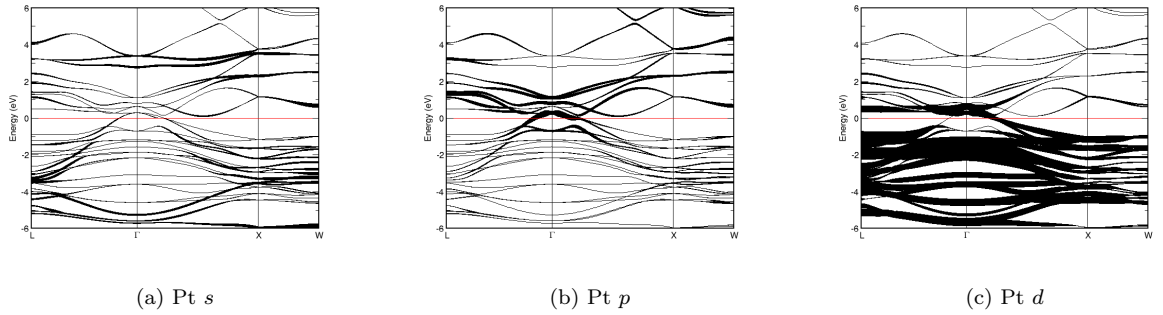

FIG. 28: Fat band representation of Pt in BaPt<sub>2</sub>

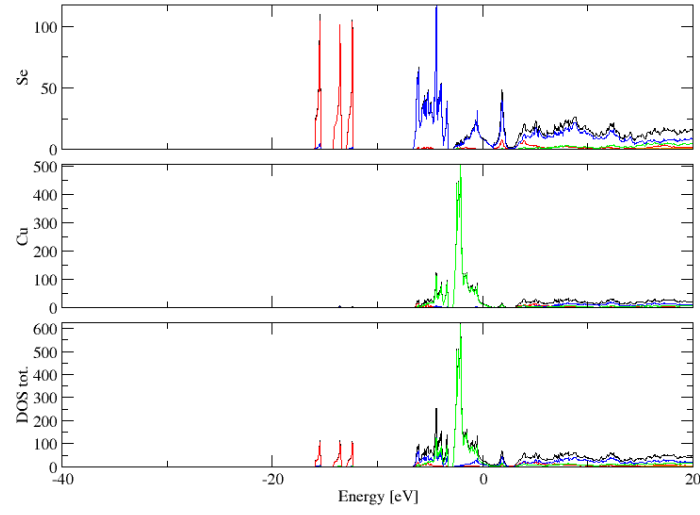

FIG. 29: (Color online) PDOS of CuSe (ICSD #240). The  $s$ -,  $p$ - and  $d$ -projected states are in red, blue and green, respectively. CuSe crystallizes in space group  $P 63/m m c$  (#194), in a hexagonal primitive structure.

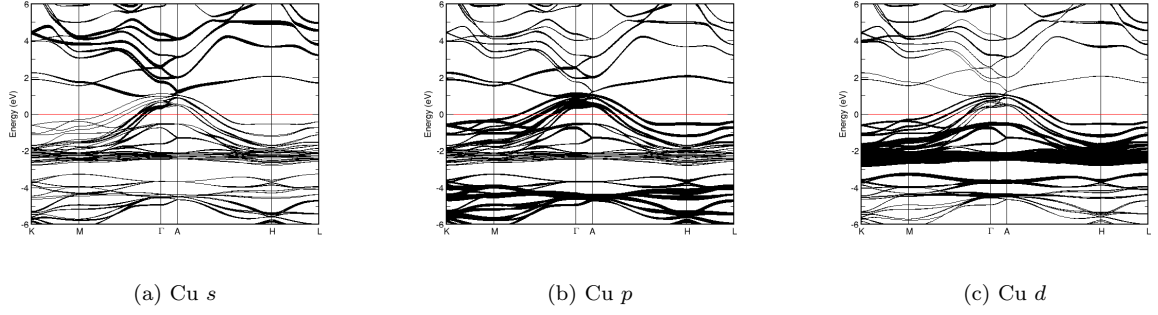

FIG. 30: Fat band representation of Cu in CuSe

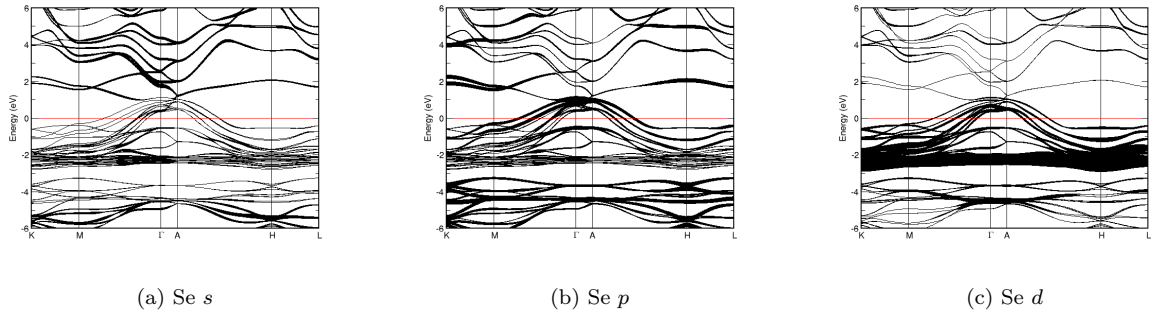

FIG. 31: Fat band representation of Se in CuSe

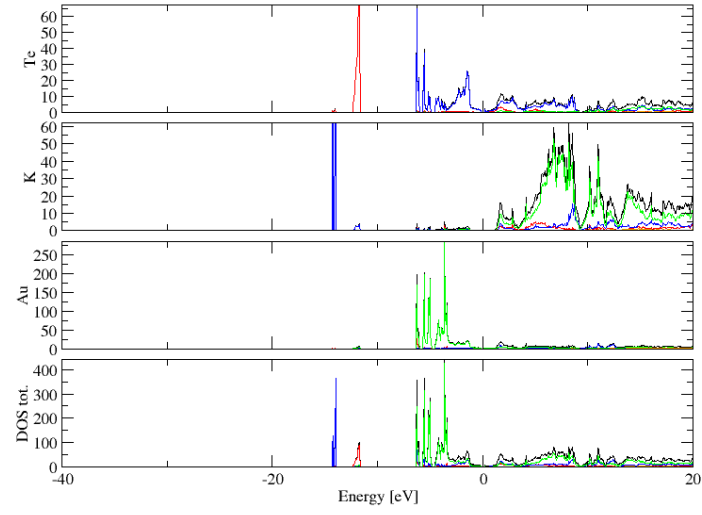

FIG. 32: (Color online) PDOS of KAuTe (ICSD #40165). The  $s$ -,  $p$ - and  $d$ -projected states are in red, blue and green, respectively. KAuTe crystallizes in space group  $P 63/m m c$  (#194), in a hexagonal primitive structure.

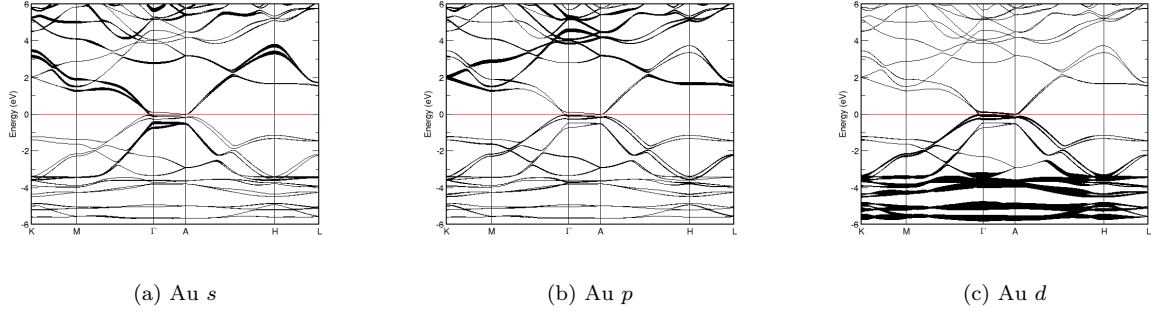

FIG. 33: Fat band representation of Au in KAuTe

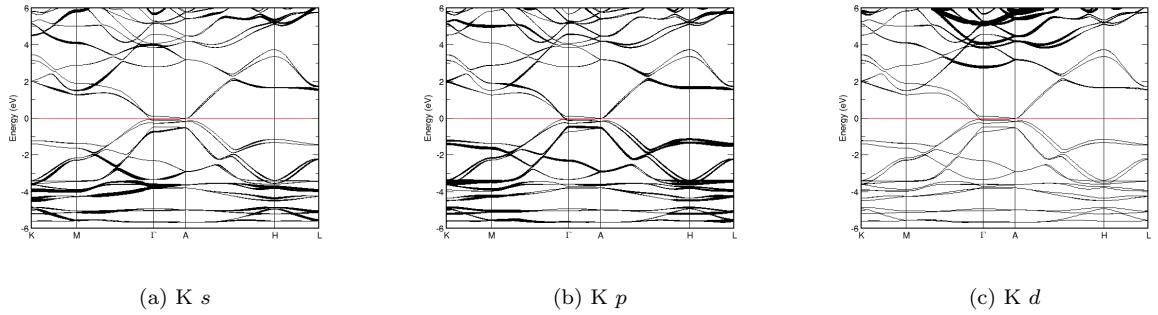

FIG. 34: Fat band representation of K in KAuTe

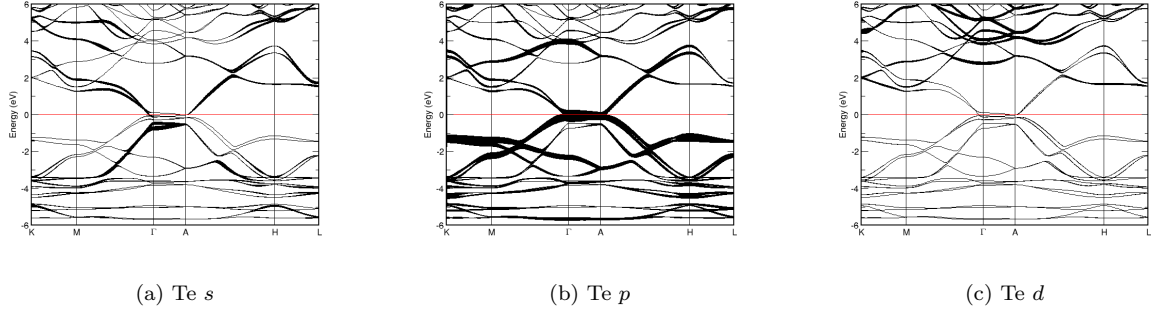

FIG. 35: Fat band representation of Te in KAuTe

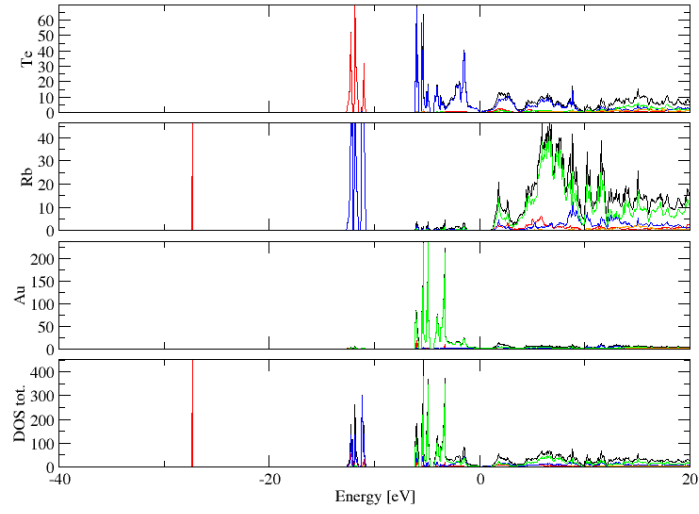FIG. 36: (Color online) PDOS of RbAuTe (ICSD #75026). The  $s$ -,  $p$ - and  $d$ -projected states are in red, blue and green, respectively. RbAuTe crystallizes in space group  $P 63/m m c$  (#194), in a hexagonal primitive structure.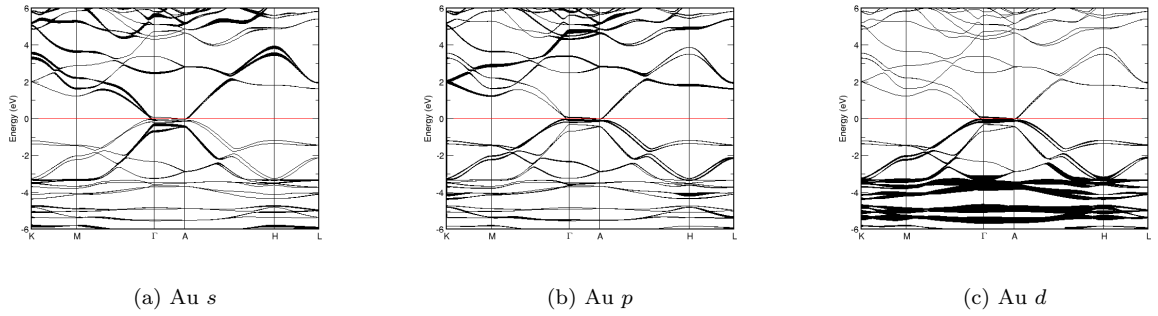

FIG. 37: Fat band representation of Au in RbAuTe

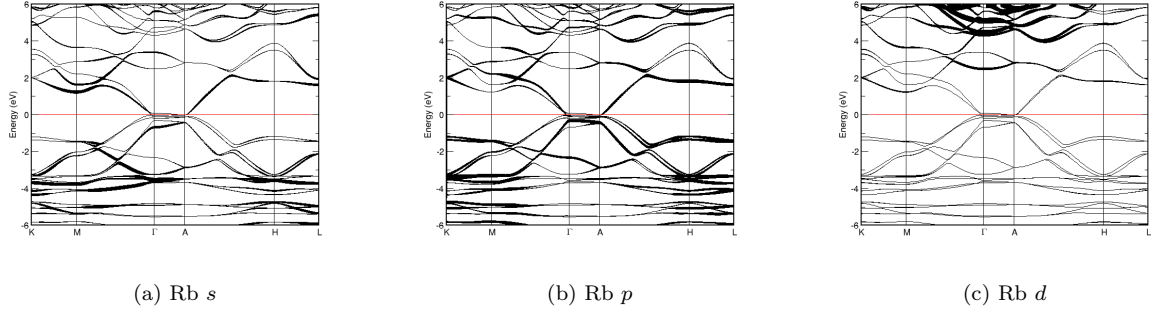

FIG. 38: Fat band representation of Rb in RbAuTe

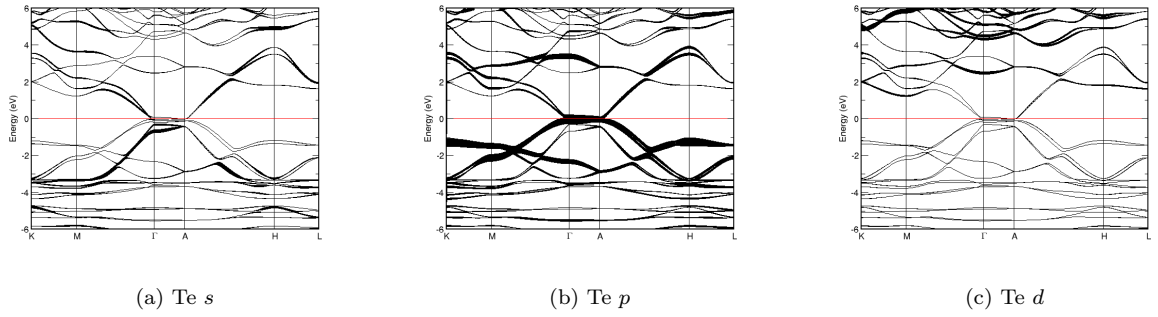

FIG. 39: Fat band representation of Te in RbAuTe

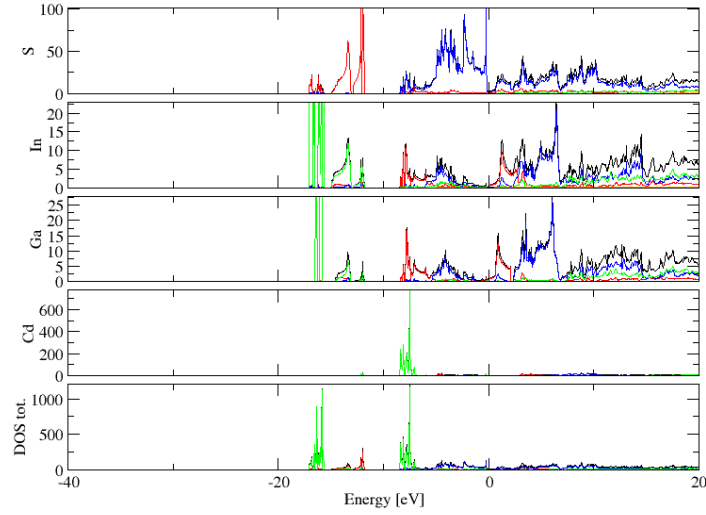FIG. 40: (Color online) PDOS of CdInGaS<sub>4</sub> (ICSD #20785). The  $s$ -,  $p$ - and  $d$ -projected states are in red, blue and green, respectively. CdInGaS<sub>4</sub> crystallizes in space group  $P\bar{3}m1$  (#164), in a hexagonal primitive structure.

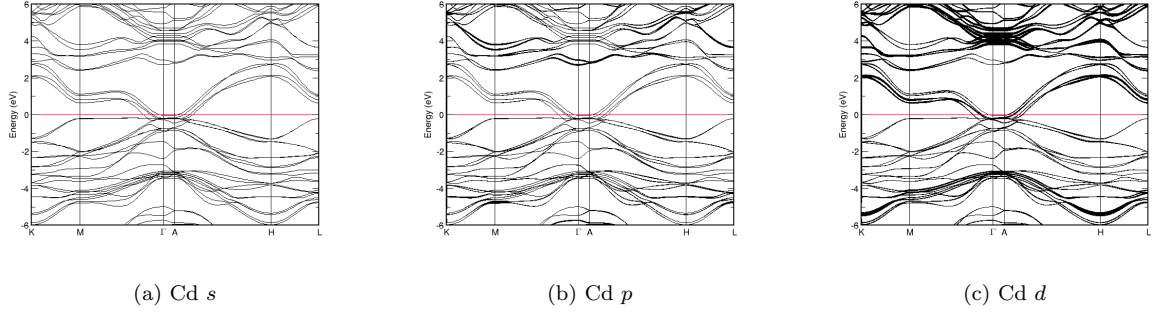FIG. 41: Fat band representation of Cd in CdInGaS<sub>4</sub>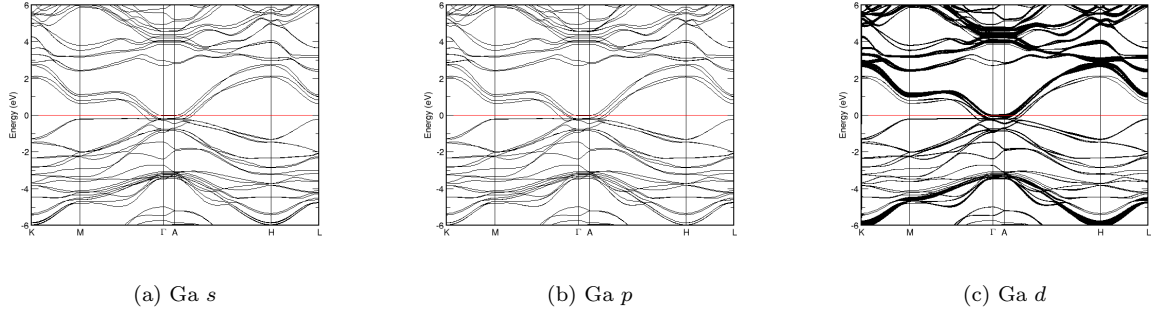FIG. 42: Fat band representation of Ga in CdInGaS<sub>4</sub>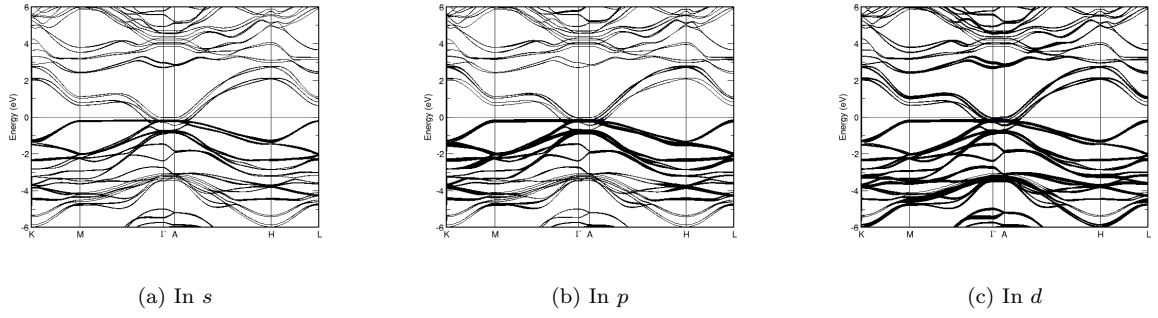FIG. 43: Fat band representation of In in CdInGaS<sub>4</sub>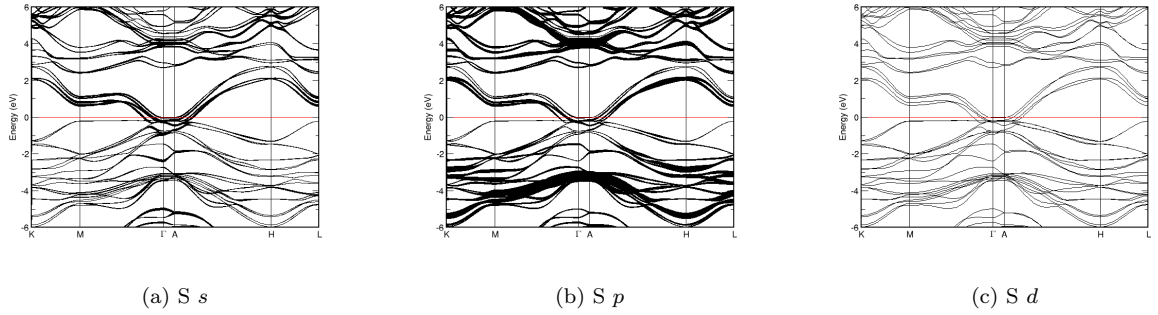FIG. 44: Fat band representation of S in CdInGaS<sub>4</sub>

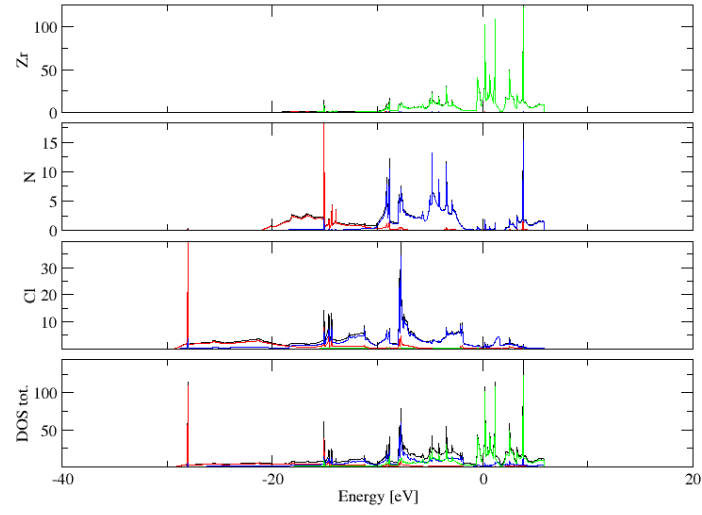

FIG. 45: (Color online) PDOS of ZrNCl (ICSD #25506). The  $s$ -,  $p$ - and  $d$ -projected states are in red, blue and green, respectively. ZrNCl crystallizes in space group  $P\bar{3}m1$  (#164), in a hexagonal primitive structure.

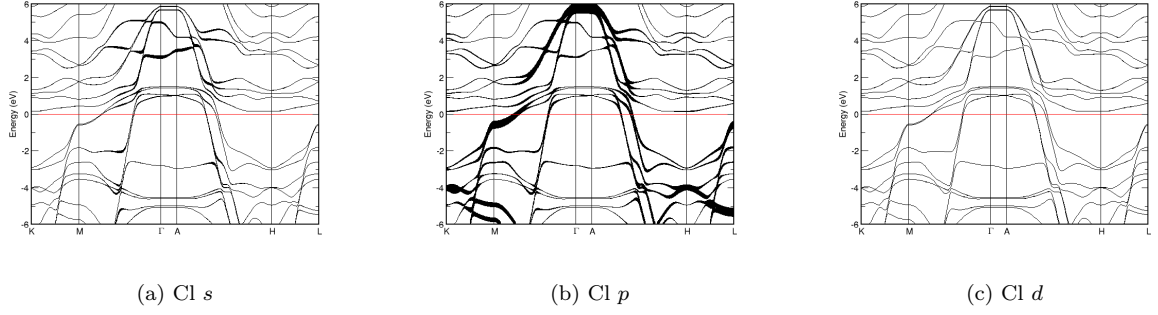

FIG. 46: Fat band representation of Cl in ZrNCl

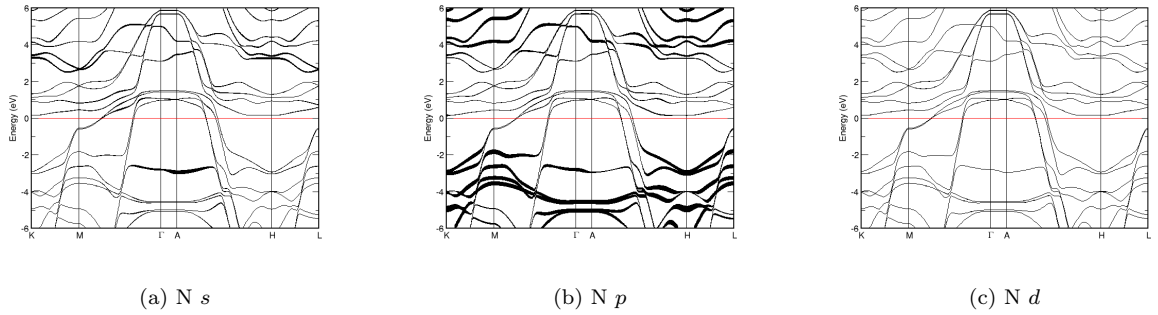

FIG. 47: Fat band representation of N in ZrNCl

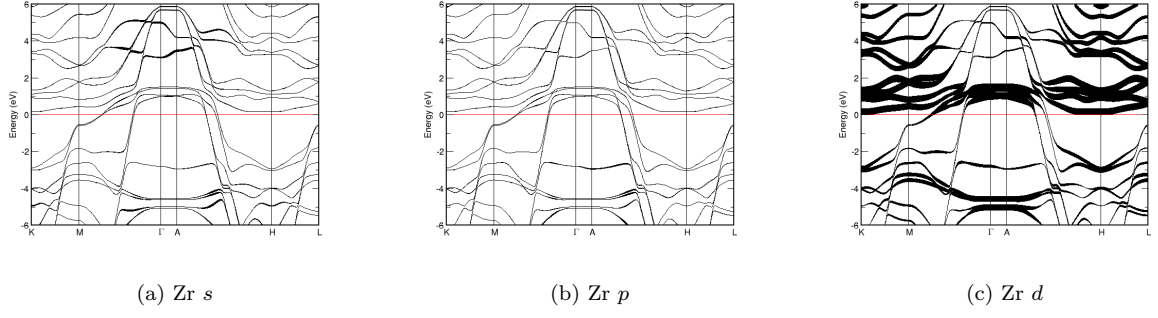

FIG. 48: Fat band representation of Zr in ZrNCl

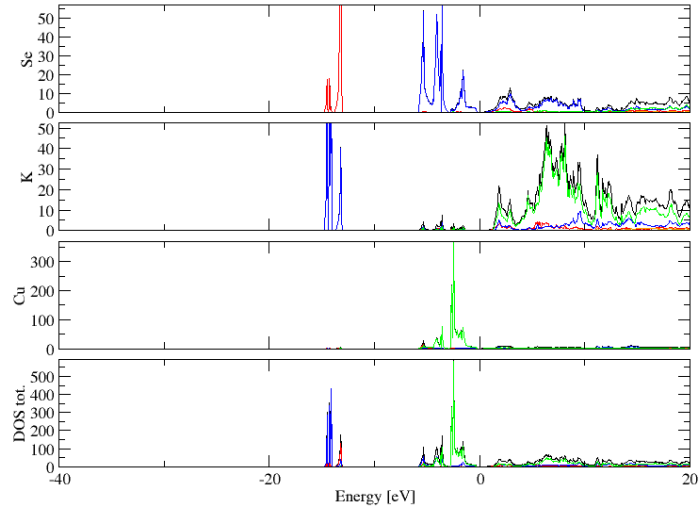FIG. 49: (Color online) PDOS of KCuSe (ICSD #12157). The  $s$ -,  $p$ - and  $d$ -projected states are in red, blue and green, respectively. KCuSe crystallizes in space group  $P 6_3/m m c$  (#194), in a hexagonal primitive structure.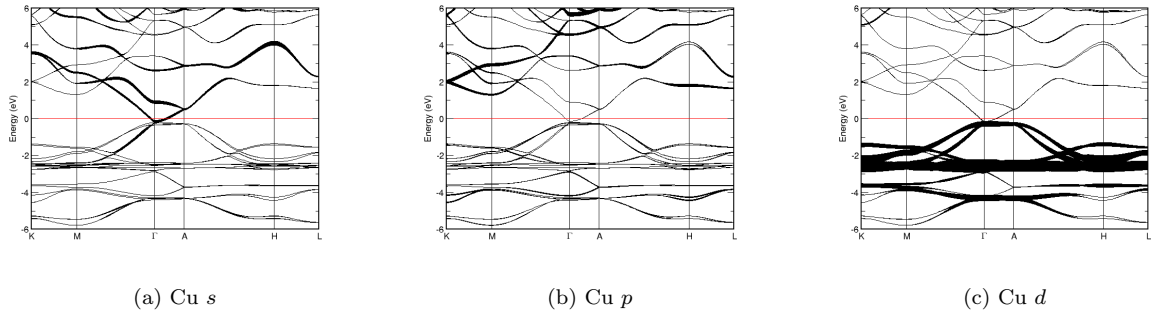

FIG. 50: Fat band representation of Cu in KCuSe



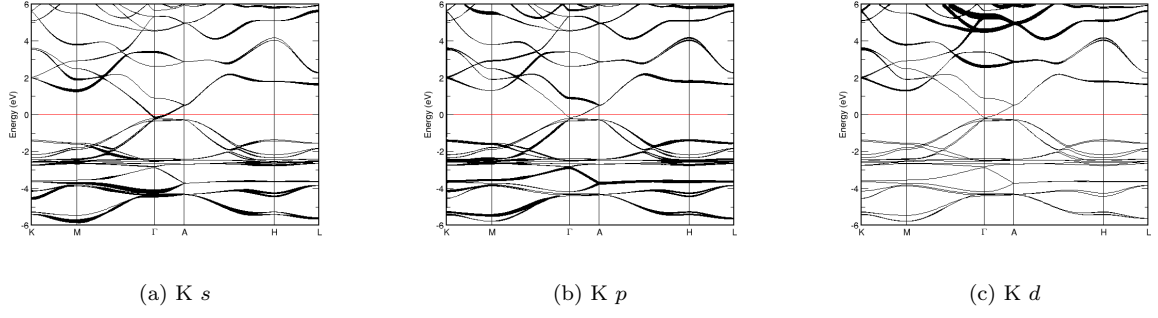

FIG. 51: Fat band representation of K in KCuSe

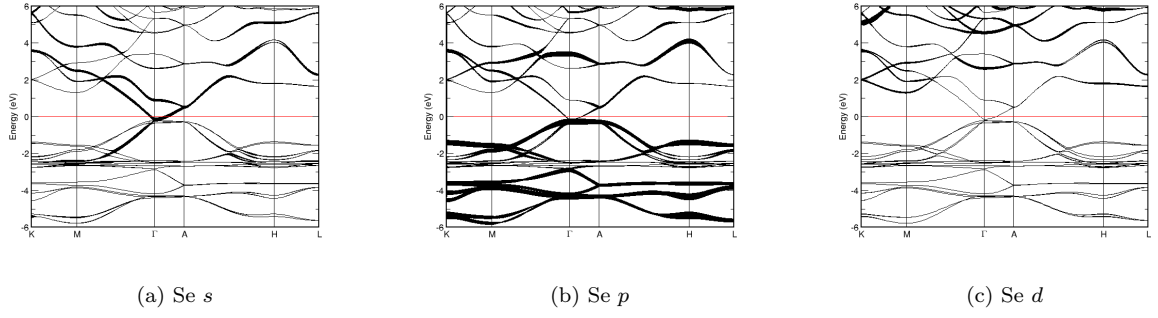

FIG. 52: Fat band representation of Se in KCuSe

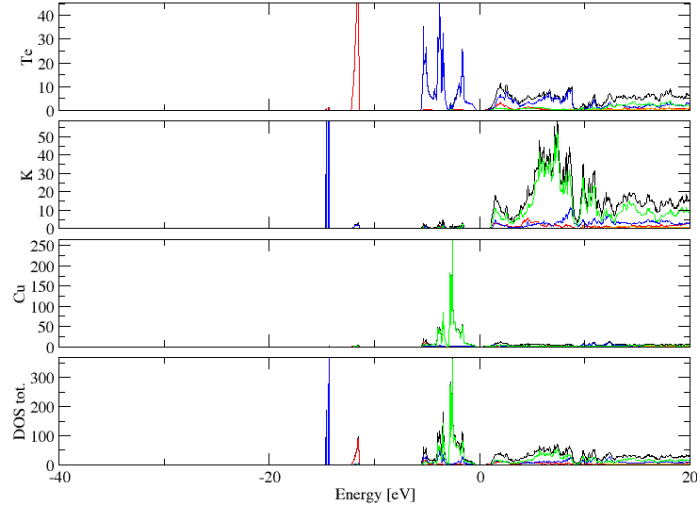FIG. 53: (Color online) PDOS of KCuTe (ICSD #12158). The  $s$ -,  $p$ - and  $d$ -projected states are in red, blue and green, respectively. KCuTe crystallizes in space group P 63/m m c (#194), in a hexagonal primitive structure.

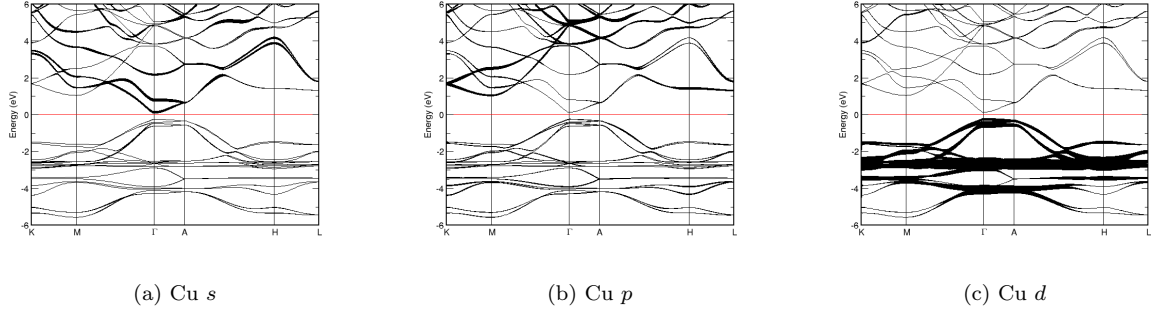

FIG. 54: Fat band representation of Cu in KCuTe

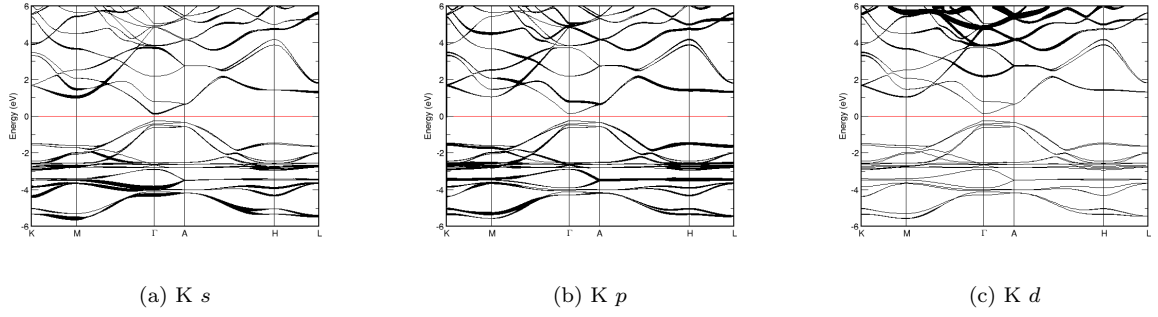

FIG. 55: Fat band representation of K in KCuTe

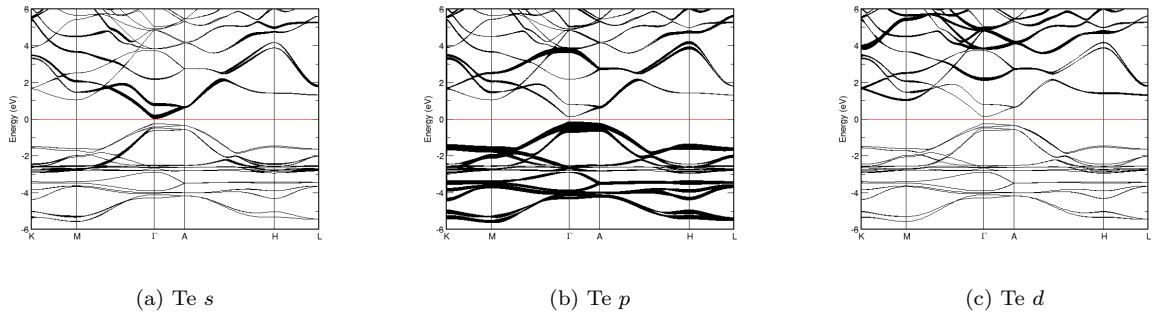

FIG. 56: Fat band representation of Te in KCuTe

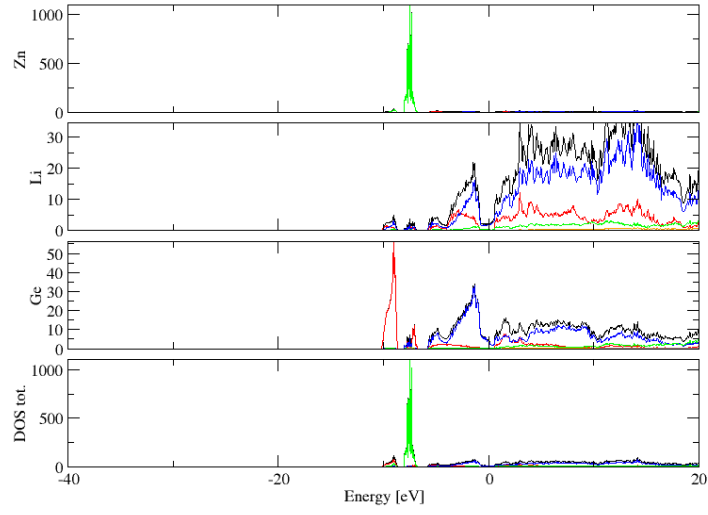

FIG. 57: (Color online) PDOS of  $\text{Li}_2\text{ZnGe}$  (ICSD #53678). The  $s$ -,  $p$ - and  $d$ -projected states are in red, blue and green, respectively.  $\text{Li}_2\text{ZnGe}$  crystallizes in space group  $P-3m1$  (#164), in a hexagonal primitive structure.

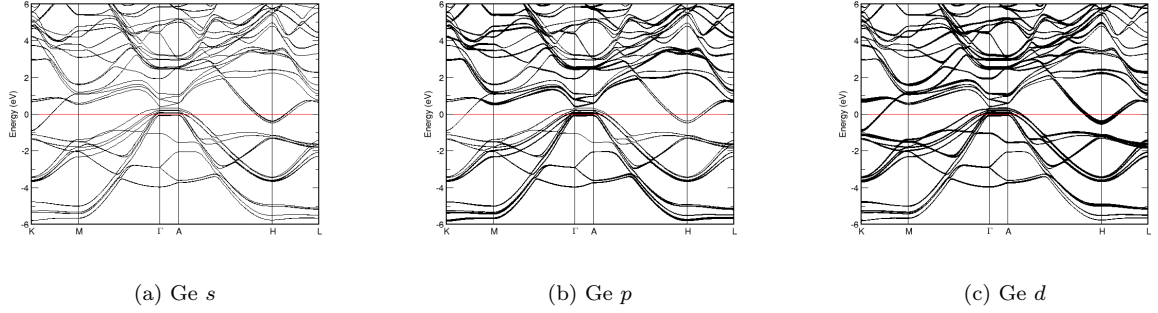

FIG. 58: Fat band representation of Ge in  $\text{Li}_2\text{ZnGe}$

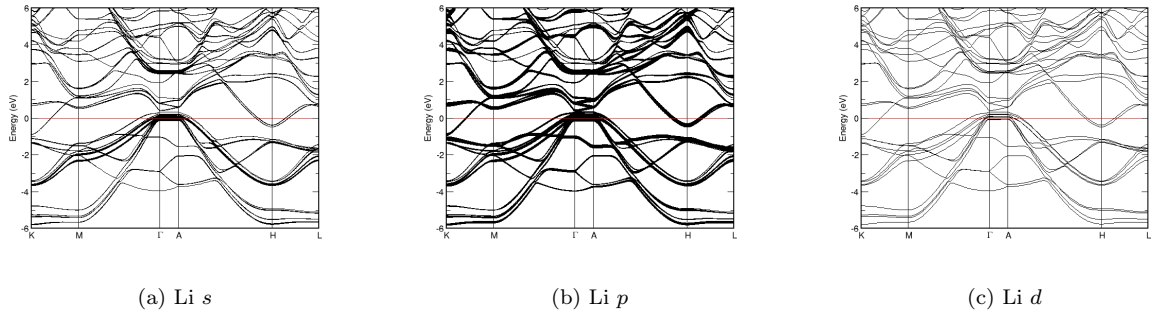

FIG. 59: Fat band representation of Li in  $\text{Li}_2\text{ZnGe}$

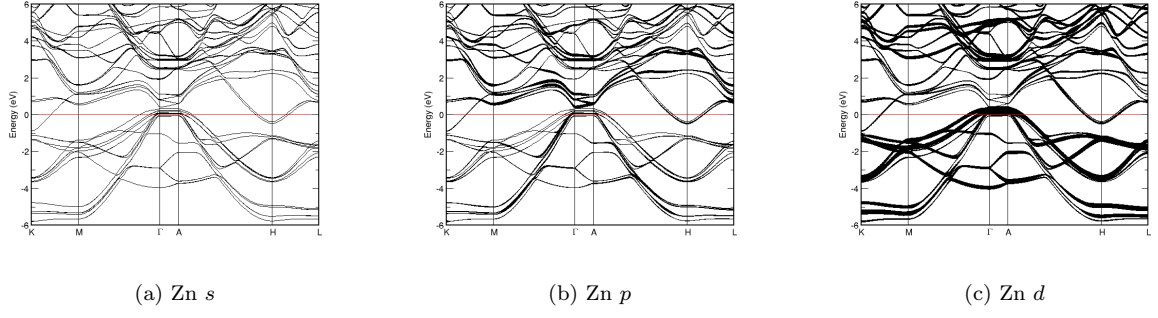FIG. 60: Fat band representation of Zn in  $\text{Li}_2\text{ZnGe}$ 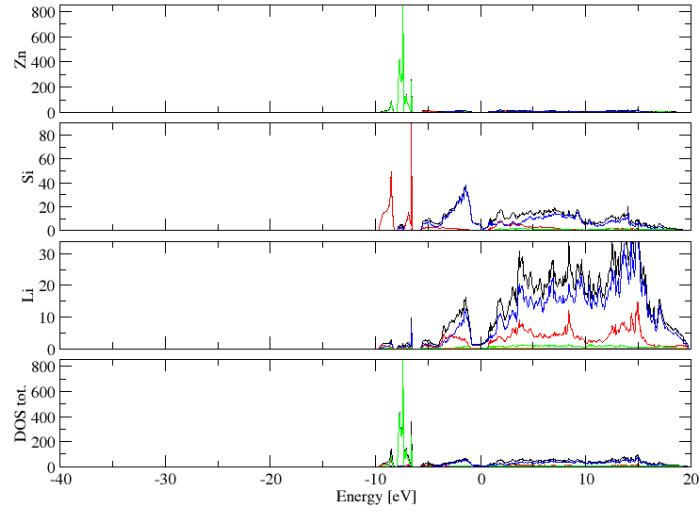FIG. 61: (Color online) PDOS of  $\text{Li}_2\text{ZnSi}$  (ICSD #16221). The  $s$ -,  $p$ - and  $d$ -projected states are in red, blue and green, respectively.  $\text{Li}_2\text{ZnSi}$  crystallizes in space group  $P-3m1$  (#164), in a hexagonal primitive structure.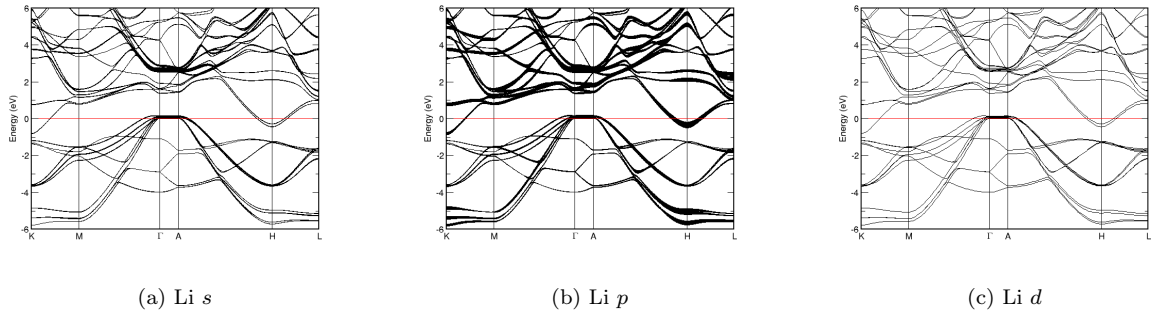FIG. 62: Fat band representation of Li in  $\text{Li}_2\text{ZnSi}$

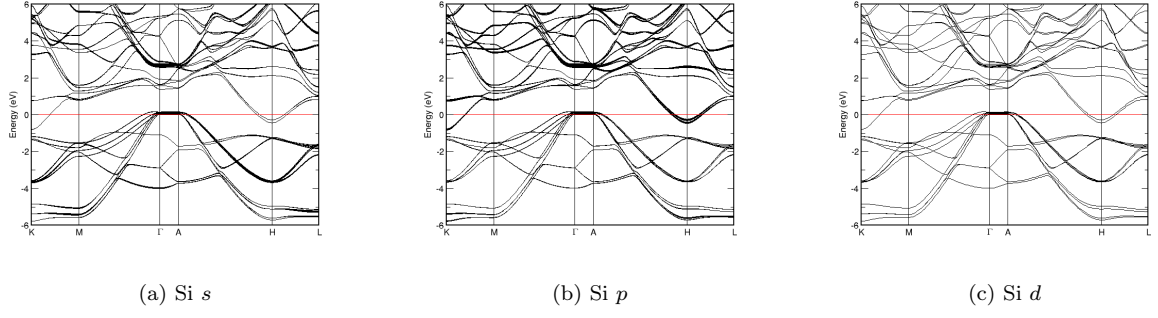FIG. 63: Fat band representation of Si in  $\text{Li}_2\text{ZnSi}$ 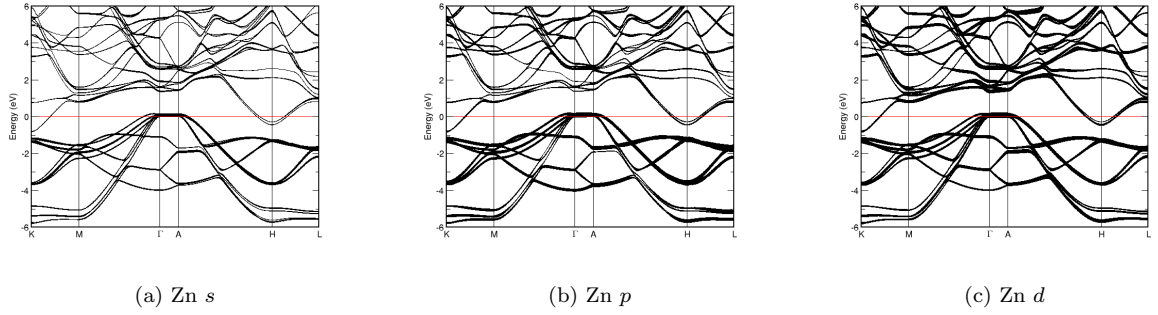FIG. 64: Fat band representation of Zn in  $\text{Li}_2\text{ZnSi}$ 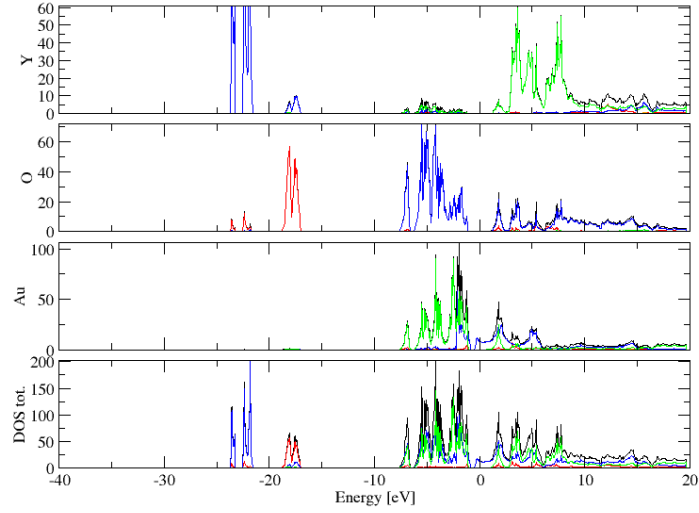FIG. 65: (Color online) PDOS of  $\text{AuYO}_2$  (ICSD #95675). The *s*-, *p*- and *d*-projected states are in red, blue and green, respectively.  $\text{AuYO}_2$  crystallizes in space group  $P\ 63/m\ m\ c$  (#194), in a hexagonal primitive structure.

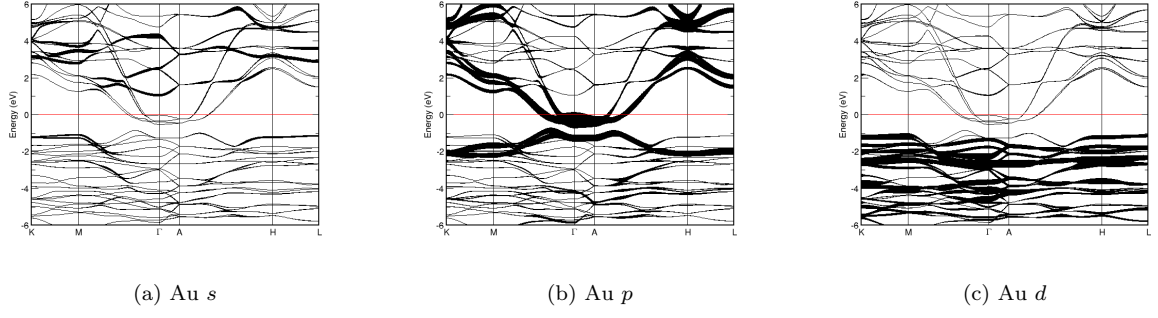FIG. 66: Fat band representation of Au in  $\text{AuYO}_2$ 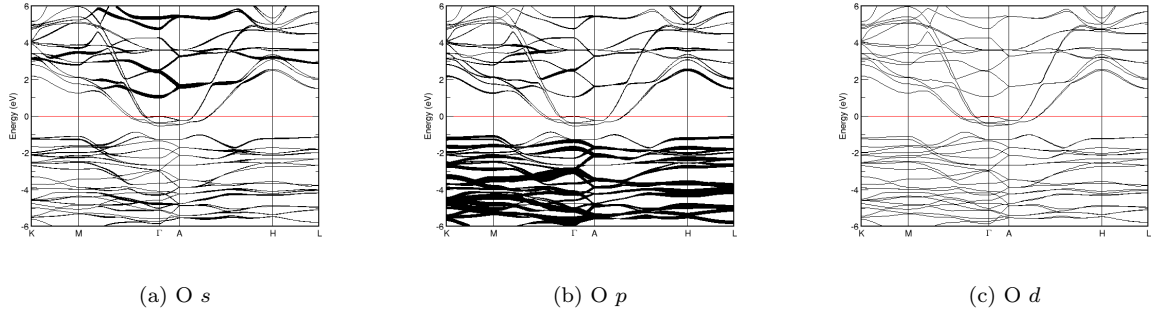FIG. 67: Fat band representation of O in  $\text{AuYO}_2$ 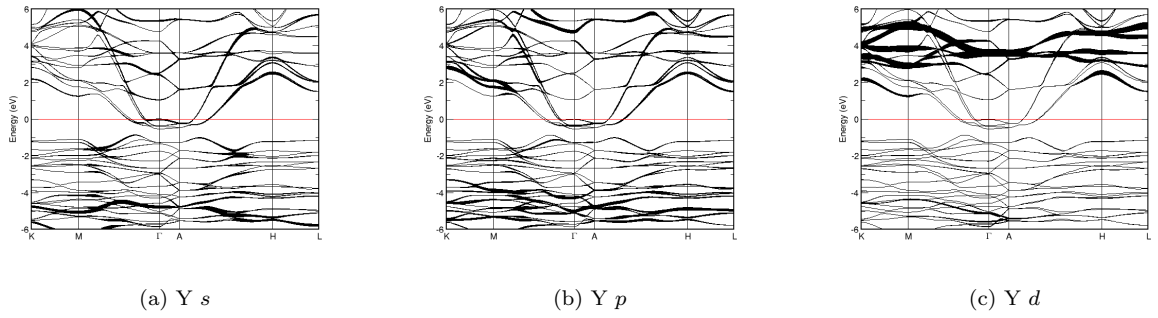FIG. 68: Fat band representation of Y in  $\text{AuYO}_2$

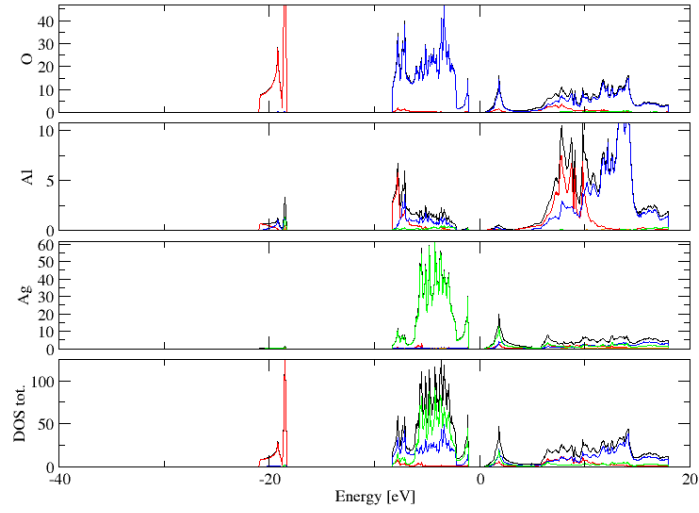

FIG. 69: (Color online) PDOS of  $\text{AgAlO}_2$  (ICSD #300020). The  $s$ -,  $p$ - and  $d$ -projected states are in red, blue and green, respectively.  $\text{AgAlO}_2$  crystallizes in space group  $P 63/m m c$  (#194), in a hexagonal primitive structure. We also note that several other members of the delafossite structure family qualify as possible high-temperature superconductors, after appropriate electron/hole doping, because of layered structure,  $p - d$ -hybridization and cosine-like dispersion around  $E_F$ .

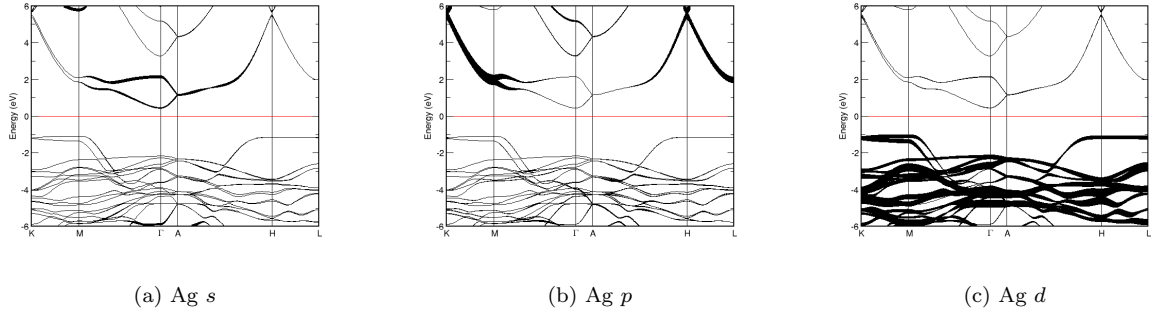

FIG. 70: Fat band representation of Ag in  $\text{AgAlO}_2$

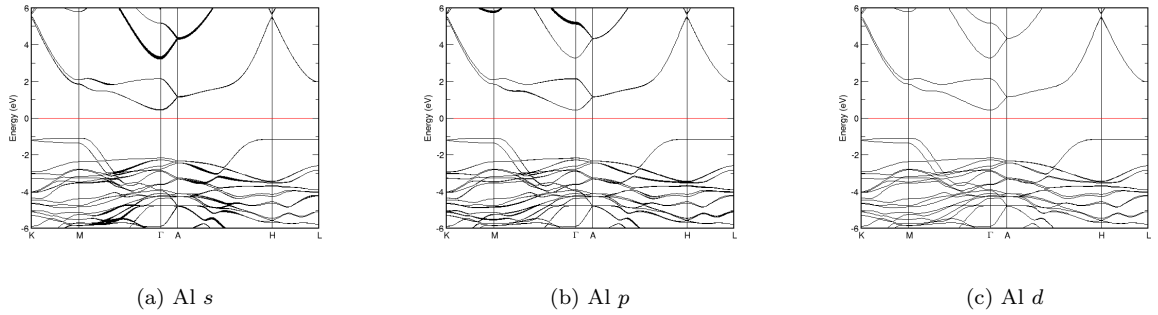

FIG. 71: Fat band representation of Al in  $\text{AgAlO}_2$

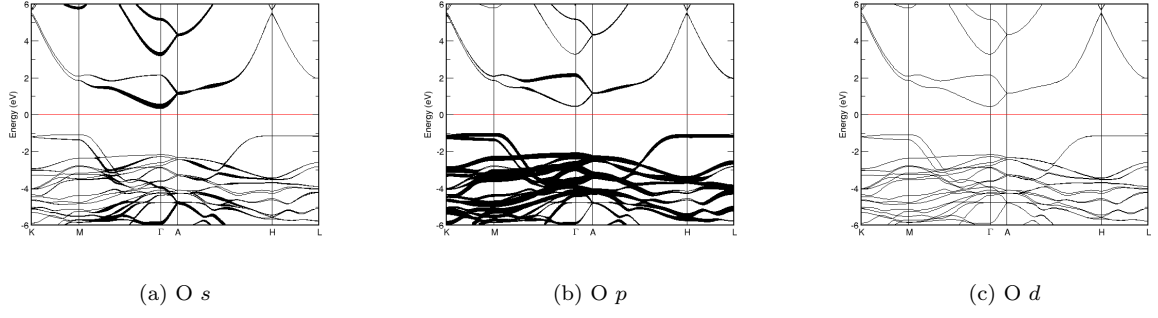FIG. 72: Fat band representation of O in AgAlO<sub>2</sub>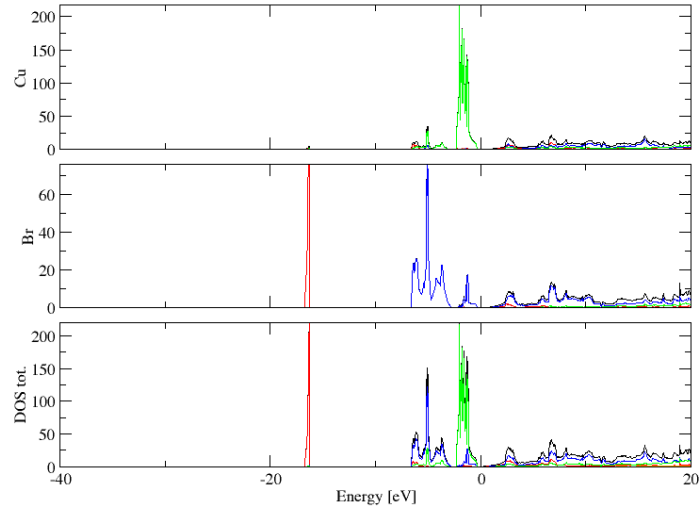FIG. 73: (Color online) PDOS of CuBr (ICSD #30092). The *s*-, *p*- and *d*-projected states are in red, blue and green, respectively. CuBr crystallizes in space group P 63 m c (#186), in a hexagonal primitive structure.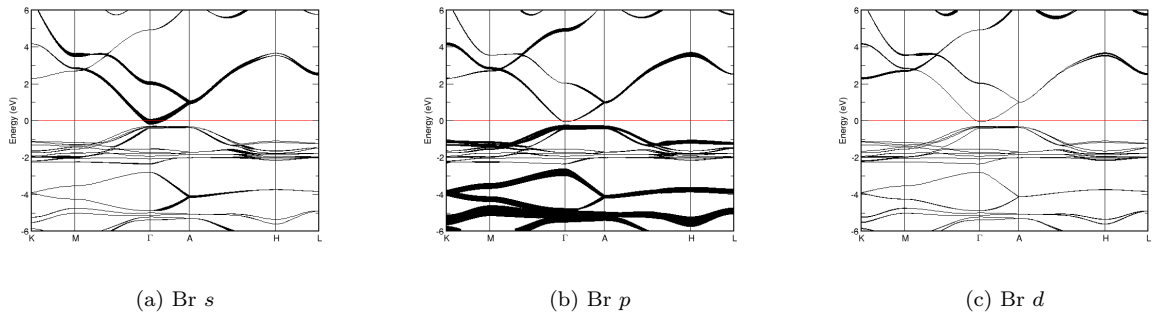

FIG. 74: Fat band representation of Br in CuBr



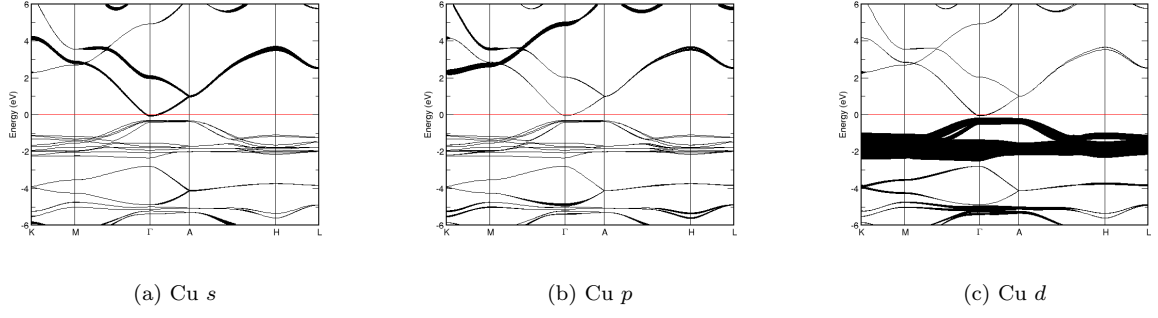

FIG. 75: Fat band representation of Cu in CuBr

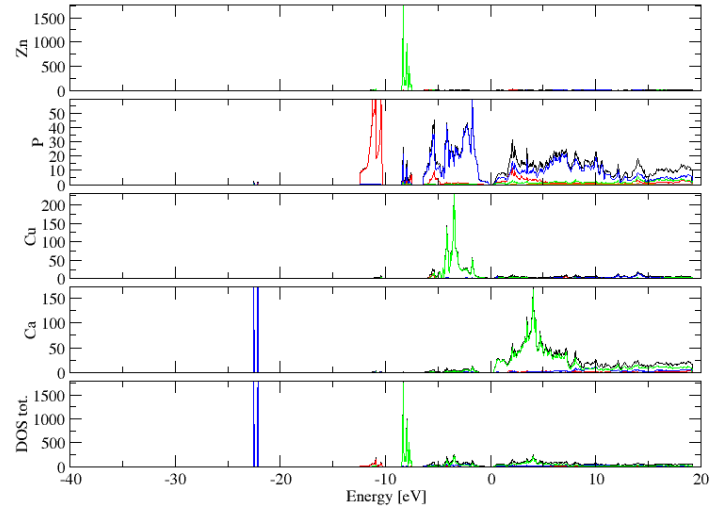FIG. 76: (Color online) PDOS of  $\text{Ca}_2\text{CuZn}_2\text{P}_3$  (ICSD #89517). The *s*-, *p*- and *d*-projected states are in red, blue and green, respectively.  $\text{Ca}_2\text{CuZn}_2\text{P}_3$  crystallizes in space group  $P\ 63/m\ m\ c$  (#194), in a hexagonal primitive structure.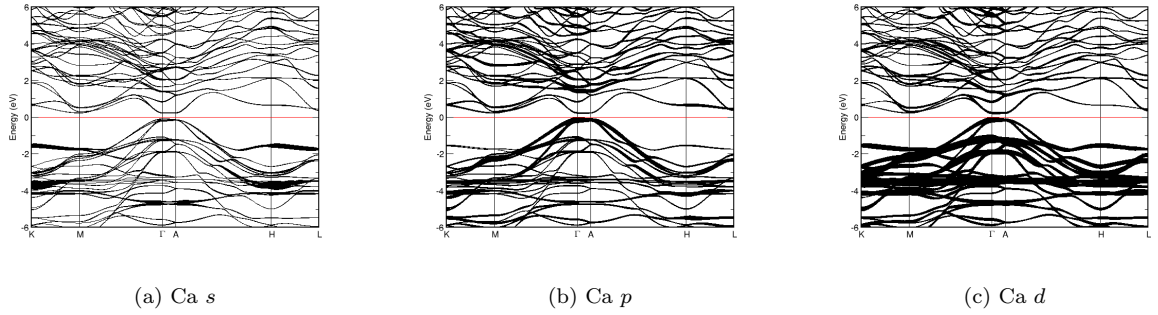FIG. 77: Fat band representation of Ca in  $\text{Ca}_2\text{CuZn}_2\text{P}_3$

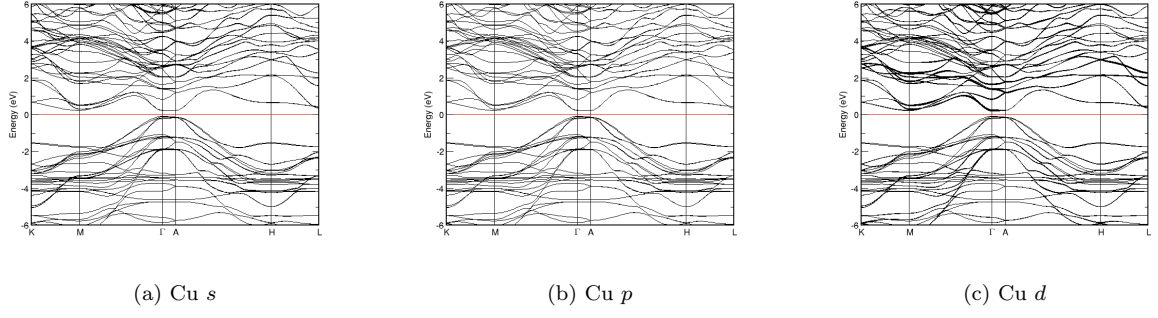FIG. 78: Fat band representation of Cu in  $\text{Ca}_2\text{CuZn}_2\text{P}_3$ 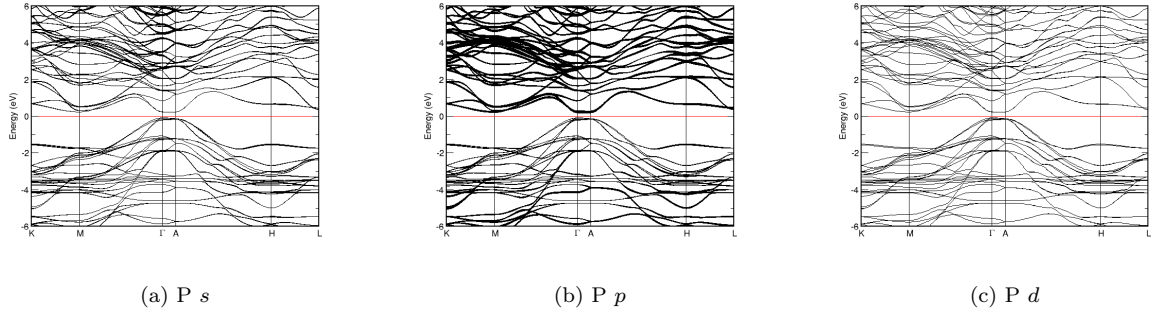FIG. 79: Fat band representation of P in  $\text{Ca}_2\text{CuZn}_2\text{P}_3$ 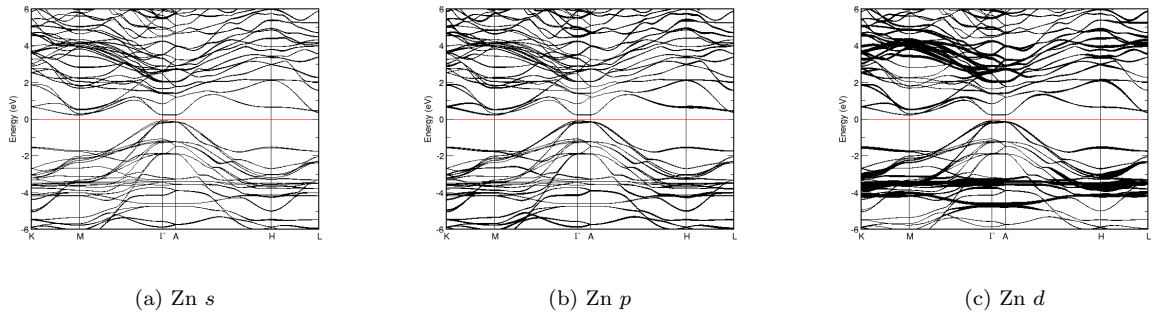FIG. 80: Fat band representation of Zn in  $\text{Ca}_2\text{CuZn}_2\text{P}_3$

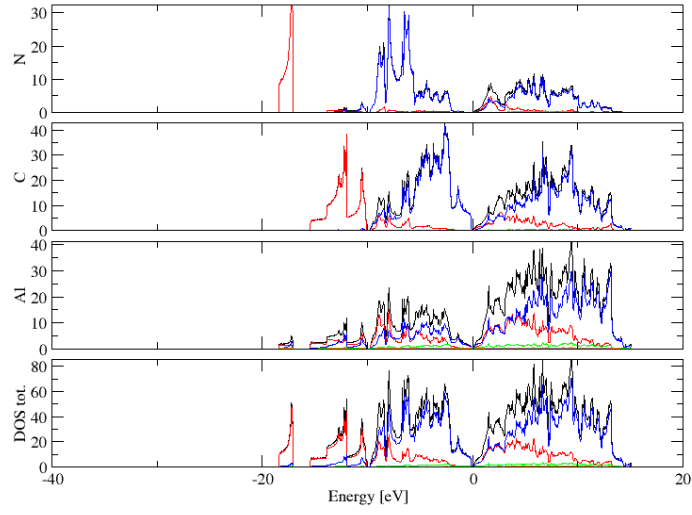

FIG. 81: (Color online) PDOS of  $\text{Al}_5\text{C}_3\text{N}$  (ICSD #26859). The  $s$ -,  $p$ - and  $d$ -projected states are in red, blue and green, respectively.  $\text{Al}_5\text{C}_3\text{N}$  crystallizes in space group P 63 m c (#186), in a hexagonal primitive structure.

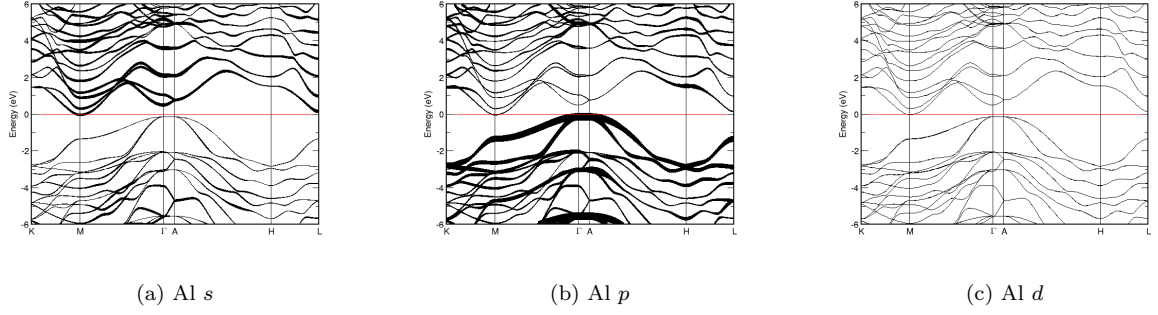

FIG. 82: Fat band representation of Al in  $\text{Al}_5\text{C}_3\text{N}$

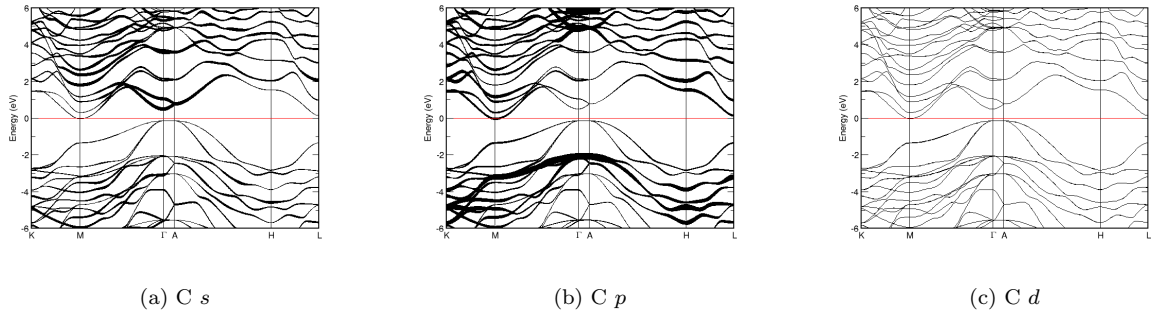

FIG. 83: Fat band representation of C in  $\text{Al}_5\text{C}_3\text{N}$

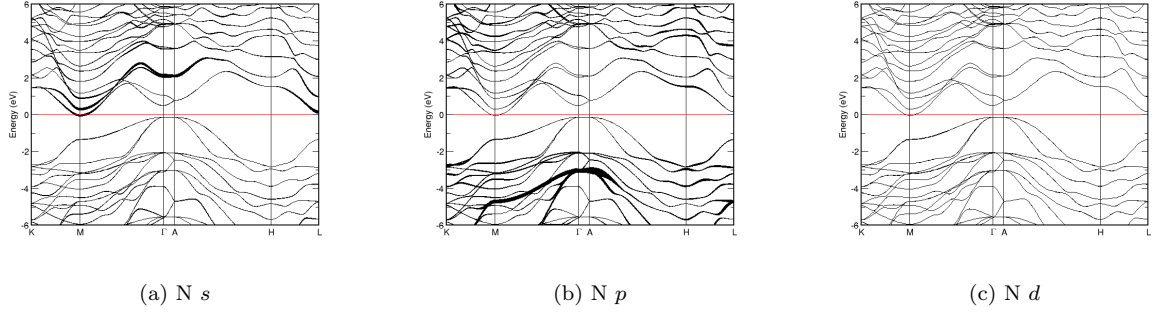FIG. 84: Fat band representation of N in  $\text{Al}_5\text{C}_3\text{N}$ 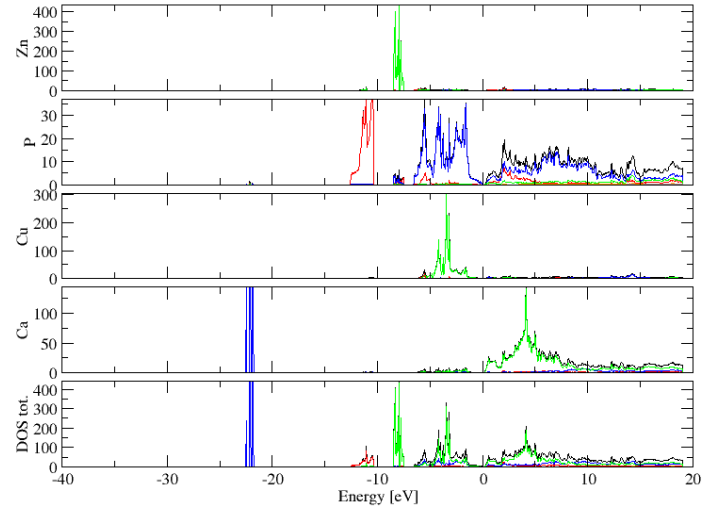FIG. 85: (Color online) PDOS of  $\text{Ca}_3\text{Cu}_2\text{Zn}_2\text{P}_4$  (ICSD #89515). The *s*-, *p*- and *d*-projected states are in red, blue and green, respectively.  $\text{Ca}_3\text{Cu}_2\text{Zn}_2\text{P}_4$  crystallizes in space group  $P\bar{3}m1$  (#164), in a hexagonal primitive structure.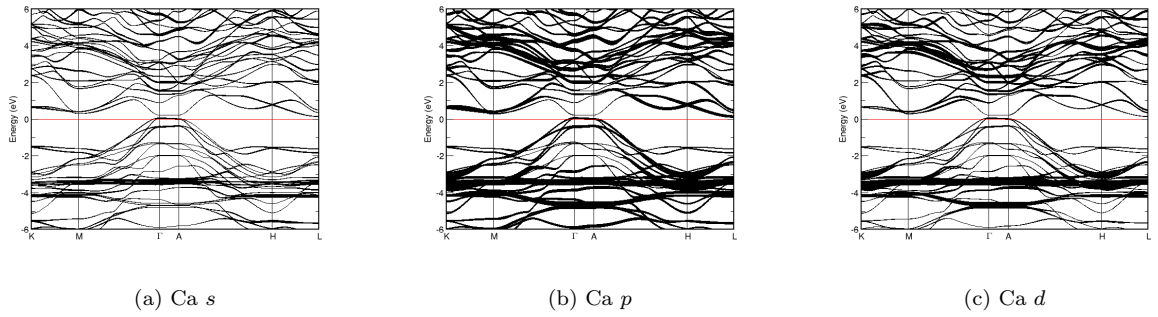FIG. 86: Fat band representation of Ca in  $\text{Ca}_3\text{Cu}_2\text{Zn}_2\text{P}_4$

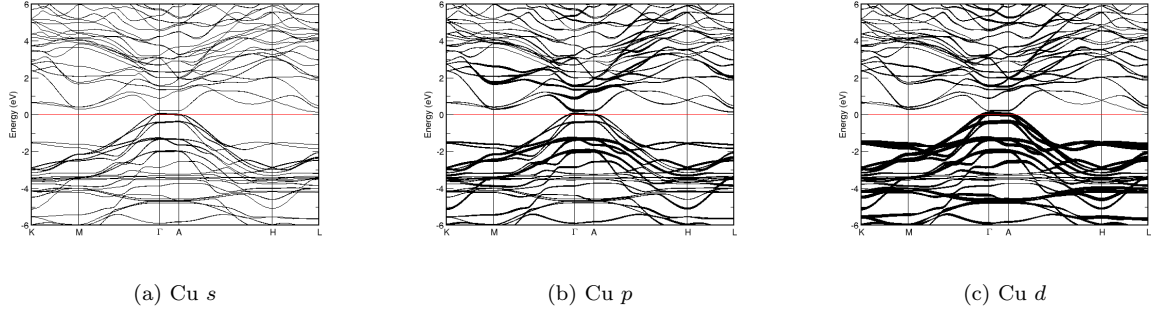FIG. 87: Fat band representation of Cu in  $\text{Ca}_3\text{Cu}_2\text{Zn}_2\text{P}_4$ 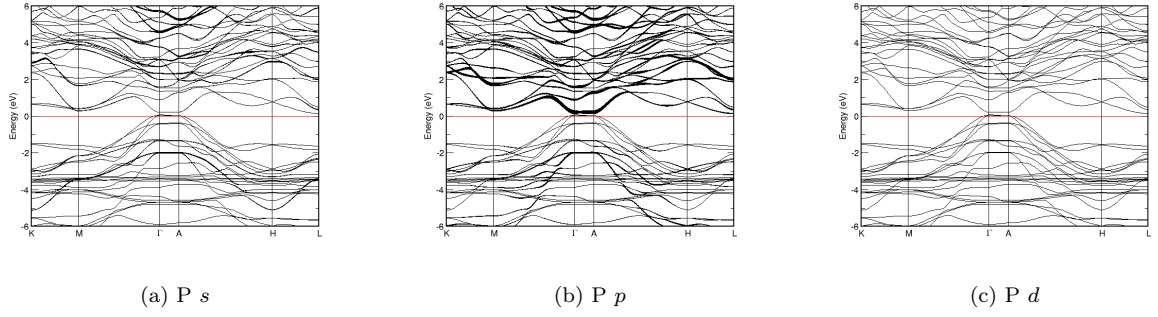FIG. 88: Fat band representation of P in  $\text{Ca}_3\text{Cu}_2\text{Zn}_2\text{P}_4$ 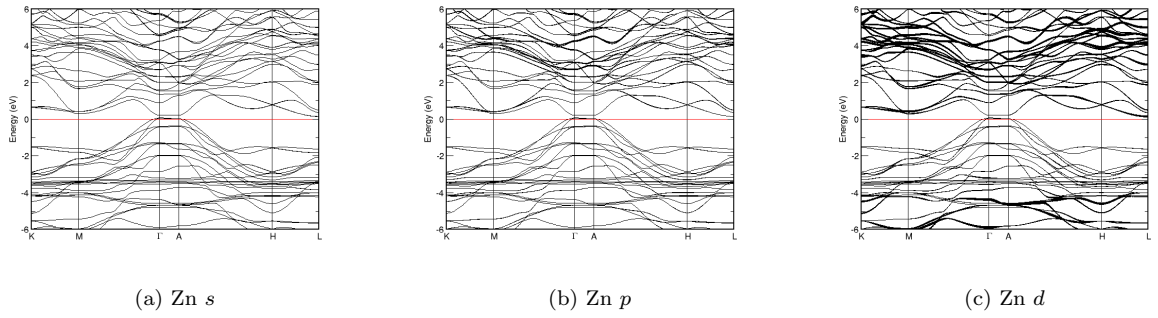FIG. 89: Fat band representation of Zn in  $\text{Ca}_3\text{Cu}_2\text{Zn}_2\text{P}_4$

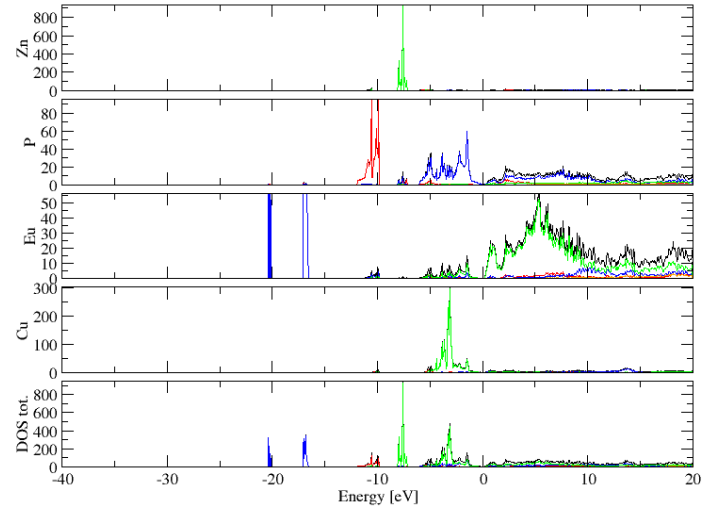

FIG. 90: (Color online) PDOS of  $\text{Eu}_3\text{Cu}_2\text{Zn}_2\text{P}_4$  (ICSD #89516). The  $s$ -,  $p$ - and  $d$ -projected states are in red, blue and green, respectively.  $\text{Eu}_3\text{Cu}_2\text{Zn}_2\text{P}_4$  crystallizes in space group  $P\bar{3}m1$  (#164), in a hexagonal primitive structure.

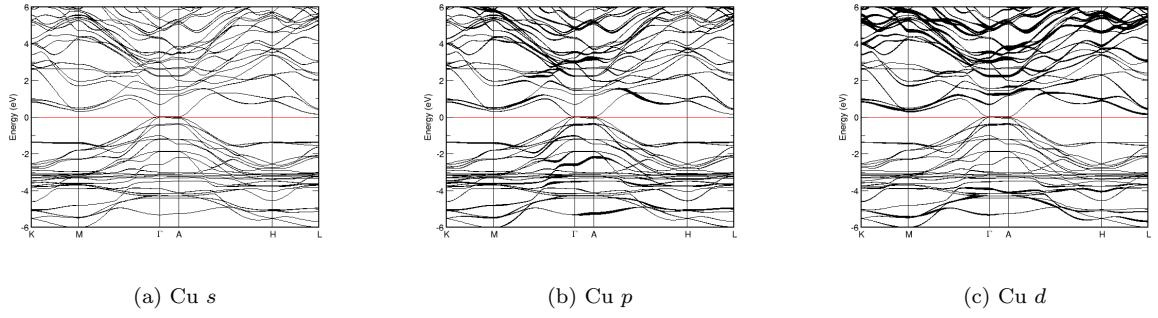

FIG. 91: Fat band representation of Cu in  $\text{Eu}_3\text{Cu}_2\text{Zn}_2\text{P}_4$

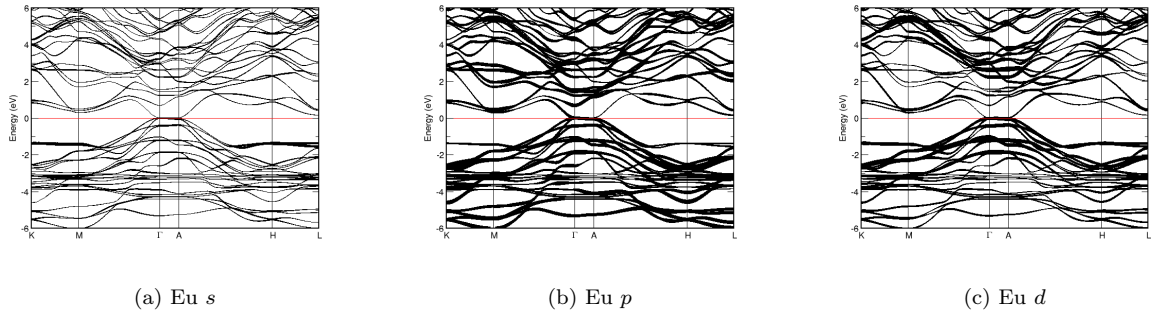

FIG. 92: Fat band representation of Eu in  $\text{Eu}_3\text{Cu}_2\text{Zn}_2\text{P}_4$

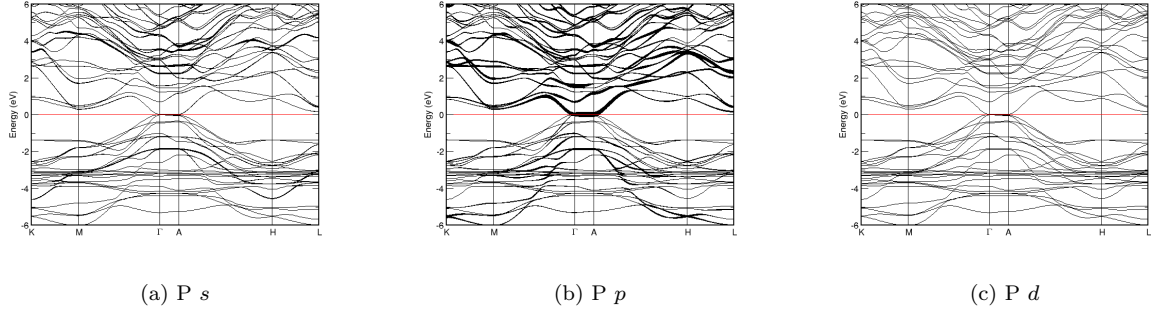FIG. 93: Fat band representation of P in  $\text{Eu}_3\text{Cu}_2\text{Zn}_2\text{P}_4$ 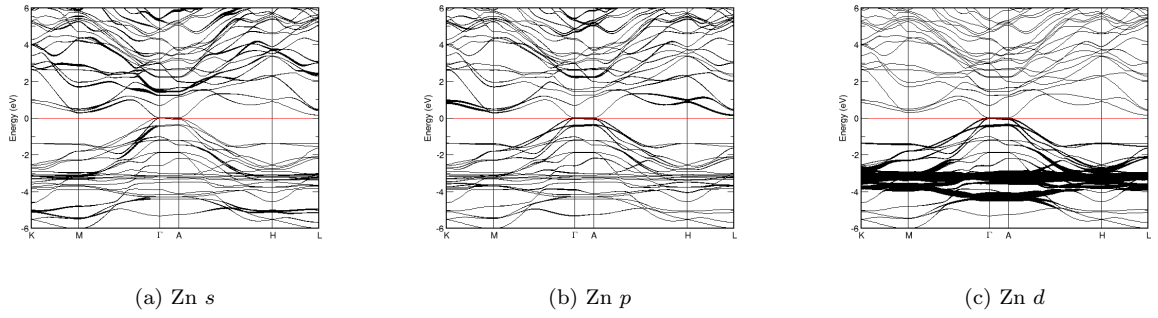FIG. 94: Fat band representation of Zn in  $\text{Eu}_3\text{Cu}_2\text{Zn}_2\text{P}_4$ 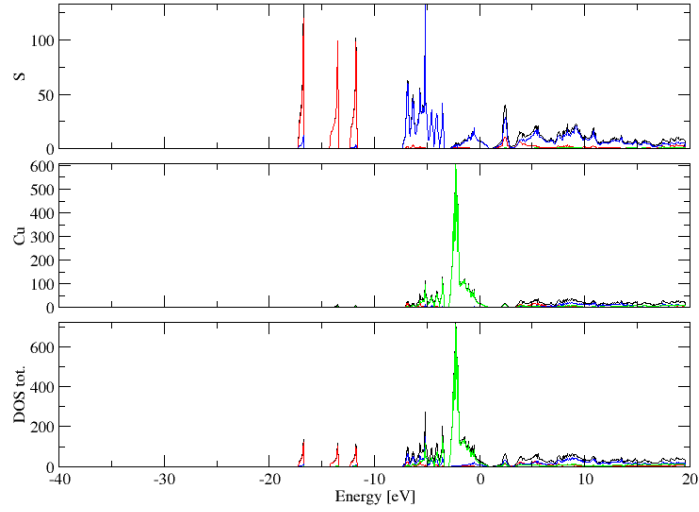FIG. 95: (Color online) PDOS of  $\text{Cu}_4(\text{S}_2)_2(\text{CuS})_2$  (ICSD #26968). The *s*-, *p*- and *d*-projected states are in red, blue and green, respectively.  $\text{Cu}_4(\text{S}_2)_2(\text{CuS})_2$  crystallizes in space group P 63/m m c (#194), in a hexagonal primitive structure.

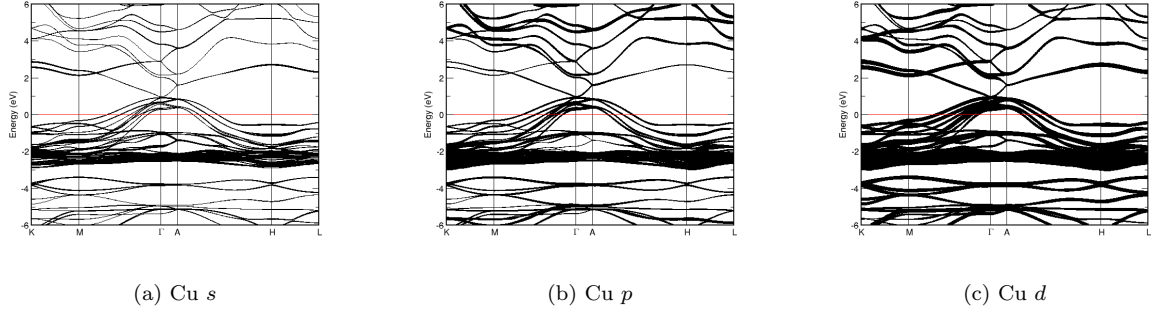

FIG. 96: Fat band representation of Cu in  $\text{Cu}_4(\text{S}_2)_2(\text{CuS})_2$

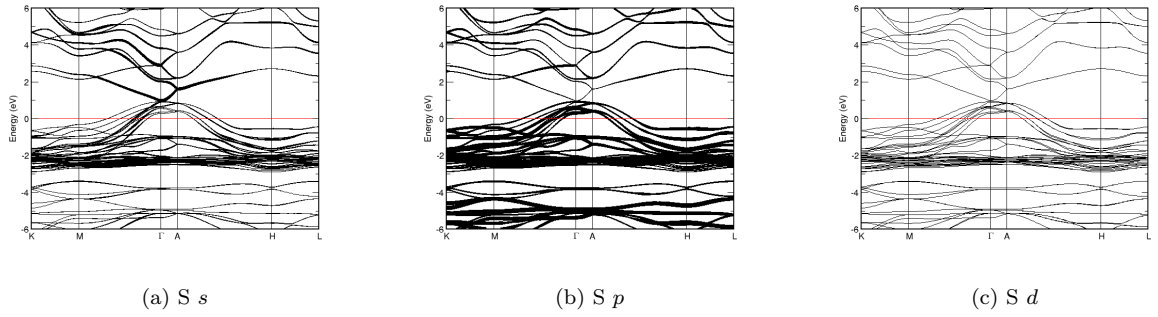

FIG. 97: Fat band representation of S in  $\text{Cu}_4(\text{S}_2)_2(\text{CuS})_2$

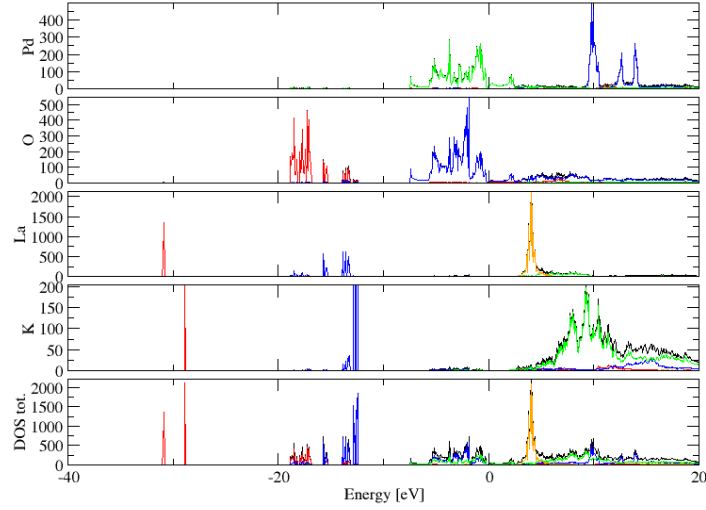

FIG. 98: (Color online) PDOS of  $\text{LaKPdO}_3$  (ICSD #417108). The *s*-, *p*- and *d*-projected states are in red, blue and green, respectively.  $\text{LaKPdO}_3$  crystallizes in space group  $C 1 2/m 1$  (#12), in a monoclinic base-centred structure.



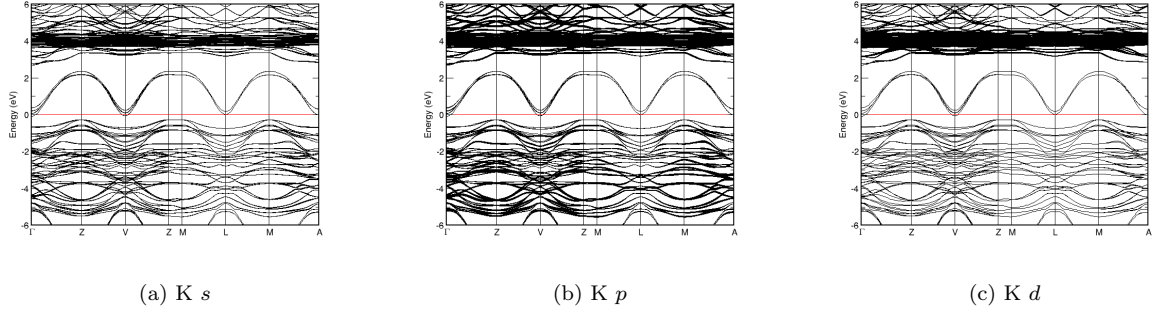FIG. 99: Fat band representation of K in LaKPdO<sub>3</sub>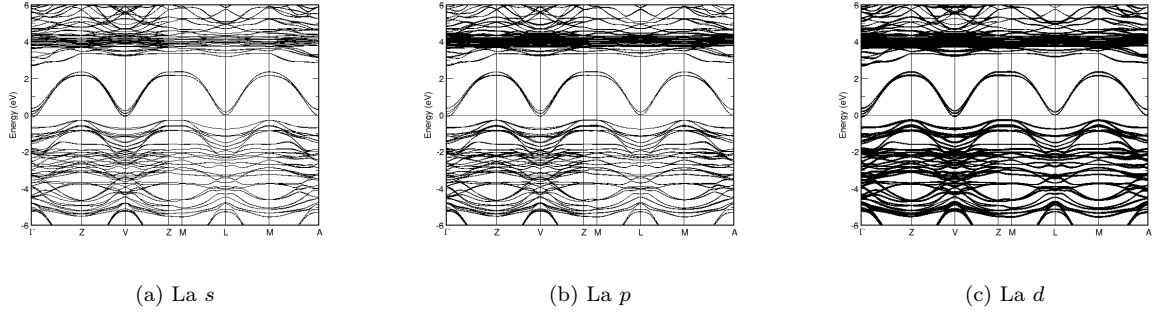FIG. 100: Fat band representation of La in LaKPdO<sub>3</sub>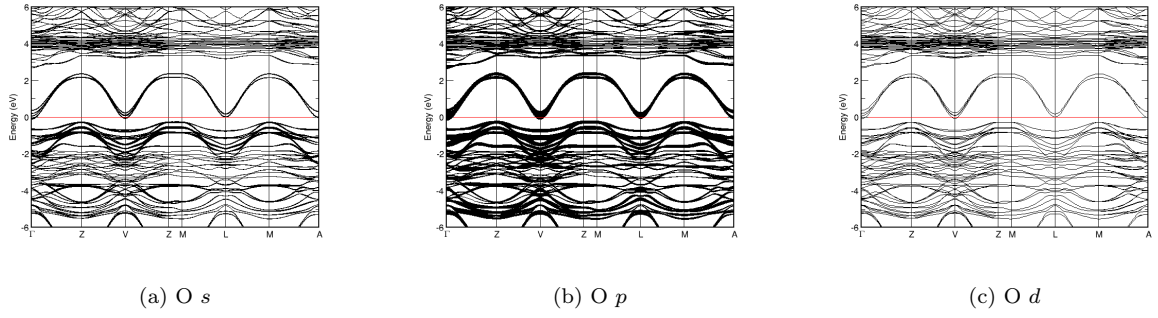FIG. 101: Fat band representation of O in LaKPdO<sub>3</sub>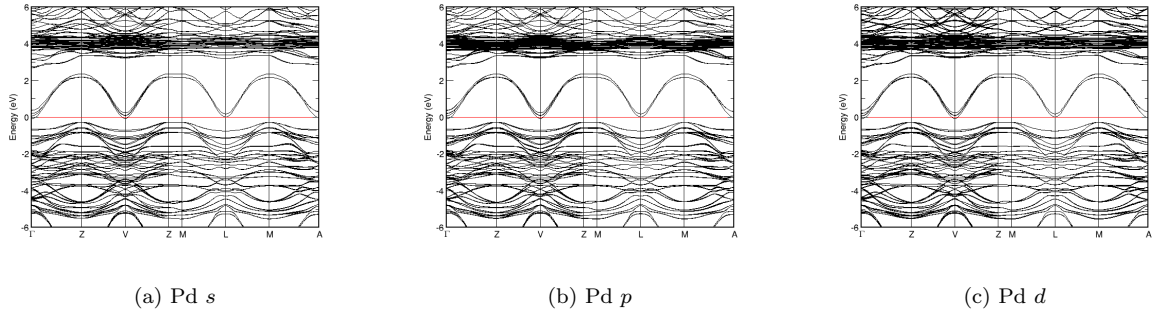FIG. 102: Fat band representation of Pd in LaKPdO<sub>3</sub>

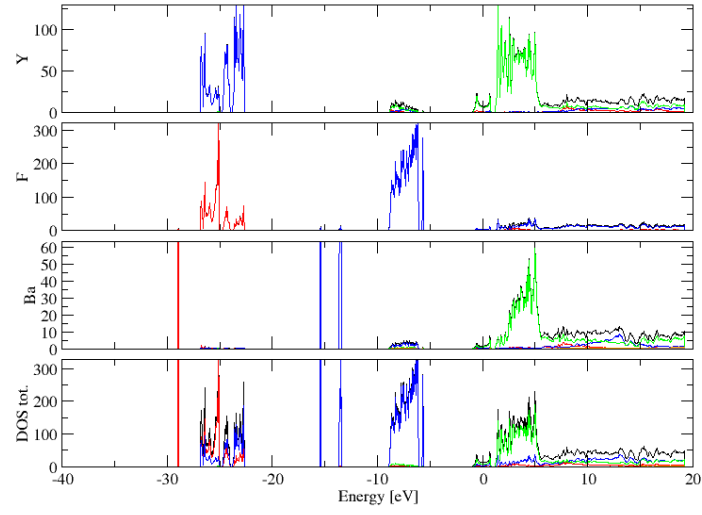

FIG. 103: (Color online) PDOS of  $\text{BaY}_2\text{F}_8$  (ICSD #74359). The  $s$ -,  $p$ - and  $d$ -projected states are in red, blue and green, respectively.  $\text{BaY}_2\text{F}_8$  crystallizes in space group  $C 1 2/m 1$  (#12), in a monoclinic base-centred structure.

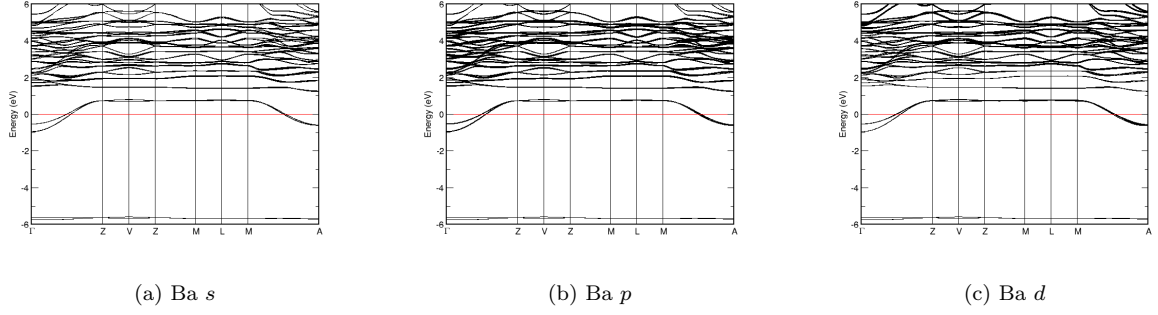

FIG. 104: Fat band representation of Ba in  $\text{BaY}_2\text{F}_8$

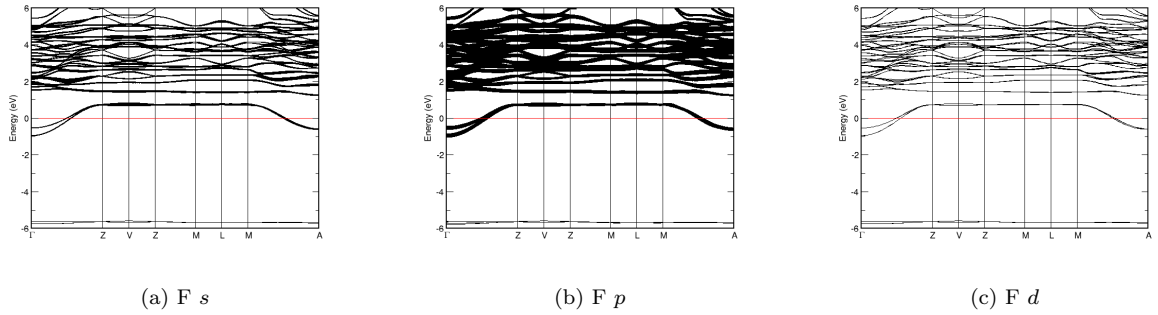

FIG. 105: Fat band representation of F in  $\text{BaY}_2\text{F}_8$

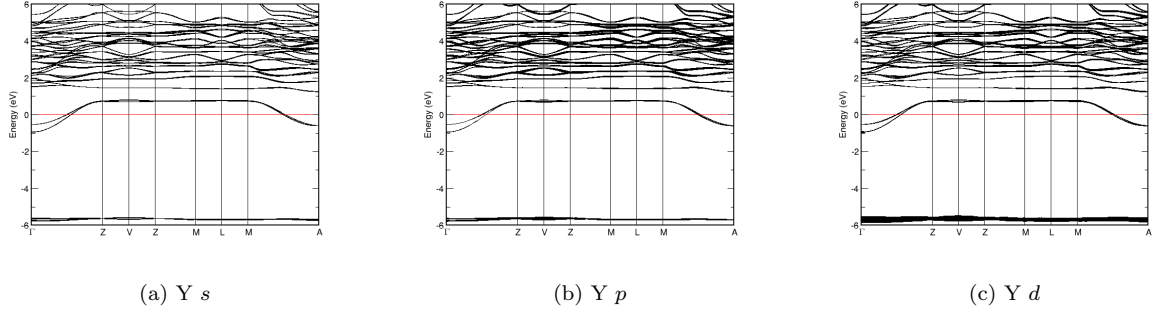FIG. 106: Fat band representation of Y in BaY<sub>2</sub>F<sub>8</sub>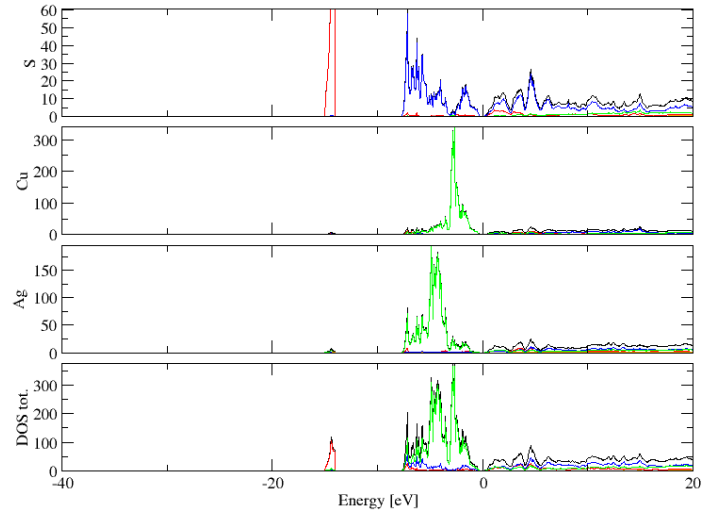FIG. 107: (Color online) PDOS of AgCuS (ICSD #30233). The *s*-, *p*- and *d*-projected states are in red, blue and green, respectively. AgCuS crystallizes in space group *C m c m* (#63), in a orthorhombic base-centred structure.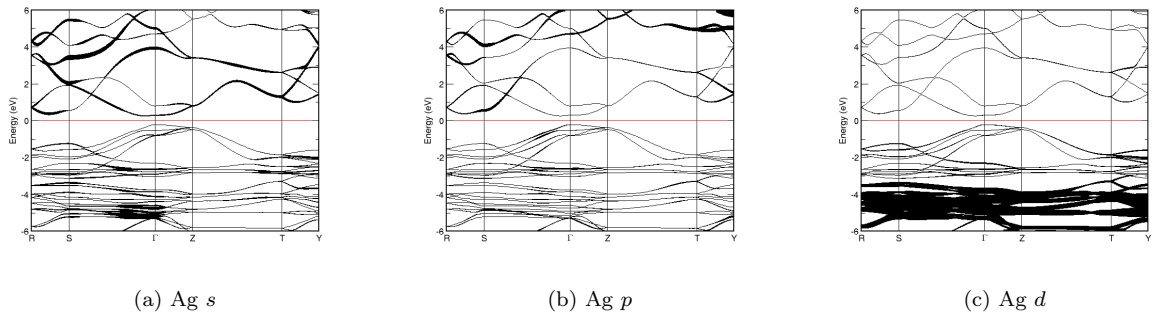

FIG. 108: Fat band representation of Ag in AgCuS

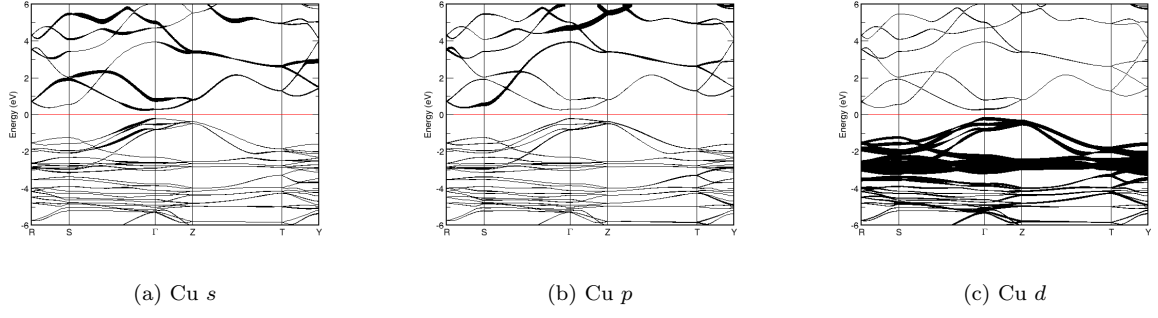

FIG. 109: Fat band representation of Cu in AgCuS

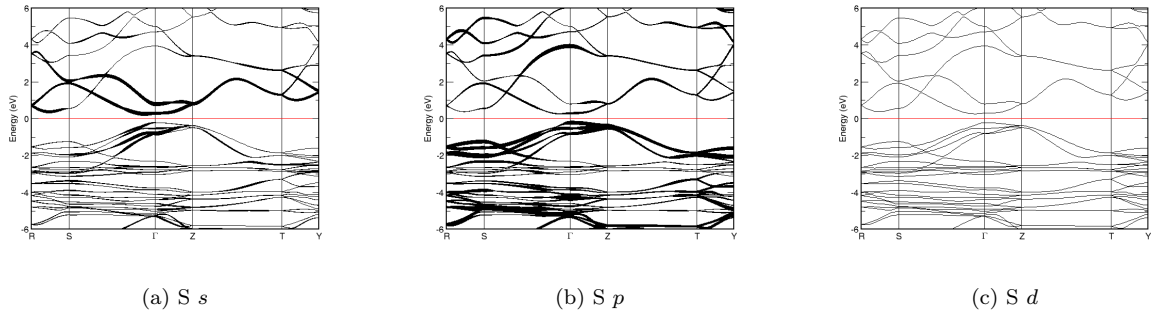

FIG. 110: Fat band representation of S in AgCuS

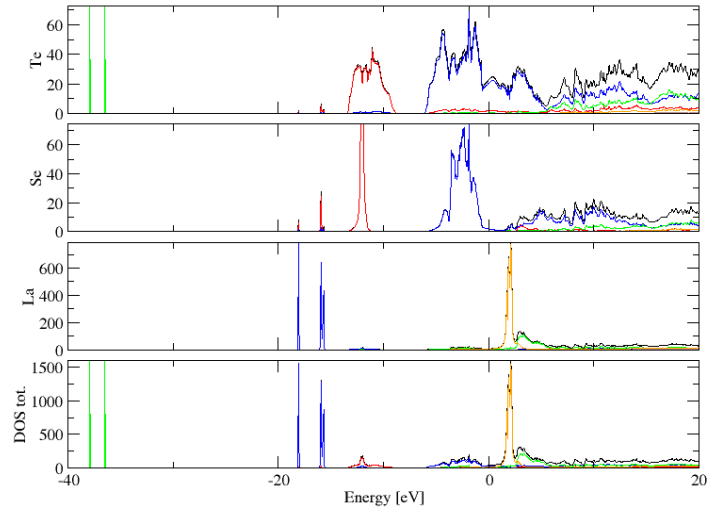FIG. 111: (Color online) PDOS of LaSeTe<sub>2</sub> (ICSD #413171). The  $s$ -,  $p$ - and  $d$ -projected states are in red, blue and green, respectively. LaSeTe<sub>2</sub> crystallizes in space group  $C m c m$  (#63), in a orthorhombic base-centred structure.

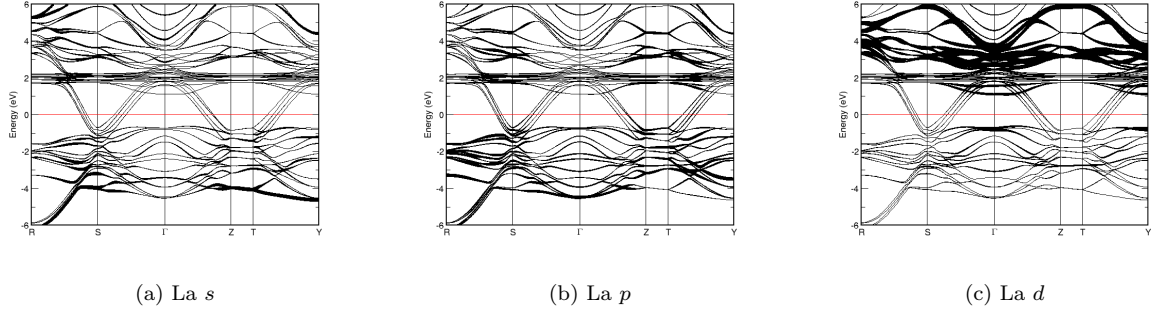FIG. 112: Fat band representation of La in  $\text{LaSeTe}_2$ 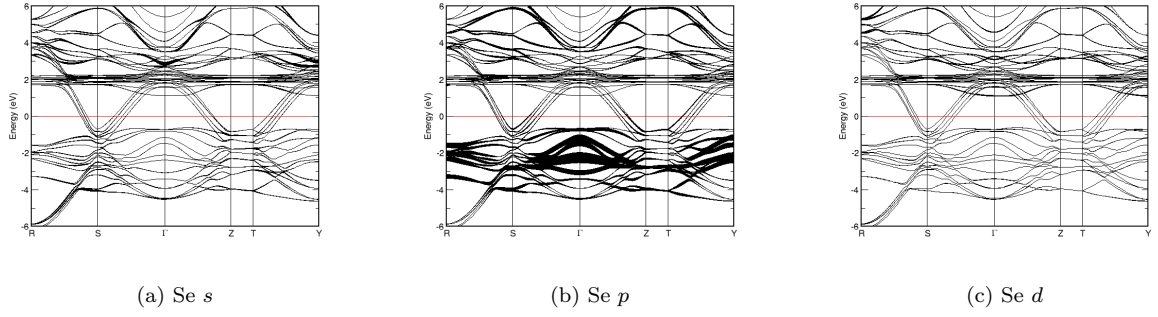FIG. 113: Fat band representation of Se in  $\text{LaSeTe}_2$ 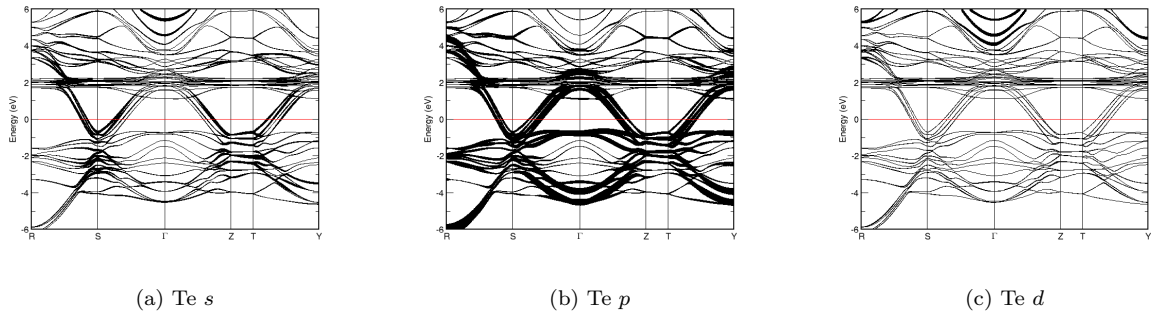FIG. 114: Fat band representation of Te in  $\text{LaSeTe}_2$

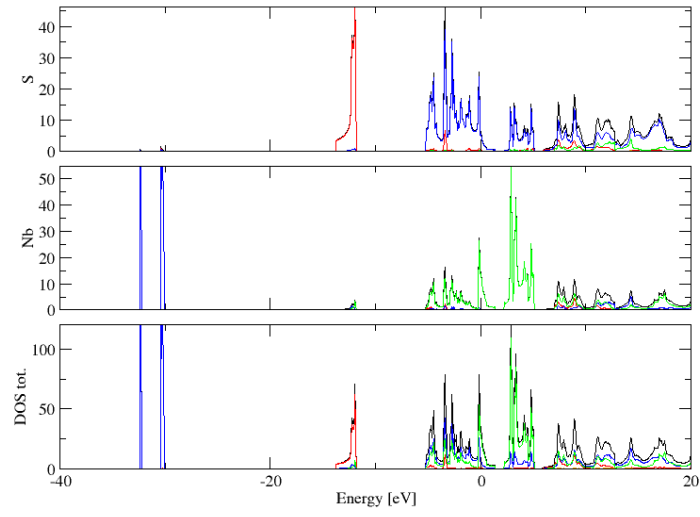

FIG. 115: (Color online) PDOS of NbS<sub>2</sub> (ICSD #67443). The *s*-, *p*- and *d*-projected states are in red, blue and green, respectively. NbS<sub>2</sub> crystallizes in space group C m 2 m (#38), in a orthorhombic base-centred structure.

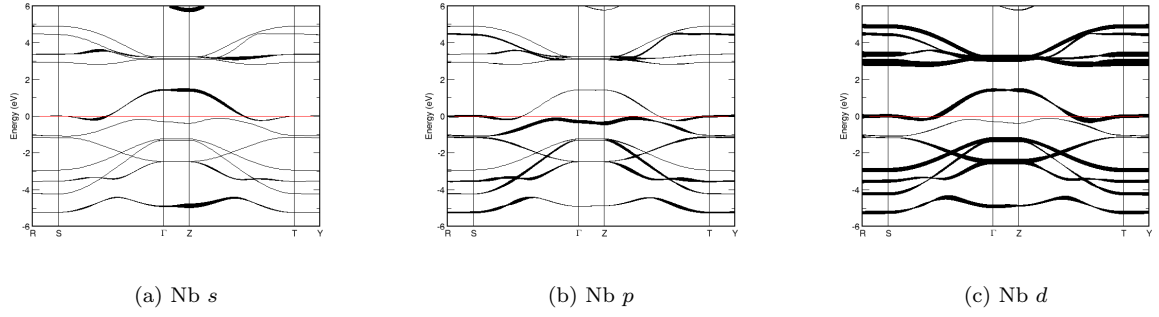

FIG. 116: Fat band representation of Nb in NbS<sub>2</sub>

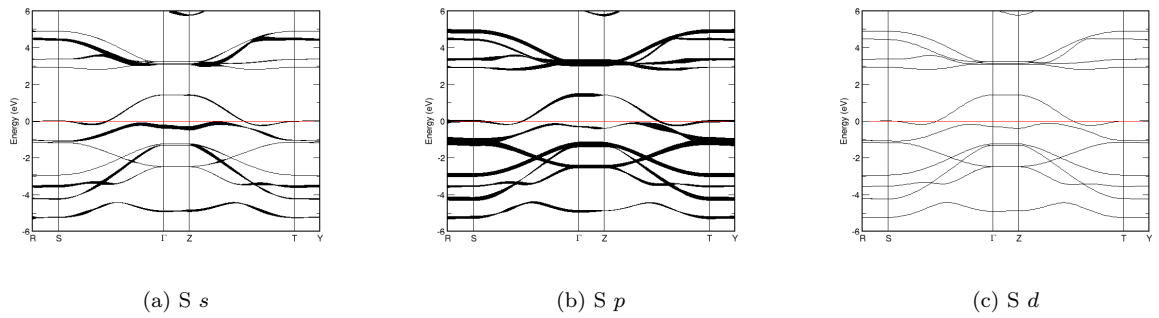

FIG. 117: Fat band representation of S in NbS<sub>2</sub>

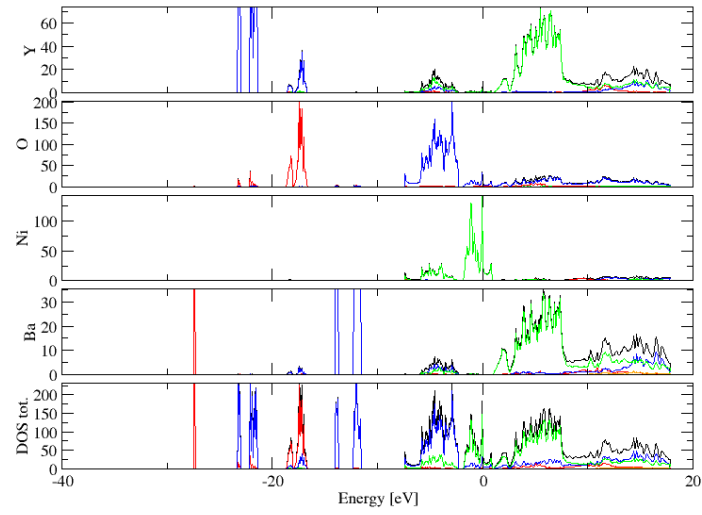

FIG. 118: (Color online) PDOS of  $\text{BaNiY}_2\text{O}_5$  (ICSD #68795). The  $s$ -,  $p$ - and  $d$ -projected states are in red, blue and green, respectively.  $\text{BaNiY}_2\text{O}_5$  crystallizes in space group  $\text{I m m m}$  (#71), in a orthorhombic body-centred structure.

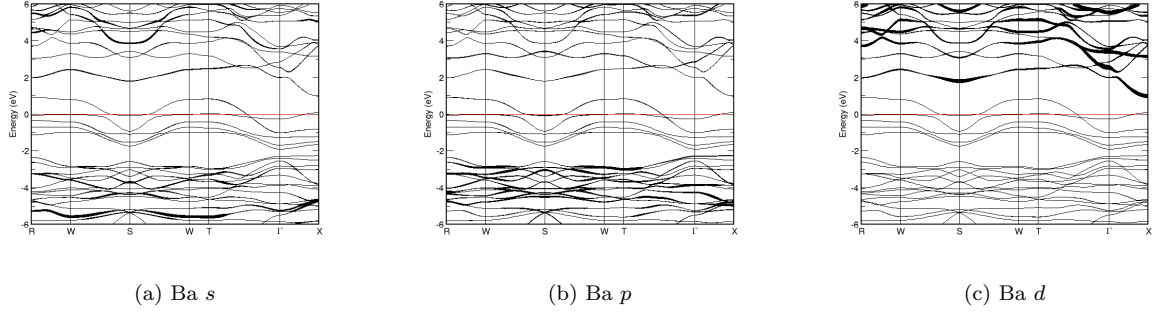

FIG. 119: Fat band representation of Ba in  $\text{BaNiY}_2\text{O}_5$

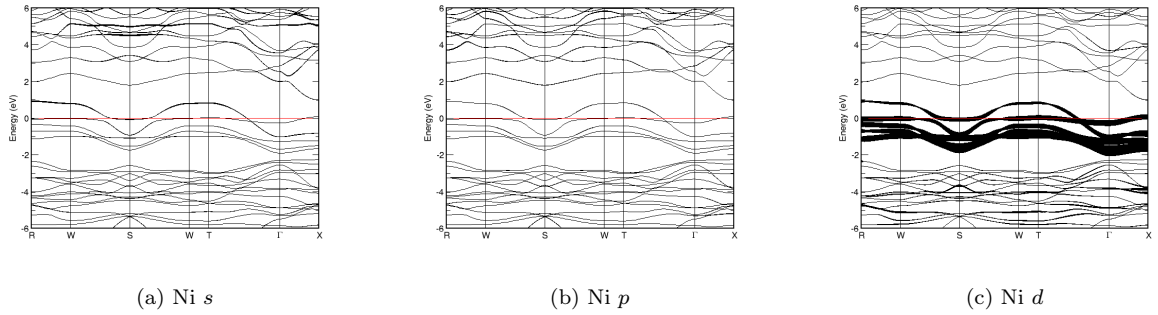

FIG. 120: Fat band representation of Ni in  $\text{BaNiY}_2\text{O}_5$

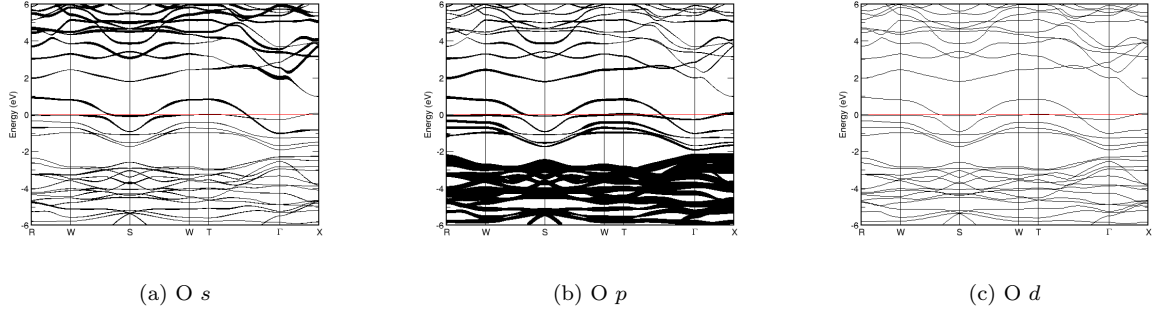FIG. 121: Fat band representation of O in  $\text{BaNiY}_2\text{O}_5$ 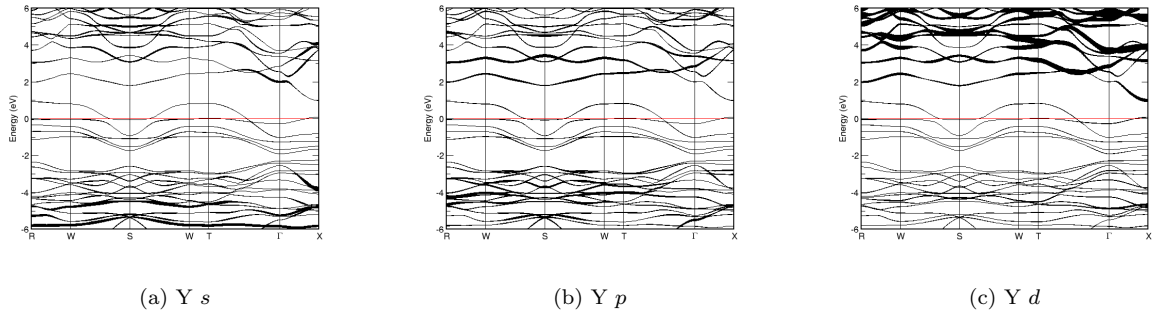FIG. 122: Fat band representation of Y in  $\text{BaNiY}_2\text{O}_5$ 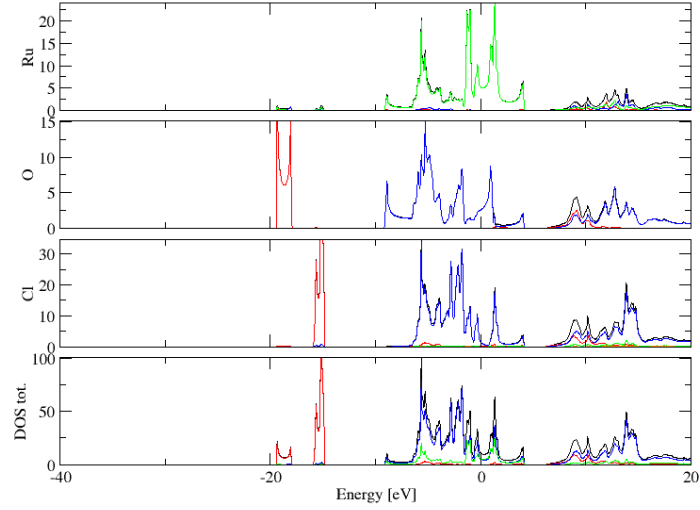

FIG. 123: (Color online) PDOS of  $\text{RuOCl}_2$  (ICSD #83883). The  $s$ -,  $p$ - and  $d$ -projected states are in red, blue and green, respectively.  $\text{RuOCl}_2$  crystallizes in space group  $I m m m$  (#71), in a orthorhombic body-centred structure.



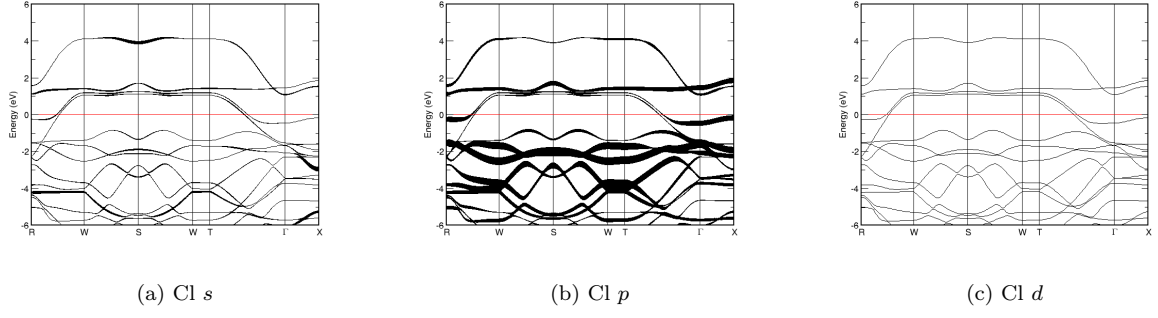FIG. 124: Fat band representation of Cl in  $\text{RuOCl}_2$ 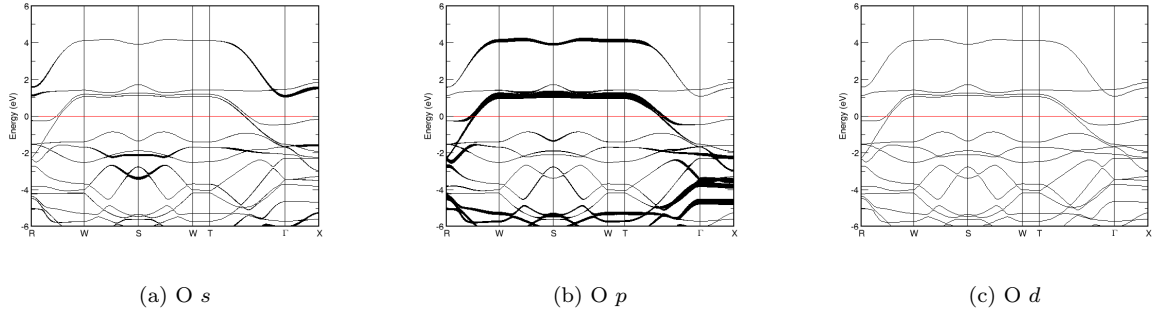FIG. 125: Fat band representation of O in  $\text{RuOCl}_2$ 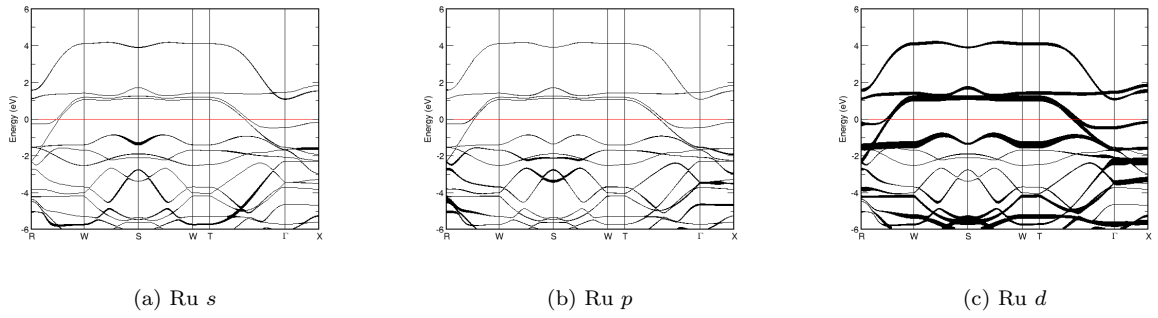FIG. 126: Fat band representation of Ru in  $\text{RuOCl}_2$

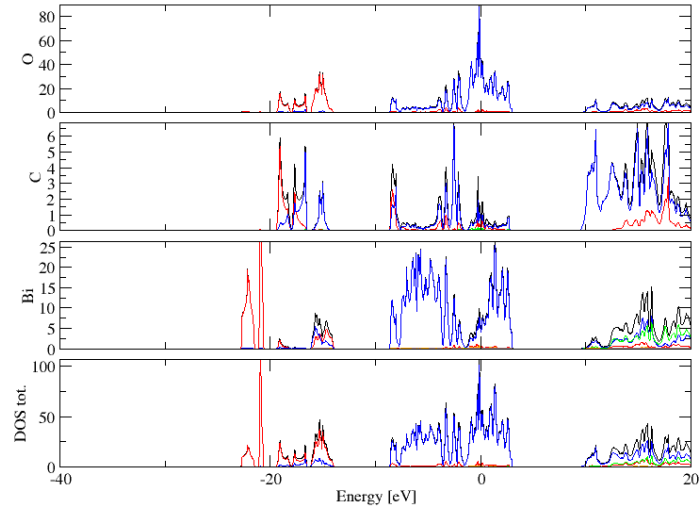

FIG. 127: (Color online) PDOS of  $\text{Bi}_2(\text{CO}_3)\text{O}_2$  (ICSD #94740). The  $s$ -,  $p$ - and  $d$ -projected states are in red, blue and green, respectively.  $\text{Bi}_2(\text{CO}_3)\text{O}_2$  crystallizes in space group  $I m m 2$  (#44), in a orthorhombic body-centred structure.

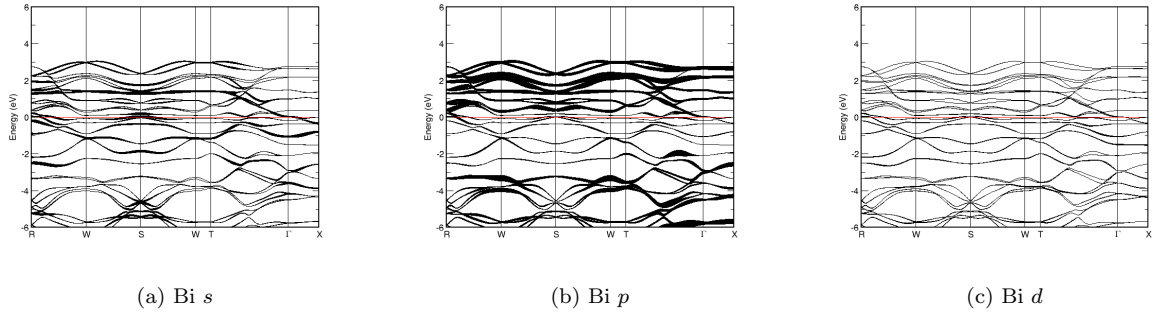

FIG. 128: Fat band representation of Bi in  $\text{Bi}_2(\text{CO}_3)\text{O}_2$

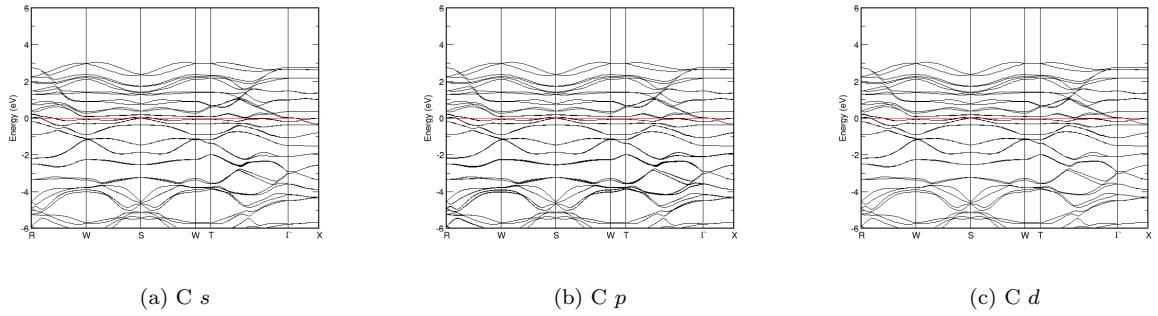

FIG. 129: Fat band representation of C in  $\text{Bi}_2(\text{CO}_3)\text{O}_2$

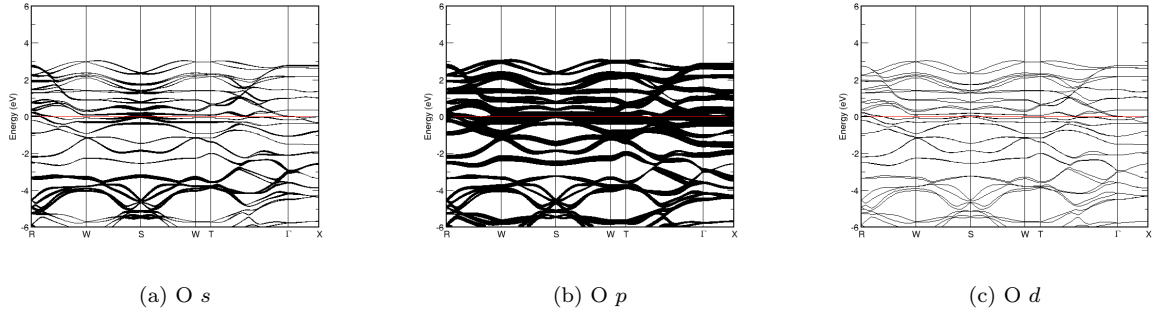

FIG. 130: Fat band representation of O in  $\text{Bi}_2(\text{CO}_3)\text{O}_2$

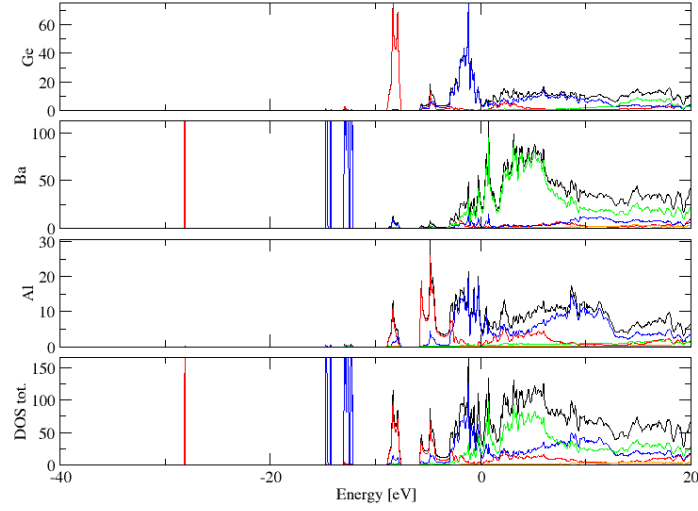

FIG. 131: (Color online) PDOS of  $\text{Al}_2\text{Ba}_3\text{Ge}_2$  (ICSD #52612). The  $s$ -,  $p$ - and  $d$ -projected states are in red, blue and green, respectively.  $\text{Al}_2\text{Ba}_3\text{Ge}_2$  crystallizes in space group  $I m m m$  (#71), in a orthorhombic body-centred structure.

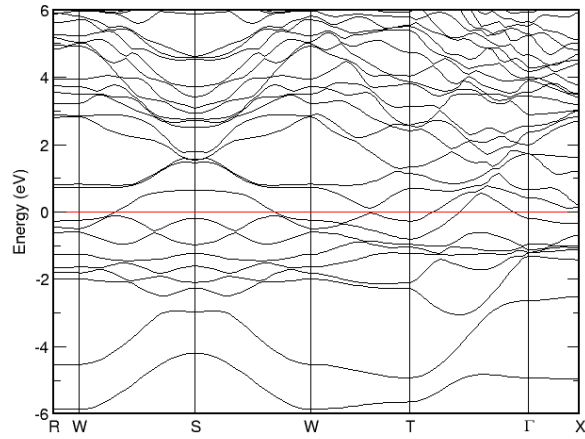

(a) E vs. k

FIG. 132: Band structure of  $\text{Ba}_3\text{Al}_2\text{Sn}_2$

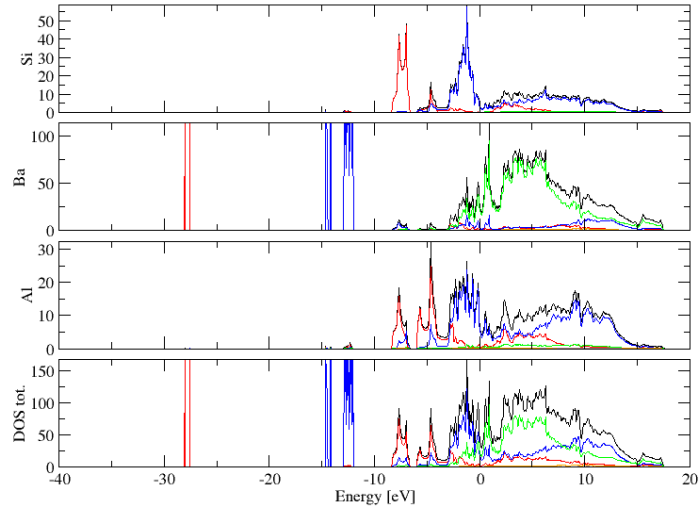

FIG. 133: (Color online) PDOS of  $\text{Ba}_3\text{Al}_2\text{Si}_2$  (ICSD #100128). The  $s$ -,  $p$ - and  $d$ -projected states are in red, blue and green, respectively.  $\text{Ba}_3\text{Al}_2\text{Si}_2$  crystallizes in space group  $I m m m$  (#71), in a orthorhombic body-centred structure.

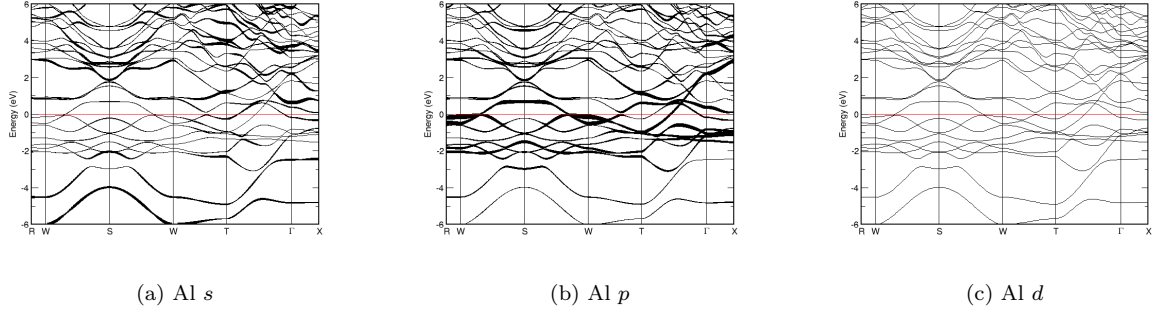

FIG. 134: Fat band representation of Al in  $\text{Ba}_3\text{Al}_2\text{Si}_2$

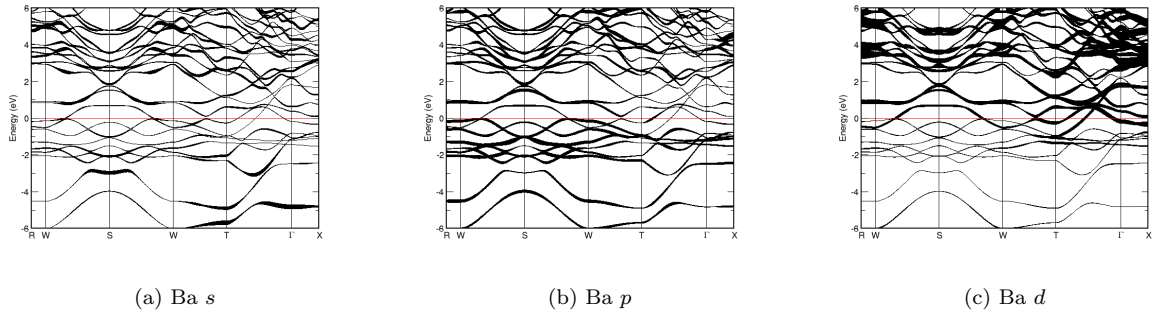

FIG. 135: Fat band representation of Ba in  $\text{Ba}_3\text{Al}_2\text{Si}_2$

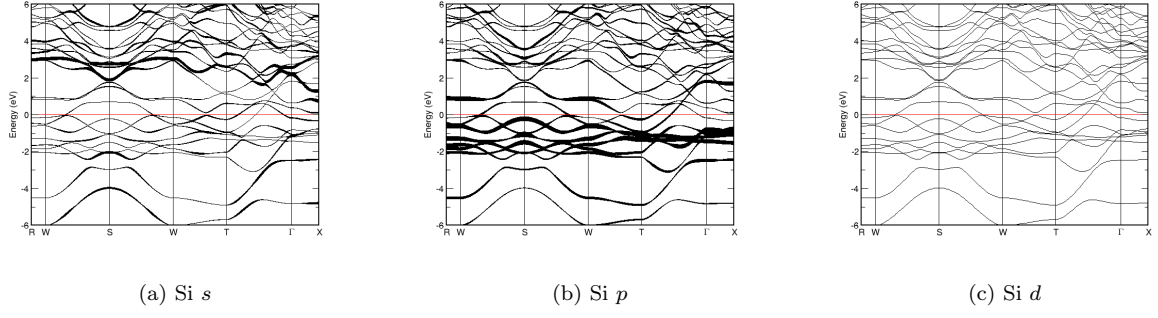FIG. 136: Fat band representation of Si in  $\text{Ba}_3\text{Al}_2\text{Si}_2$ 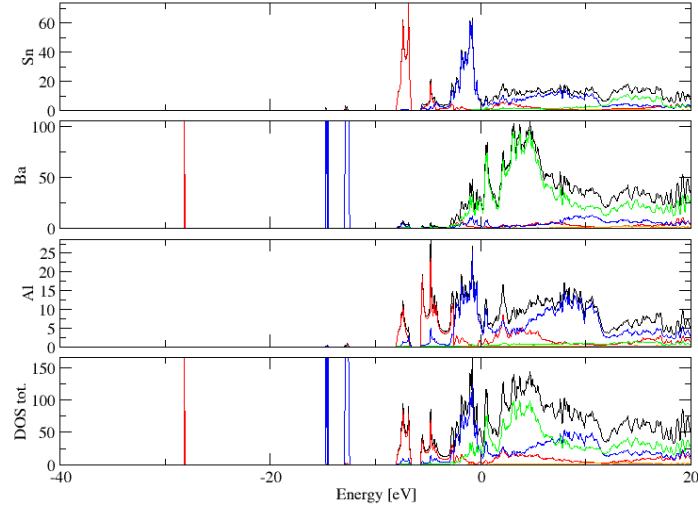FIG. 137: (Color online) PDOS of  $\text{Ba}_3\text{Al}_2\text{Sn}_2$  (ICSD #9565). The  $s$ -,  $p$ - and  $d$ -projected states are in red, blue and green, respectively.  $\text{Ba}_3\text{Al}_2\text{Sn}_2$  crystallizes in space group  $I m m m$  (#71), in a orthorhombic body-centred structure.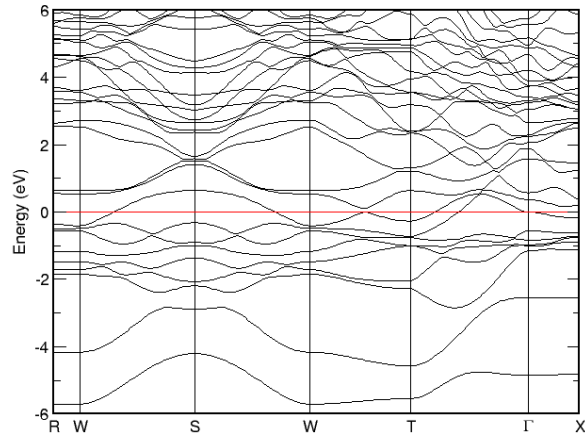(a)  $E$  vs.  $k$ FIG. 138: Band structure of  $\text{Ba}_3\text{Al}_2\text{Sn}_2$

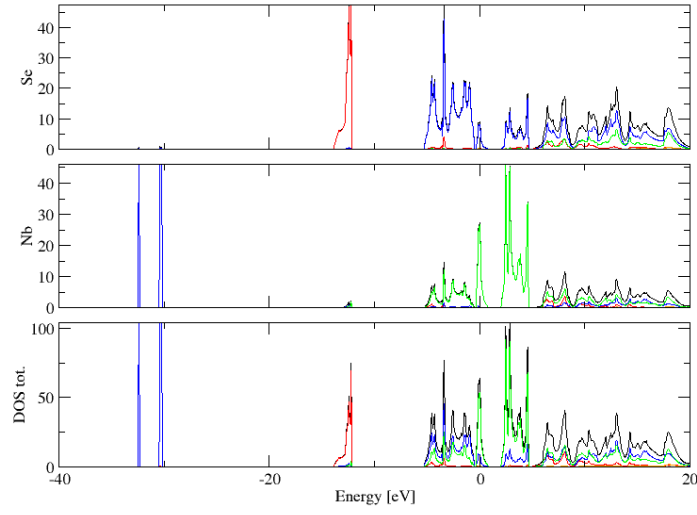

FIG. 139: (Color online) PDOS of NbSe<sub>2</sub> (ICSD #71339). The *s*-, *p*- and *d*-projected states are in red, blue and green, respectively. NbSe<sub>2</sub> crystallizes in space group  $Fm\bar{2}m$  (#42), in a orthorhombic face-centred structure.

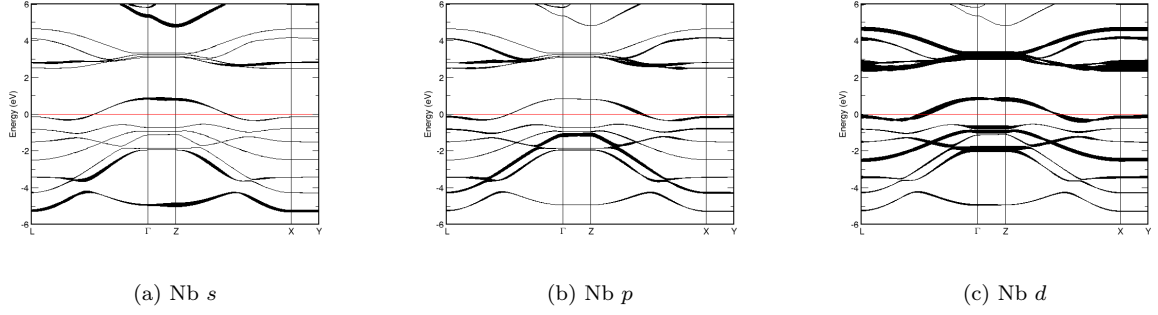

FIG. 140: Fat band representation of Nb in NbSe<sub>2</sub>

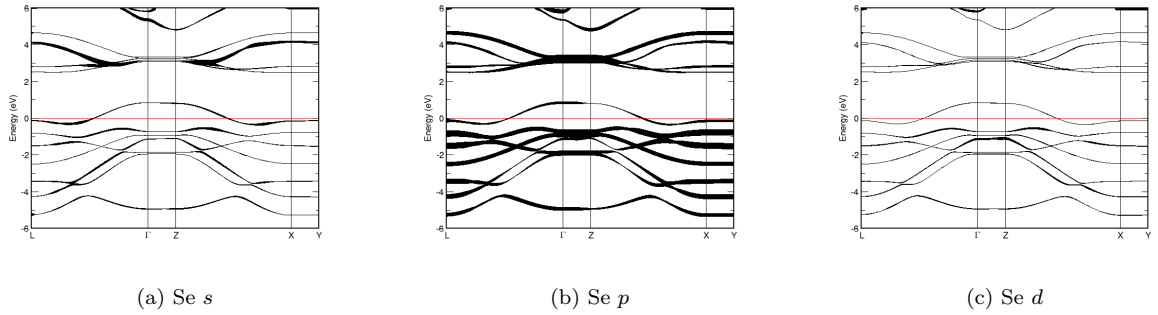

FIG. 141: Fat band representation of Se in NbSe<sub>2</sub>

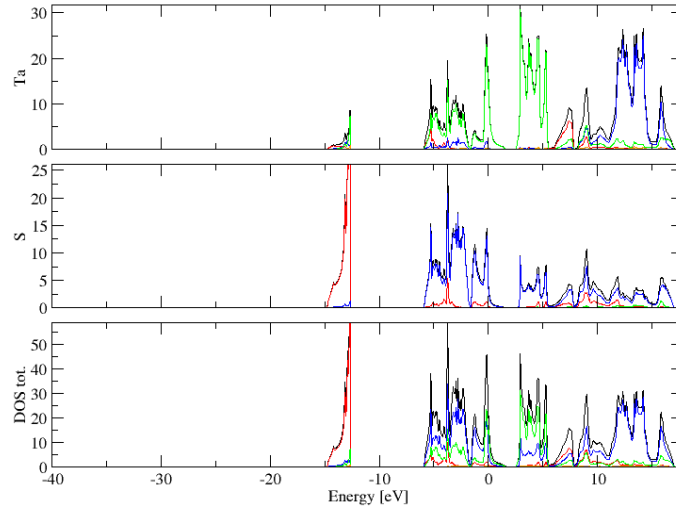

FIG. 142: (Color online) PDOS of TaS<sub>2</sub> (ICSD #280988). The *s*-, *p*- and *d*-projected states are in red, blue and green, respectively. TaS<sub>2</sub> crystallizes in space group F m 2 m (#42), in a orthorhombic face-centred structure.

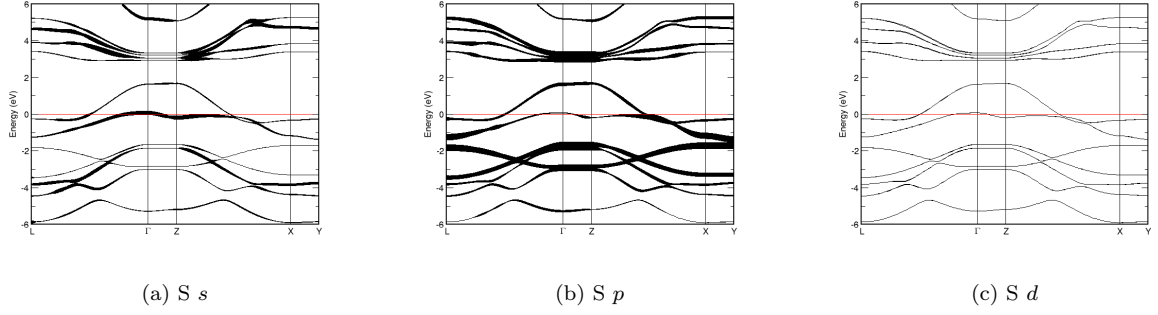

FIG. 143: Fat band representation of S in TaS<sub>2</sub>

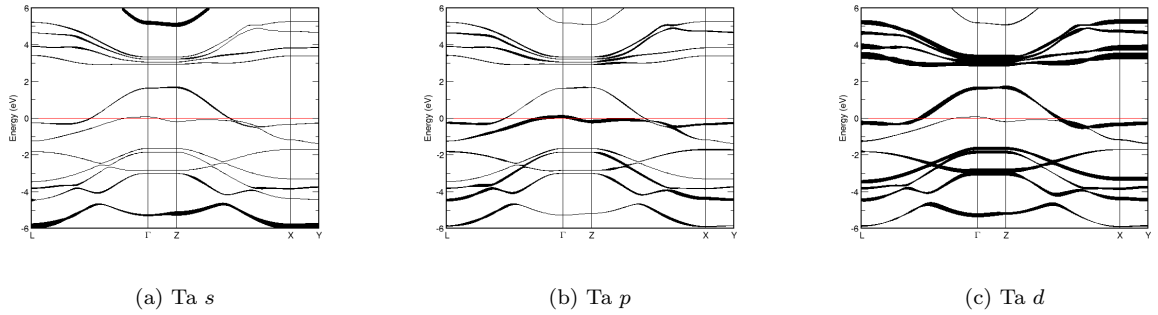

FIG. 144: Fat band representation of Ta in TaS<sub>2</sub>

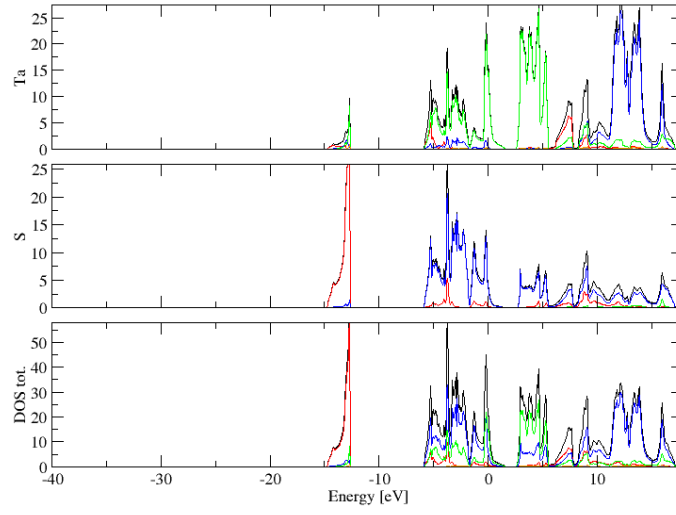

FIG. 145: (Color online) PDOS of TaS<sub>2</sub> (ICSD #67651). The *s*-, *p*- and *d*-projected states are in red, blue and green, respectively. TaS<sub>2</sub> crystallizes in space group *F* 2 *m* *m* (#42), in a orthorhombic face-centred structure.

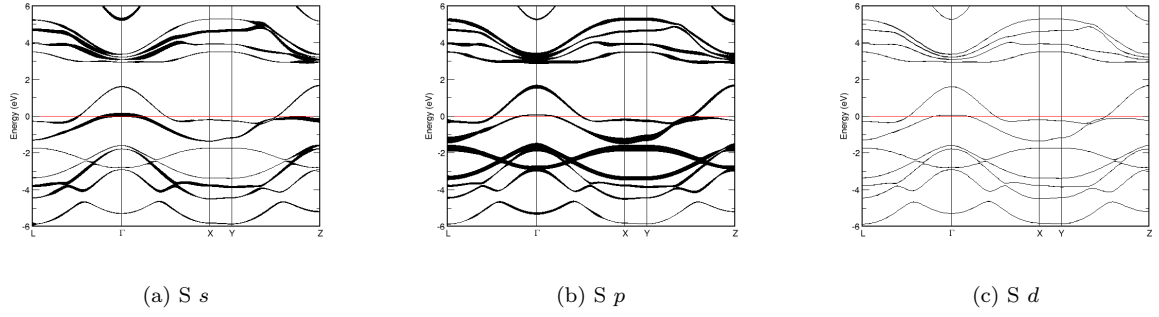

FIG. 146: Fat band representation of S in TaS<sub>2</sub>

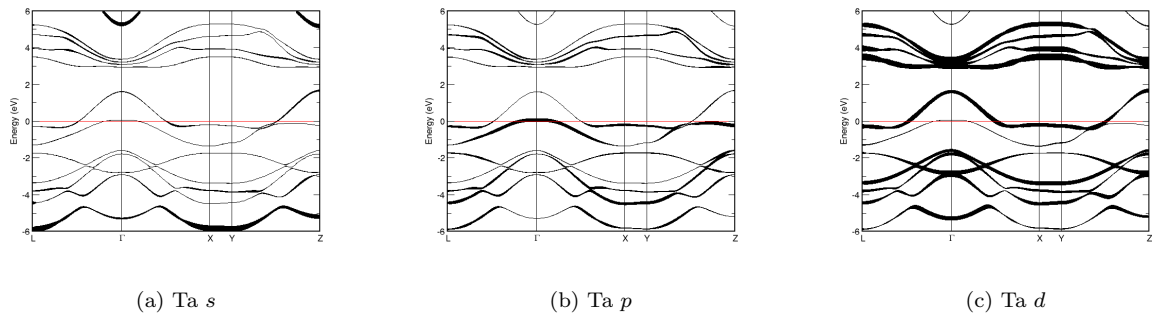

FIG. 147: Fat band representation of Ta in TaS<sub>2</sub>



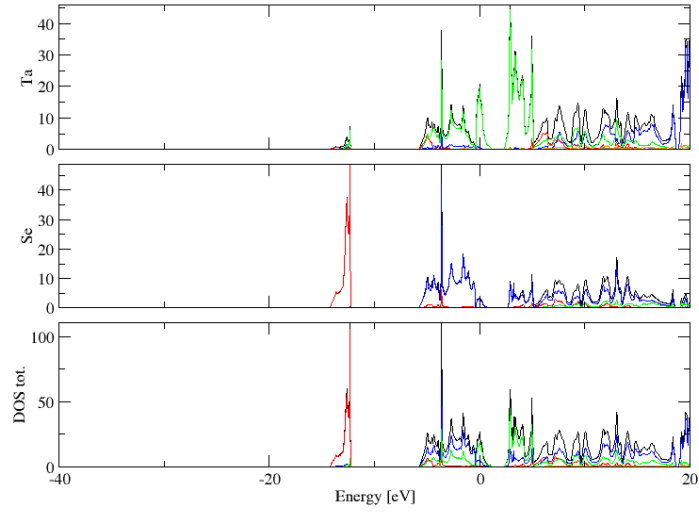

FIG. 148: (Color online) PDOS of TaSe<sub>2</sub> (ICSD #72198). The *s*-, *p*- and *d*-projected states are in red, blue and green, respectively. TaSe<sub>2</sub> crystallizes in space group *F m 2 m* (#42), in a orthorhombic face-centred structure.

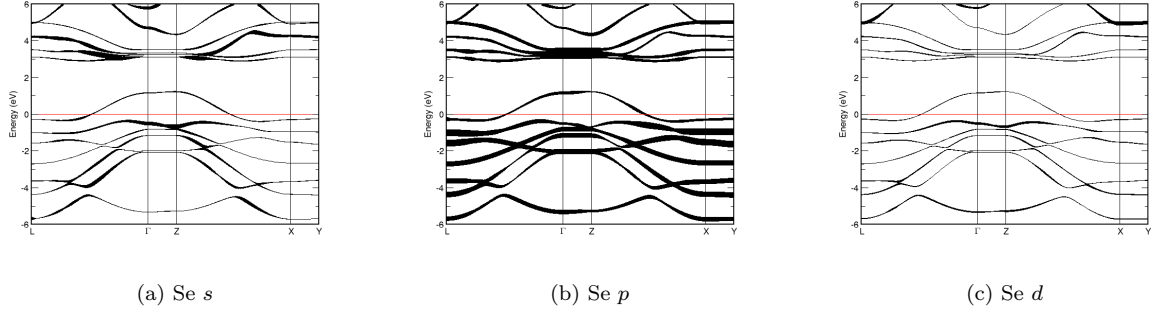

FIG. 149: Fat band representation of Se in TaSe<sub>2</sub>

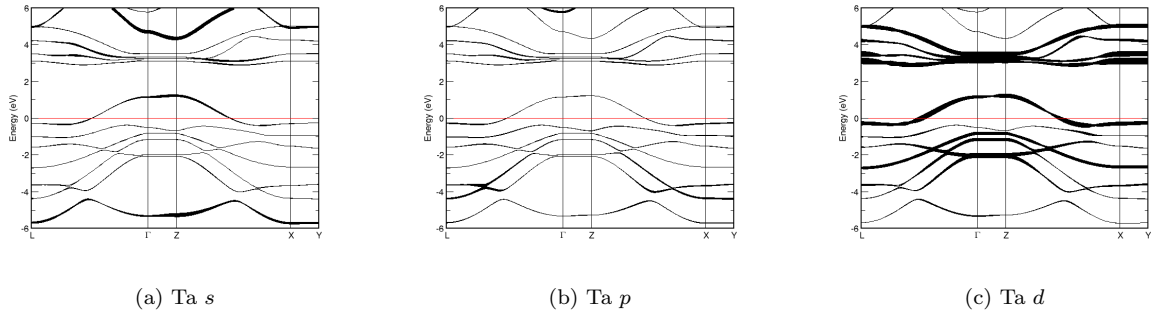

FIG. 150: Fat band representation of Ta in TaSe<sub>2</sub>

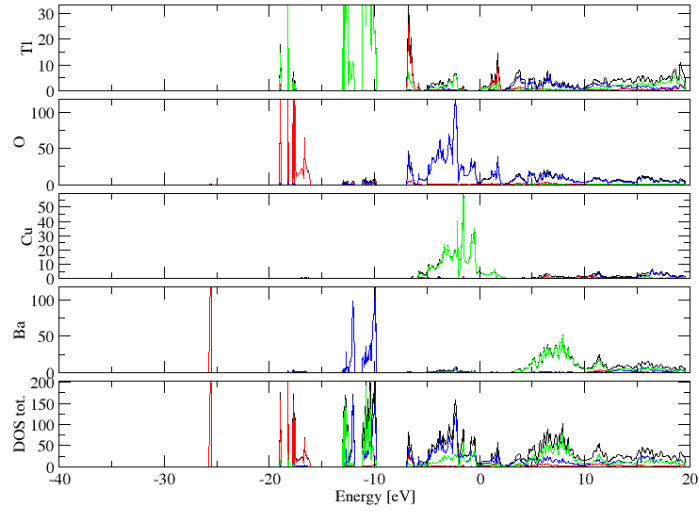

FIG. 151: (Color online) PDOS of  $\text{Tl}_2\text{Ba}_2\text{CuO}_6$  (ICSD #41569). The  $s$ -,  $p$ - and  $d$ -projected states are in red, blue and green, respectively.  $\text{Tl}_2\text{Ba}_2\text{CuO}_6$  crystallizes in space group  $F m m m$  (#69), in a orthorhombic face-centred structure.

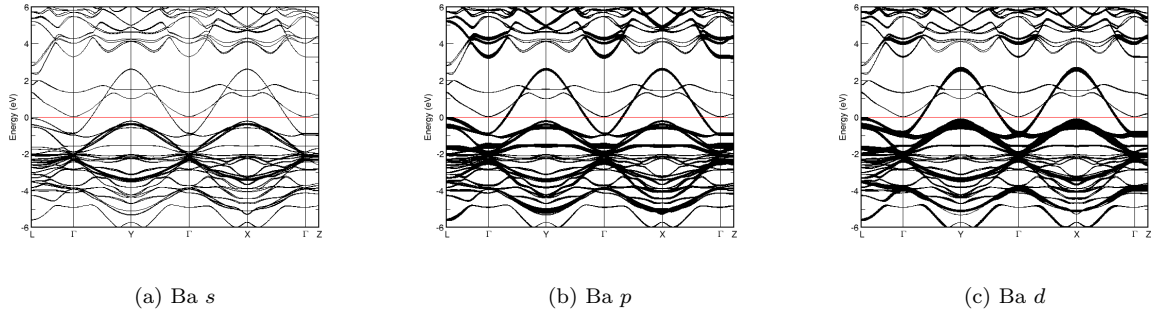

FIG. 152: Fat band representation of Ba in  $\text{Tl}_2\text{Ba}_2\text{CuO}_6$

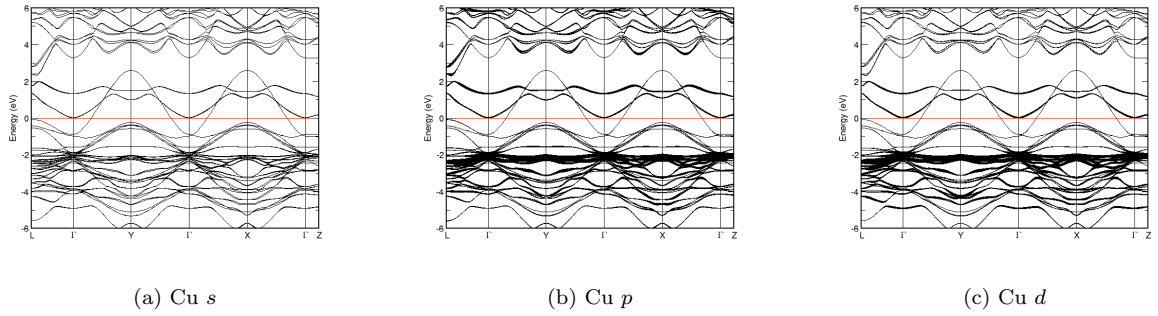

FIG. 153: Fat band representation of Cu in  $\text{Tl}_2\text{Ba}_2\text{CuO}_6$

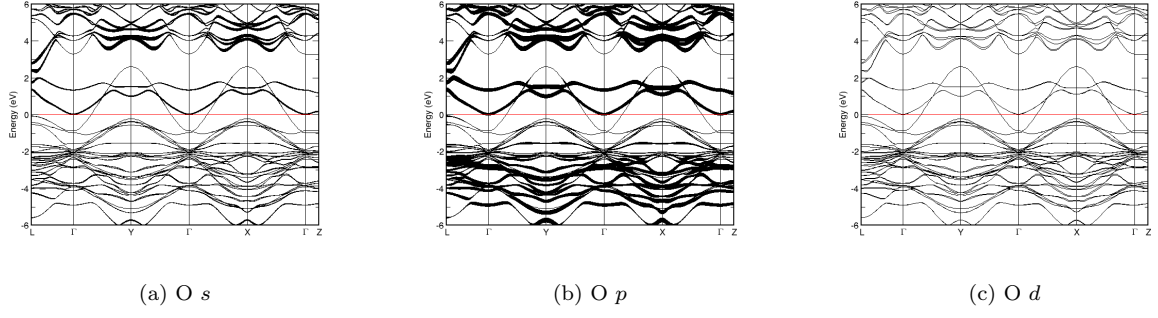FIG. 154: Fat band representation of O in  $\text{Tl}_2\text{Ba}_2\text{CuO}_6$ 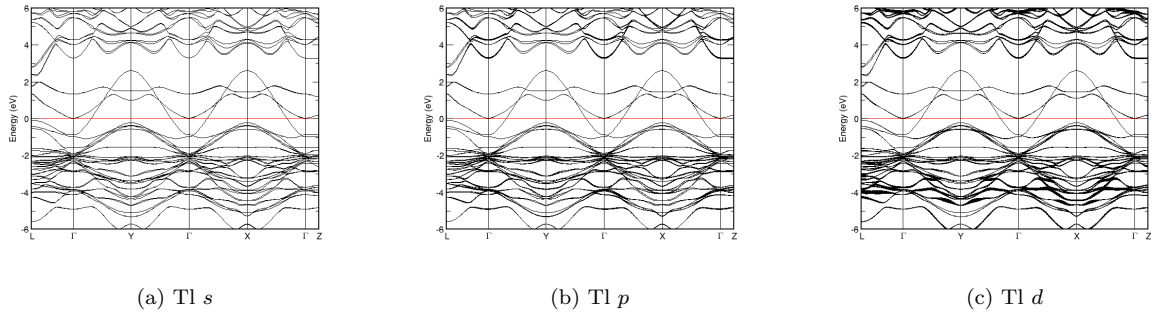FIG. 155: Fat band representation of Tl in  $\text{Tl}_2\text{Ba}_2\text{CuO}_6$ 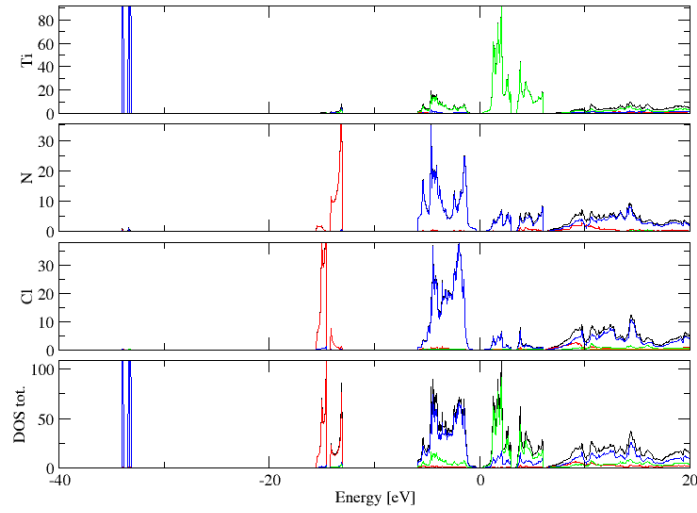FIG. 156: (Color online) PDOS of TiNCI (ICSD #27396). The  $s$ -,  $p$ - and  $d$ -projected states are in red, blue and green, respectively. TiNCI crystallizes in space group  $P m m n$  (#59), in a orthorhombic primitive structure.

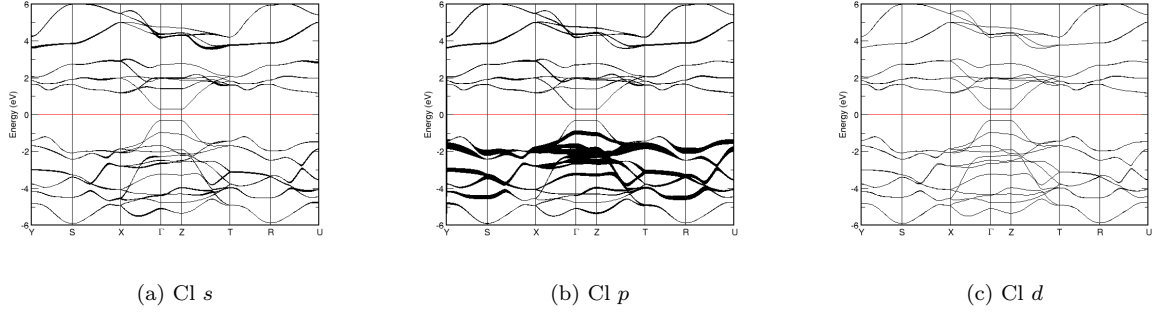

FIG. 157: Fat band representation of Cl in TiNCl

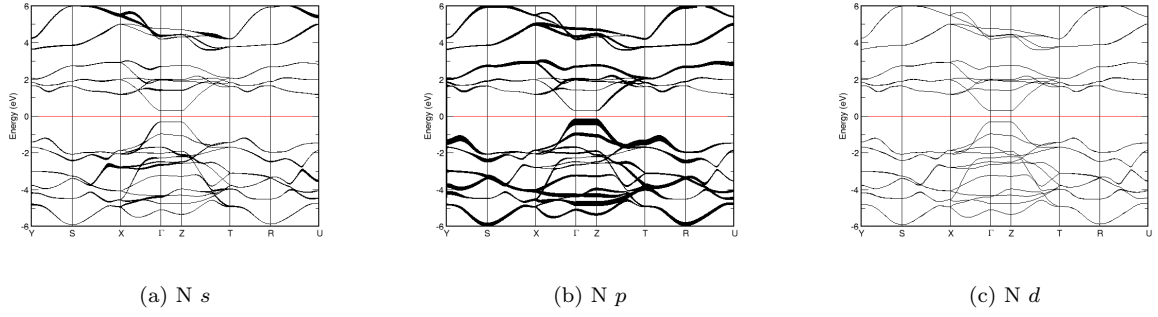

FIG. 158: Fat band representation of N in TiNCl

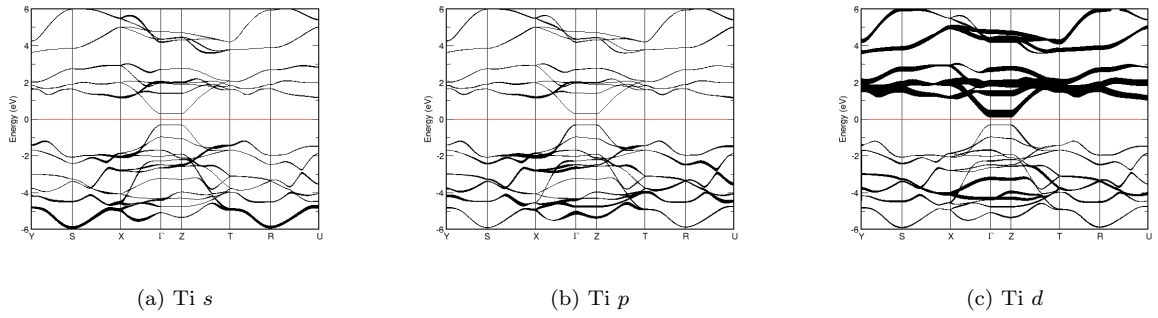

FIG. 159: Fat band representation of Ti in TiNCl

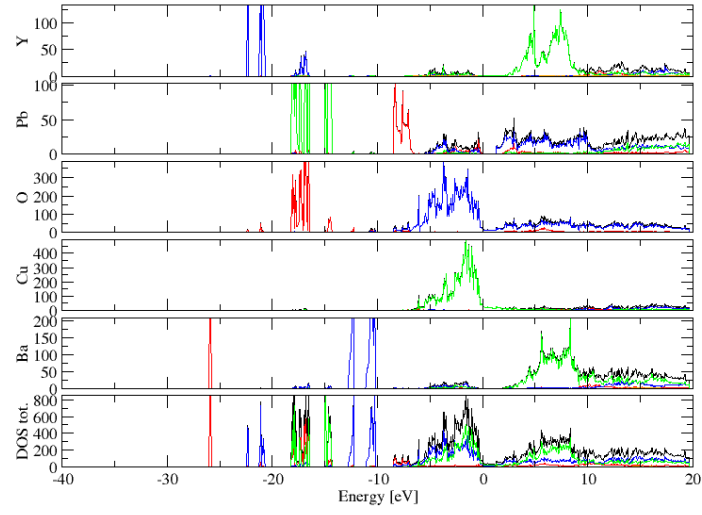

FIG. 160: (Color online) PDOS of  $\text{Pb}_2\text{Ba}_2\text{YCuCu}_2\text{O}_8$  (ICSD #66088). The  $s$ -,  $p$ - and  $d$ -projected states are in red, blue and green, respectively.  $\text{Pb}_2\text{Ba}_2\text{YCuCu}_2\text{O}_8$  crystallizes in space group  $P 2_1 2_1 2$  (#17), in a orthorhombic primitive structure.

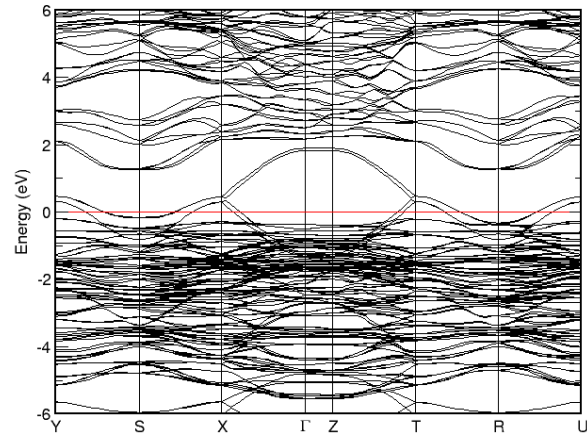

(a)  $E$  vs.  $k$

FIG. 161: Band structure of  $\text{Pb}_2\text{Ba}_2\text{YCuCu}_2\text{O}_8$

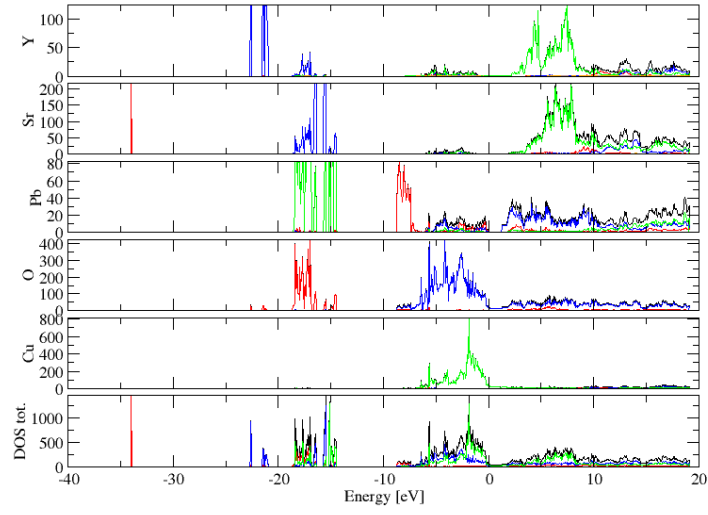

FIG. 162: (Color online) PDOS of  $\text{Pb}_2\text{Sr}_2\text{YCu}_3\text{O}_8$  (ICSD #66587). The  $s$ -,  $p$ - and  $d$ -projected states are in red, blue and green, respectively.  $\text{Pb}_2\text{Sr}_2\text{YCu}_3\text{O}_8$  crystallizes in space group  $P 2_1 2$  (#17), in a orthorhombic primitive structure.

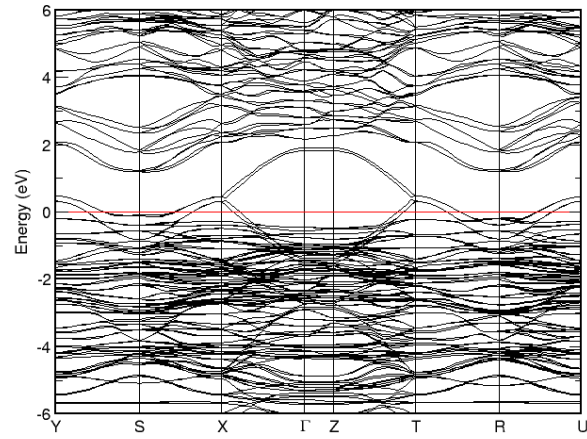

(a)  $E$  vs.  $k$

FIG. 163: Band structure of  $\text{Pb}_2\text{Sr}_2\text{YCu}_3\text{O}_8$

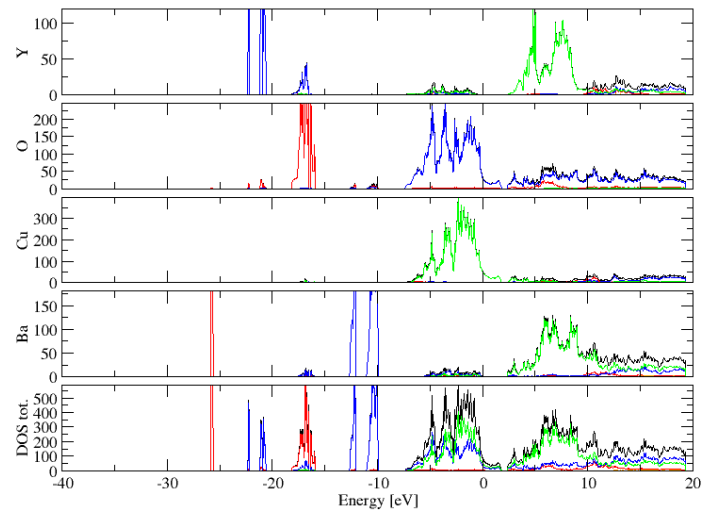

FIG. 164: (Color online) PDOS of  $\text{YBa}_2\text{Cu}_3\text{O}_{6.5}$  (ICSD #75697). The  $s$ -,  $p$ - and  $d$ -projected states are in red, blue and green, respectively.  $\text{YBa}_2\text{Cu}_3\text{O}_{6.5}$  crystallizes in space group  $P m m m$  (#47), in a orthorhombic primitive structure.

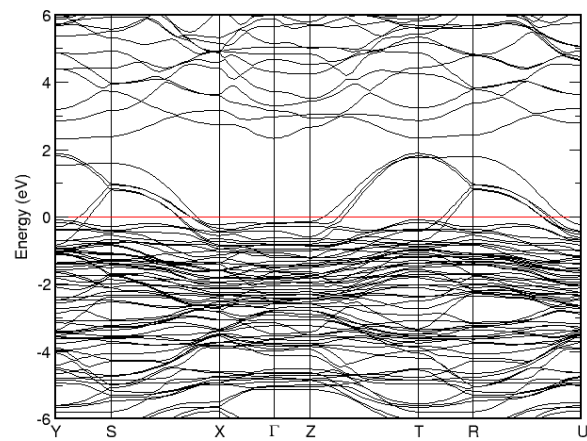

(a)  $E$  vs.  $k$

FIG. 165: Band structure of  $\text{YBa}_2\text{Cu}_3\text{O}_{6.5}$

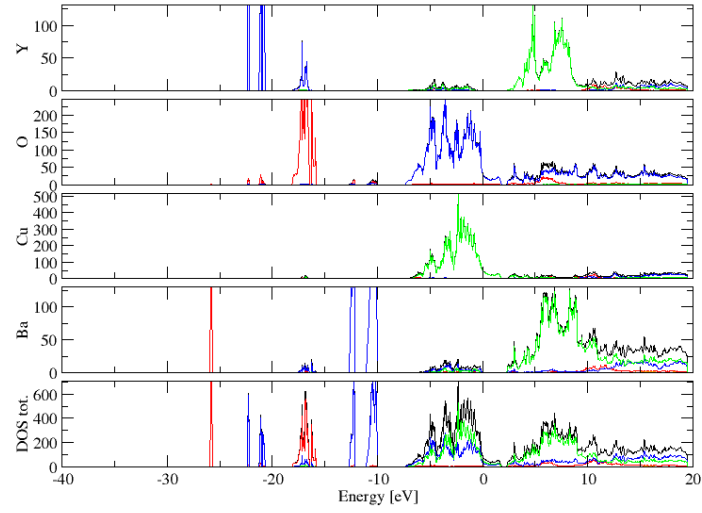

FIG. 166: (Color online) PDOS of  $\text{YBa}_2\text{Cu}_3\text{O}_{6.5}$  (ICSD #96016). The  $s$ -,  $p$ - and  $d$ -projected states are in red, blue and green, respectively.  $\text{YBa}_2\text{Cu}_3\text{O}_{6.5}$  crystallizes in space group  $P m m m$  (#47), in a orthorhombic primitive structure.

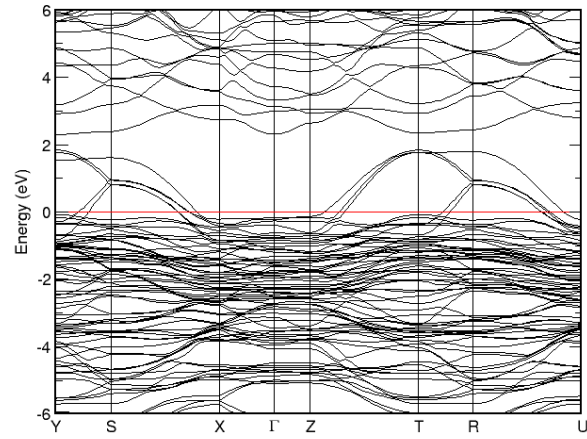

(a)  $E$  vs.  $k$

FIG. 167: Band structure of  $\text{YBa}_2\text{Cu}_3\text{O}_{6.5}$



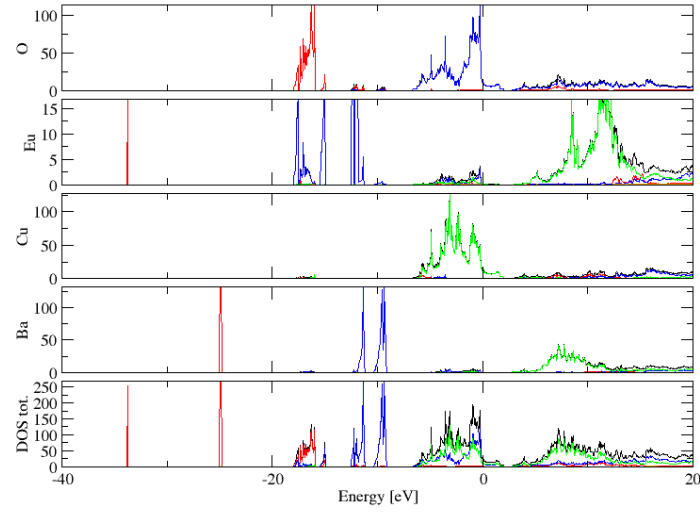

FIG. 168: (Color online) PDOS of  $\text{EuBa}_2\text{Cu}_3\text{O}_7$  (ICSD #81171). The  $s$ -,  $p$ - and  $d$ -projected states are in red, blue and green, respectively.  $\text{EuBa}_2\text{Cu}_3\text{O}_7$  crystallizes in space group  $P m m m$  (#47), in a orthorhombic primitive structure.

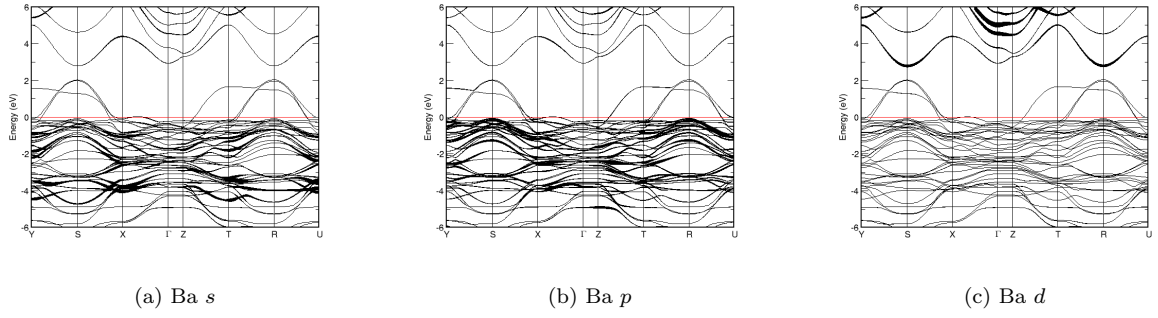

FIG. 169: Fat band representation of Ba in  $\text{EuBa}_2\text{Cu}_3\text{O}_7$

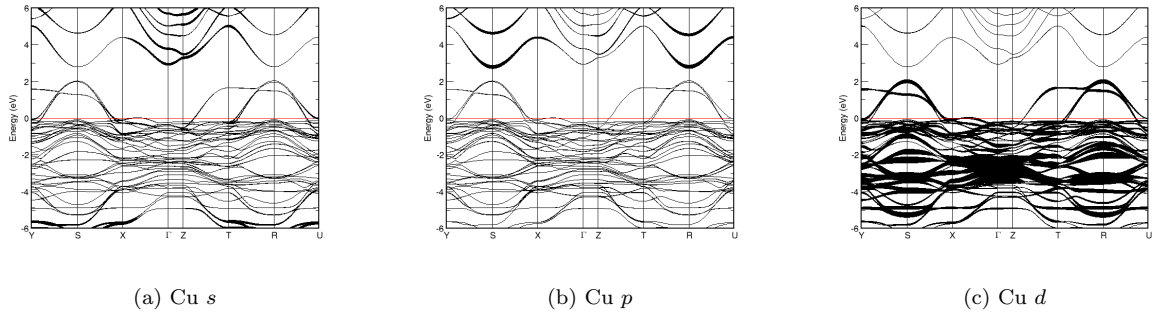

FIG. 170: Fat band representation of Cu in  $\text{EuBa}_2\text{Cu}_3\text{O}_7$

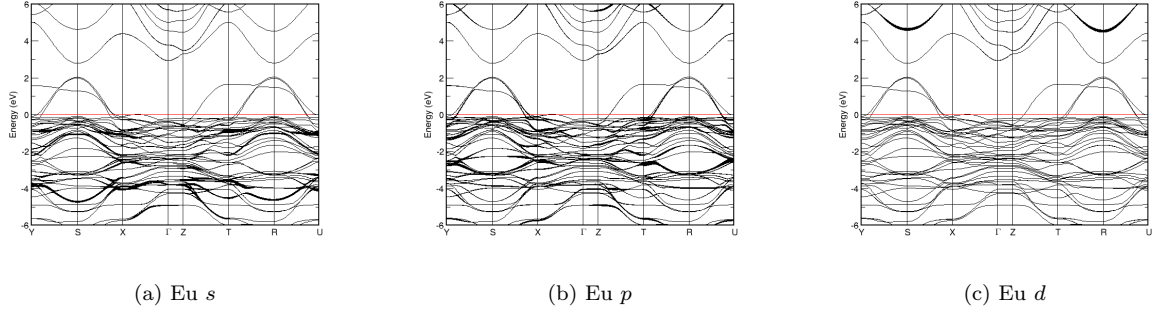FIG. 171: Fat band representation of Eu in  $\text{EuBa}_2\text{Cu}_3\text{O}_7$ 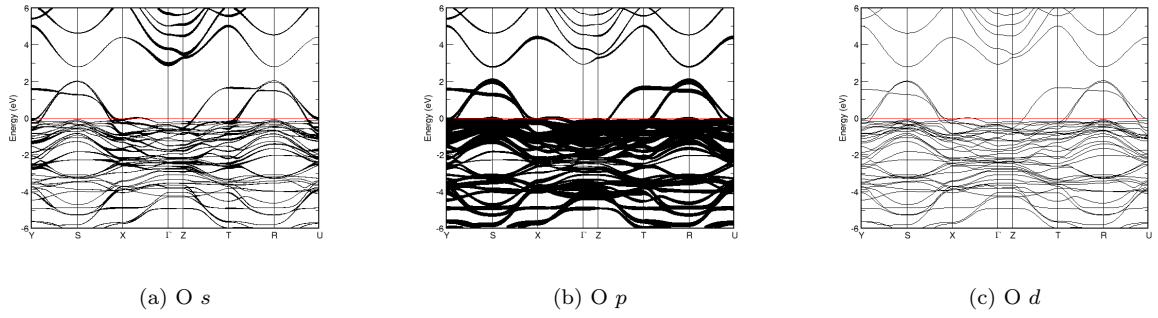FIG. 172: Fat band representation of O in  $\text{EuBa}_2\text{Cu}_3\text{O}_7$ 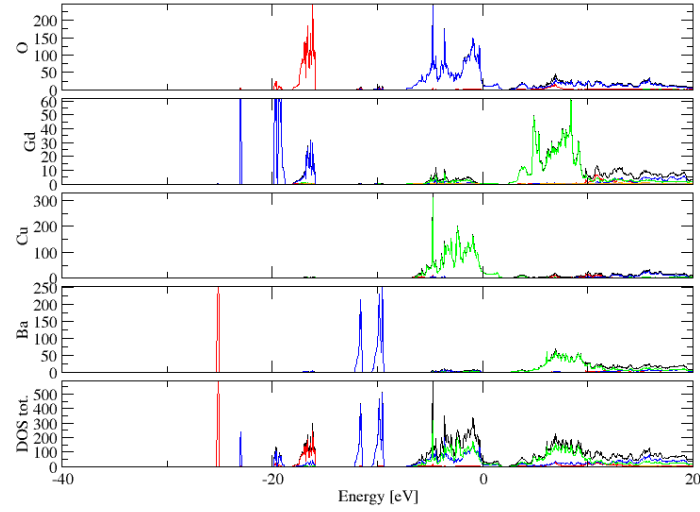

FIG. 173: (Color online) PDOS of  $\text{Ba}_2\text{GdCu}_3\text{O}_7$  (ICSD #56514). The *s*-, *p*- and *d*-projected states are in red, blue and green, respectively.  $\text{Ba}_2\text{GdCu}_3\text{O}_7$  crystallizes in space group  $P m m m$  (#47), in a orthorhombic primitive structure.

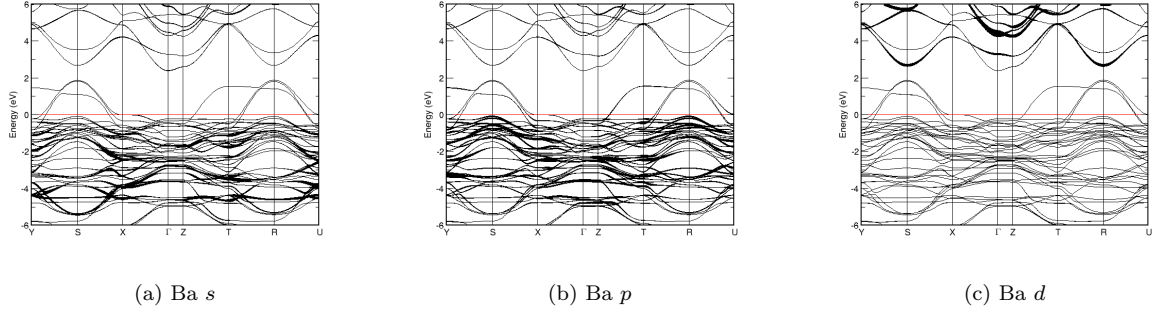FIG. 174: Fat band representation of Ba in  $\text{Ba}_2\text{GdCu}_3\text{O}_7$ 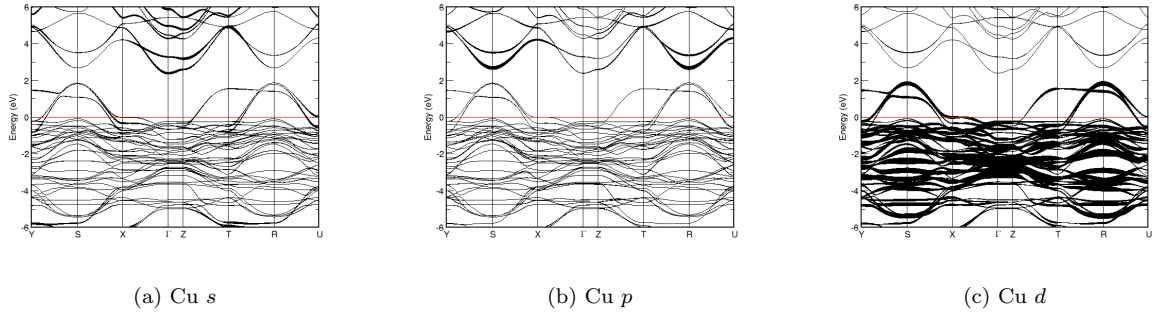FIG. 175: Fat band representation of Cu in  $\text{Ba}_2\text{GdCu}_3\text{O}_7$ 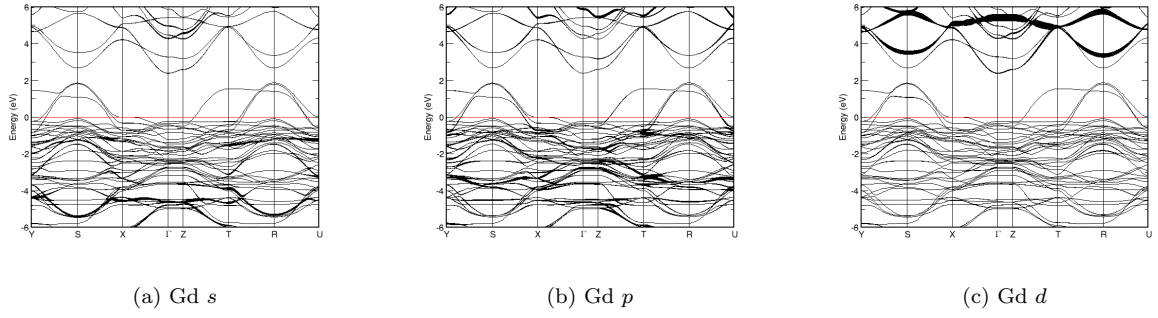FIG. 176: Fat band representation of Gd in  $\text{Ba}_2\text{GdCu}_3\text{O}_7$ 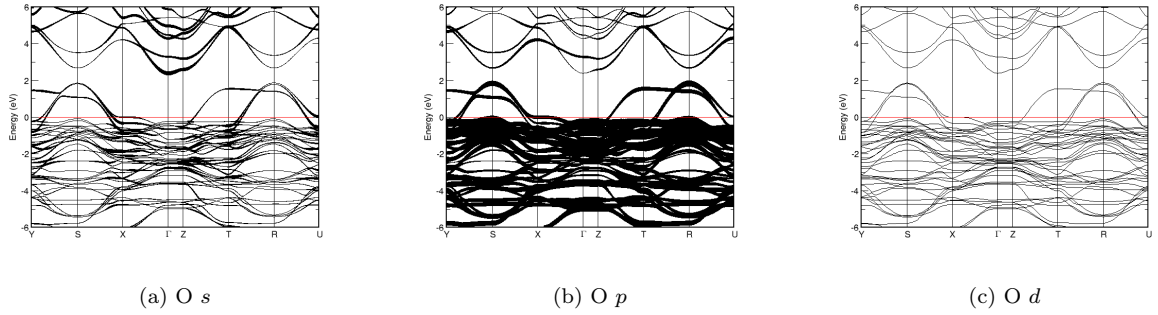FIG. 177: Fat band representation of O in  $\text{Ba}_2\text{GdCu}_3\text{O}_7$

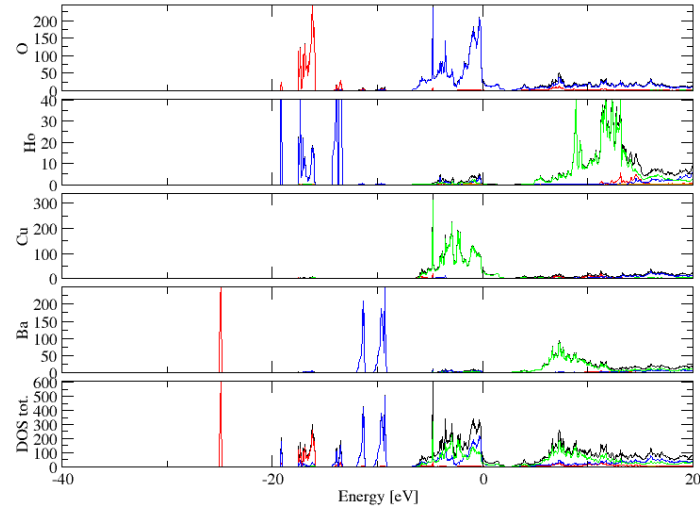

FIG. 178: (Color online) PDOS of  $\text{HoBa}_2\text{Cu}_3\text{O}_7$  (ICSD #68044). The  $s$ -,  $p$ - and  $d$ -projected states are in red, blue and green, respectively.  $\text{HoBa}_2\text{Cu}_3\text{O}_7$  crystallizes in space group  $P m m m$  (#47), in a orthorhombic primitive structure.

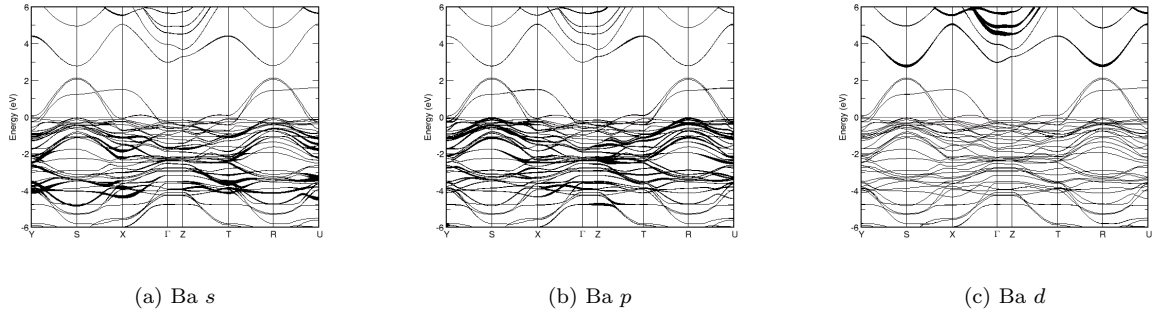

FIG. 179: Fat band representation of Ba in  $\text{HoBa}_2\text{Cu}_3\text{O}_7$

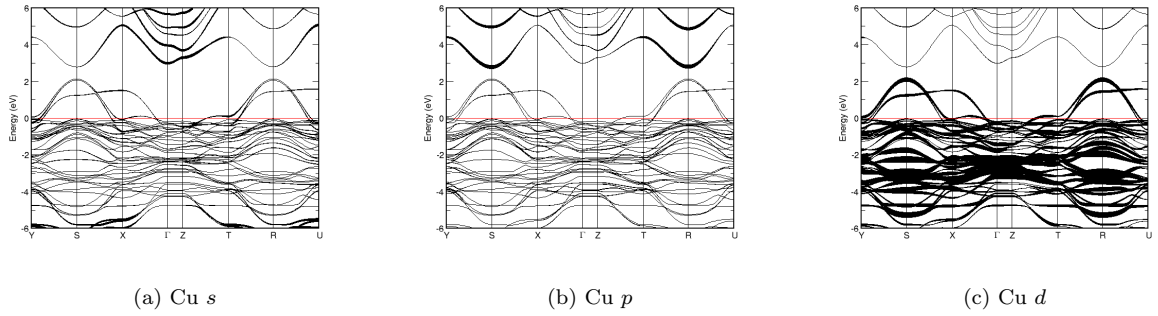

FIG. 180: Fat band representation of Cu in  $\text{HoBa}_2\text{Cu}_3\text{O}_7$

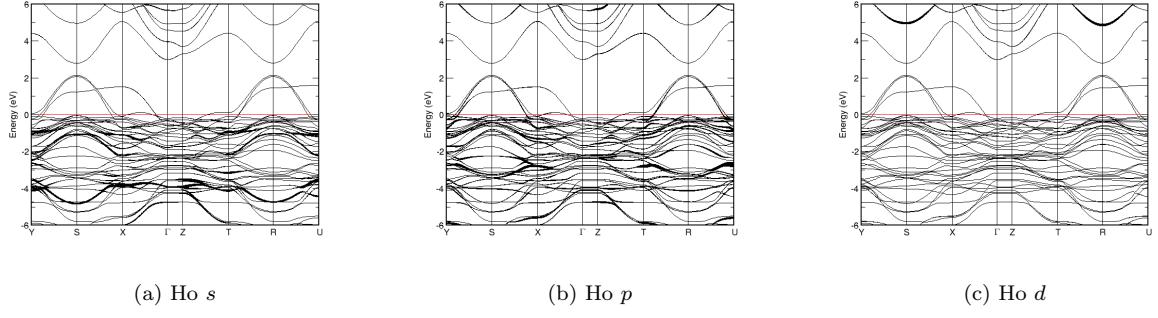FIG. 181: Fat band representation of Ho in  $\text{HoBa}_2\text{Cu}_3\text{O}_7$ 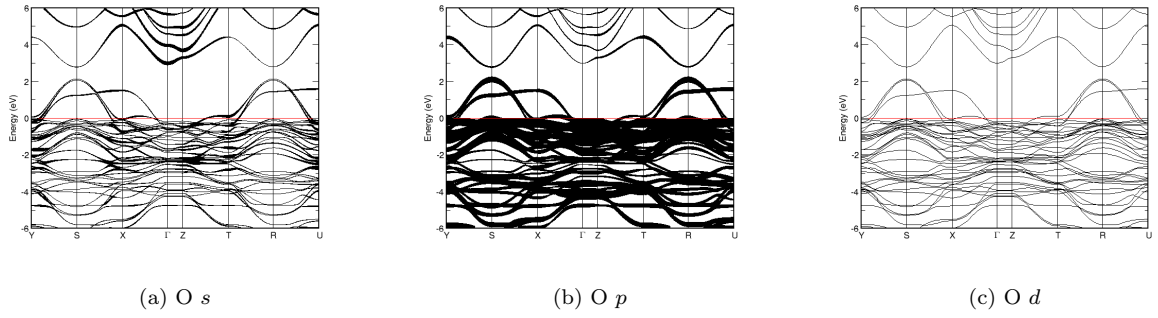FIG. 182: Fat band representation of O in  $\text{HoBa}_2\text{Cu}_3\text{O}_7$ 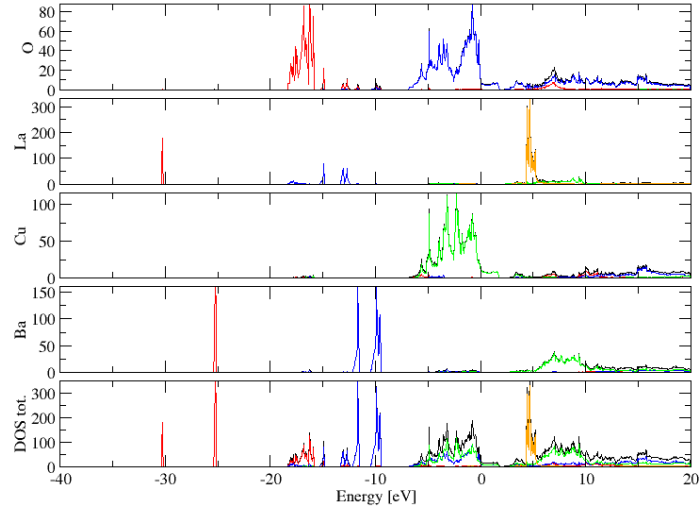FIG. 183: (Color online) PDOS of  $\text{LaBa}_2\text{Cu}_3\text{O}_7$  (ICSD #81167). The *s*-, *p*- and *d*-projected states are in red, blue and green, respectively.  $\text{LaBa}_2\text{Cu}_3\text{O}_7$  crystallizes in space group  $P m m m$  (#47), in a orthorhombic primitive structure.

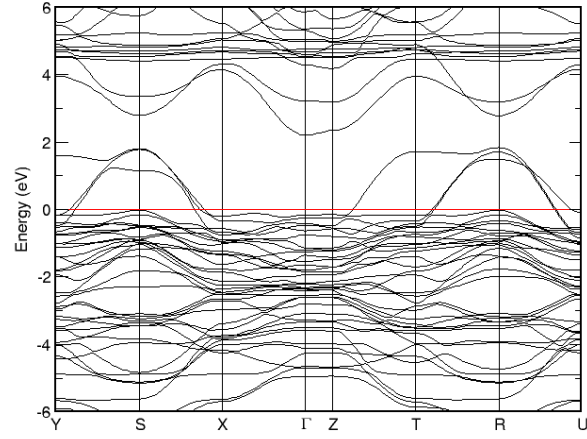(a)  $E$  vs.  $k$ FIG. 184: Band structure of  $\text{LaBa}_2\text{Cu}_3\text{O}_7$ 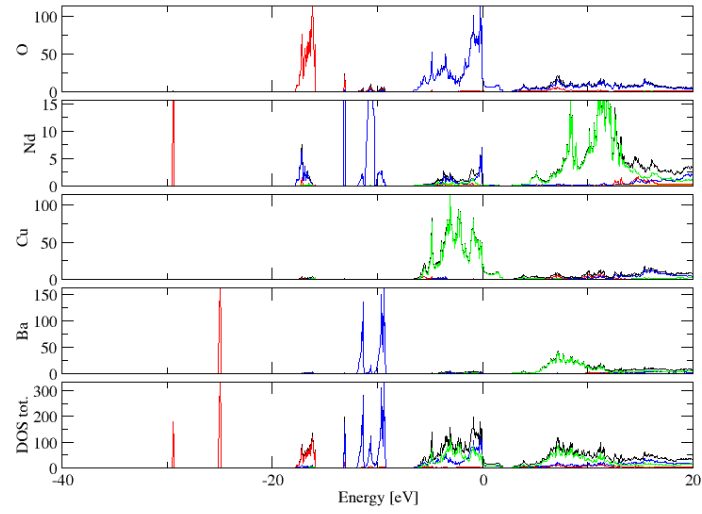

FIG. 185: (Color online) PDOS of  $\text{NdBa}_2\text{Cu}_3\text{O}_7$  (ICSD #81169). The  $s$ -,  $p$ - and  $d$ -projected states are in red, blue and green, respectively.  $\text{NdBa}_2\text{Cu}_3\text{O}_7$  crystallizes in space group  $P m m m$  (#47), in a orthorhombic primitive structure.

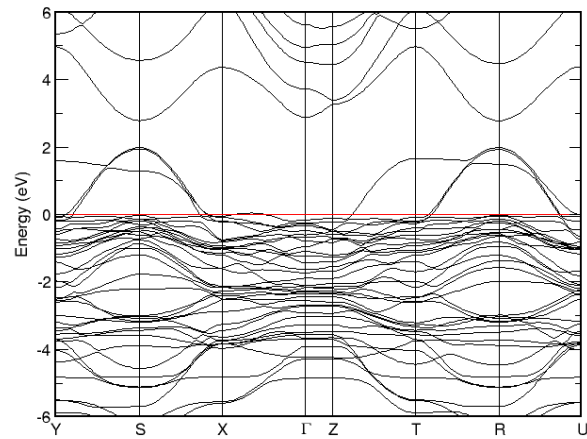(a)  $E$  vs.  $k$ FIG. 186: Band structure of  $\text{NdBa}_2\text{Cu}_3\text{O}_7$ 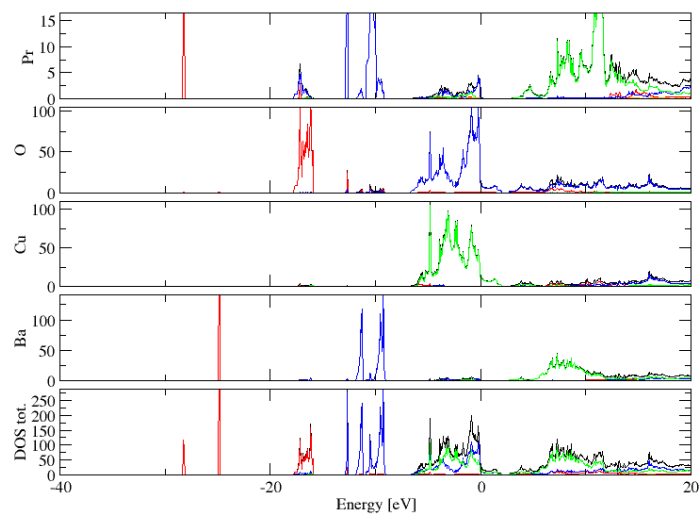

FIG. 187: (Color online) PDOS of  $\text{PrBa}_2\text{Cu}_3\text{O}_7$  (ICSD #81168). The  $s$ -,  $p$ - and  $d$ -projected states are in red, blue and green, respectively.  $\text{PrBa}_2\text{Cu}_3\text{O}_7$  crystallizes in space group  $P m m m$  (#47), in a orthorhombic primitive structure.

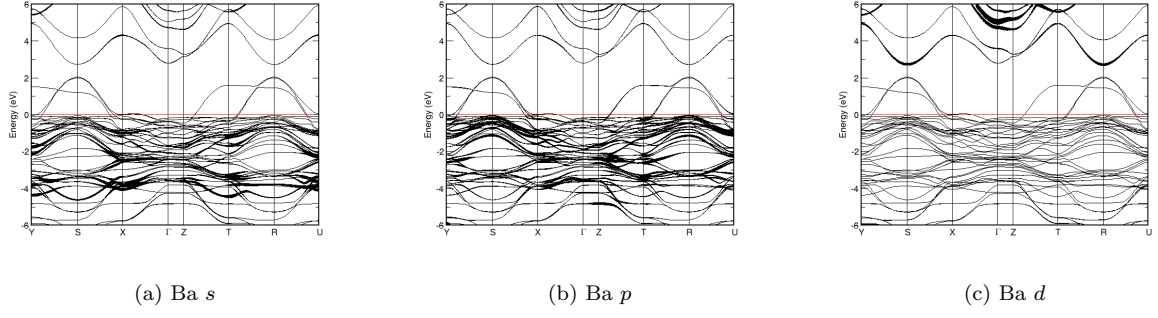FIG. 188: Fat band representation of Ba in  $\text{PrBa}_2\text{Cu}_3\text{O}_7$ 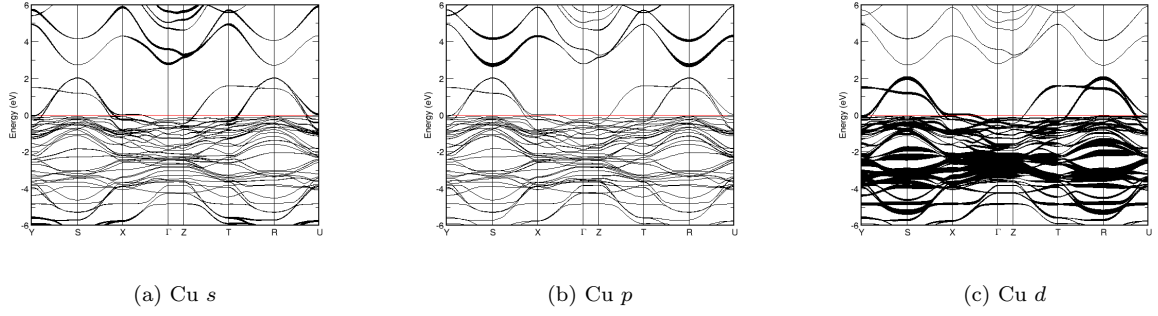FIG. 189: Fat band representation of Cu in  $\text{PrBa}_2\text{Cu}_3\text{O}_7$ 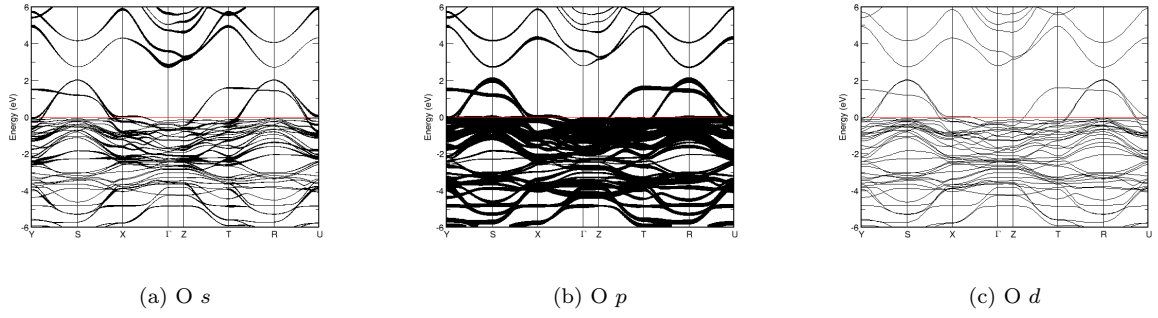FIG. 190: Fat band representation of O in  $\text{PrBa}_2\text{Cu}_3\text{O}_7$ 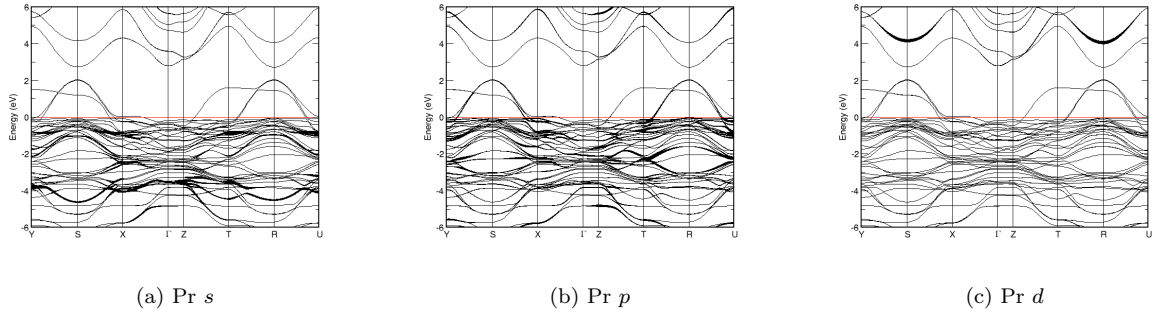FIG. 191: Fat band representation of Pr in  $\text{PrBa}_2\text{Cu}_3\text{O}_7$



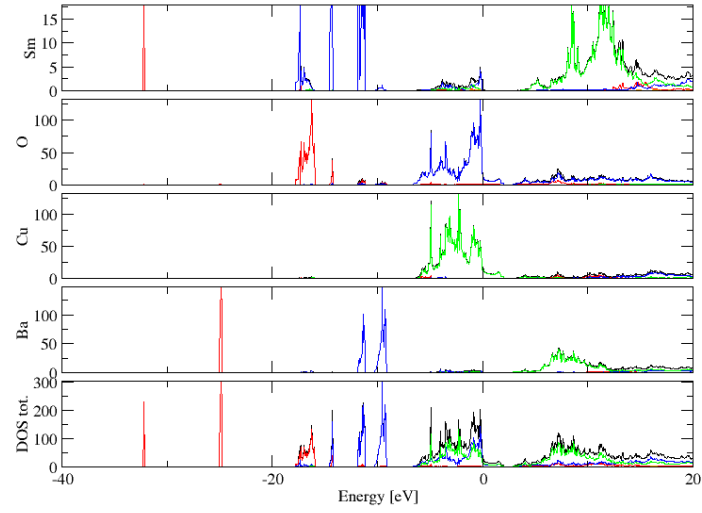

FIG. 192: (Color online) PDOS of  $\text{SmBa}_2\text{Cu}_3\text{O}_7$  (ICSD #71705). The  $s$ -,  $p$ - and  $d$ -projected states are in red, blue and green, respectively.  $\text{SmBa}_2\text{Cu}_3\text{O}_7$  crystallizes in space group  $P m m m$  (#47), in a orthorhombic primitive structure.

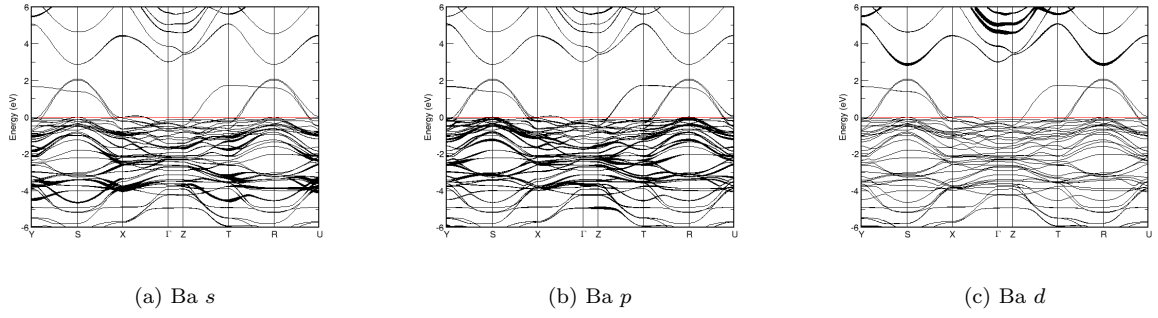

FIG. 193: Fat band representation of Ba in  $\text{SmBa}_2\text{Cu}_3\text{O}_7$

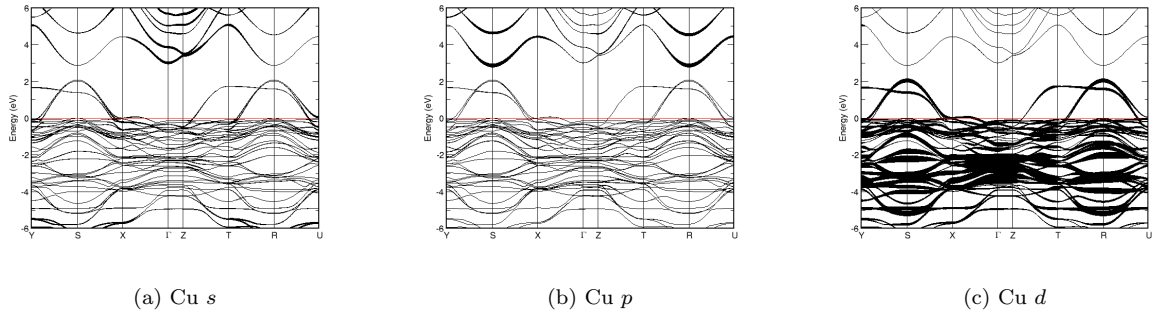

FIG. 194: Fat band representation of Cu in  $\text{SmBa}_2\text{Cu}_3\text{O}_7$

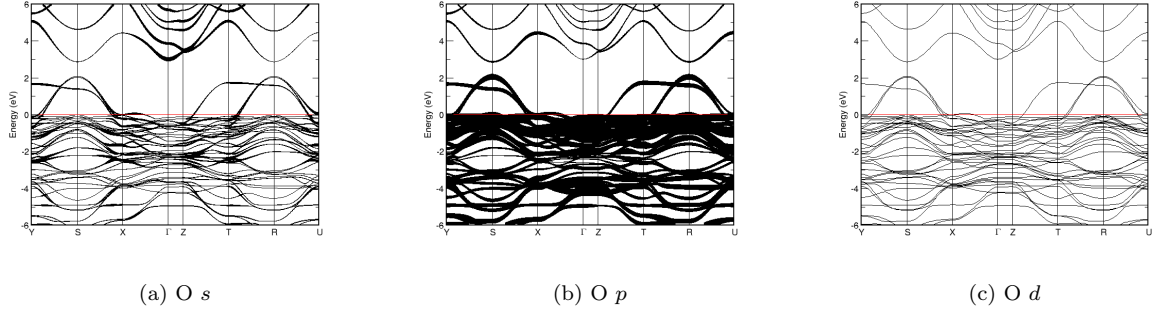FIG. 195: Fat band representation of O in  $\text{SmBa}_2\text{Cu}_3\text{O}_7$ 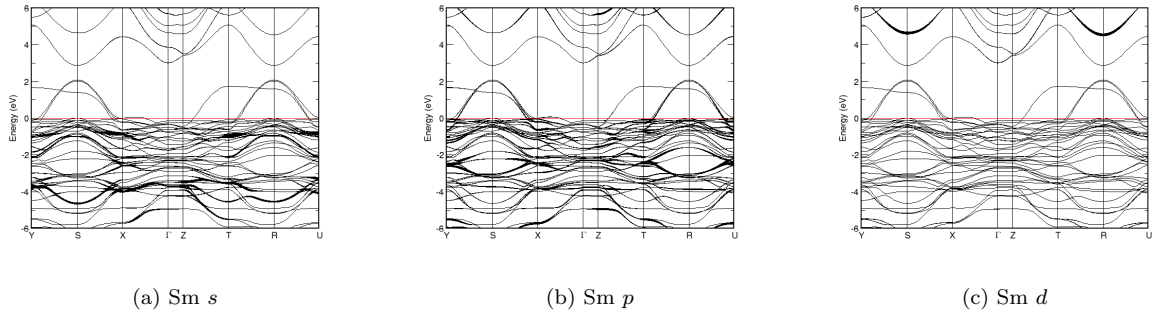FIG. 196: Fat band representation of Sm in  $\text{SmBa}_2\text{Cu}_3\text{O}_7$ 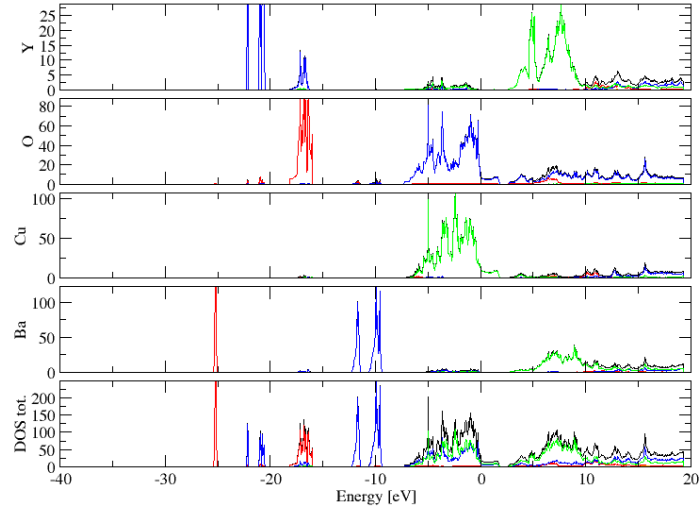

FIG. 197: (Color online) PDOS of  $\text{Ba}_2\text{YCu}_3\text{O}_7$  (ICSD #202770). The *s*-, *p*- and *d*-projected states are in red, blue and green, respectively.  $\text{Ba}_2\text{YCu}_3\text{O}_7$  crystallizes in space group  $P m m m$  (#47), in a orthorhombic primitive structure.

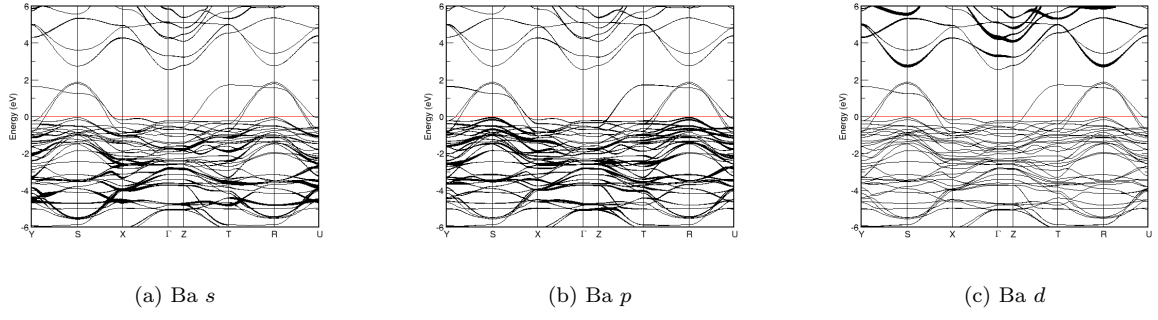FIG. 198: Fat band representation of Ba in  $\text{Ba}_2\text{YCu}_3\text{O}_7$ 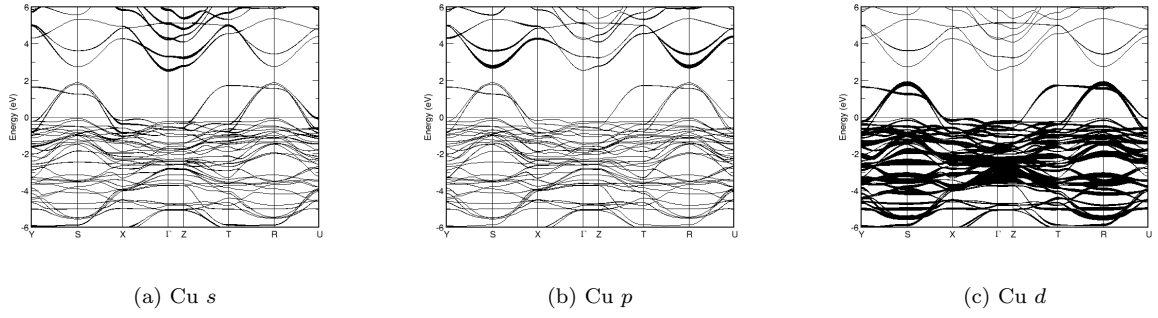FIG. 199: Fat band representation of Cu in  $\text{Ba}_2\text{YCu}_3\text{O}_7$ 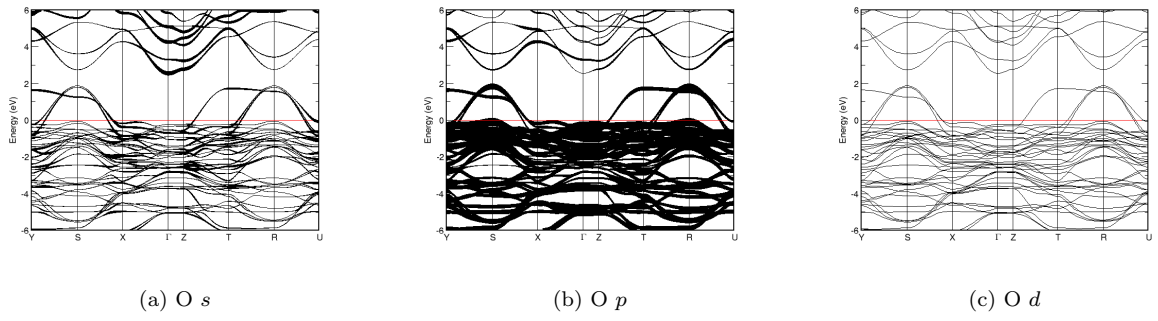FIG. 200: Fat band representation of O in  $\text{Ba}_2\text{YCu}_3\text{O}_7$ 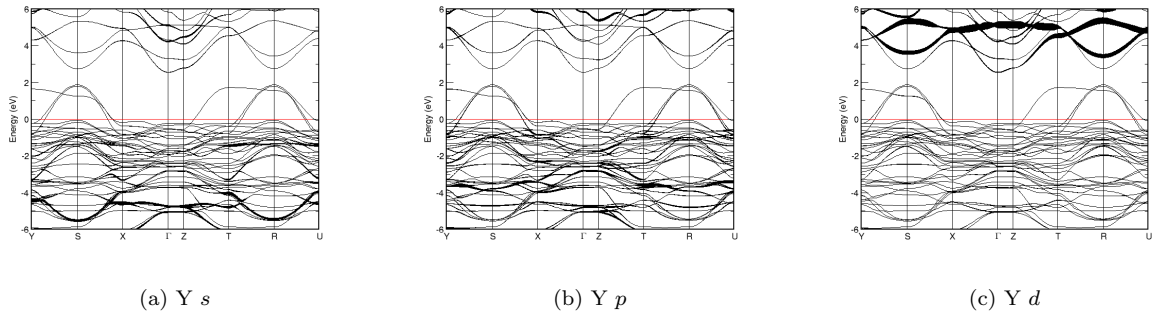FIG. 201: Fat band representation of Y in  $\text{Ba}_2\text{YCu}_3\text{O}_7$

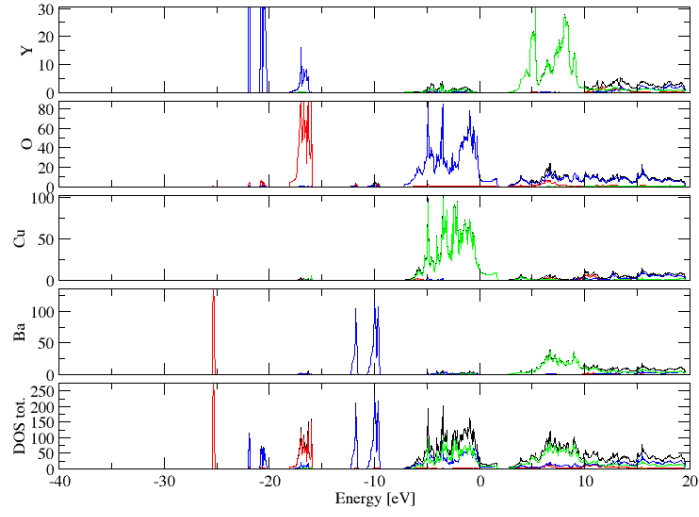

FIG. 202: (Color online) PDOS of  $\text{Ba}_2\text{YCu}_3\text{O}_7$  (ICSD #77737). The  $s$ -,  $p$ - and  $d$ -projected states are in red, blue and green, respectively.  $\text{Ba}_2\text{YCu}_3\text{O}_7$  crystallizes in space group  $P m m m$  (#47), in a orthorhombic primitive structure.

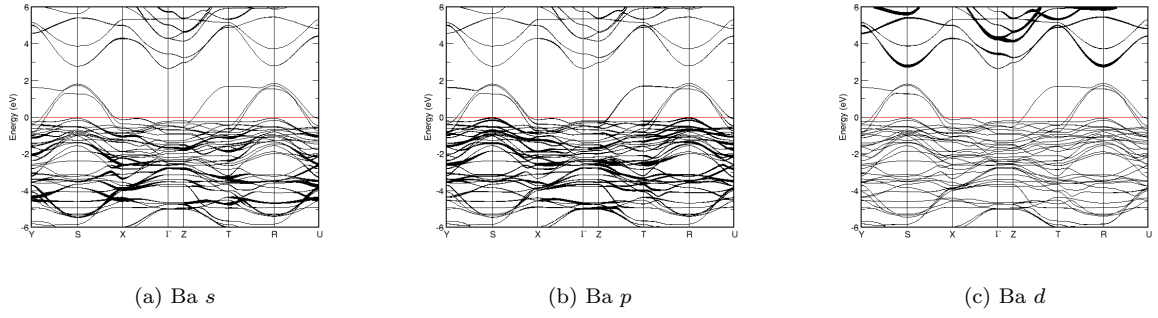

FIG. 203: Fat band representation of Ba in  $\text{Ba}_2\text{YCu}_3\text{O}_7$

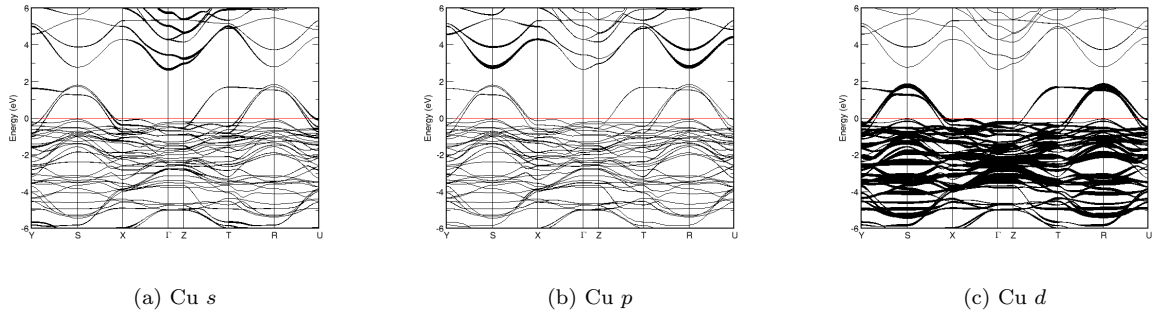

FIG. 204: Fat band representation of Cu in  $\text{Ba}_2\text{YCu}_3\text{O}_7$

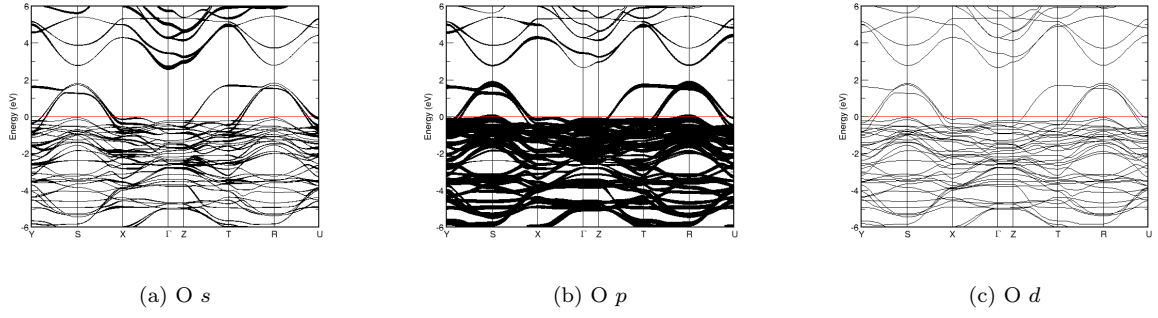FIG. 205: Fat band representation of O in  $\text{Ba}_2\text{YCu}_3\text{O}_7$ 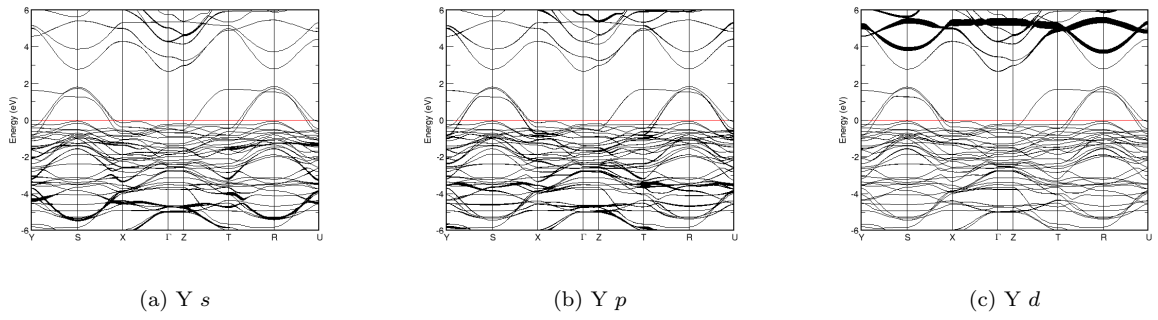FIG. 206: Fat band representation of Y in  $\text{Ba}_2\text{YCu}_3\text{O}_7$ 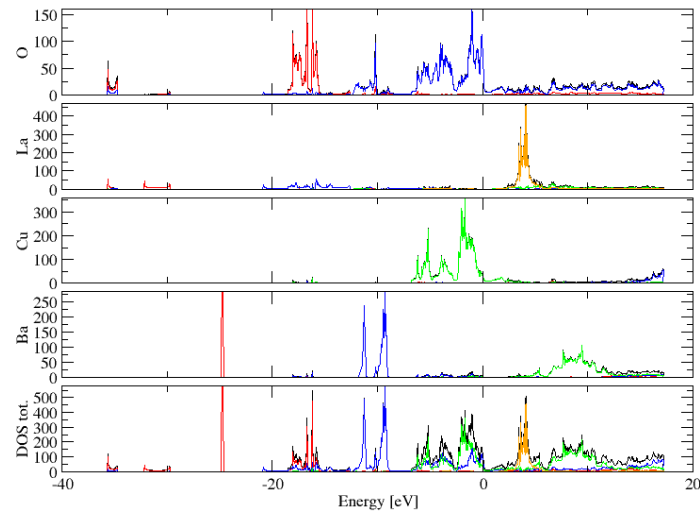

FIG. 207: (Color online) PDOS of  $\text{LaBa}_2\text{Cu}_3\text{O}_8$  (ICSD #85291). The *s*-, *p*- and *d*-projected states are in red, blue and green, respectively.  $\text{LaBa}_2\text{Cu}_3\text{O}_8$  crystallizes in space group  $P m m m$  (#47), in a orthorhombic primitive structure.

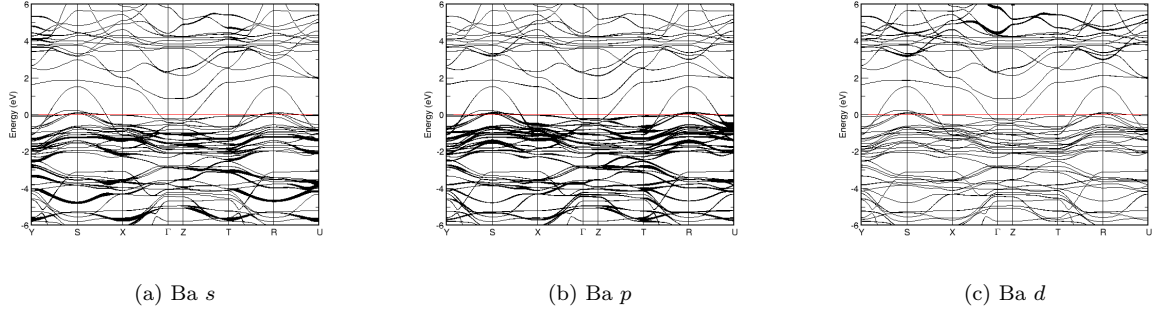FIG. 208: Fat band representation of Ba in  $\text{LaBa}_2\text{Cu}_3\text{O}_8$ 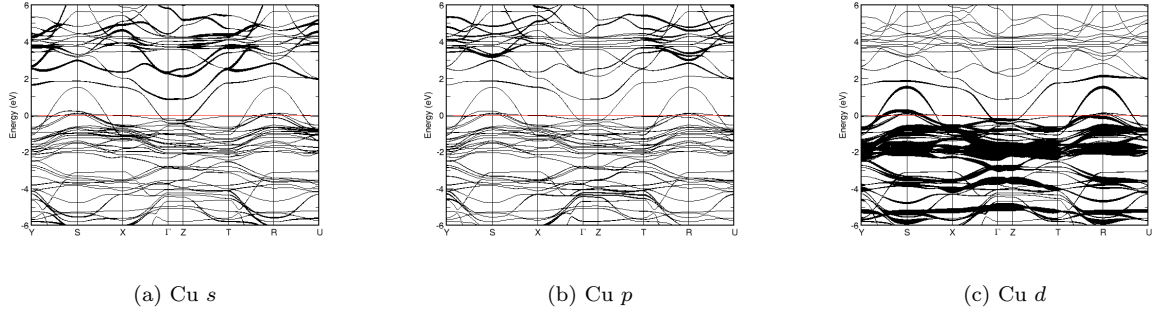FIG. 209: Fat band representation of Cu in  $\text{LaBa}_2\text{Cu}_3\text{O}_8$ 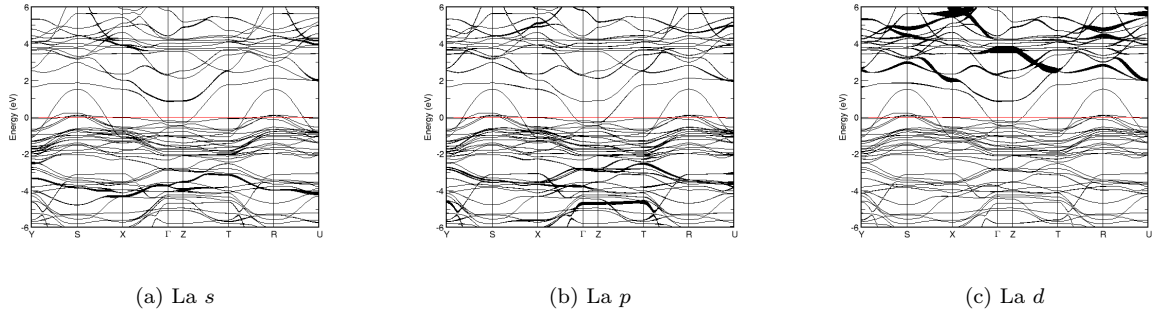FIG. 210: Fat band representation of La in  $\text{LaBa}_2\text{Cu}_3\text{O}_8$ 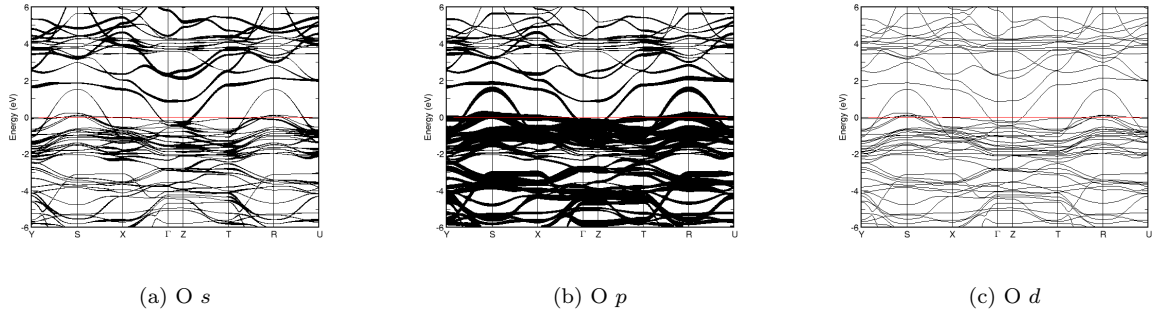FIG. 211: Fat band representation of O in  $\text{LaBa}_2\text{Cu}_3\text{O}_8$

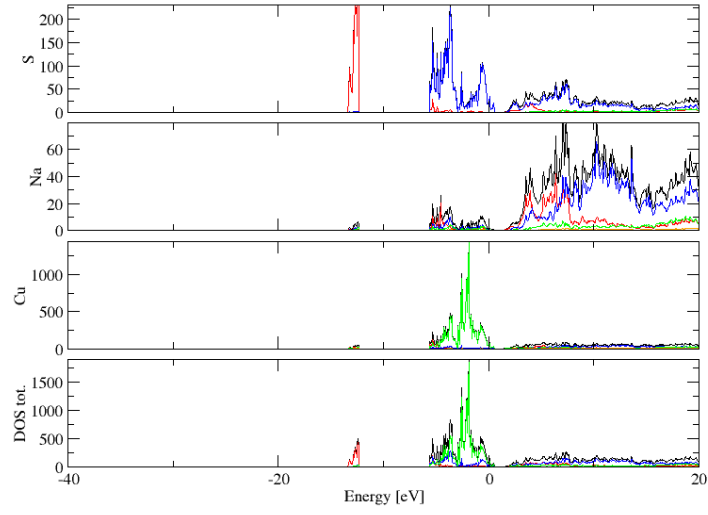

FIG. 212: (Color online) PDOS of  $\text{Na}_3\text{Cu}_4\text{S}_4$  (ICSD #10004). The  $s$ -,  $p$ - and  $d$ -projected states are in red, blue and green, respectively.  $\text{Na}_3\text{Cu}_4\text{S}_4$  crystallizes in space group  $P b a m$  (#55), in a orthorhombic primitive structure.

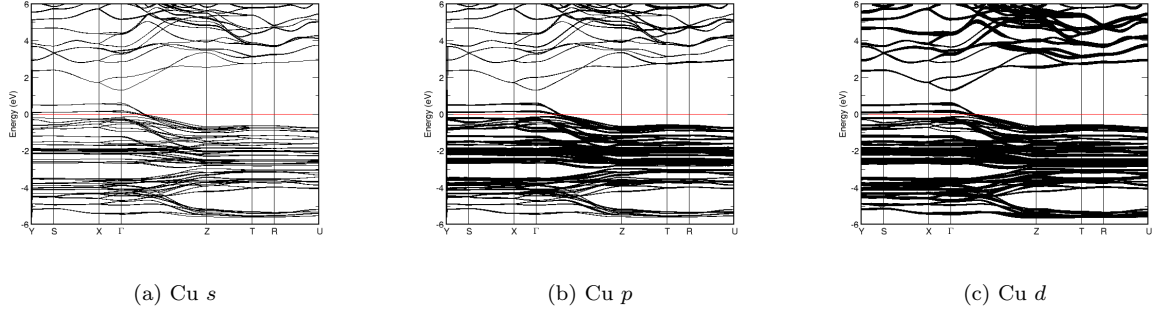

FIG. 213: Fat band representation of Cu in  $\text{Na}_3\text{Cu}_4\text{S}_4$

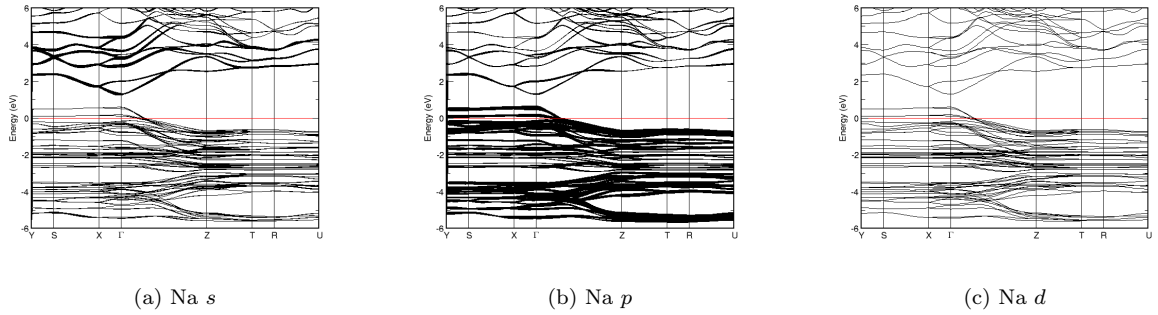

FIG. 214: Fat band representation of Na in  $\text{Na}_3\text{Cu}_4\text{S}_4$

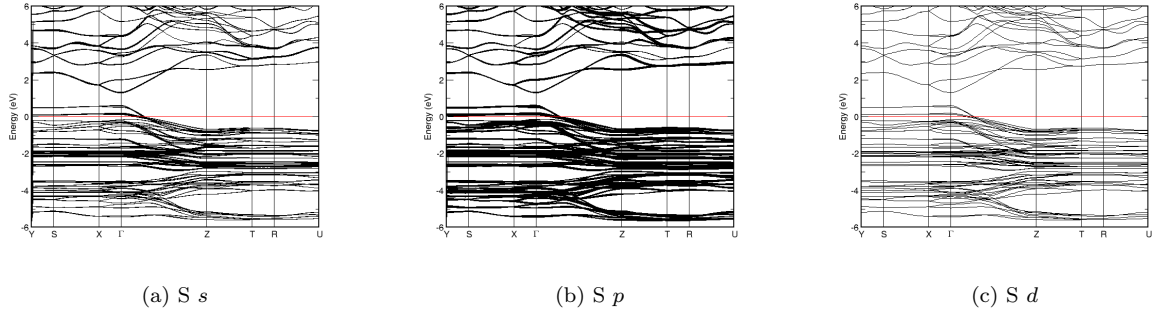FIG. 215: Fat band representation of S in  $\text{Na}_3\text{Cu}_4\text{S}_4$ 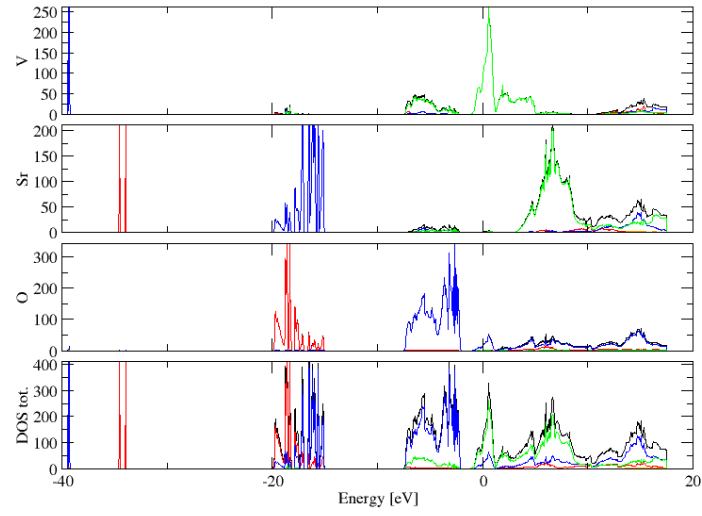FIG. 216: (Color online) PDOS of  $\text{Sr}_4\text{V}_3\text{O}_{10}$  (ICSD #73698). The *s*-, *p*- and *d*-projected states are in red, blue and green, respectively.  $\text{Sr}_4\text{V}_3\text{O}_{10}$  crystallizes in space group  $I 4/m m m$  (#139), in a tetragonal body-centred structure.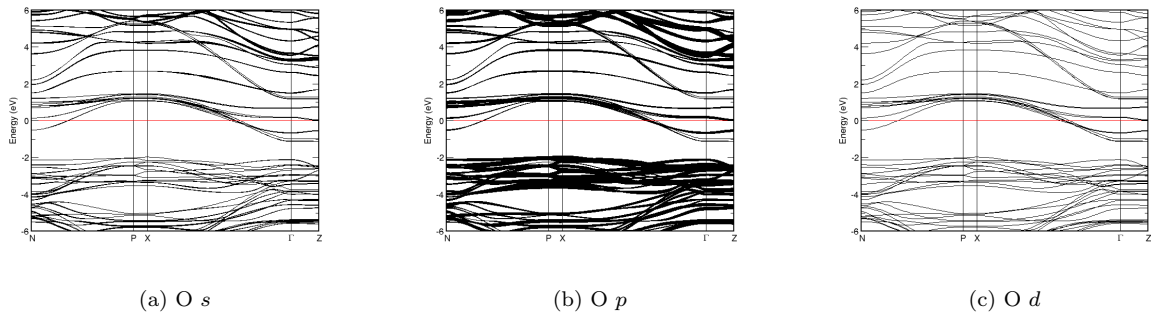FIG. 217: Fat band representation of O in  $\text{Sr}_4\text{V}_3\text{O}_{10}$



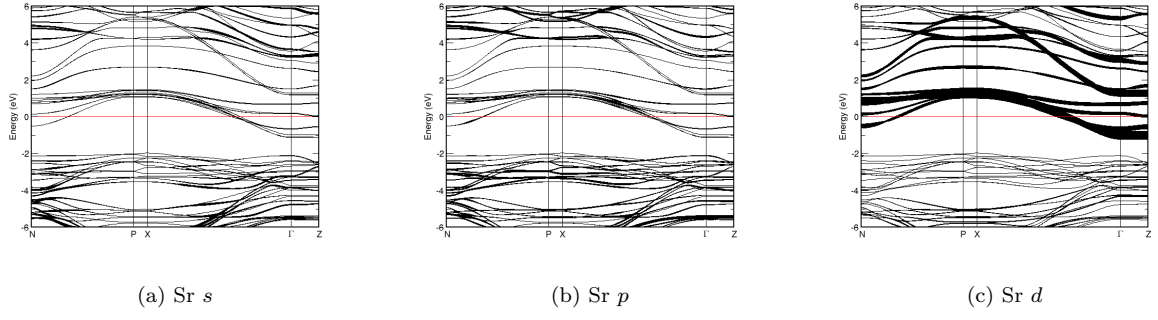FIG. 218: Fat band representation of Sr in  $\text{Sr}_4\text{V}_3\text{O}_{10}$ 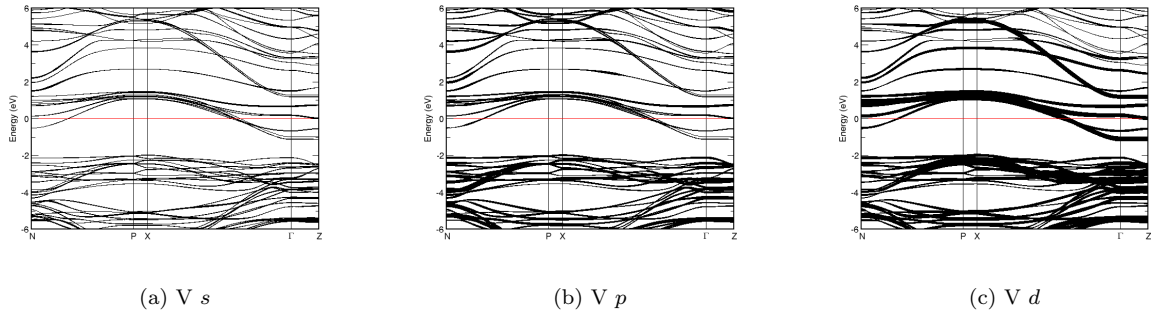FIG. 219: Fat band representation of V in  $\text{Sr}_4\text{V}_3\text{O}_{10}$ 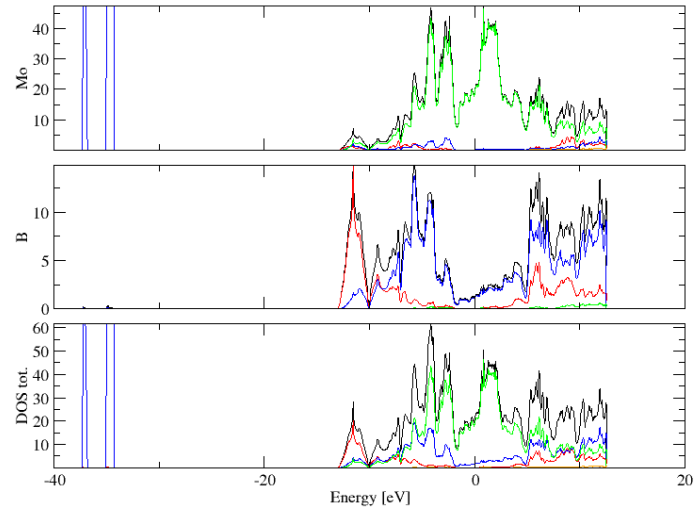FIG. 220: (Color online) PDOS of MoB (ICSD #24280). The *s*-, *p*- and *d*-projected states are in red, blue and green, respectively. MoB crystallizes in space group  $I 41/a m d S$  (#141), in a tetragonal body-centred structure.

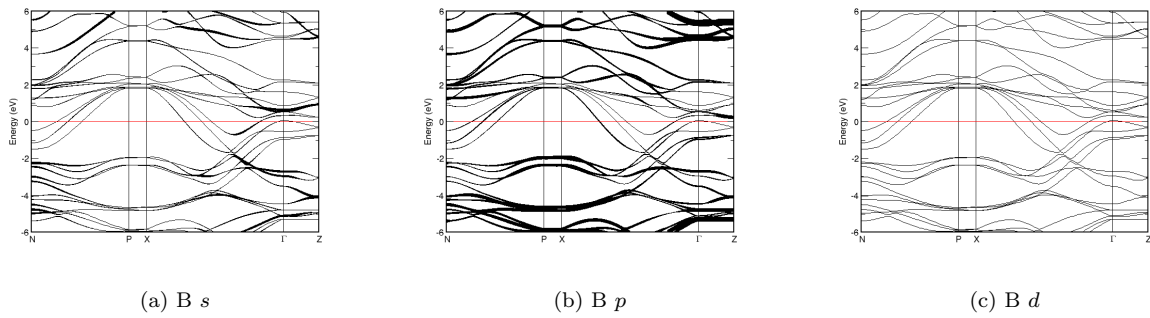

FIG. 221: Fat band representation of B in MoB

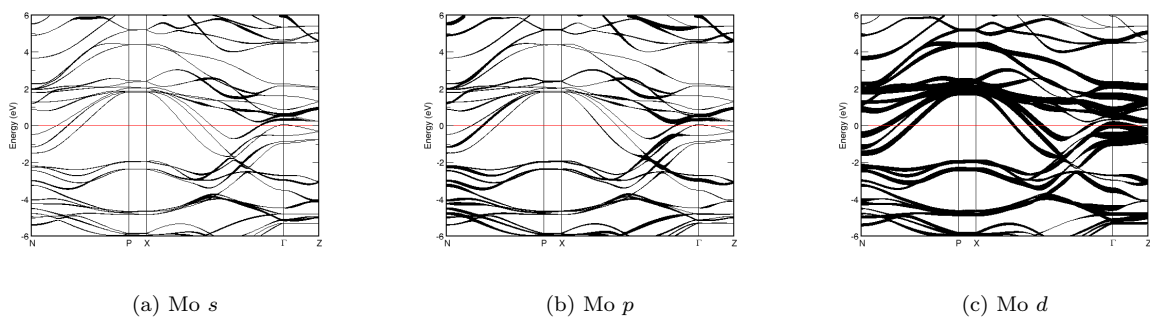

FIG. 222: Fat band representation of Mo in MoB

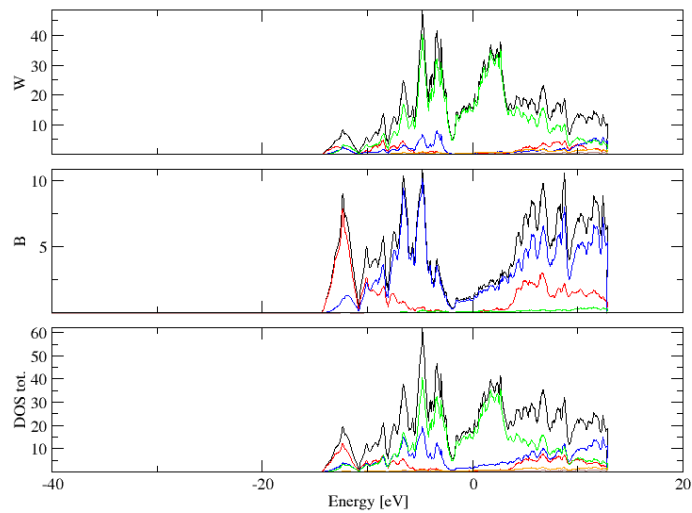

FIG. 223: (Color online) PDOS of WB (ICSD #24281). The *s*-, *p*- and *d*-projected states are in red, blue and green, respectively. WB crystallizes in space group  $I 41/a m d S$  (#141), in a tetragonal body-centred structure.

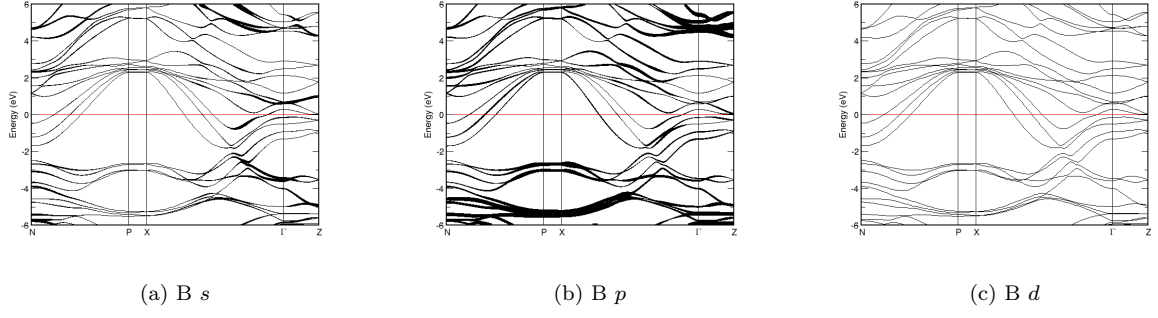

FIG. 224: Fat band representation of B in WB

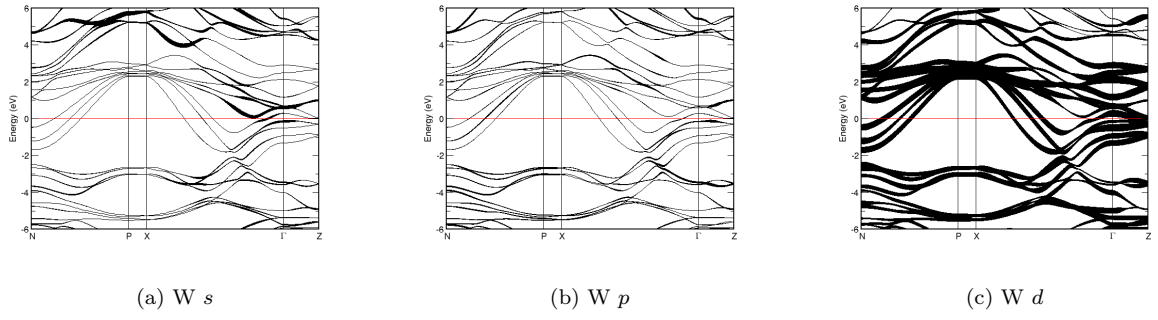

FIG. 225: Fat band representation of W in WB

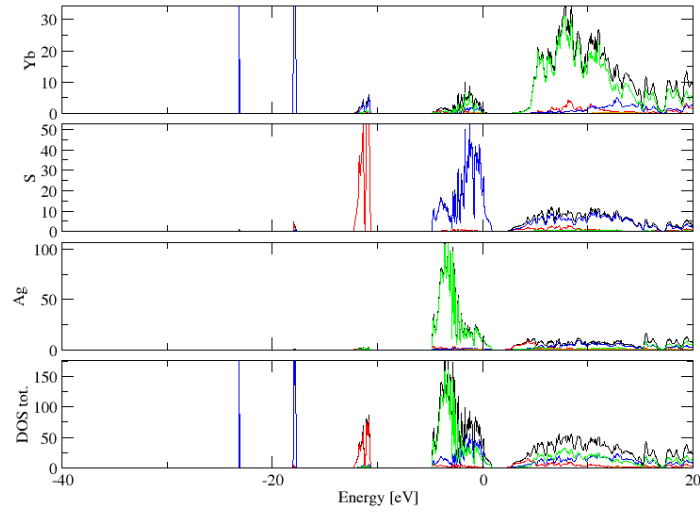

FIG. 226: (Color online) PDOS of  $\text{Yb}(\text{AgS}_2)$  (ICSD #27091). The  $s$ -,  $p$ - and  $d$ -projected states are in red, blue and green, respectively.  $\text{Yb}(\text{AgS}_2)$  crystallizes in space group  $I 41 m d$  (#109), in a tetragonal body-centred structure.

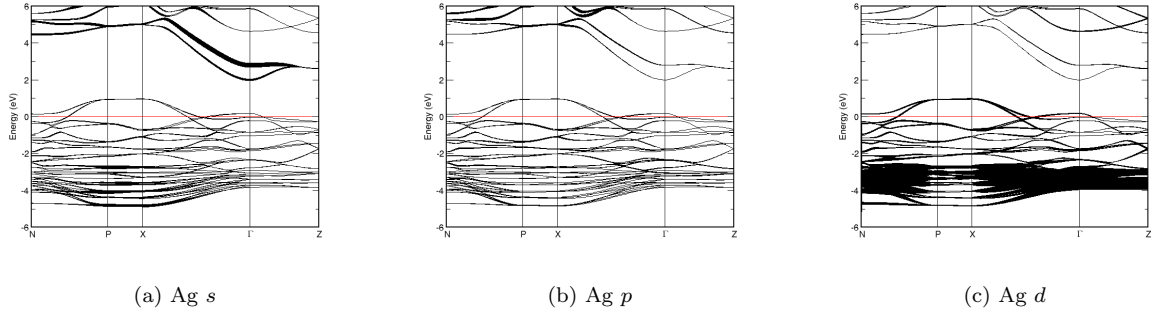

FIG. 227: Fat band representation of Ag in  $\text{Yb}(\text{AgS}_2)$

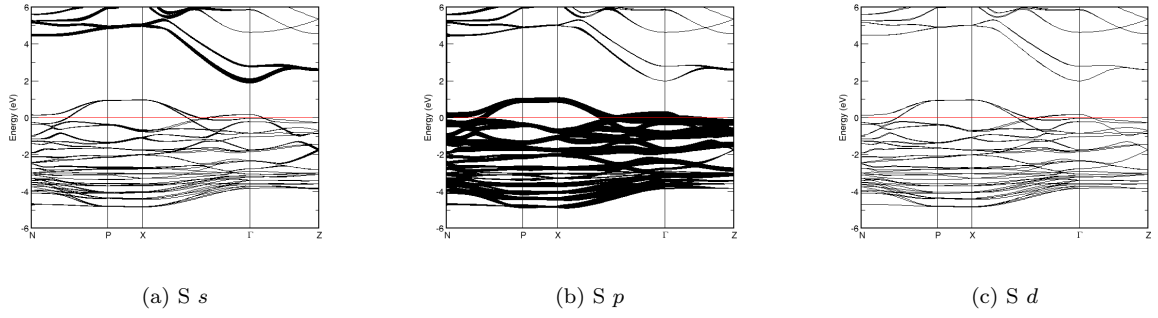

FIG. 228: Fat band representation of S in  $\text{Yb}(\text{AgS}_2)$

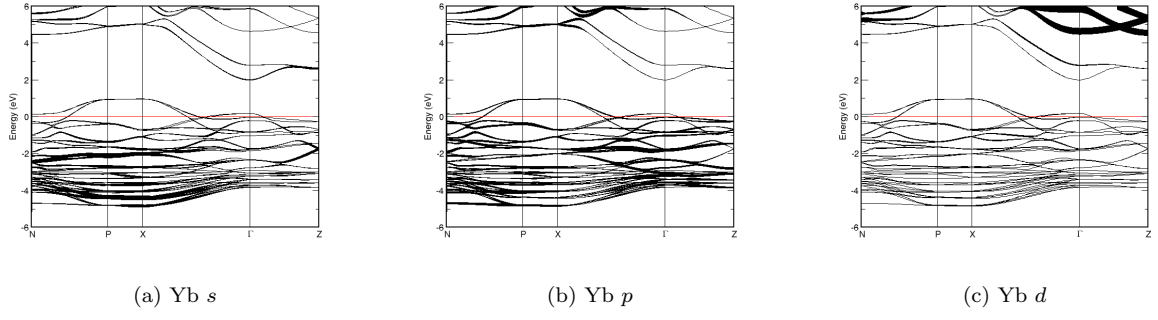

FIG. 229: Fat band representation of Yb in Yb(AgS<sub>2</sub>)

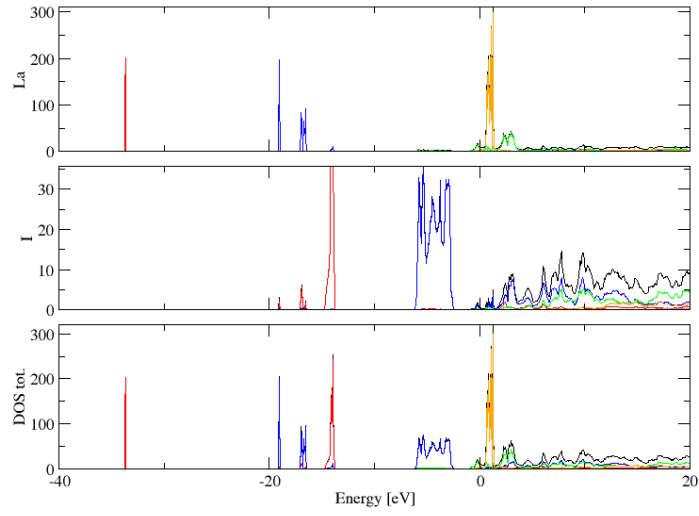

FIG. 230: (Color online) PDOS of LaI<sub>2</sub> (ICSD #202452). The *s*-, *p*- and *d*-projected states are in red, blue and green, respectively. LaI<sub>2</sub> crystallizes in space group I 4/m m m (#139), in a tetragonal body-centred structure.

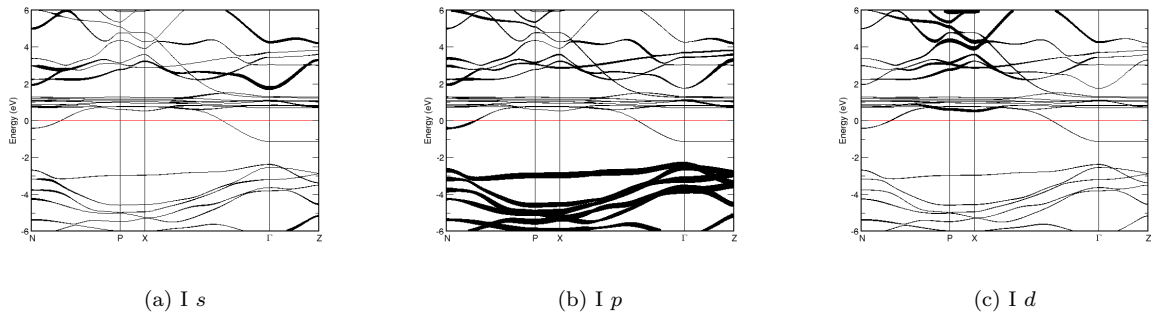

FIG. 231: Fat band representation of I in LaI<sub>2</sub>

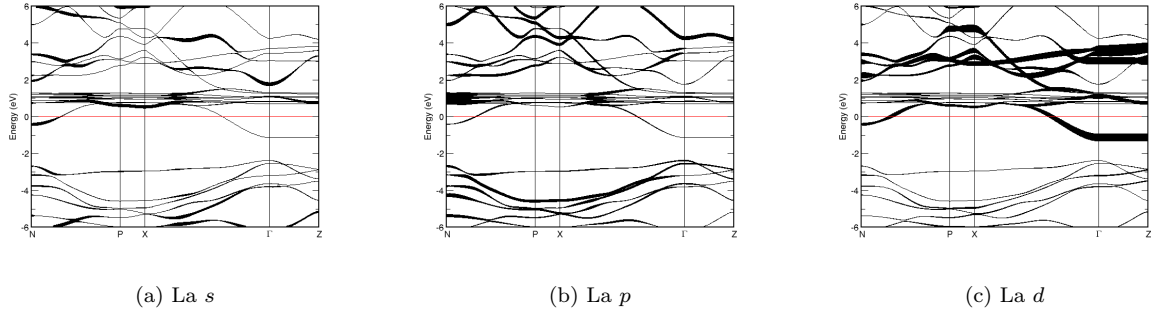FIG. 232: Fat band representation of La in  $\text{LaI}_2$ 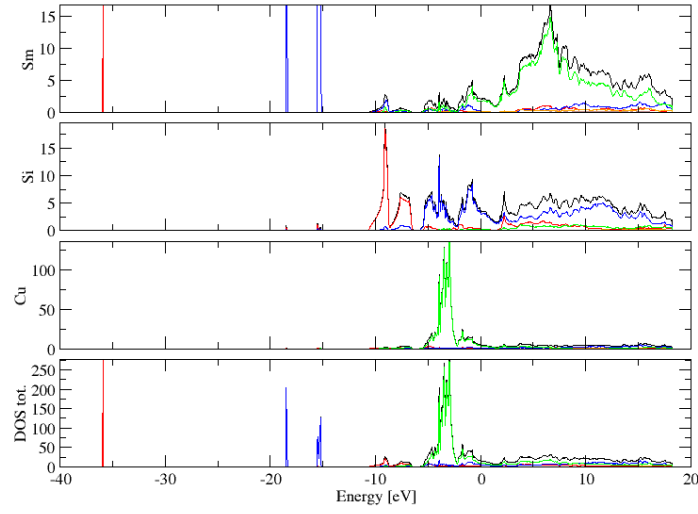FIG. 233: (Color online) PDOS of  $\text{SmCu}_2\text{Si}_2$  (ICSD #106843). The  $s$ -,  $p$ - and  $d$ -projected states are in red, blue and green, respectively.  $\text{SmCu}_2\text{Si}_2$  crystallizes in space group  $I 4/m m m$  (#139), in a tetragonal body-centred structure.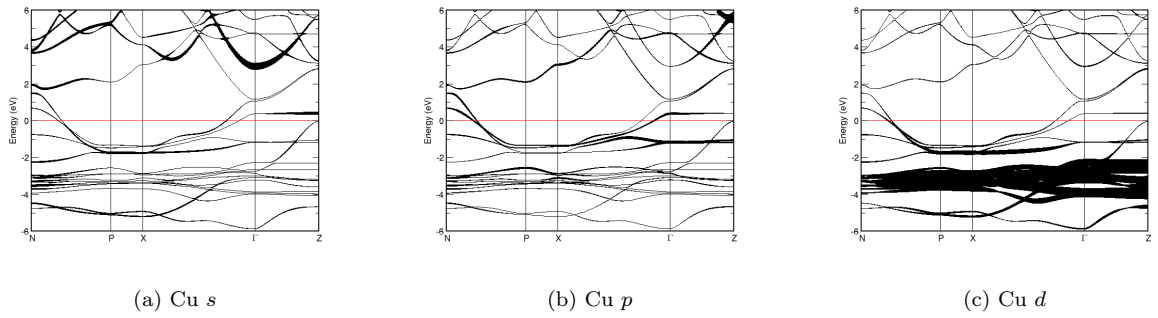FIG. 234: Fat band representation of Cu in  $\text{SmCu}_2\text{Si}_2$

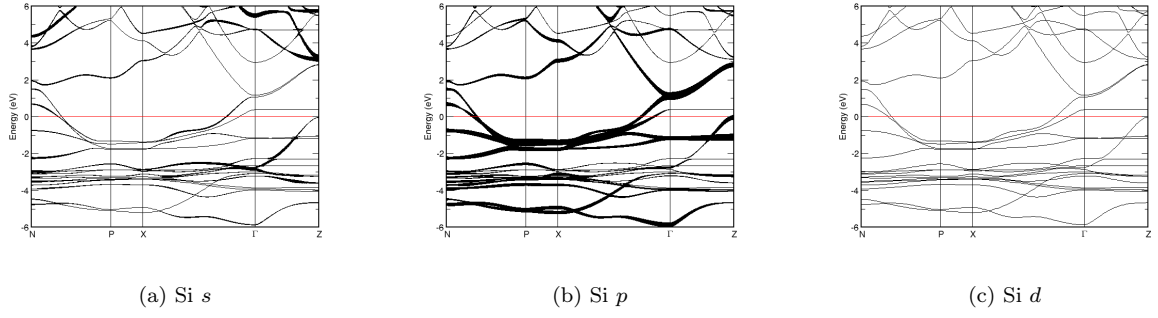FIG. 235: Fat band representation of Si in  $\text{SmCu}_2\text{Si}_2$ 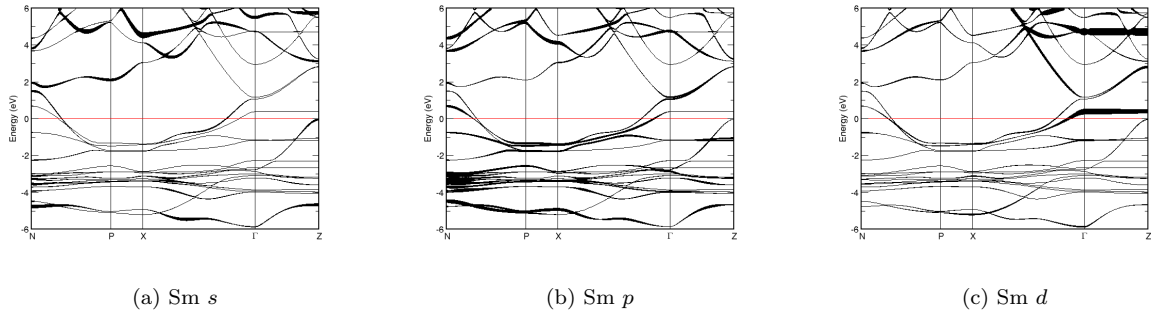FIG. 236: Fat band representation of Sm in  $\text{SmCu}_2\text{Si}_2$ 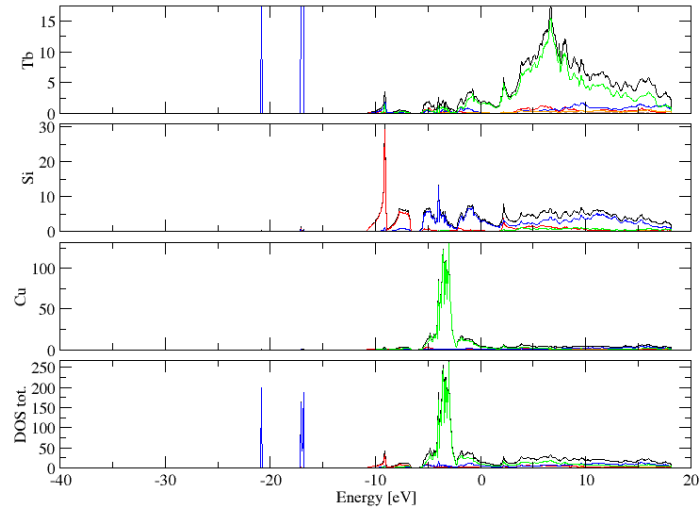FIG. 237: (Color online) PDOS of  $\text{TbCu}_2\text{Si}_2$  (ICSD #106844). The  $s$ -,  $p$ - and  $d$ -projected states are in red, blue and green, respectively.  $\text{TbCu}_2\text{Si}_2$  crystallizes in space group  $I 4/m m m$  (#139), in a tetragonal body-centred structure.

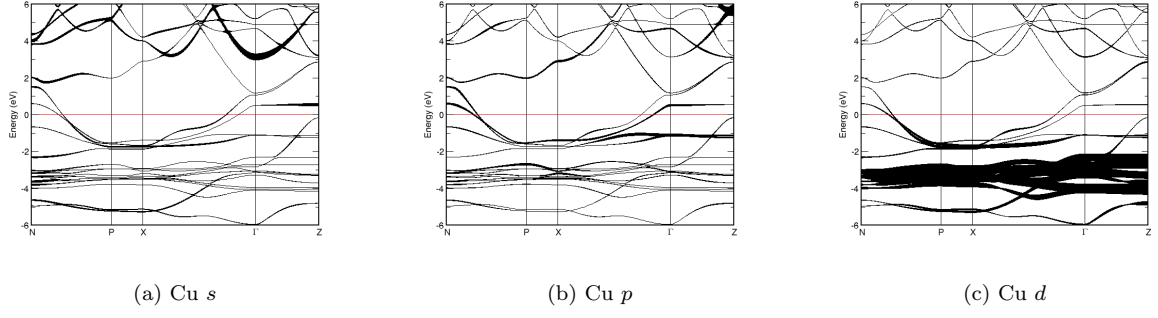FIG. 238: Fat band representation of Cu in TbCu<sub>2</sub>Si<sub>2</sub>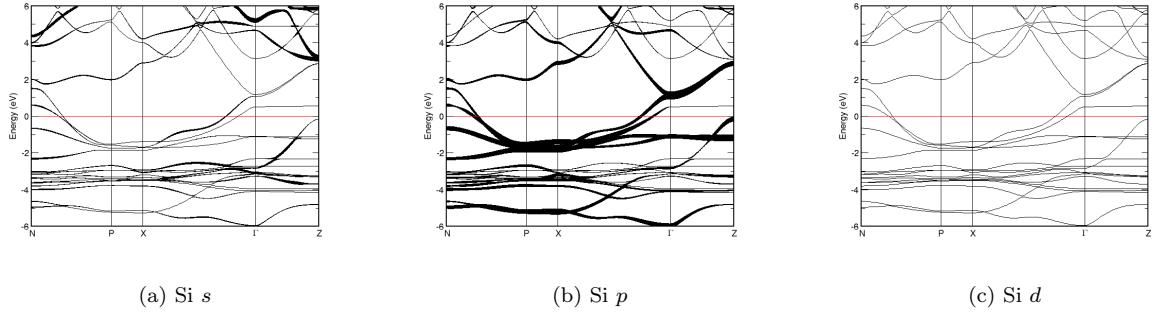FIG. 239: Fat band representation of Si in TbCu<sub>2</sub>Si<sub>2</sub>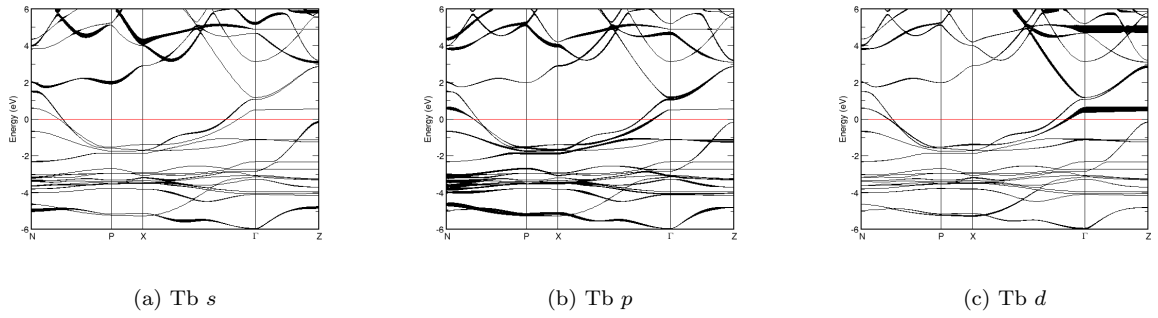FIG. 240: Fat band representation of Tb in TbCu<sub>2</sub>Si<sub>2</sub>



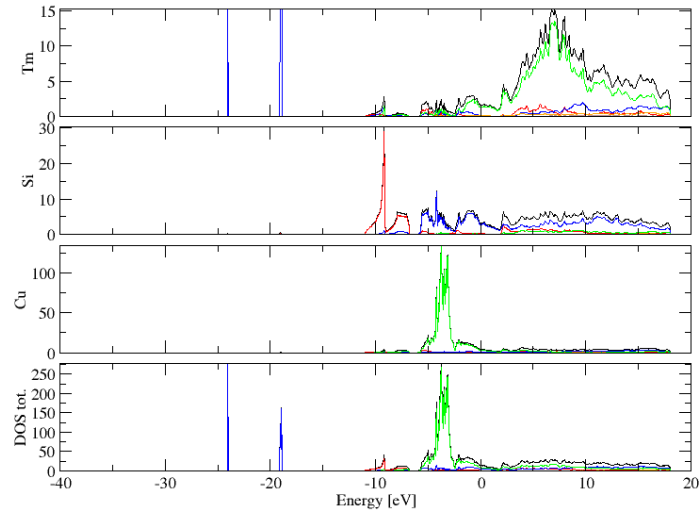

FIG. 241: (Color online) PDOS of  $\text{Cu}_2\text{TmSi}_2$  (ICSD #53349). The  $s$ -,  $p$ - and  $d$ -projected states are in red, blue and green, respectively.  $\text{Cu}_2\text{TmSi}_2$  crystallizes in space group  $I 4/m m m$  (#139), in a tetragonal body-centred structure.

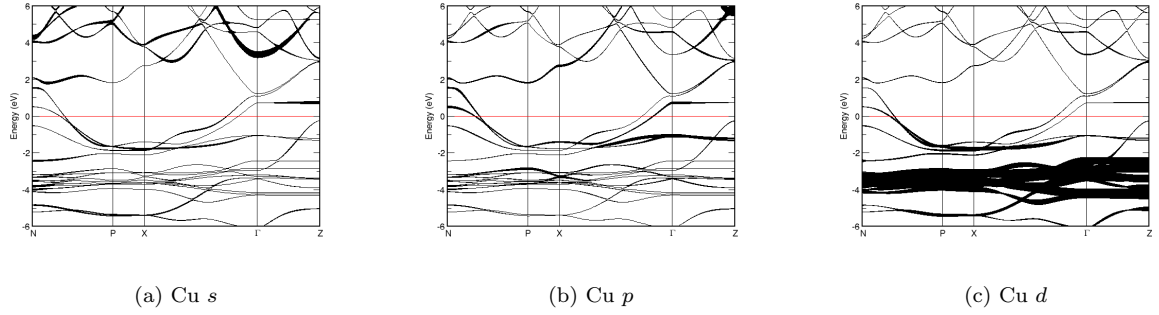

FIG. 242: Fat band representation of Cu in  $\text{Cu}_2\text{TmSi}_2$

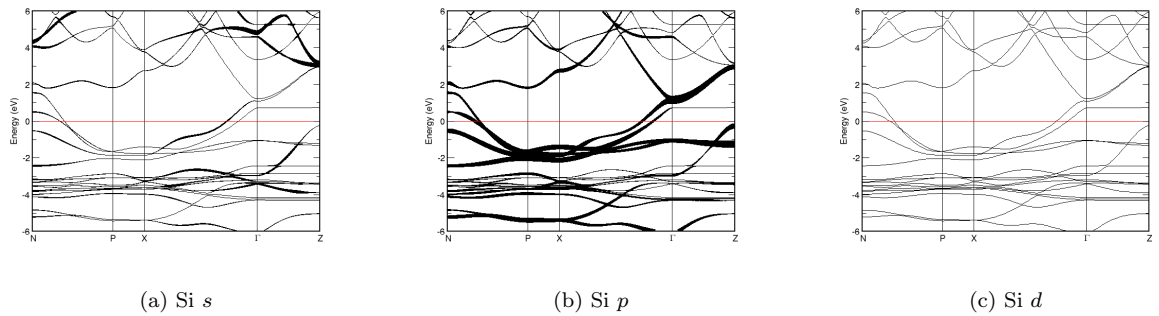

FIG. 243: Fat band representation of Si in  $\text{Cu}_2\text{TmSi}_2$

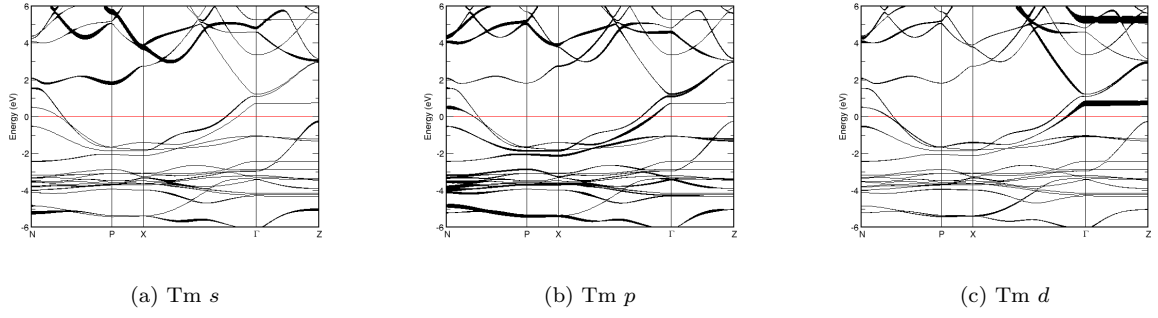FIG. 244: Fat band representation of Tm in  $\text{Cu}_2\text{TmSi}_2$ 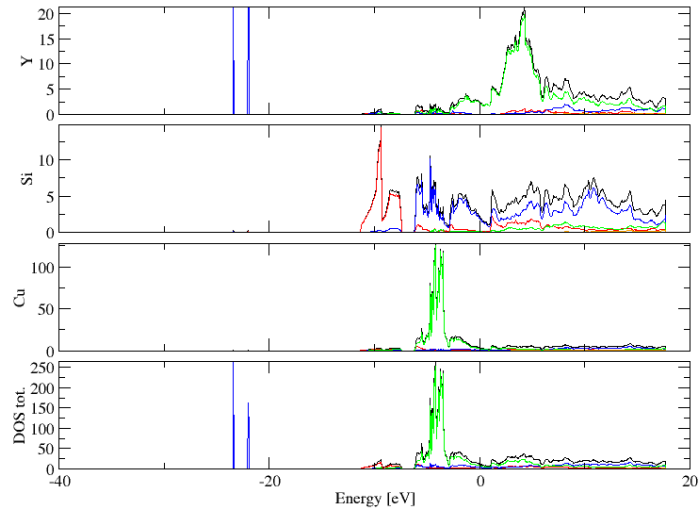FIG. 245: (Color online) PDOS of  $\text{Cu}_2\text{YSi}_2$  (ICSD #23551). The *s*-, *p*- and *d*-projected states are in red, blue and green, respectively.  $\text{Cu}_2\text{YSi}_2$  crystallizes in space group I 4/m m m (#139), in a tetragonal body-centred structure.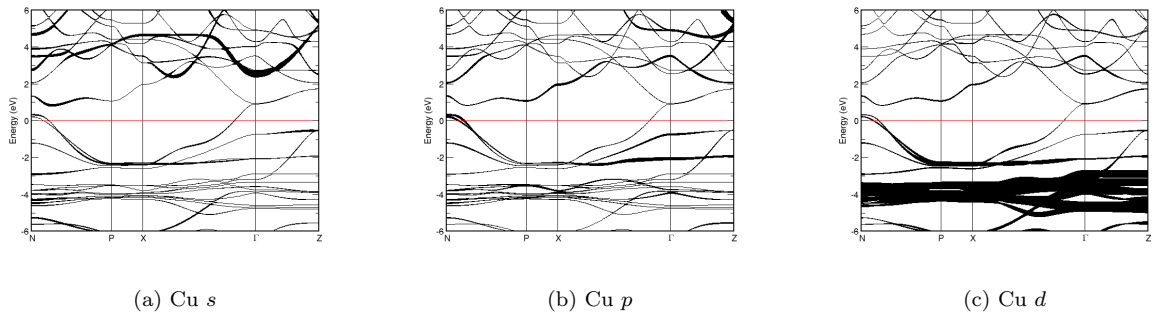FIG. 246: Fat band representation of Cu in  $\text{Cu}_2\text{YSi}_2$

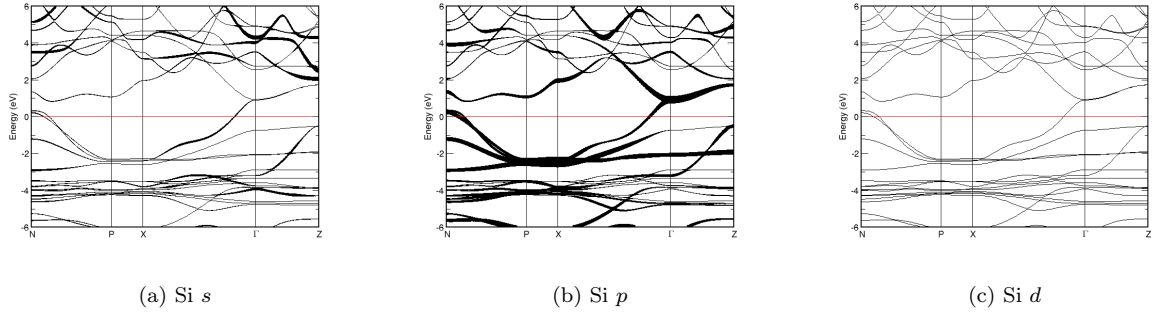FIG. 247: Fat band representation of Si in  $\text{Cu}_2\text{YSi}_2$ 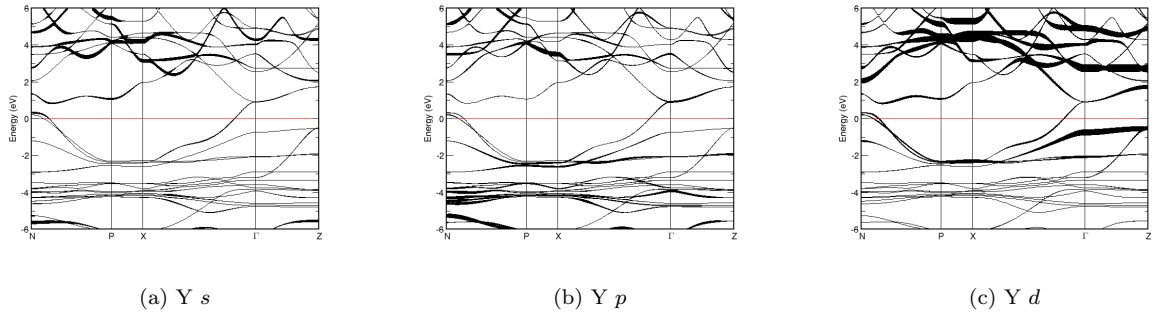FIG. 248: Fat band representation of Y in  $\text{Cu}_2\text{YSi}_2$ 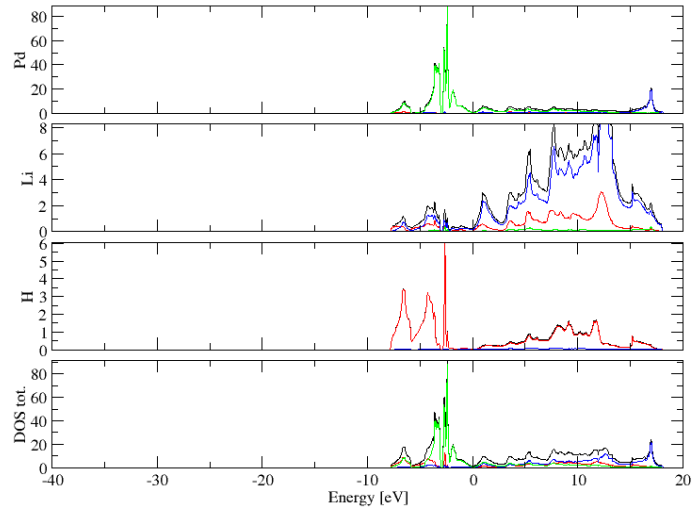FIG. 249: (Color online) PDOS of  $\text{Li}_2\text{PdH}_2$  (ICSD #108534). The *s*-, *p*- and *d*-projected states are in red, blue and green, respectively.  $\text{Li}_2\text{PdH}_2$  crystallizes in space group I  $4/m\ m\ m$  (#139), in a tetragonal body-centred structure.

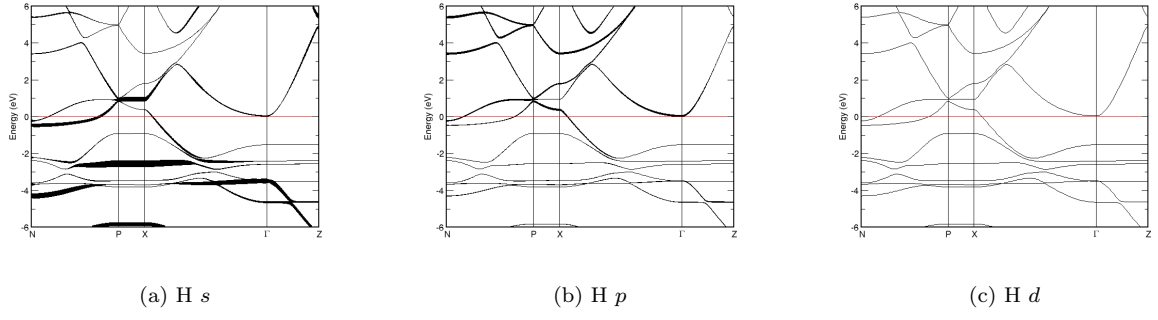FIG. 250: Fat band representation of H in  $\text{Li}_2\text{PdH}_2$ 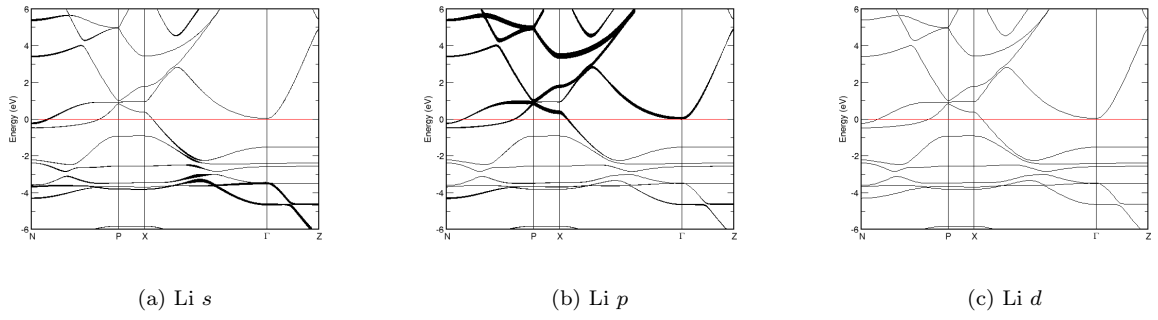FIG. 251: Fat band representation of Li in  $\text{Li}_2\text{PdH}_2$ 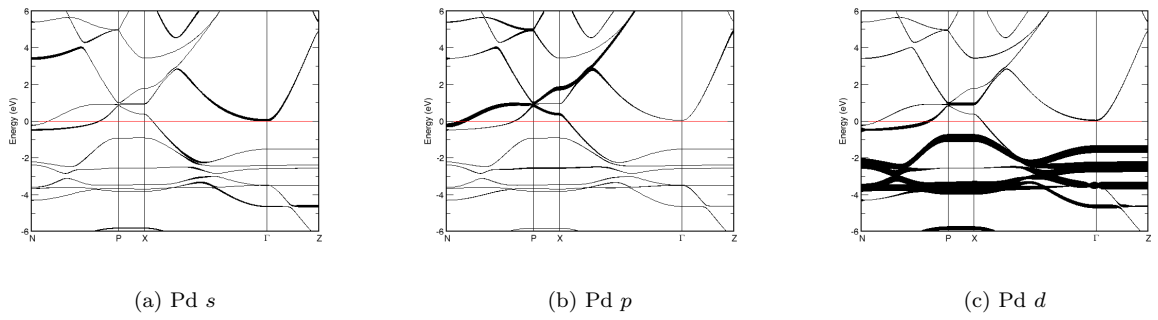FIG. 252: Fat band representation of Pd in  $\text{Li}_2\text{PdH}_2$

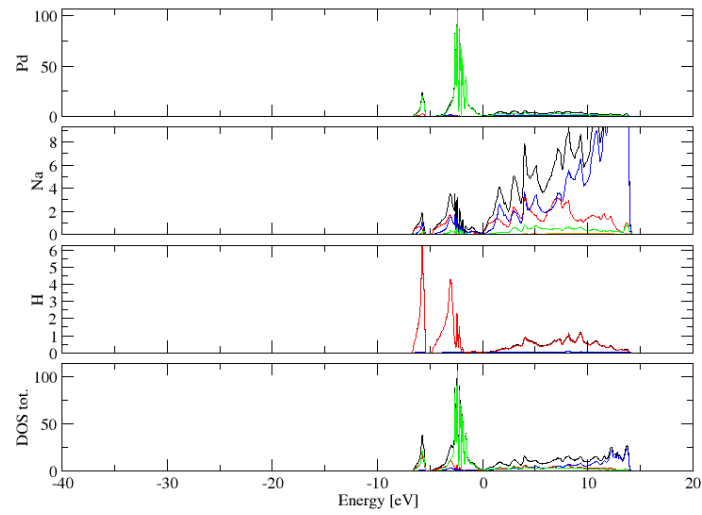

FIG. 253: (Color online) PDOS of  $\text{Na}_2\text{PdH}_2$  (ICSD #68071). The  $s$ -,  $p$ - and  $d$ -projected states are in red, blue and green, respectively.  $\text{Na}_2\text{PdH}_2$  crystallizes in space group  $I 4/m m m$  (#139), in a tetragonal body-centred structure.

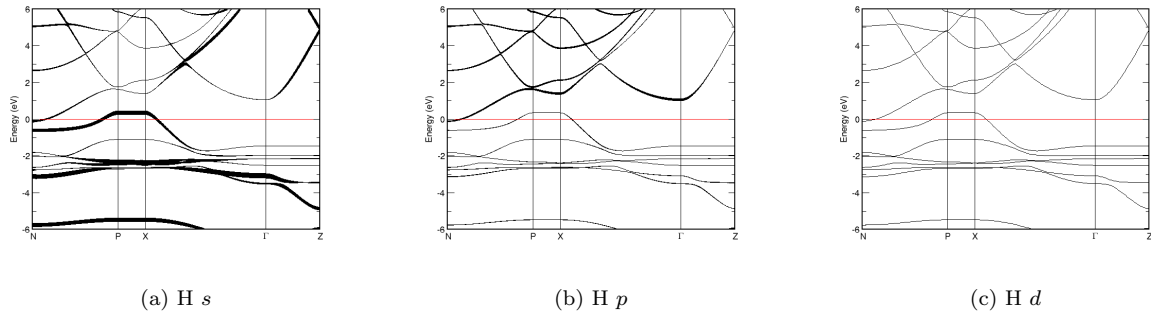

FIG. 254: Fat band representation of H in  $\text{Na}_2\text{PdH}_2$

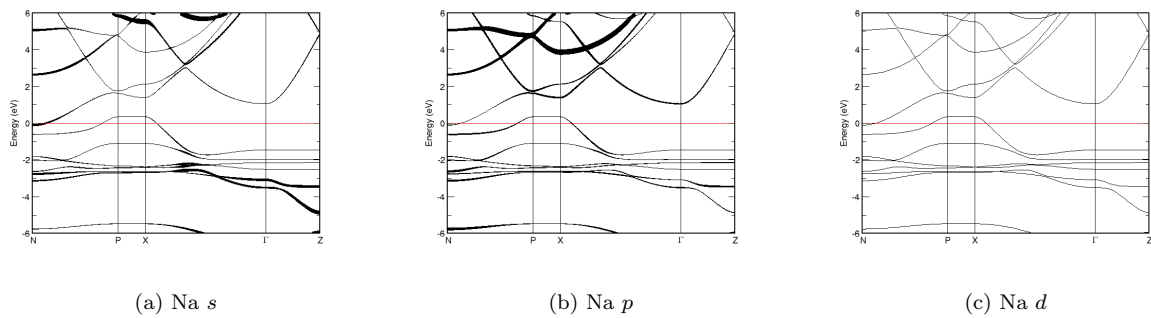

FIG. 255: Fat band representation of Na in  $\text{Na}_2\text{PdH}_2$

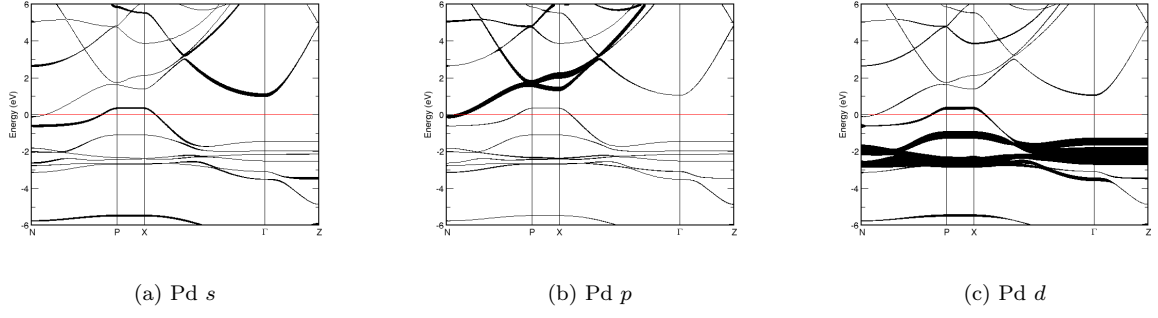FIG. 256: Fat band representation of Pd in  $\text{Na}_2\text{PdH}_2$ 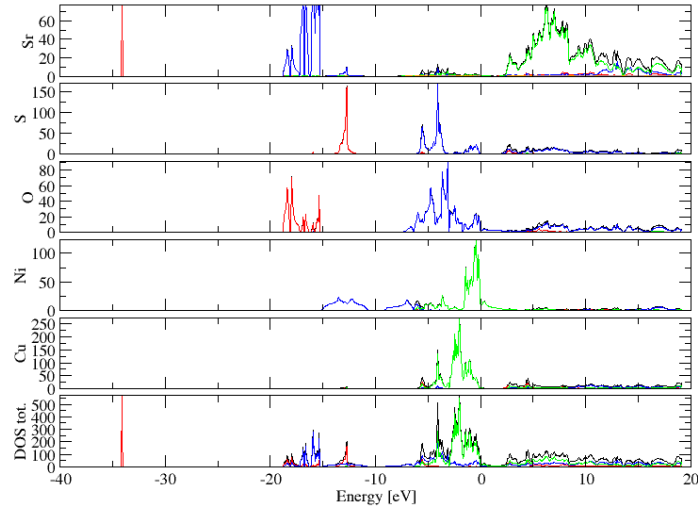FIG. 257: (Color online) PDOS of  $(\text{Cu}_2\text{S}_2)(\text{Sr}_2\text{NiO}_2)$  (ICSD #88424). The *s*-, *p*- and *d*-projected states are in red, blue and green, respectively.  $(\text{Cu}_2\text{S}_2)(\text{Sr}_2\text{NiO}_2)$  crystallizes in space group  $I 4/m m m$  (#139), in a tetragonal body-centred structure.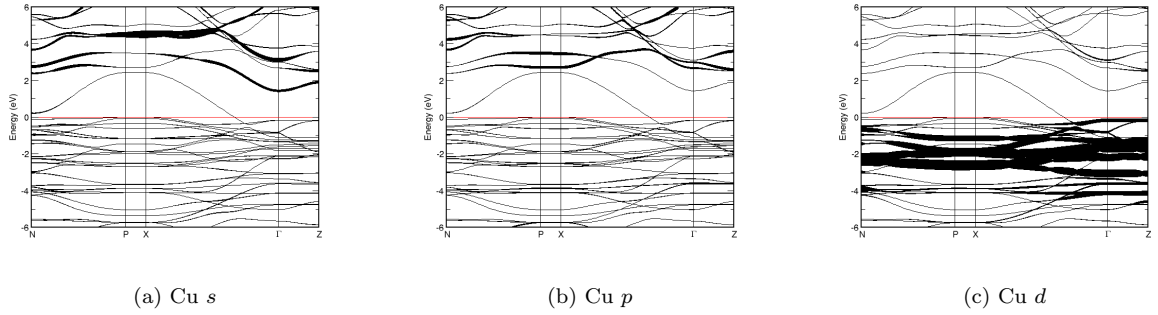FIG. 258: Fat band representation of Cu in  $(\text{Cu}_2\text{S}_2)(\text{Sr}_2\text{NiO}_2)$

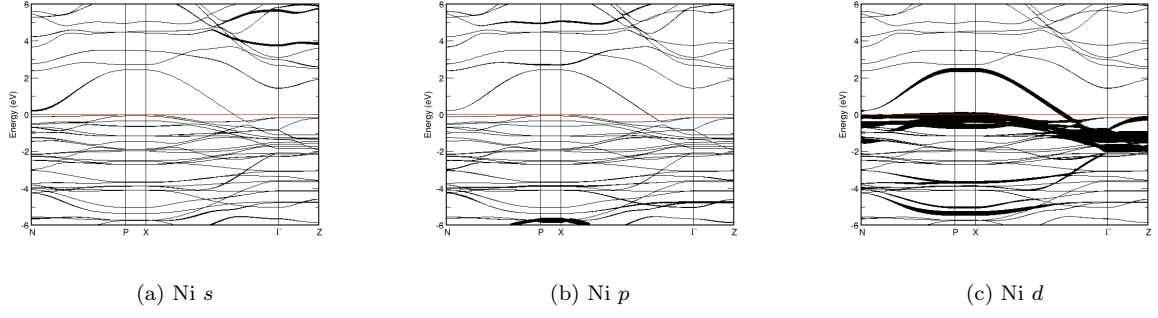FIG. 259: Fat band representation of Ni in  $(\text{Cu}_2\text{S}_2)(\text{Sr}_2\text{NiO}_2)$ 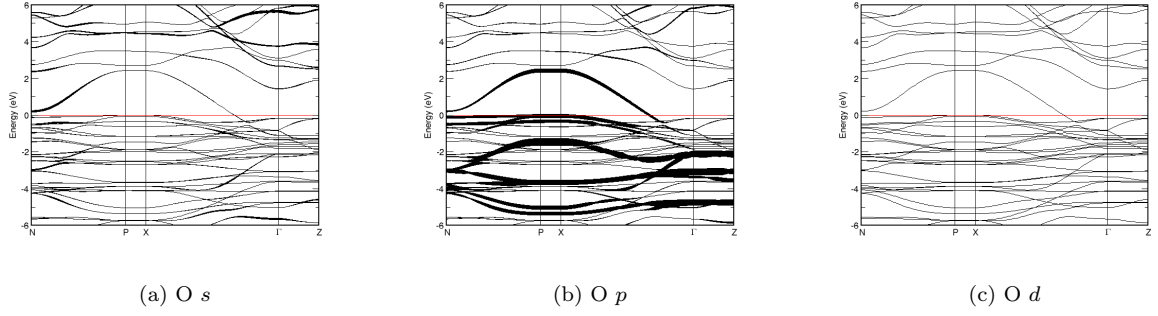FIG. 260: Fat band representation of O in  $(\text{Cu}_2\text{S}_2)(\text{Sr}_2\text{NiO}_2)$ 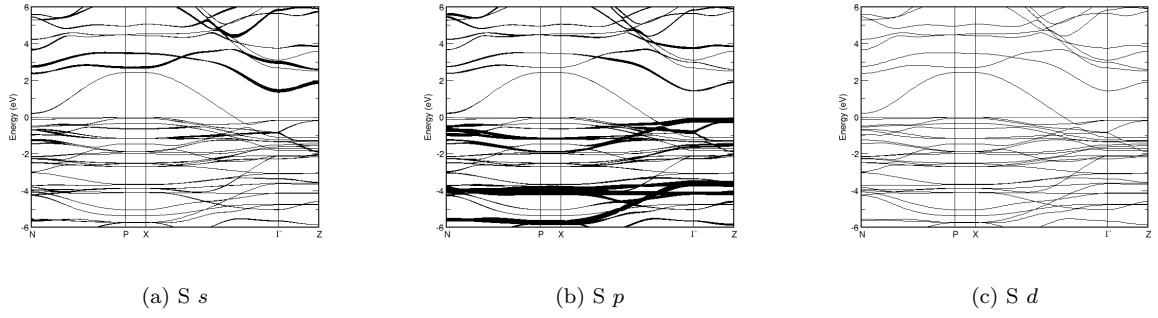FIG. 261: Fat band representation of S in  $(\text{Cu}_2\text{S}_2)(\text{Sr}_2\text{NiO}_2)$ 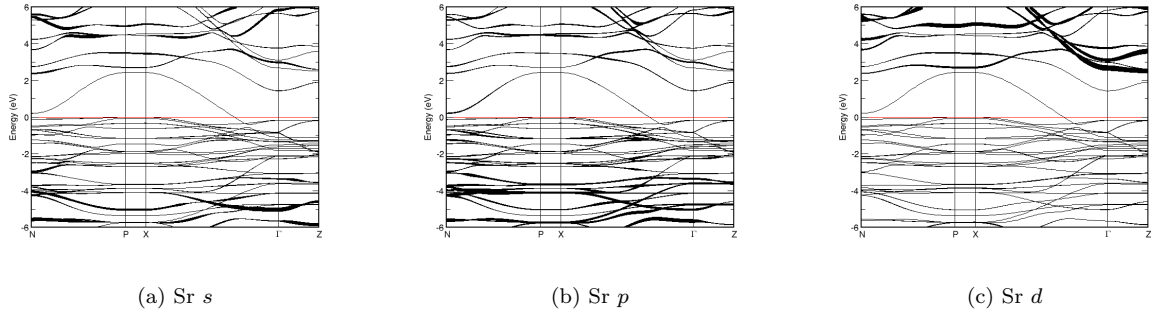FIG. 262: Fat band representation of Sr in  $(\text{Cu}_2\text{S}_2)(\text{Sr}_2\text{NiO}_2)$

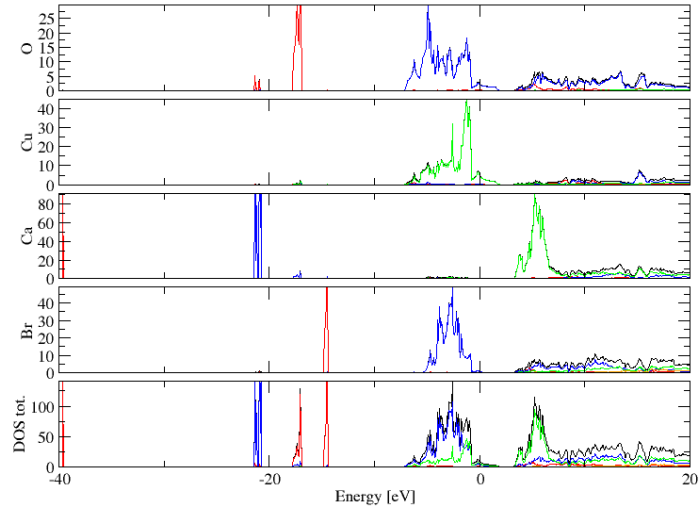

FIG. 263: (Color online) PDOS of  $\text{Ca}_2(\text{CuBr}_2\text{O}_2)$  (ICSD #1028). The  $s$ -,  $p$ - and  $d$ -projected states are in red, blue and green, respectively.  $\text{Ca}_2(\text{CuBr}_2\text{O}_2)$  crystallizes in space group  $I 4/m m m$  (#139), in a tetragonal body-centred structure.

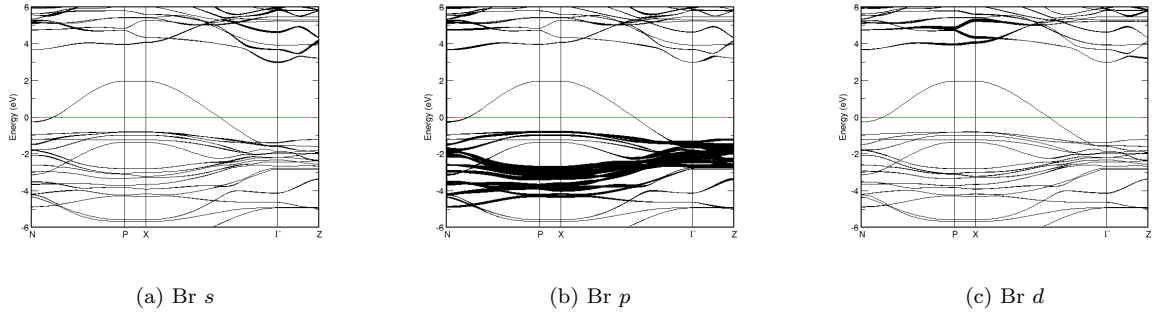

FIG. 264: Fat band representation of Br in  $\text{Ca}_2(\text{CuBr}_2\text{O}_2)$

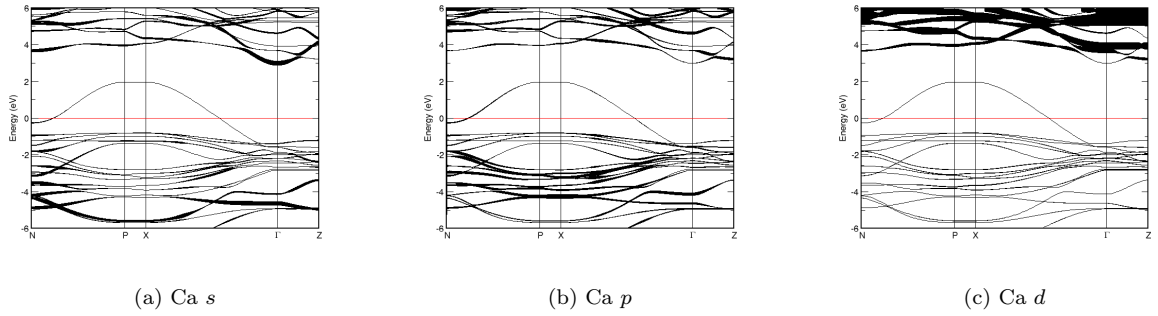

FIG. 265: Fat band representation of Ca in  $\text{Ca}_2(\text{CuBr}_2\text{O}_2)$



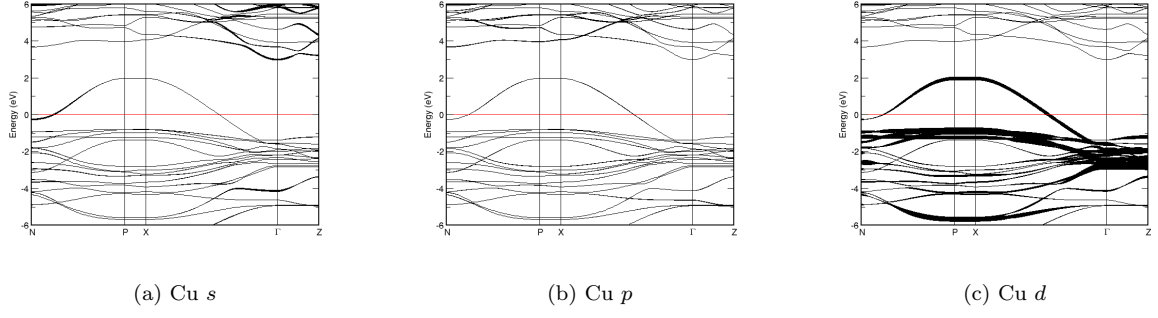

FIG. 266: Fat band representation of Cu in  $\text{Ca}_2(\text{CuBr}_2\text{O}_2)$

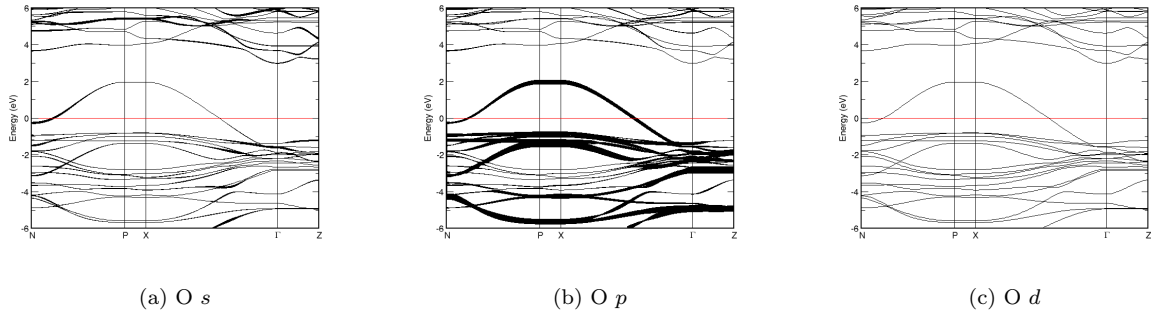

FIG. 267: Fat band representation of O in  $\text{Ca}_2(\text{CuBr}_2\text{O}_2)$

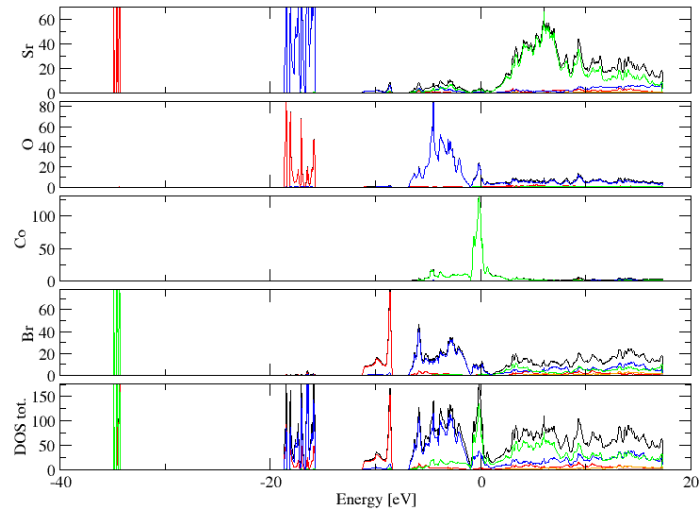

FIG. 268: (Color online) PDOS of  $\text{Sr}_2\text{CoO}_2\text{Br}_2$  (ICSD #151789). The *s*-, *p*- and *d*-projected states are in red, blue and green, respectively.  $\text{Sr}_2\text{CoO}_2\text{Br}_2$  crystallizes in space group  $I 4/m m m$  (#139), in a tetragonal body-centred structure.

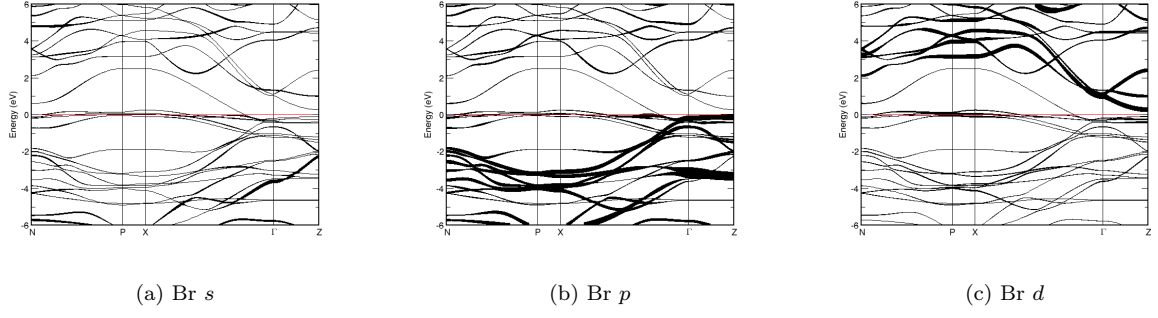FIG. 269: Fat band representation of Br in  $\text{Sr}_2\text{CoO}_2\text{Br}_2$ 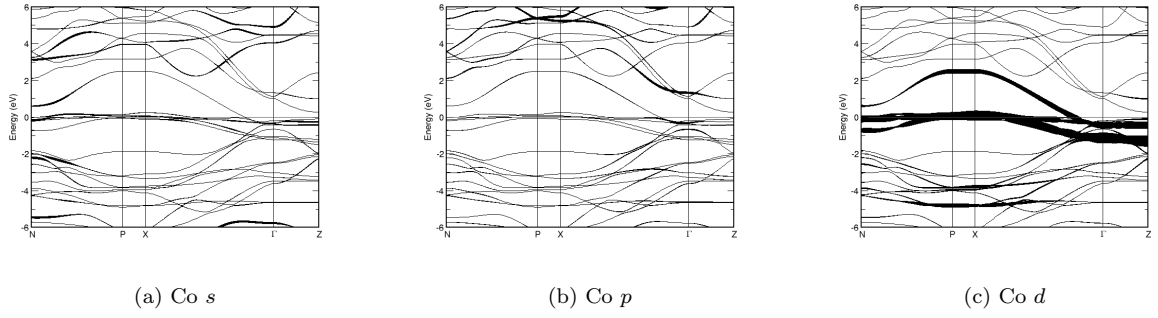FIG. 270: Fat band representation of Co in  $\text{Sr}_2\text{CoO}_2\text{Br}_2$ 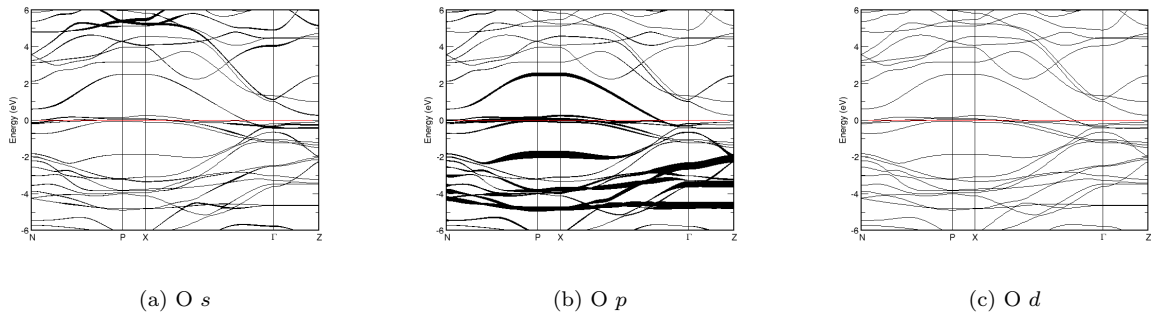FIG. 271: Fat band representation of O in  $\text{Sr}_2\text{CoO}_2\text{Br}_2$ 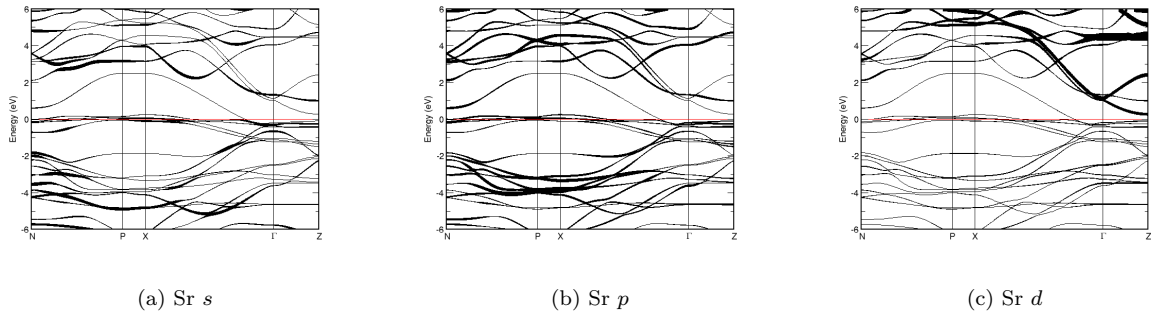FIG. 272: Fat band representation of Sr in  $\text{Sr}_2\text{CoO}_2\text{Br}_2$

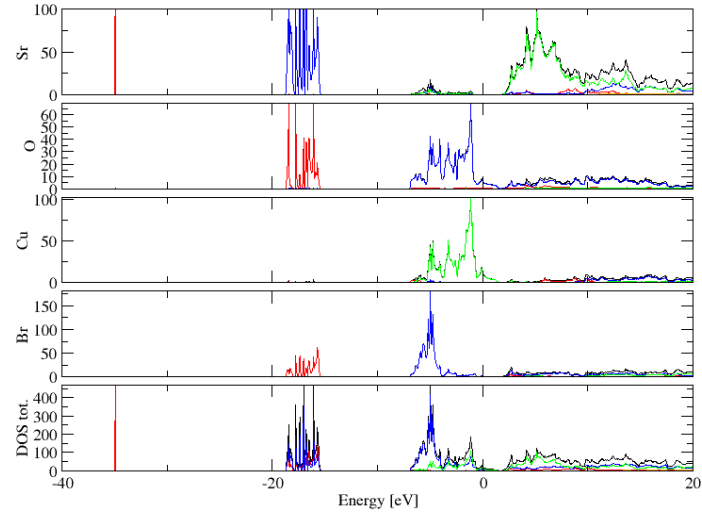

FIG. 273: (Color online) PDOS of  $\text{CuSr}_2\text{Br}_2\text{O}_2$  (ICSD #1178). The  $s$ -,  $p$ - and  $d$ -projected states are in red, blue and green, respectively.  $\text{CuSr}_2\text{Br}_2\text{O}_2$  crystallizes in space group  $I 4/m m m$  (#139), in a tetragonal body-centred structure.

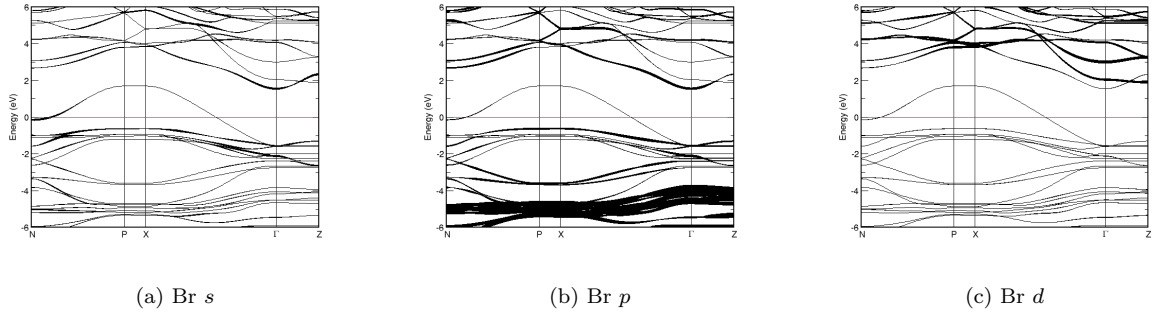

FIG. 274: Fat band representation of Br in  $\text{CuSr}_2\text{Br}_2\text{O}_2$

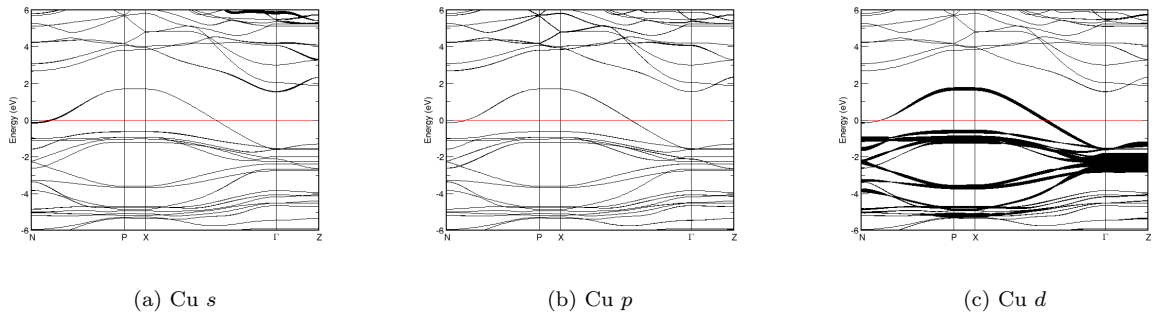

FIG. 275: Fat band representation of Cu in  $\text{CuSr}_2\text{Br}_2\text{O}_2$

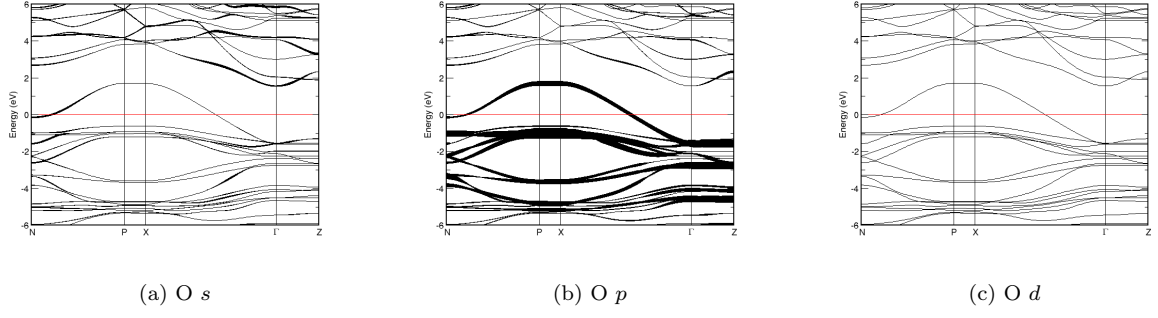FIG. 276: Fat band representation of O in  $\text{CuSr}_2\text{Br}_2\text{O}_2$ 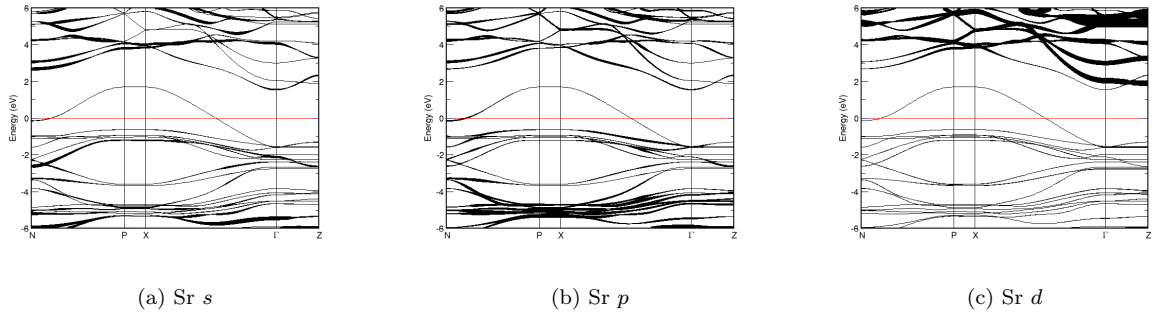FIG. 277: Fat band representation of Sr in  $\text{CuSr}_2\text{Br}_2\text{O}_2$ 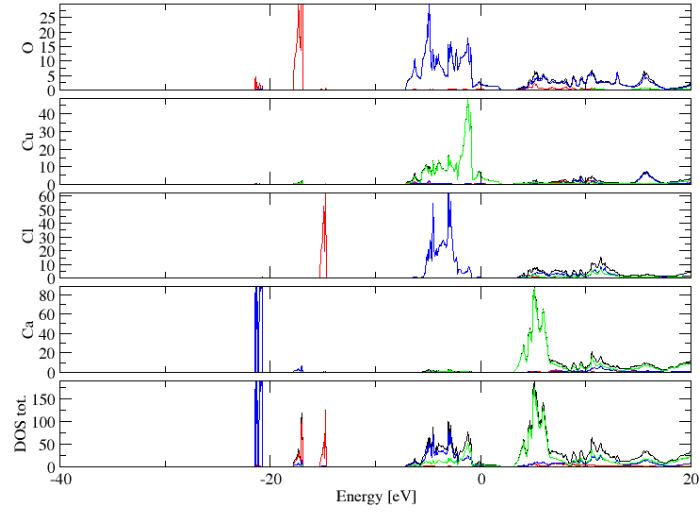

FIG. 278: (Color online) PDOS of  $\text{Ca}_2(\text{CuCl}_2\text{O}_2)$  (ICSD #1027). The *s*-, *p*- and *d*-projected states are in red, blue and green, respectively.  $\text{Ca}_2(\text{CuCl}_2\text{O}_2)$  crystallizes in space group  $I 4/m m m$  (#139), in a tetragonal body-centred structure.

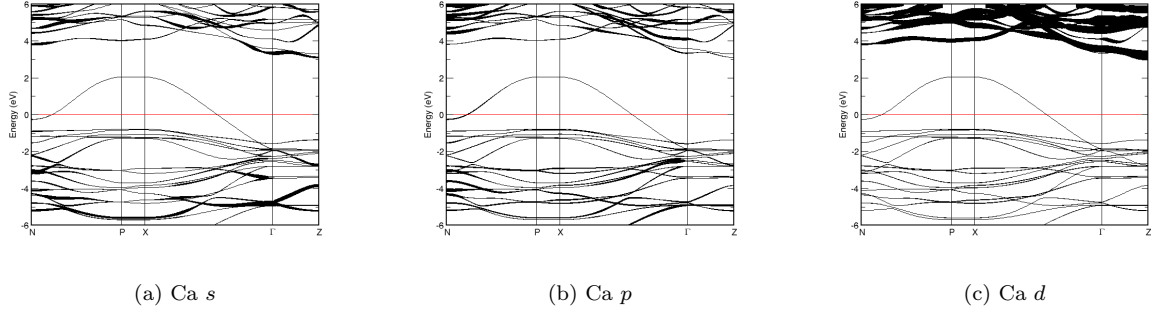FIG. 279: Fat band representation of Ca in  $\text{Ca}_2(\text{CuCl}_2\text{O}_2)$ 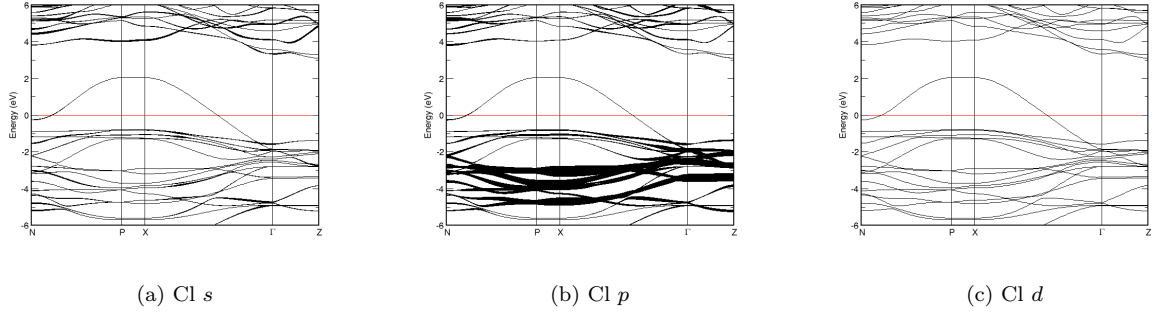FIG. 280: Fat band representation of Cl in  $\text{Ca}_2(\text{CuCl}_2\text{O}_2)$ 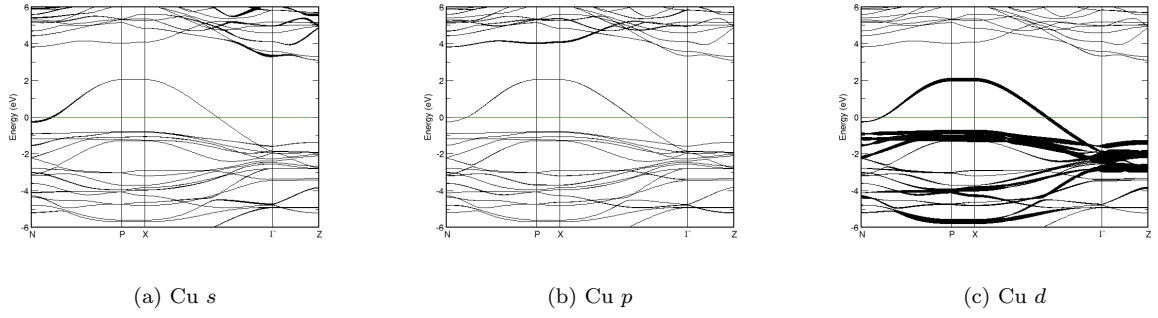FIG. 281: Fat band representation of Cu in  $\text{Ca}_2(\text{CuCl}_2\text{O}_2)$ 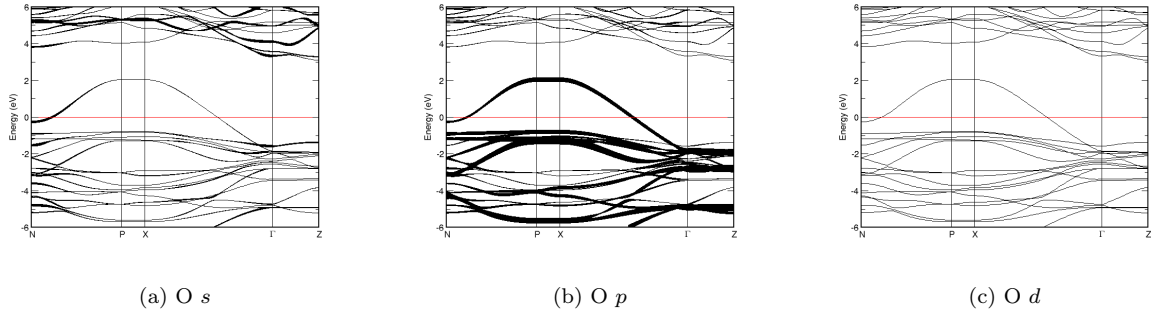FIG. 282: Fat band representation of O in  $\text{Ca}_2(\text{CuCl}_2\text{O}_2)$

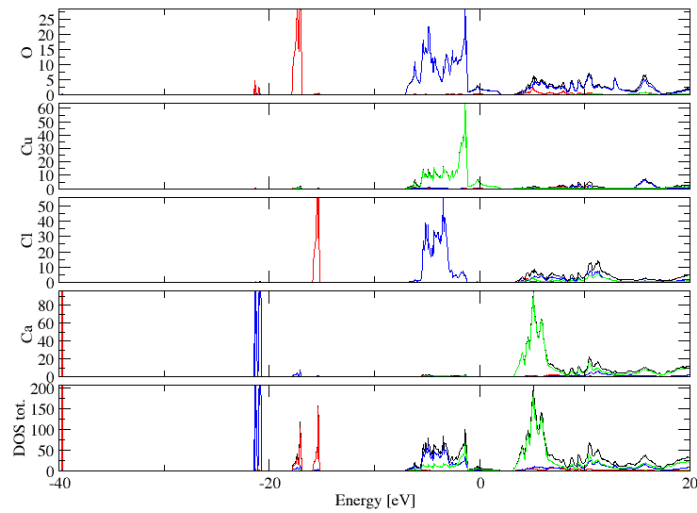

FIG. 283: (Color online) PDOS of  $\text{Ca}_2\text{CuO}_2\text{Cl}_2$  (ICSD #83117). The  $s$ -,  $p$ - and  $d$ -projected states are in red, blue and green, respectively.  $\text{Ca}_2\text{CuO}_2\text{Cl}_2$  crystallizes in space group  $I 4/m m m$  (#139), in a tetragonal body-centred structure.

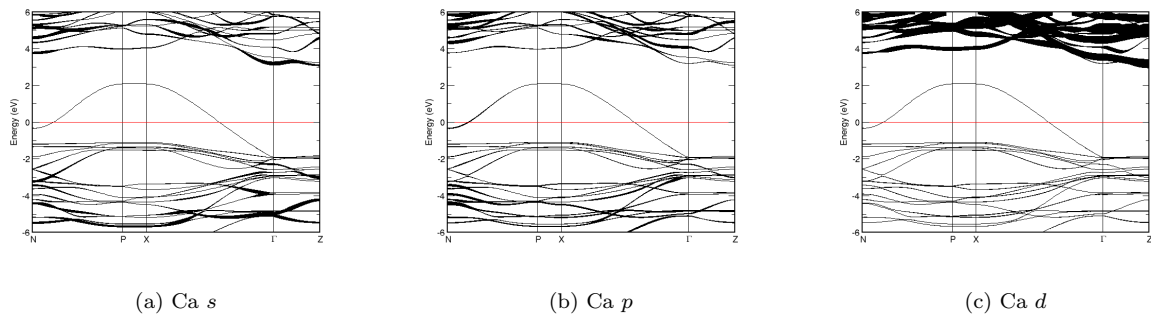

FIG. 284: Fat band representation of Ca in  $\text{Ca}_2\text{CuO}_2\text{Cl}_2$

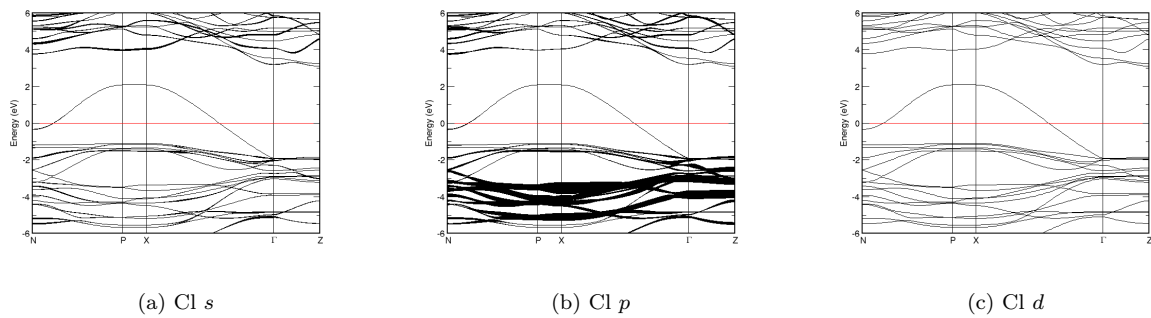

FIG. 285: Fat band representation of Cl in  $\text{Ca}_2\text{CuO}_2\text{Cl}_2$

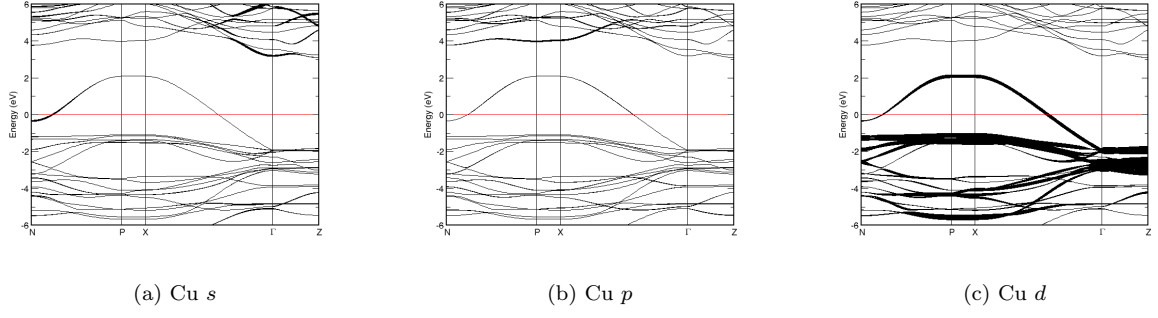FIG. 286: Fat band representation of Cu in  $\text{Ca}_2\text{CuO}_2\text{Cl}_2$ 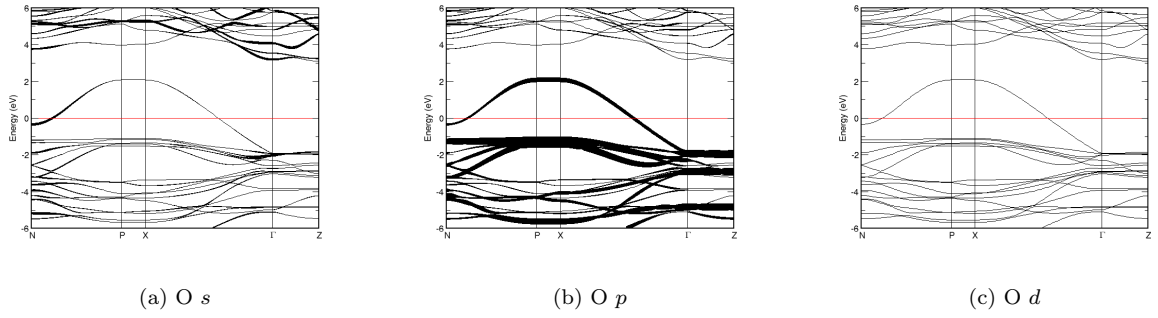FIG. 287: Fat band representation of O in  $\text{Ca}_2\text{CuO}_2\text{Cl}_2$ 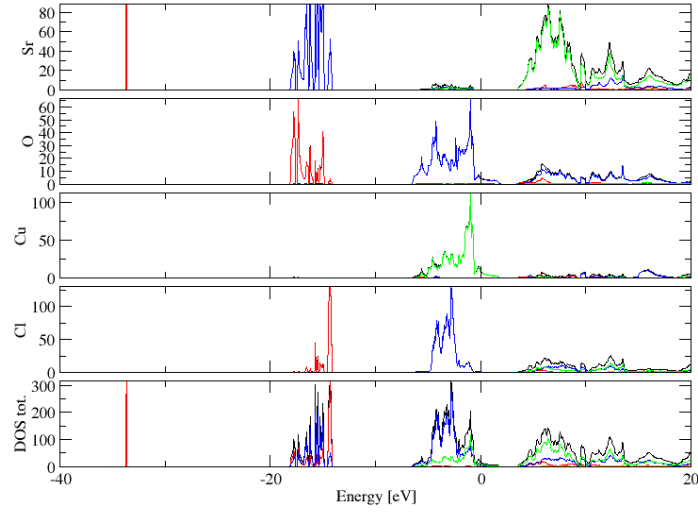

FIG. 288: (Color online) PDOS of  $\text{Sr}_2\text{CuO}_2\text{Cl}_2$  (ICSD #4087). The *s*-, *p*- and *d*-projected states are in red, blue and green, respectively.  $\text{Sr}_2\text{CuO}_2\text{Cl}_2$  crystallizes in space group  $I 4/m m m$  (#139), in a tetragonal body-centred structure.

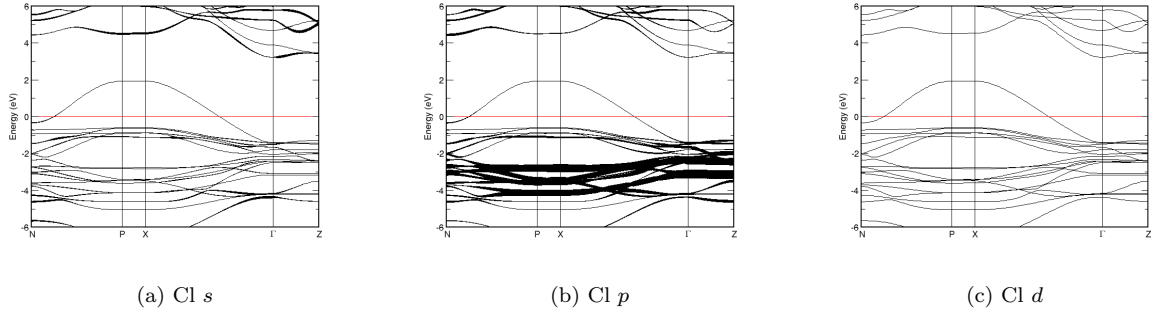FIG. 289: Fat band representation of Cl in  $\text{Sr}_2\text{CuO}_2\text{Cl}_2$ 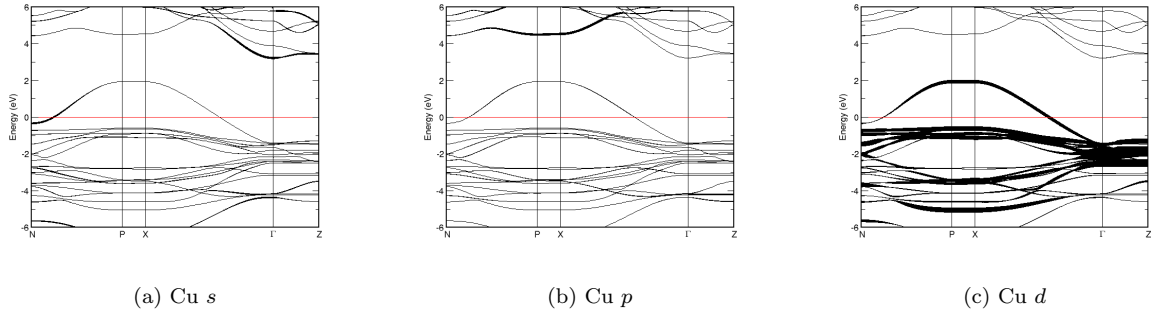FIG. 290: Fat band representation of Cu in  $\text{Sr}_2\text{CuO}_2\text{Cl}_2$ 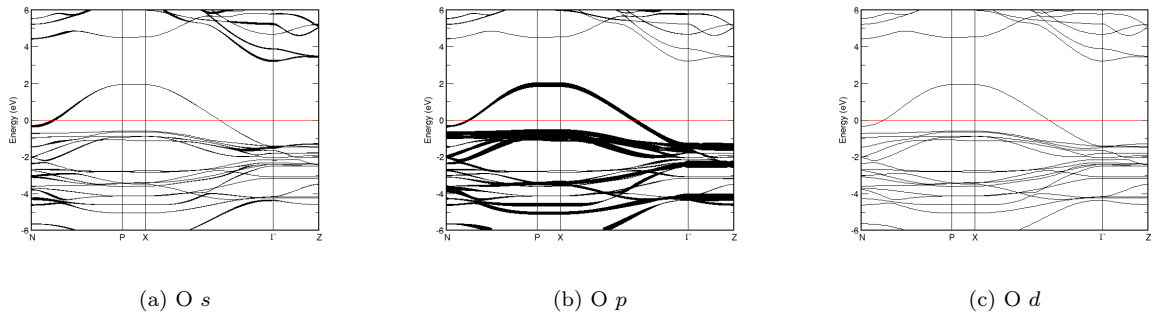FIG. 291: Fat band representation of O in  $\text{Sr}_2\text{CuO}_2\text{Cl}_2$ 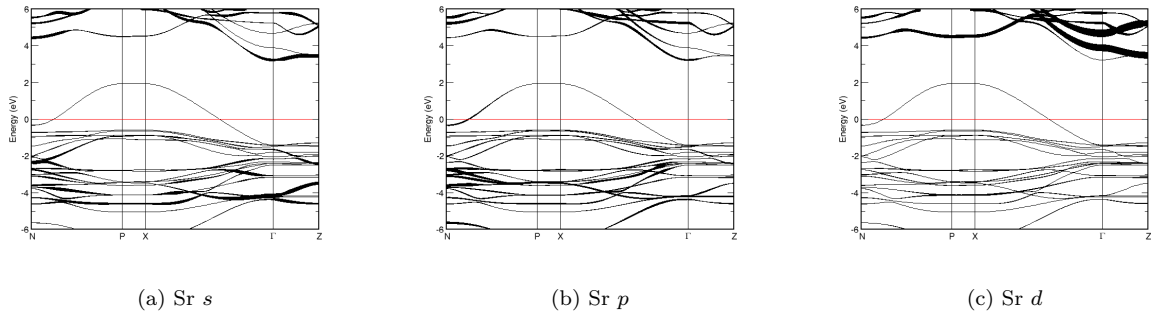FIG. 292: Fat band representation of Sr in  $\text{Sr}_2\text{CuO}_2\text{Cl}_2$



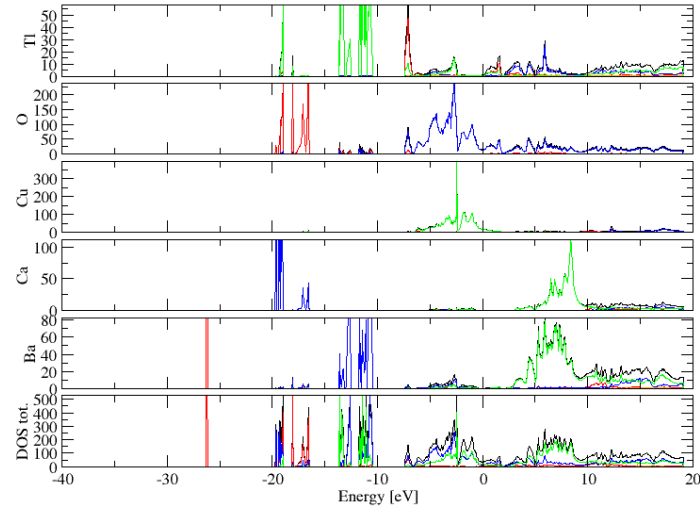

FIG. 293: (Color online) PDOS of  $\text{Tl}_2\text{Ba}_2\text{CaCu}_2\text{O}_8$  (ICSD #78592). The  $s$ -,  $p$ - and  $d$ -projected states are in red, blue and green, respectively.  $\text{Tl}_2\text{Ba}_2\text{CaCu}_2\text{O}_8$  crystallizes in space group  $I 4/m m m$  (#139), in a tetragonal body-centred structure.

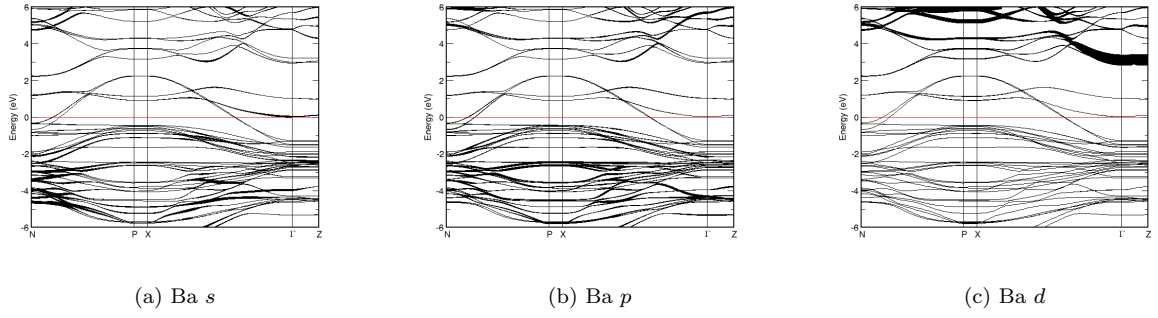

FIG. 294: Fat band representation of Ba in  $\text{Tl}_2\text{Ba}_2\text{CaCu}_2\text{O}_8$

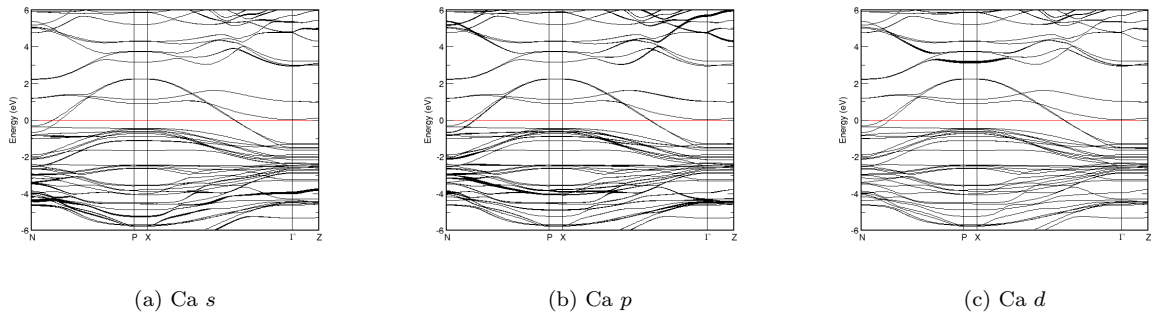

FIG. 295: Fat band representation of Ca in  $\text{Tl}_2\text{Ba}_2\text{CaCu}_2\text{O}_8$

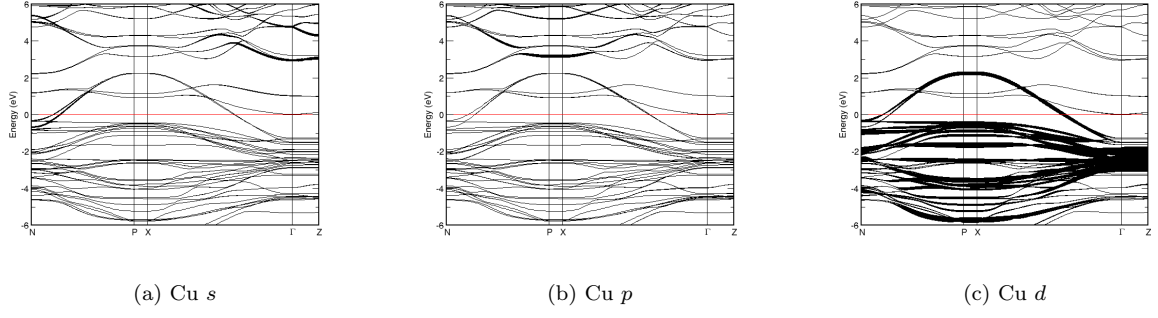FIG. 296: Fat band representation of Cu in  $\text{Tl}_2\text{Ba}_2\text{CaCu}_2\text{O}_8$ 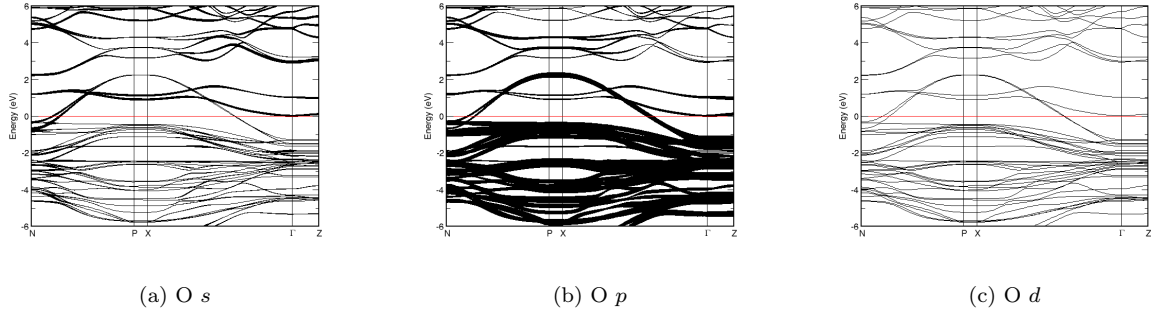FIG. 297: Fat band representation of O in  $\text{Tl}_2\text{Ba}_2\text{CaCu}_2\text{O}_8$ 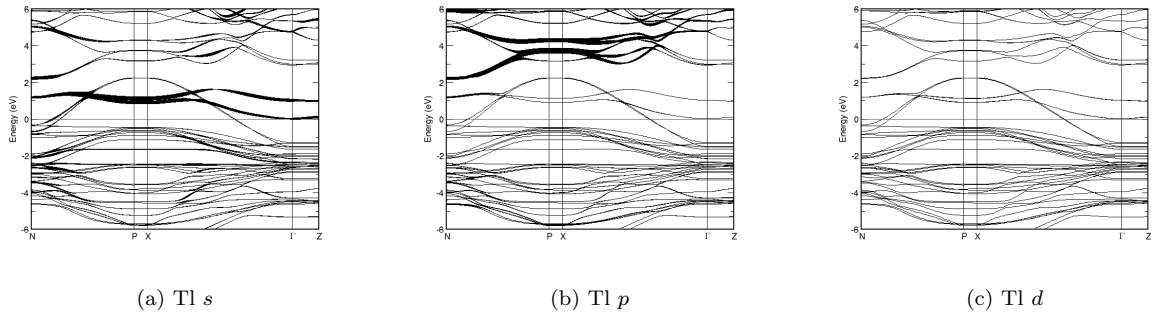FIG. 298: Fat band representation of Tl in  $\text{Tl}_2\text{Ba}_2\text{CaCu}_2\text{O}_8$

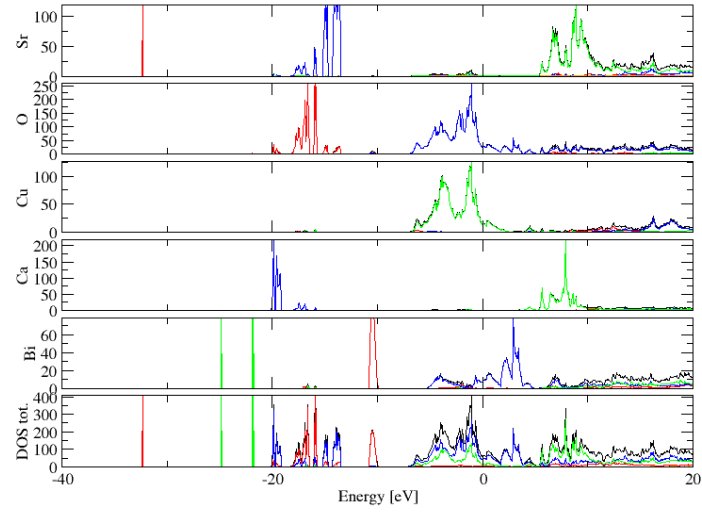

FIG. 299: (Color online) PDOS of  $\text{Bi}_2\text{Sr}_2\text{CaCu}_2\text{O}_8$  (ICSD #68188). The  $s$ -,  $p$ - and  $d$ -projected states are in red, blue and green, respectively.  $\text{Bi}_2\text{Sr}_2\text{CaCu}_2\text{O}_8$  crystallizes in space group  $I 4/m m m$  (#139), in a tetragonal body-centred structure.

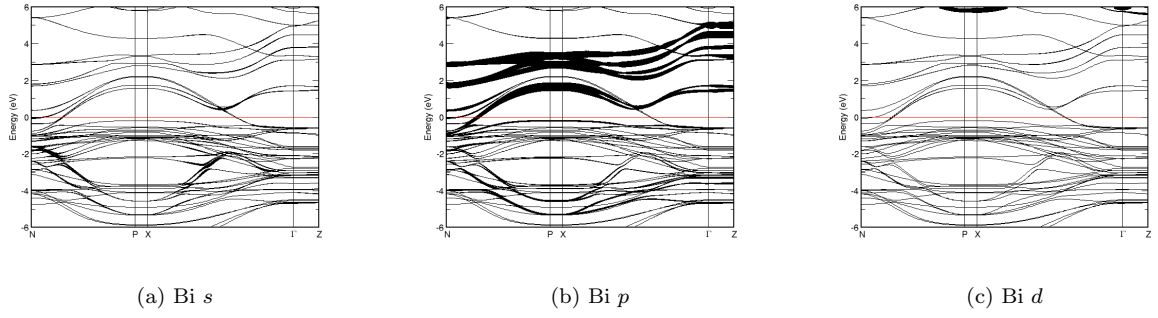

FIG. 300: Fat band representation of Bi in  $\text{Bi}_2\text{Sr}_2\text{CaCu}_2\text{O}_8$

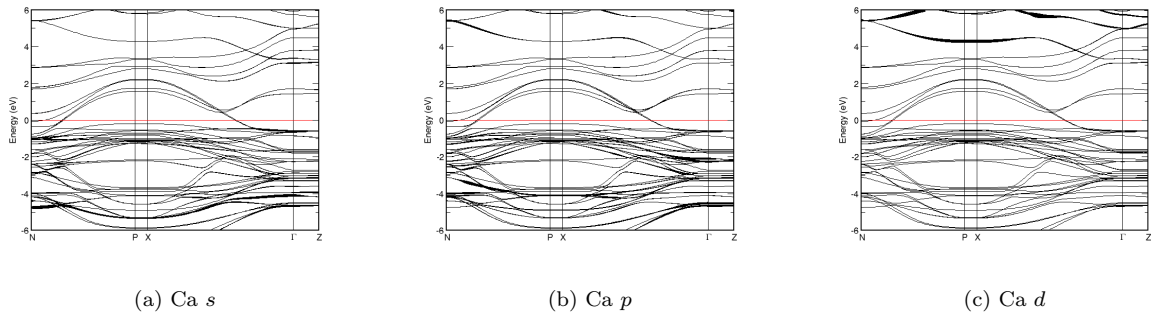

FIG. 301: Fat band representation of Ca in  $\text{Bi}_2\text{Sr}_2\text{CaCu}_2\text{O}_8$

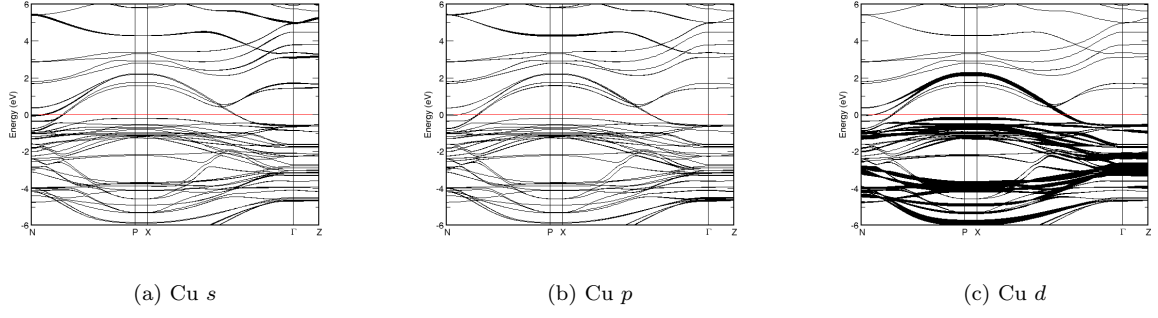FIG. 302: Fat band representation of Cu in  $\text{Bi}_2\text{Sr}_2\text{CaCu}_2\text{O}_8$ 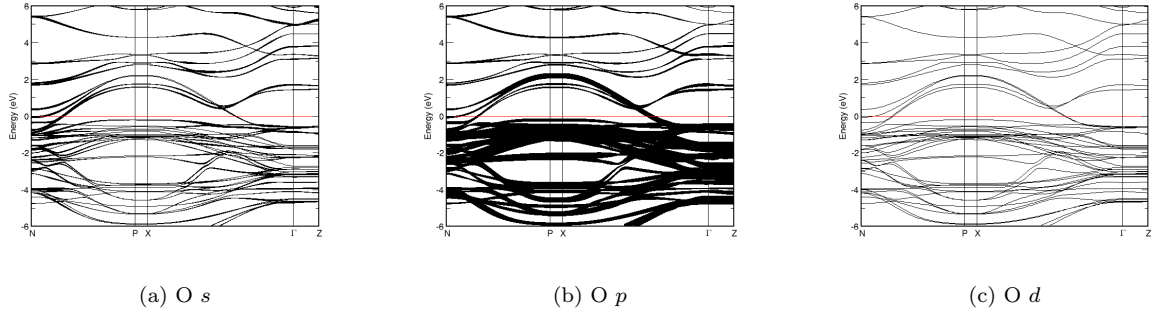FIG. 303: Fat band representation of O in  $\text{Bi}_2\text{Sr}_2\text{CaCu}_2\text{O}_8$ 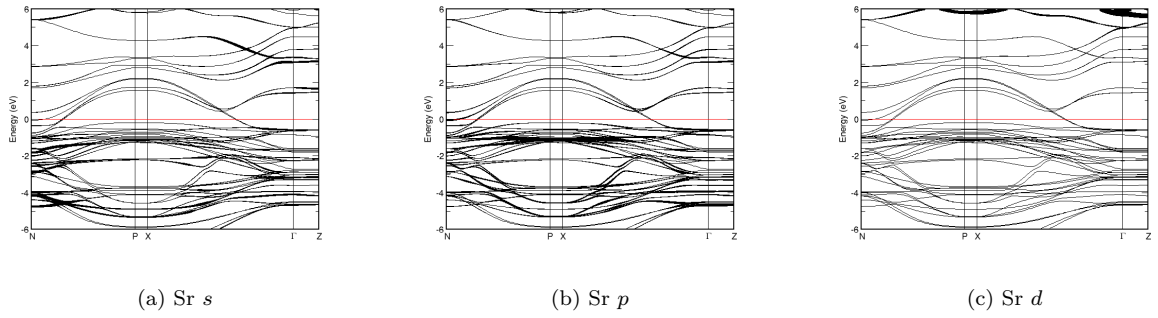FIG. 304: Fat band representation of Sr in  $\text{Bi}_2\text{Sr}_2\text{CaCu}_2\text{O}_8$

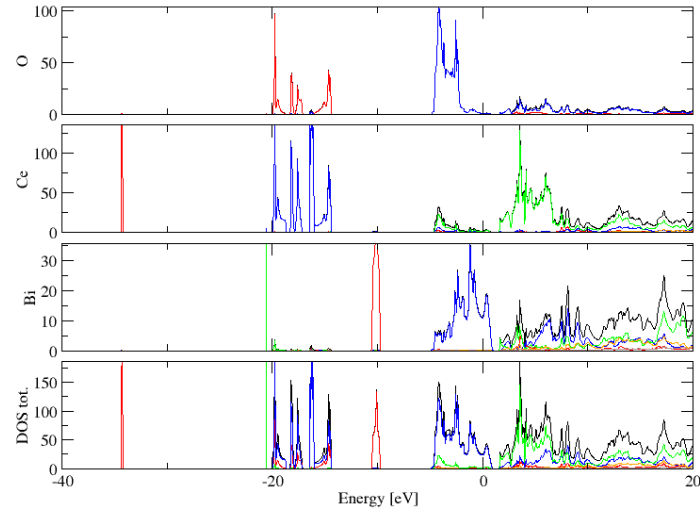

FIG. 305: (Color online) PDOS of  $\text{Ce}_2\text{BiO}_2$  (ICSD #9099). The  $s$ -,  $p$ - and  $d$ -projected states are in red, blue and green, respectively.  $\text{Ce}_2\text{BiO}_2$  crystallizes in space group  $I 4/m m m$  (#139), in a tetragonal body-centred structure.

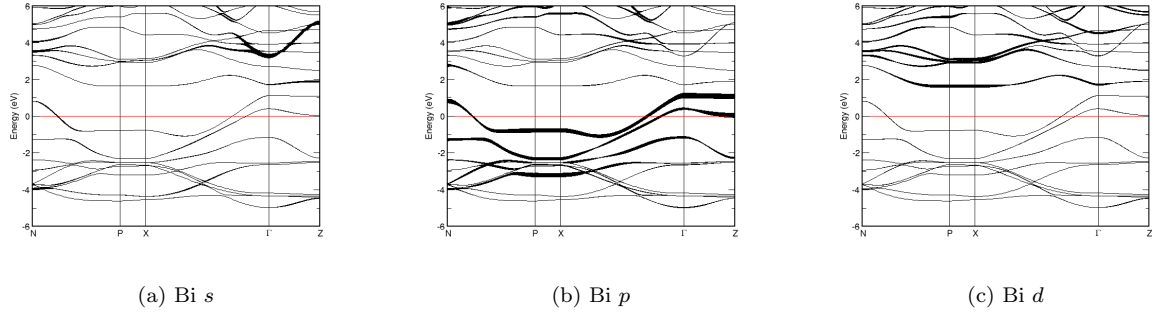

FIG. 306: Fat band representation of Bi in  $\text{Ce}_2\text{BiO}_2$

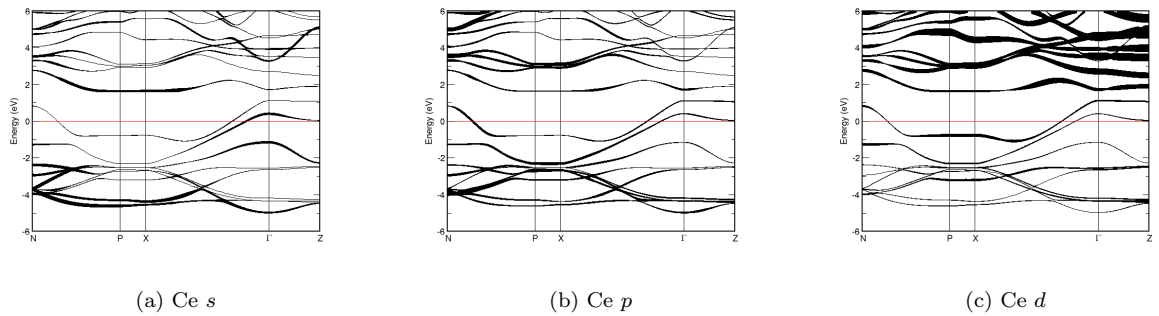

FIG. 307: Fat band representation of Ce in  $\text{Ce}_2\text{BiO}_2$

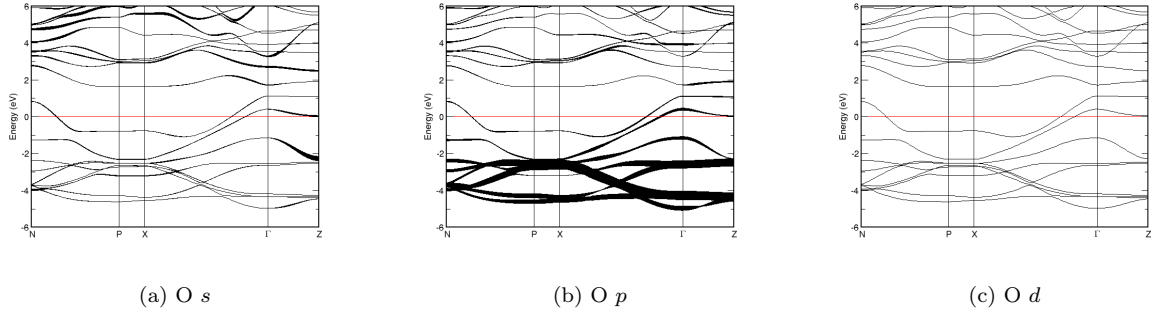FIG. 308: Fat band representation of O in  $\text{Ce}_2\text{BiO}_2$ 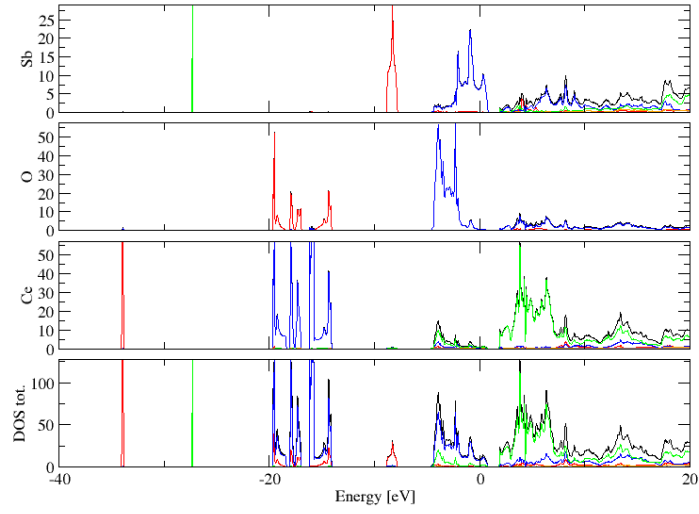FIG. 309: (Color online) PDOS of  $\text{Ce}_2\text{SbO}_2$  (ICSD #9100). The *s*-, *p*- and *d*-projected states are in red, blue and green, respectively.  $\text{Ce}_2\text{SbO}_2$  crystallizes in space group  $I 4/m m m$  (#139), in a tetragonal body-centred structure.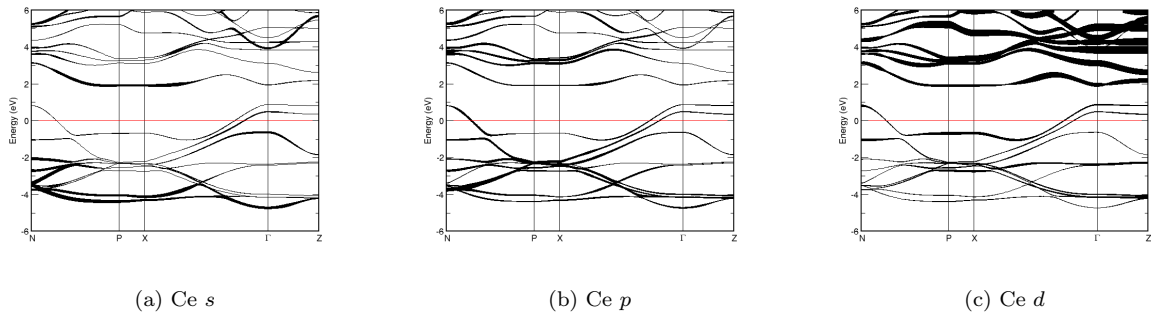FIG. 310: Fat band representation of Ce in  $\text{Ce}_2\text{SbO}_2$

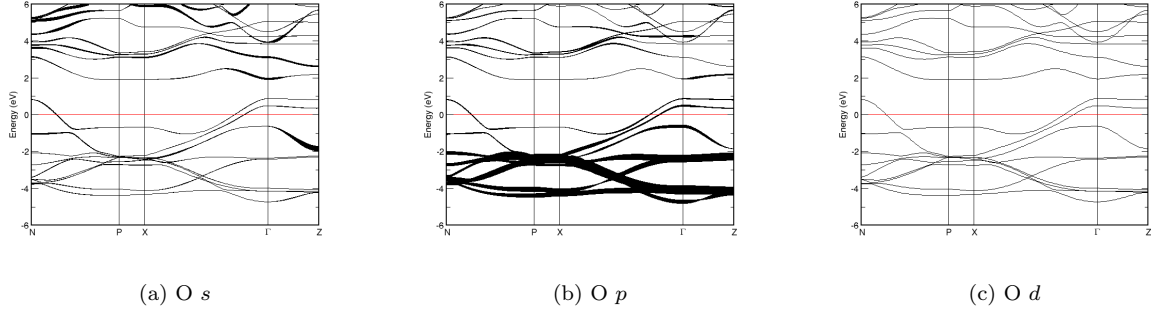FIG. 311: Fat band representation of O in  $\text{Ce}_2\text{SbO}_2$ 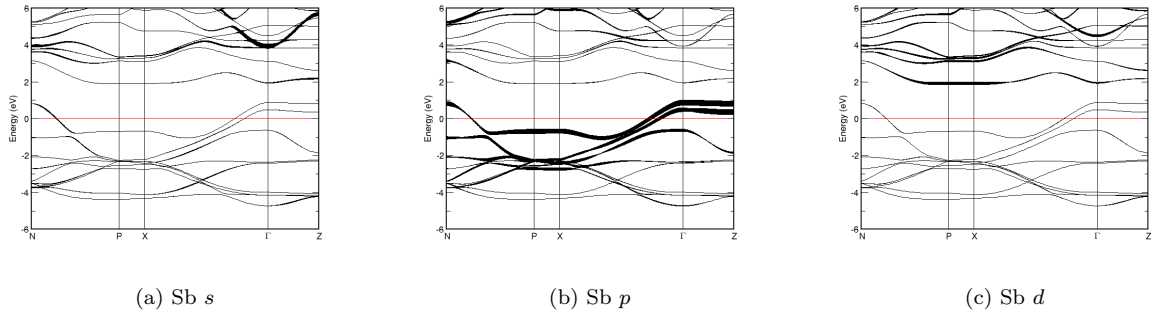FIG. 312: Fat band representation of Sb in  $\text{Ce}_2\text{SbO}_2$ 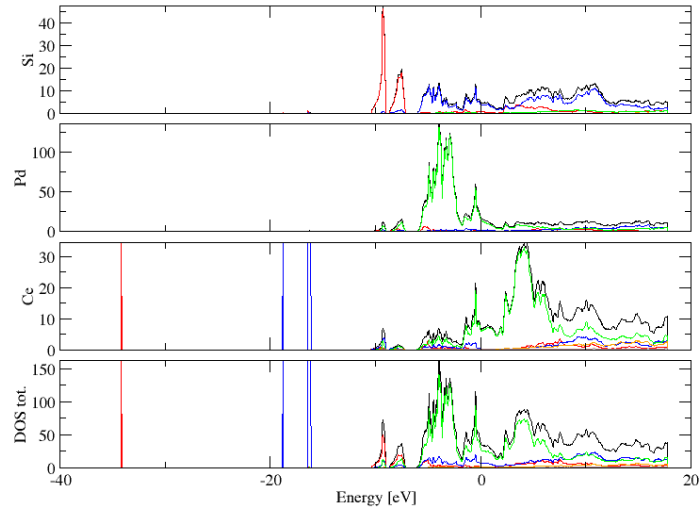FIG. 313: (Color online) PDOS of  $\text{CePd}_2\text{Si}_2$  (ICSD #621852). The *s*-, *p*- and *d*-projected states are in red, blue and green, respectively.  $\text{CePd}_2\text{Si}_2$  crystallizes in space group  $I 4/m m m$  (#139), in a tetragonal body-centred structure.

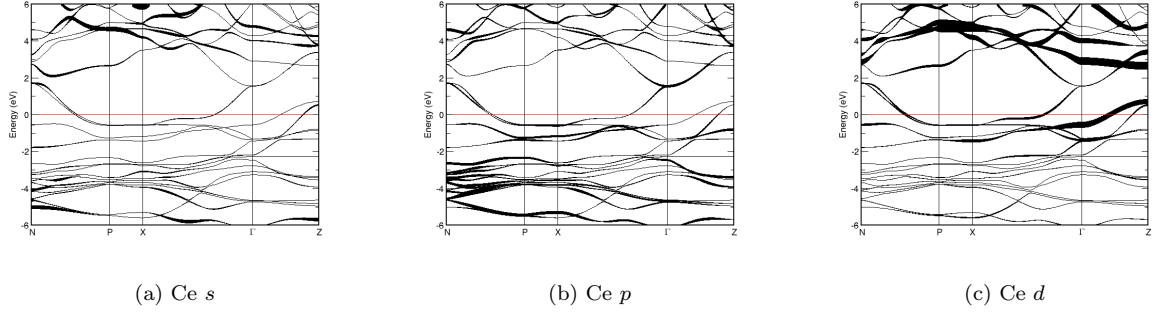FIG. 314: Fat band representation of Ce in  $\text{CePd}_2\text{Si}_2$ 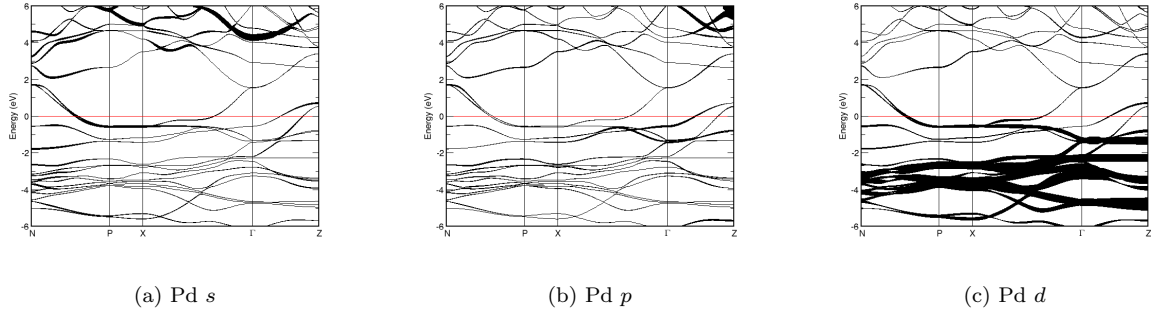FIG. 315: Fat band representation of Pd in  $\text{CePd}_2\text{Si}_2$ 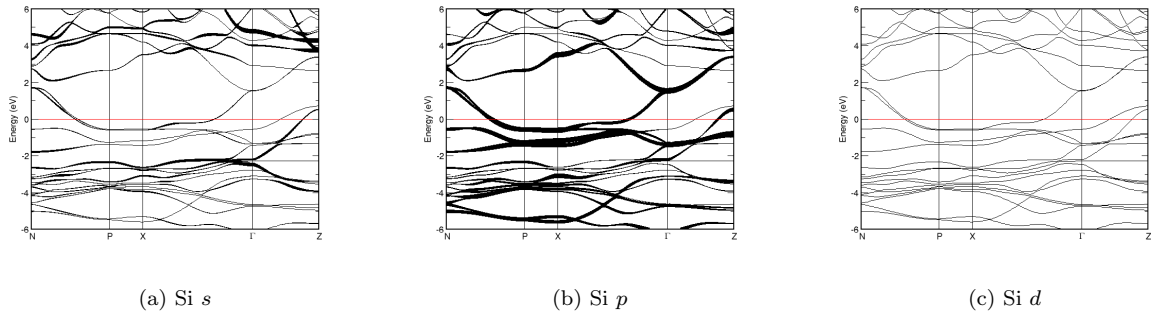FIG. 316: Fat band representation of Si in  $\text{CePd}_2\text{Si}_2$



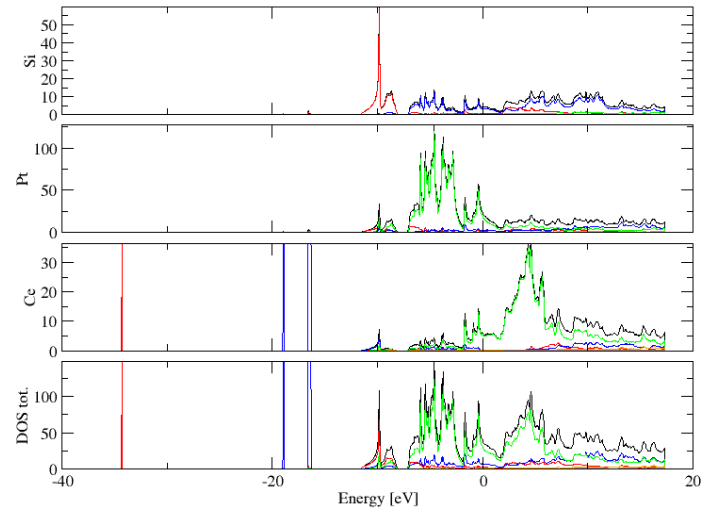

FIG. 317: (Color online) PDOS of  $\text{CePt}_2\text{Si}_2$  (ICSD #52895). The  $s$ -,  $p$ - and  $d$ -projected states are in red, blue and green, respectively.  $\text{CePt}_2\text{Si}_2$  crystallizes in space group  $I 4/m m m$  (#139), in a tetragonal body-centred structure.

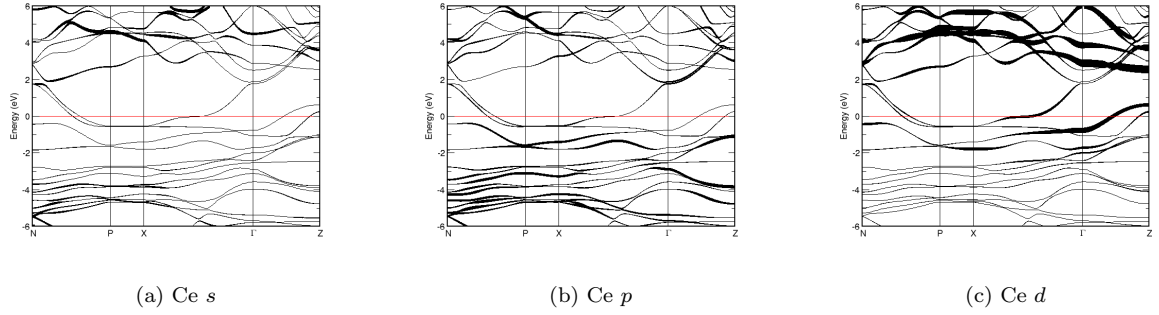

FIG. 318: Fat band representation of Ce in  $\text{CePt}_2\text{Si}_2$

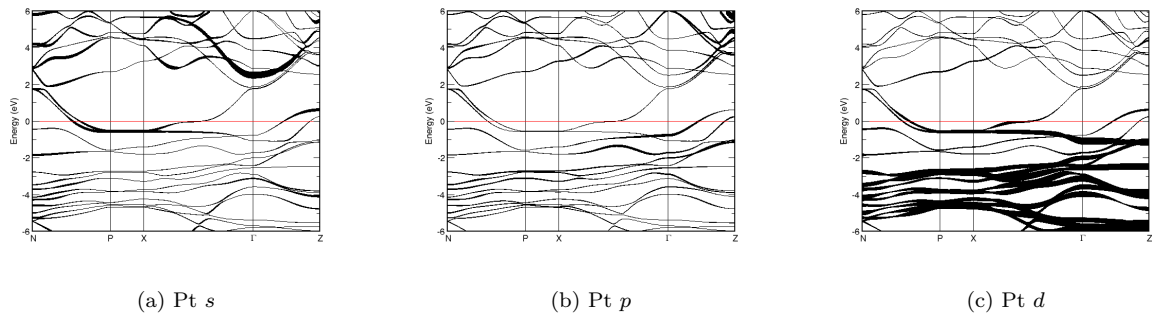

FIG. 319: Fat band representation of Pt in  $\text{CePt}_2\text{Si}_2$

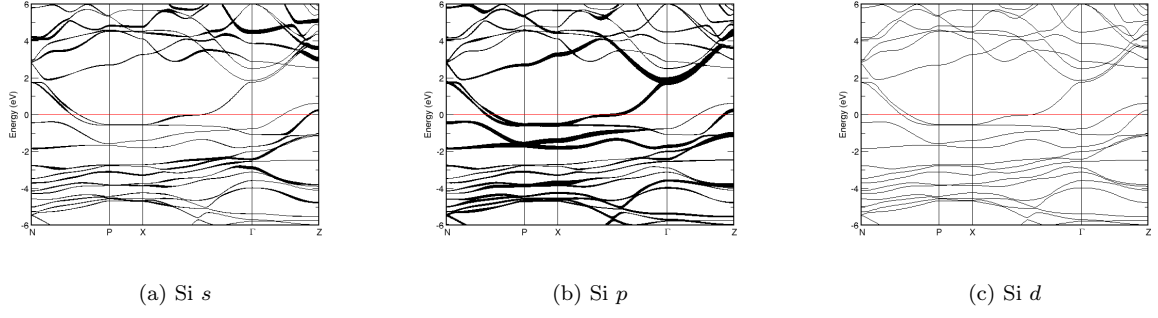FIG. 320: Fat band representation of Si in  $\text{CePt}_2\text{Si}_2$ 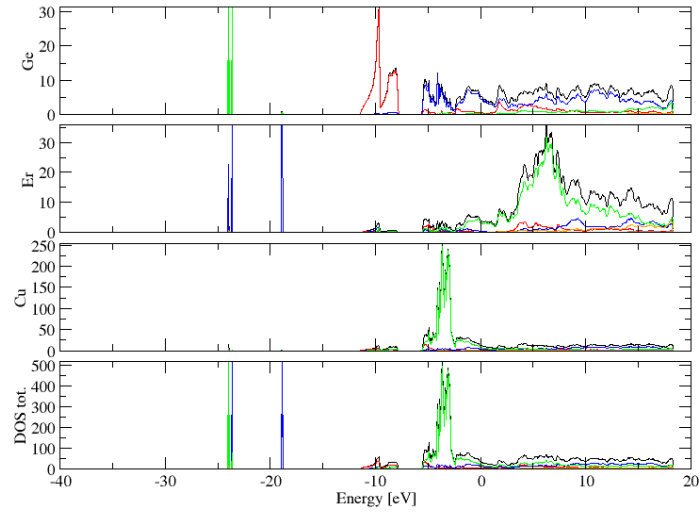FIG. 321: (Color online) PDOS of  $\text{Cu}_2\text{ErGe}_2$  (ICSD #53251). The *s*-, *p*- and *d*-projected states are in red, blue and green, respectively.  $\text{Cu}_2\text{ErGe}_2$  crystallizes in space group  $I 4/m m m$  (#139), in a tetragonal body-centred structure.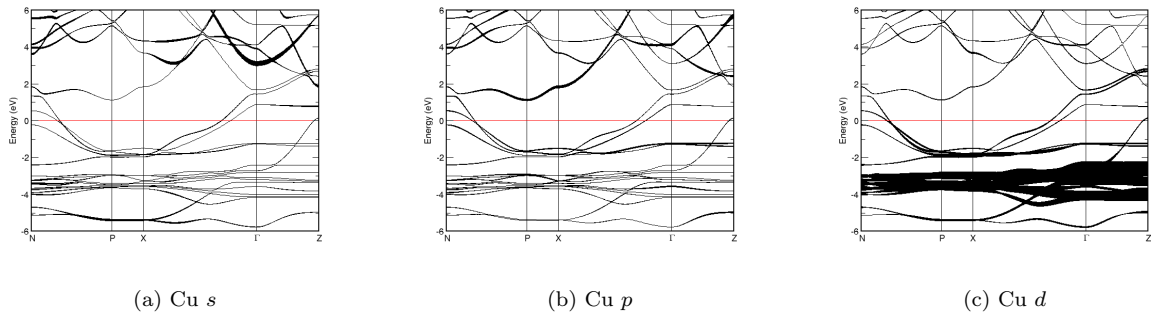FIG. 322: Fat band representation of Cu in  $\text{Cu}_2\text{ErGe}_2$

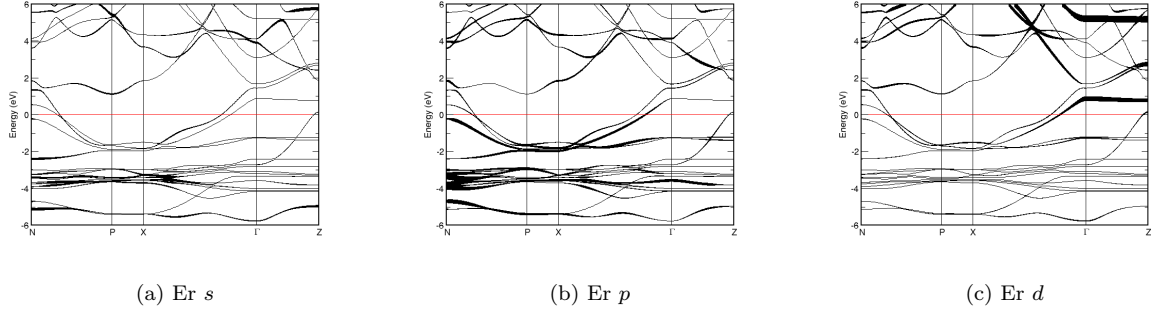FIG. 323: Fat band representation of Er in  $\text{Cu}_2\text{ErGe}_2$ 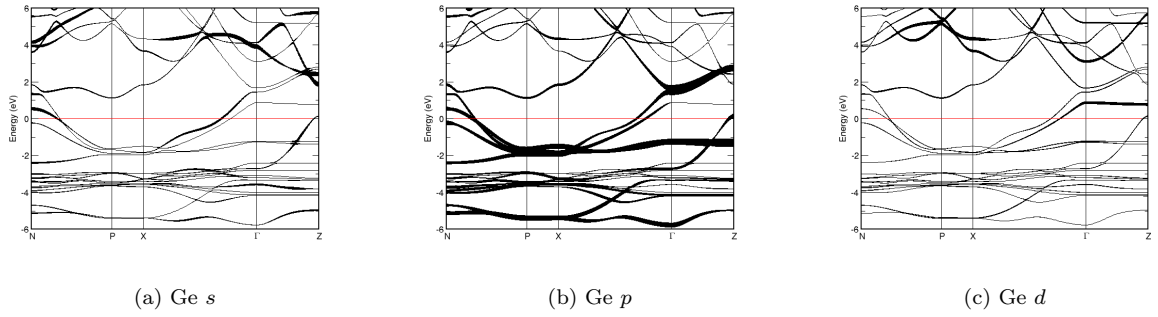FIG. 324: Fat band representation of Ge in  $\text{Cu}_2\text{ErGe}_2$ 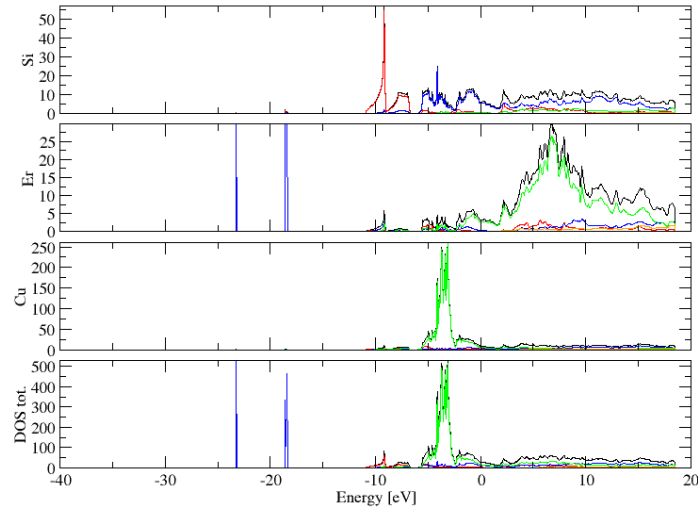FIG. 325: (Color online) PDOS of  $\text{ErCu}_2\text{Si}_2$  (ICSD #106845). The *s*-, *p*- and *d*-projected states are in red, blue and green, respectively.  $\text{ErCu}_2\text{Si}_2$  crystallizes in space group  $I 4/m m m$  (#139), in a tetragonal body-centred structure.

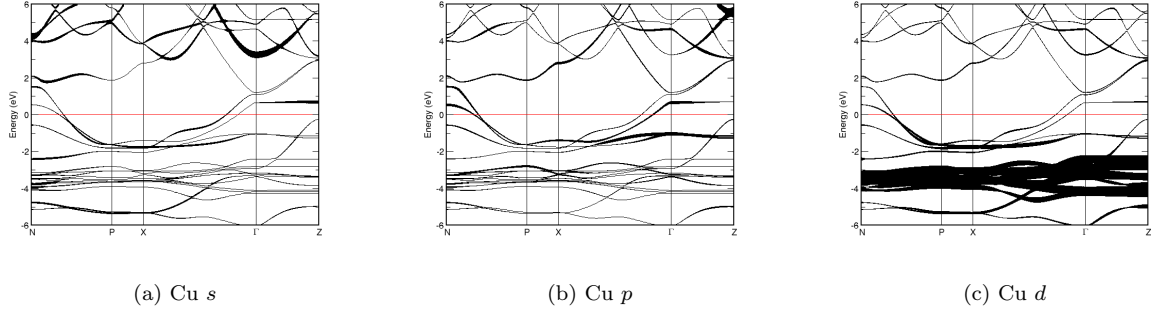FIG. 326: Fat band representation of Cu in  $\text{ErCu}_2\text{Si}_2$ 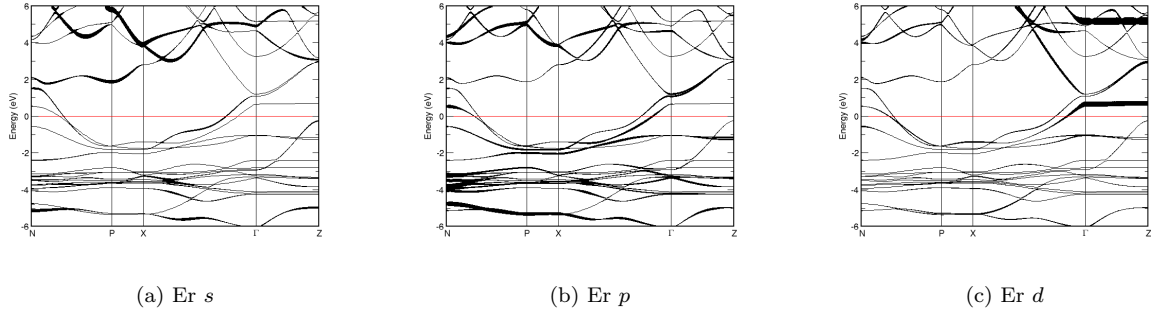FIG. 327: Fat band representation of Er in  $\text{ErCu}_2\text{Si}_2$ 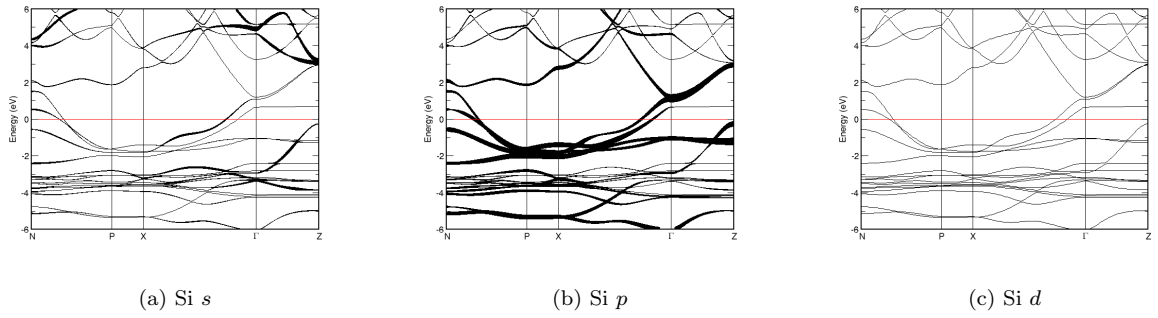FIG. 328: Fat band representation of Si in  $\text{ErCu}_2\text{Si}_2$

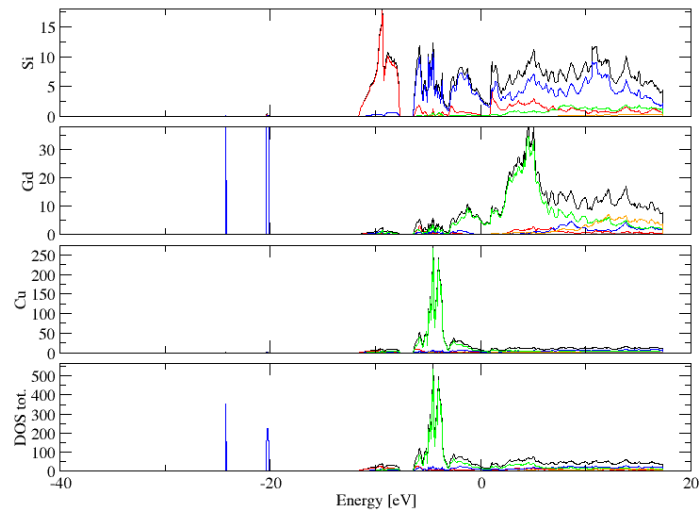

FIG. 329: (Color online) PDOS of  $\text{Cu}_2\text{GdSi}_2$  (ICSD #64825). The  $s$ -,  $p$ - and  $d$ -projected states are in red, blue and green, respectively.  $\text{Cu}_2\text{GdSi}_2$  crystallizes in space group  $I 4/m m m$  (#139), in a tetragonal body-centred structure.

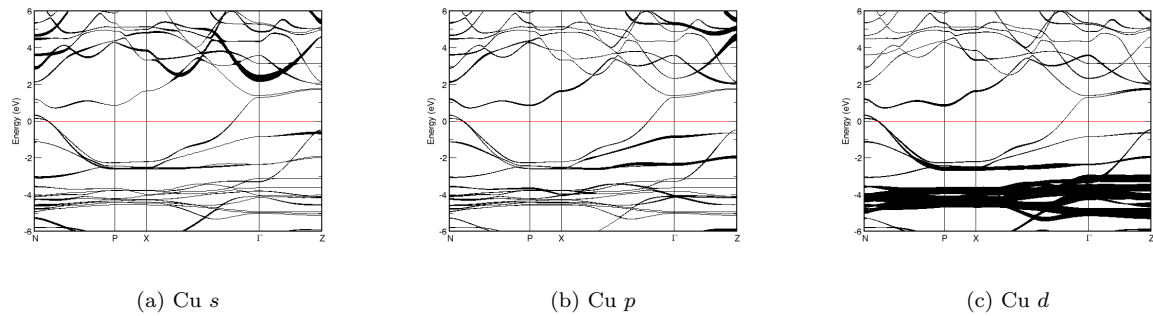

FIG. 330: Fat band representation of Cu in  $\text{Cu}_2\text{GdSi}_2$

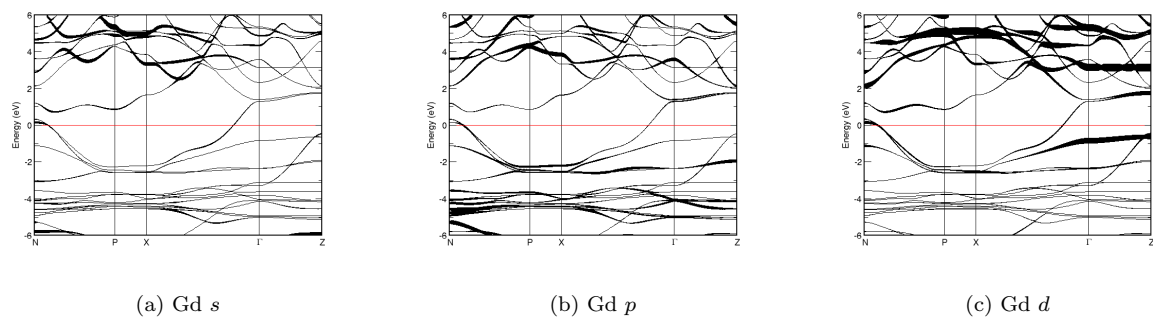

FIG. 331: Fat band representation of Gd in  $\text{Cu}_2\text{GdSi}_2$

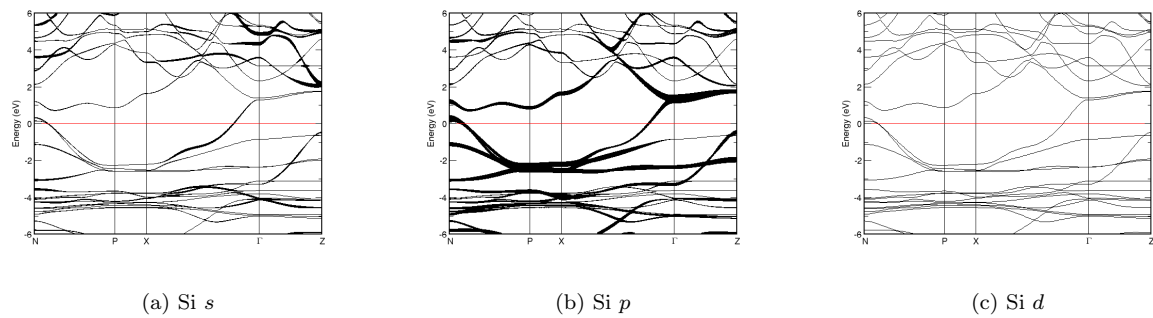FIG. 332: Fat band representation of Si in  $\text{Cu}_2\text{GdSi}_2$ 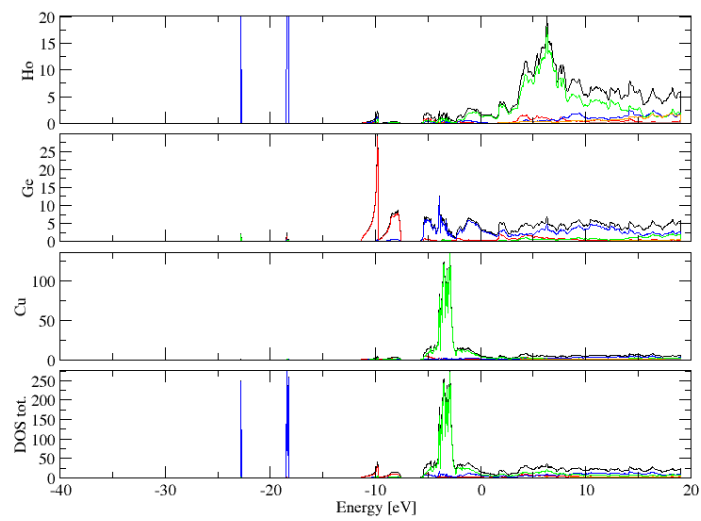FIG. 333: (Color online) PDOS of  $\text{Cu}_2\text{HoGe}_2$  (ICSD #53270). The  $s$ -,  $p$ - and  $d$ -projected states are in red, blue and green, respectively.  $\text{Cu}_2\text{HoGe}_2$  crystallizes in space group  $I 4/m m m$  (#139), in a tetragonal body-centred structure.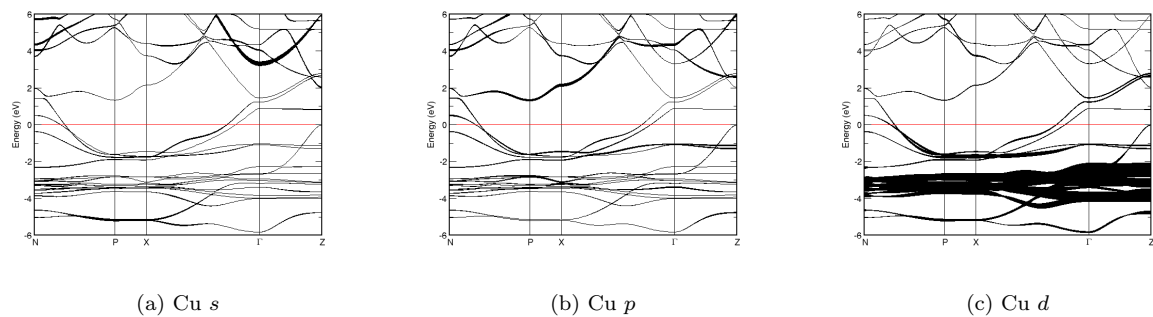FIG. 334: Fat band representation of Cu in  $\text{Cu}_2\text{HoGe}_2$

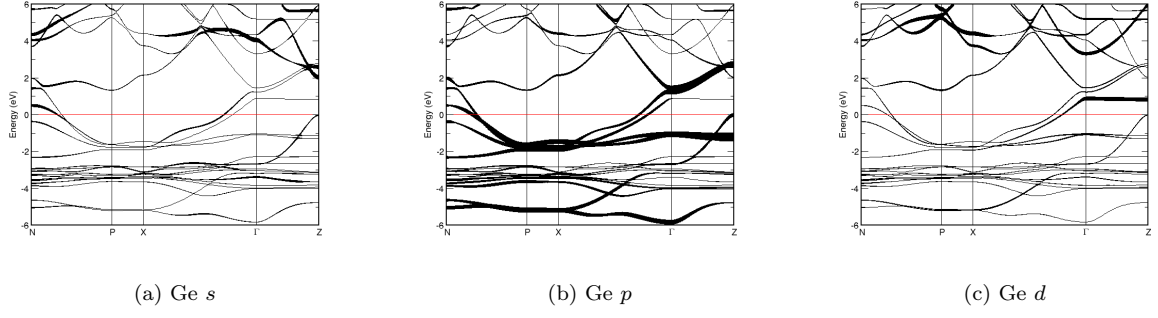FIG. 335: Fat band representation of Ge in  $\text{Cu}_2\text{HoGe}_2$ 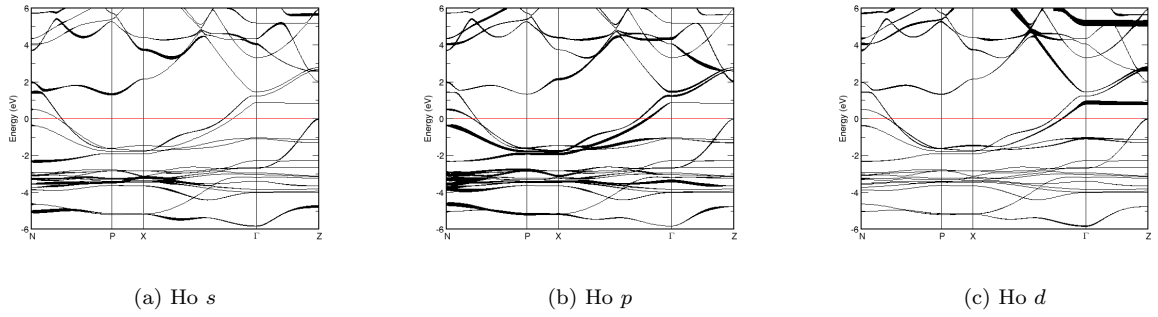FIG. 336: Fat band representation of Ho in  $\text{Cu}_2\text{HoGe}_2$ 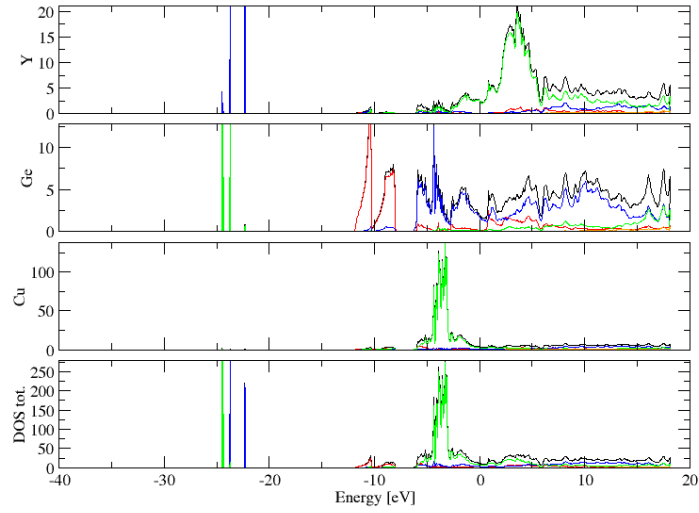FIG. 337: (Color online) PDOS of  $\text{YCu}_2\text{Ge}_2$  (ICSD #52764). The *s*-, *p*- and *d*-projected states are in red, blue and green, respectively.  $\text{YCu}_2\text{Ge}_2$  crystallizes in space group  $I 4/m m m$  (#139), in a tetragonal body-centred structure.

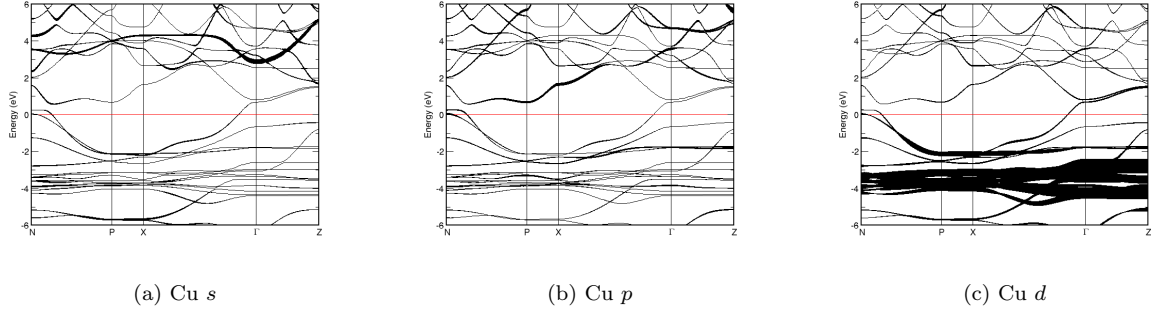FIG. 338: Fat band representation of Cu in  $\text{YCu}_2\text{Ge}_2$ 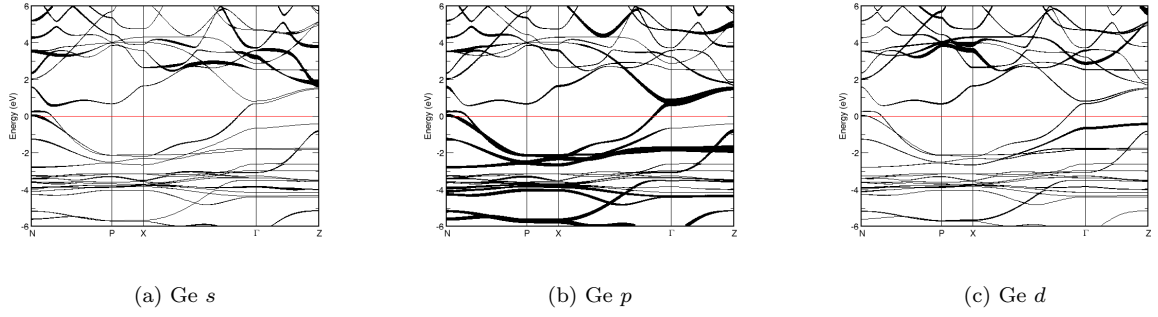FIG. 339: Fat band representation of Ge in  $\text{YCu}_2\text{Ge}_2$ 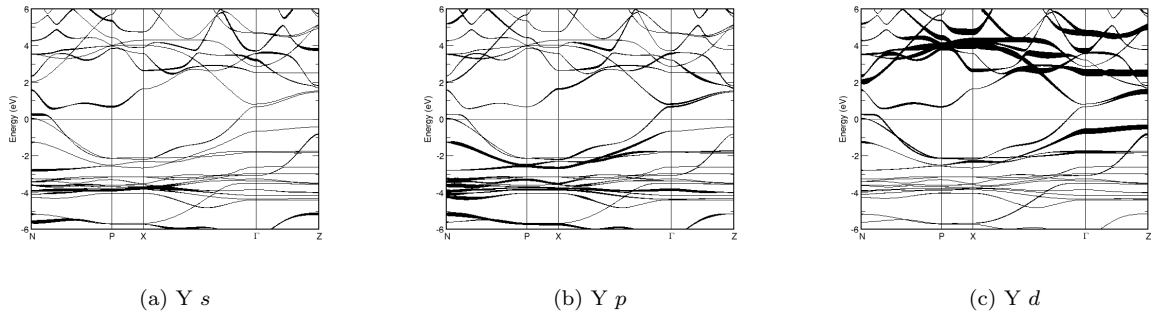FIG. 340: Fat band representation of Y in  $\text{YCu}_2\text{Ge}_2$



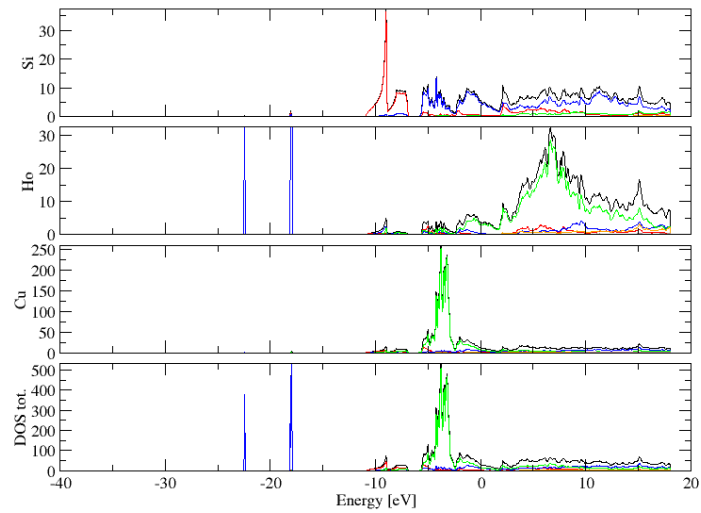

FIG. 341: (Color online) PDOS of  $\text{Cu}_2\text{HoSi}_2$  (ICSD #53289). The  $s$ -,  $p$ - and  $d$ -projected states are in red, blue and green, respectively.  $\text{Cu}_2\text{HoSi}_2$  crystallizes in space group  $I 4/m m m$  (#139), in a tetragonal body-centred structure.

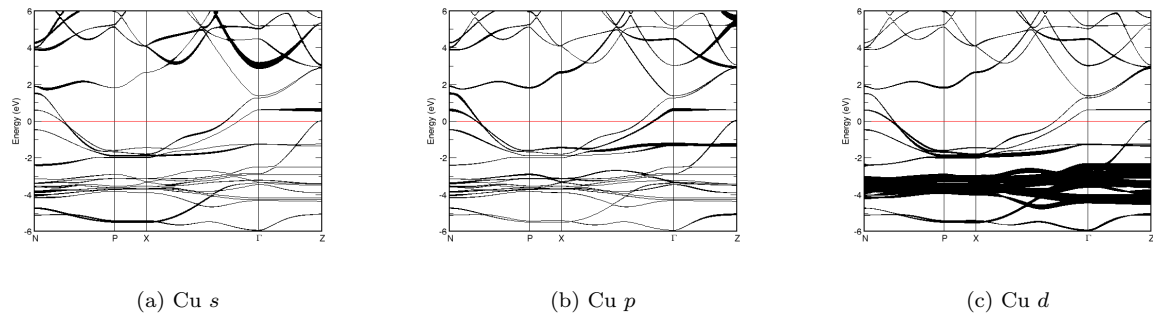

FIG. 342: Fat band representation of Cu in  $\text{Cu}_2\text{HoSi}_2$

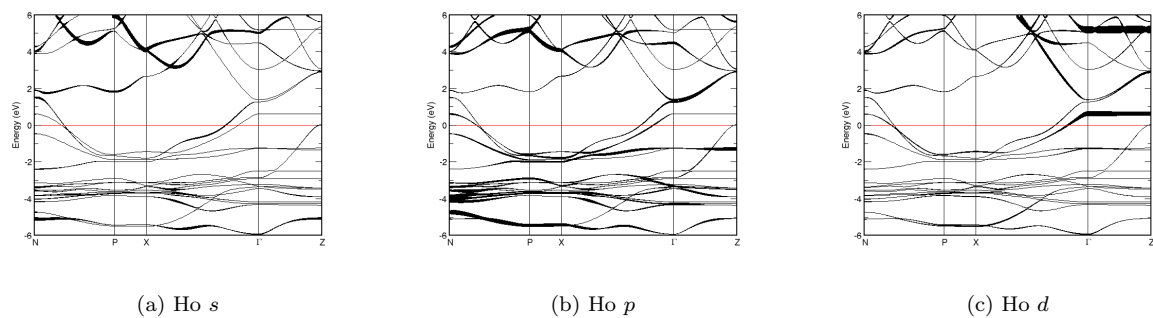

FIG. 343: Fat band representation of Ho in  $\text{Cu}_2\text{HoSi}_2$

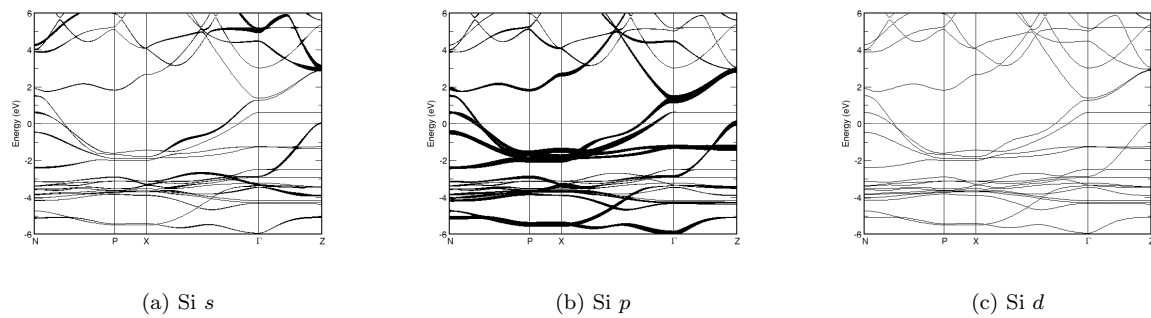FIG. 344: Fat band representation of Si in  $\text{Cu}_2\text{HoSi}_2$ 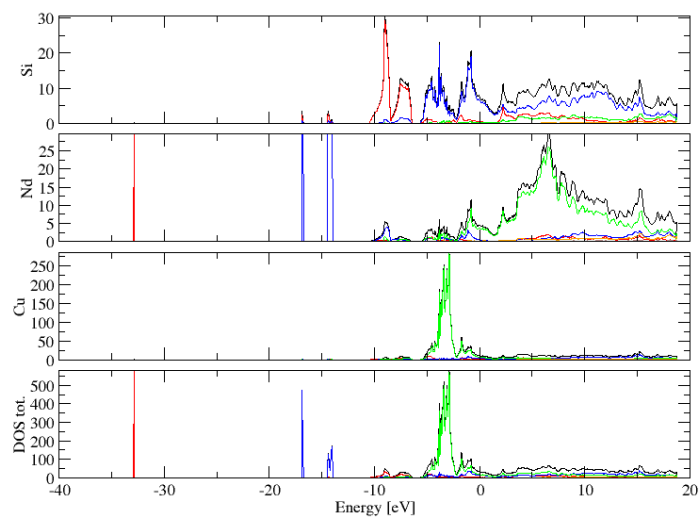FIG. 345: (Color online) PDOS of  $\text{NdCu}_2\text{Si}_2$  (ICSD #106842). The *s*-, *p*- and *d*-projected states are in red, blue and green, respectively.  $\text{NdCu}_2\text{Si}_2$  crystallizes in space group I  $4/m\ m\ m$  (#139), in a tetragonal body-centred structure.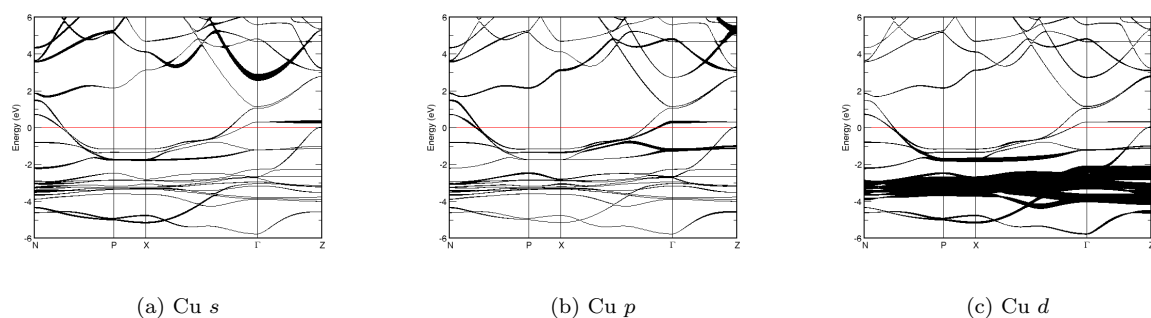FIG. 346: Fat band representation of Cu in  $\text{NdCu}_2\text{Si}_2$

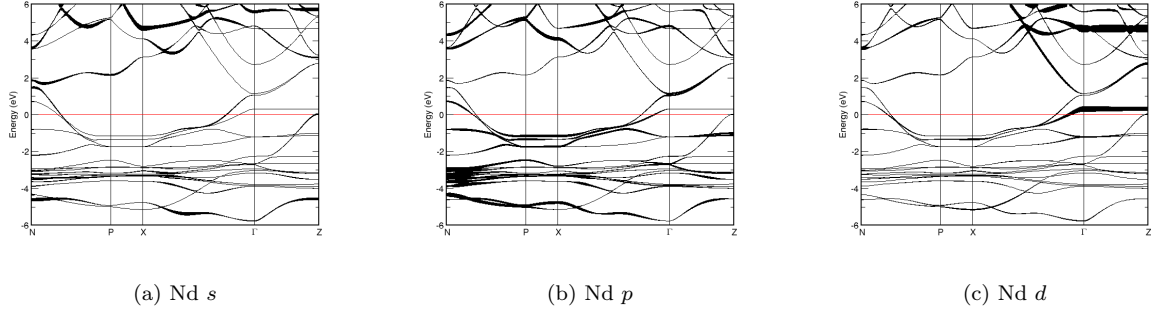FIG. 347: Fat band representation of Nd in NdCu<sub>2</sub>Si<sub>2</sub>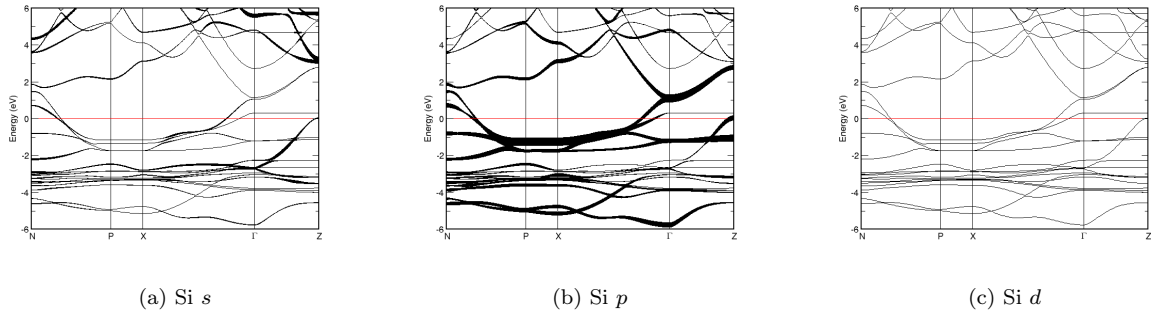FIG. 348: Fat band representation of Si in NdCu<sub>2</sub>Si<sub>2</sub>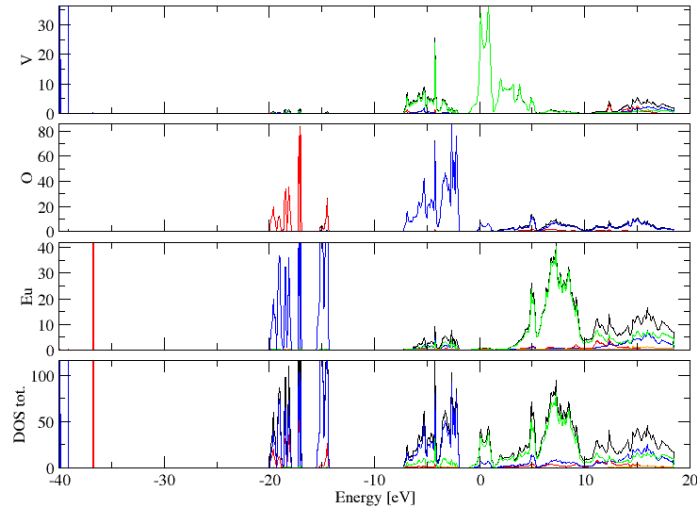FIG. 349: (Color online) PDOS of Eu<sub>2</sub>(VO<sub>4</sub>) (ICSD #89000). The *s*-, *p*- and *d*-projected states are in red, blue and green, respectively. Eu<sub>2</sub>(VO<sub>4</sub>) crystallizes in space group I 4/m m m (#139), in a tetragonal body-centred structure.

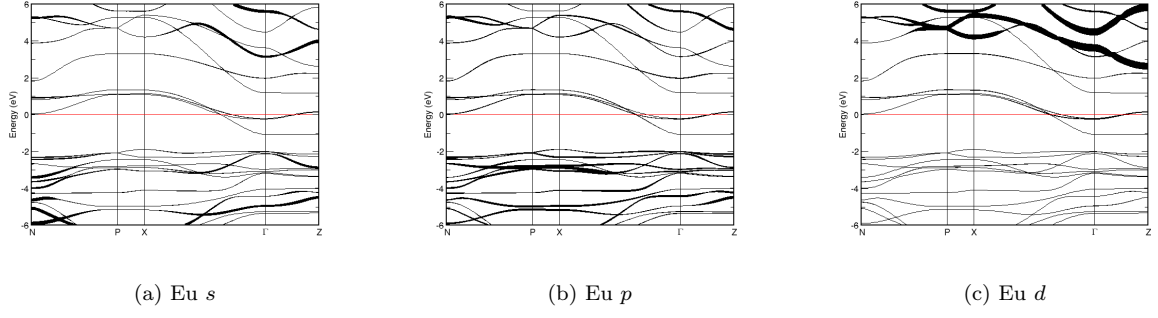FIG. 350: Fat band representation of Eu in  $\text{Eu}_2(\text{VO}_4)$ 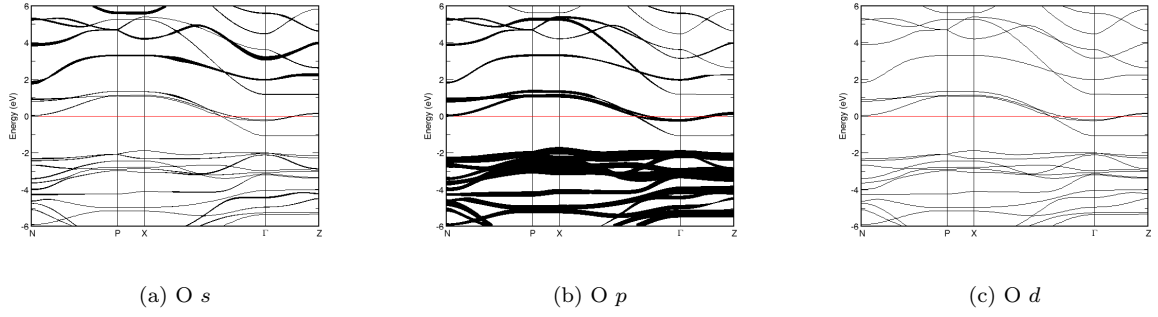FIG. 351: Fat band representation of O in  $\text{Eu}_2(\text{VO}_4)$ 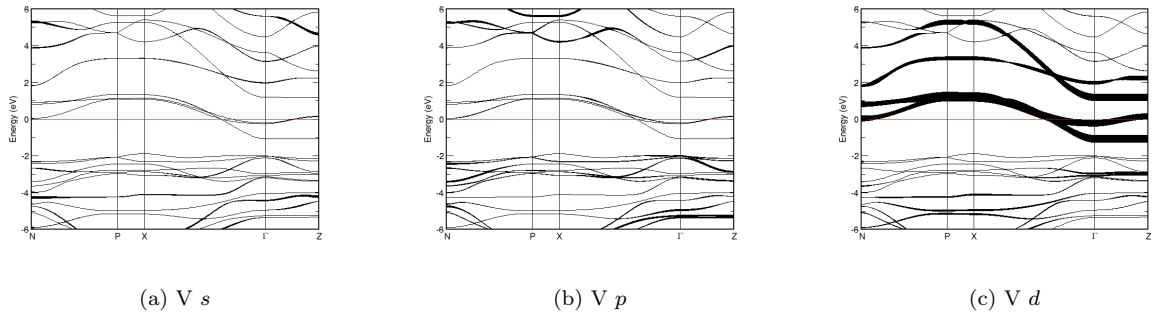FIG. 352: Fat band representation of V in  $\text{Eu}_2(\text{VO}_4)$

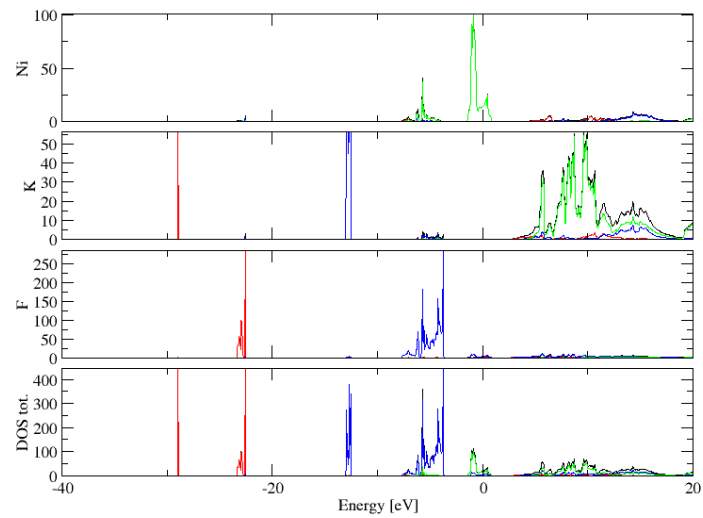

FIG. 353: (Color online) PDOS of  $\text{K}_2(\text{NiF}_4)$  (ICSD #15576). The  $s$ -,  $p$ - and  $d$ -projected states are in red, blue and green, respectively.  $\text{K}_2(\text{NiF}_4)$  crystallizes in space group  $I 4/m m m$  (#139), in a tetragonal body-centred structure.

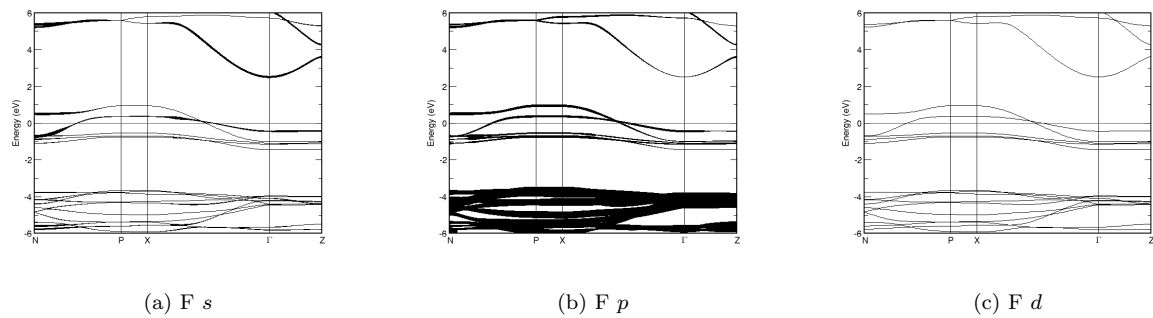

FIG. 354: Fat band representation of F in  $\text{K}_2(\text{NiF}_4)$

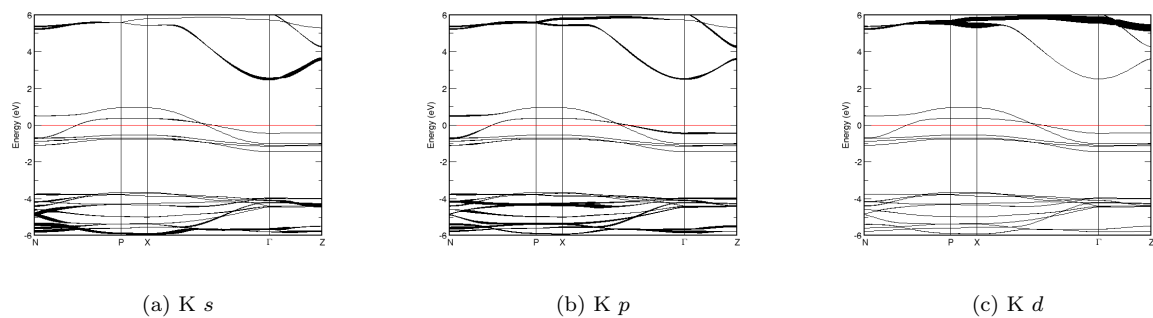

FIG. 355: Fat band representation of K in  $\text{K}_2(\text{NiF}_4)$

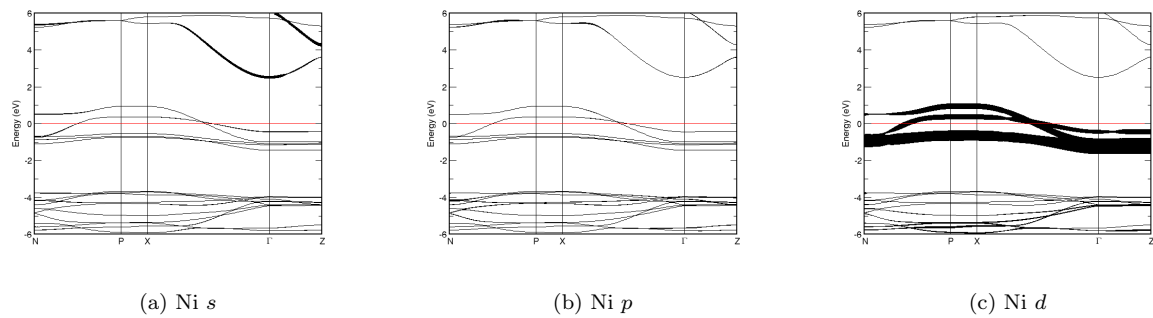FIG. 356: Fat band representation of Ni in  $K_2(NiF_4)$ 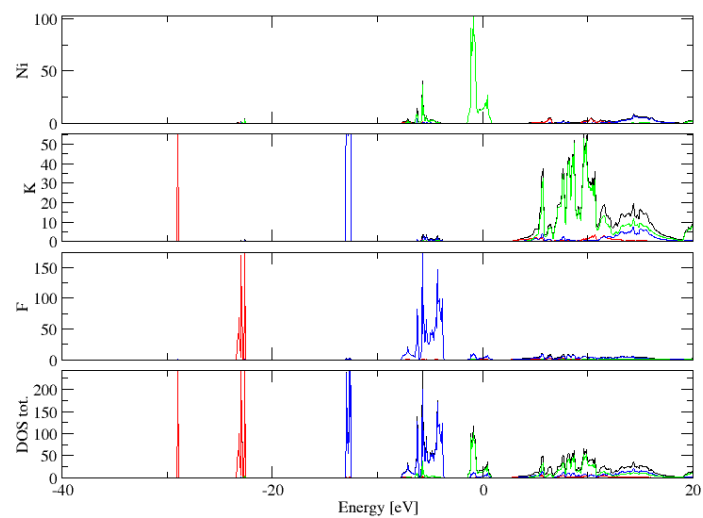FIG. 357: (Color online) PDOS of  $K_2(NiF_4)$  (ICSD #631720). The *s*-, *p*- and *d*-projected states are in red, blue and green, respectively.  $K_2(NiF_4)$  crystallizes in space group  $I 4/m m m$  (#139), in a tetragonal body-centred structure.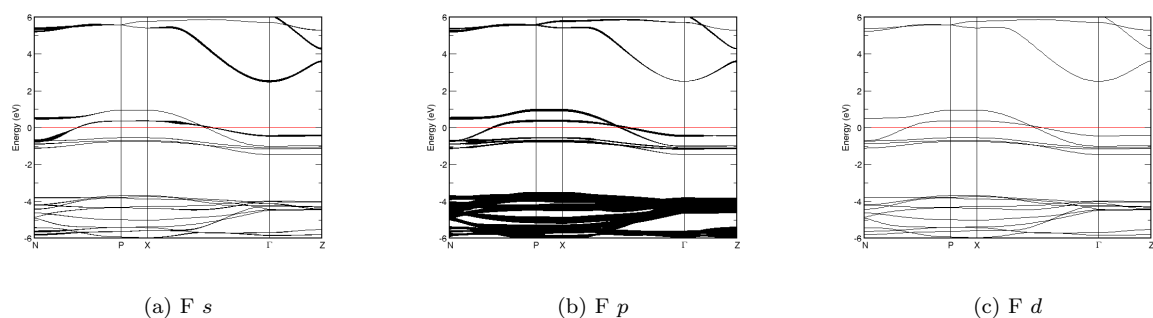FIG. 358: Fat band representation of F in  $K_2(NiF_4)$

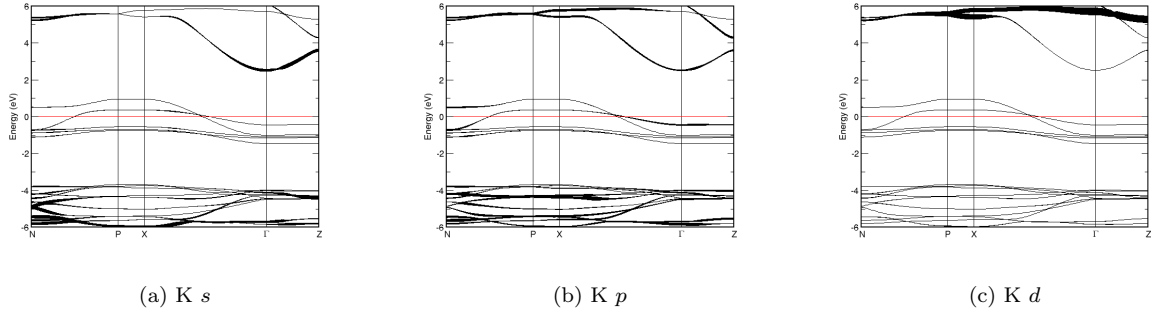FIG. 359: Fat band representation of K in  $K_2(NiF_4)$ 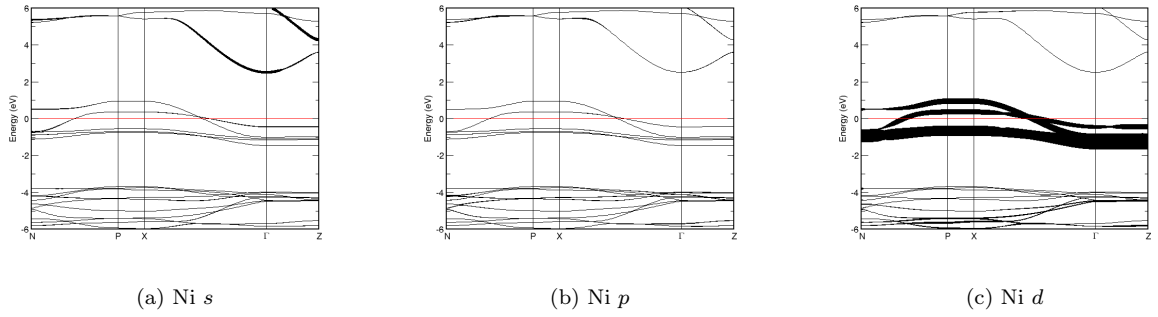FIG. 360: Fat band representation of Ni in  $K_2(NiF_4)$ 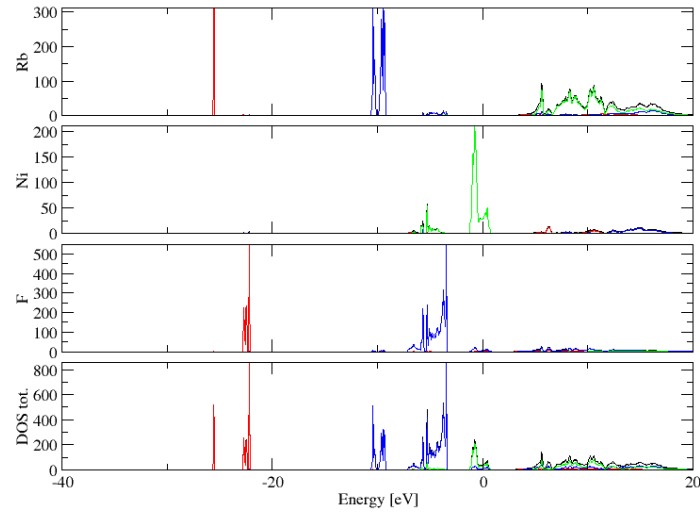FIG. 361: (Color online) PDOS of  $Rb_2(NiF_4)$  (ICSD #69682). The *s*-, *p*- and *d*-projected states are in red, blue and green, respectively.  $Rb_2(NiF_4)$  crystallizes in space group  $I 4/m m m$  (#139), in a tetragonal body-centred structure.

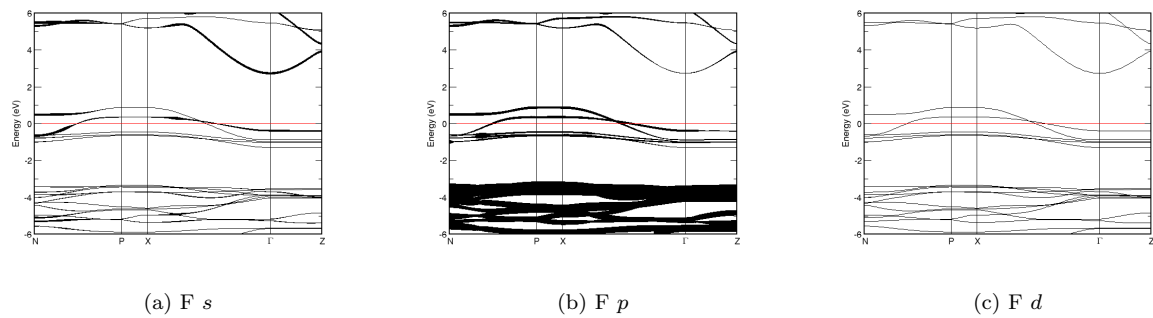FIG. 362: Fat band representation of F in  $\text{Rb}_2(\text{NiF}_4)$ 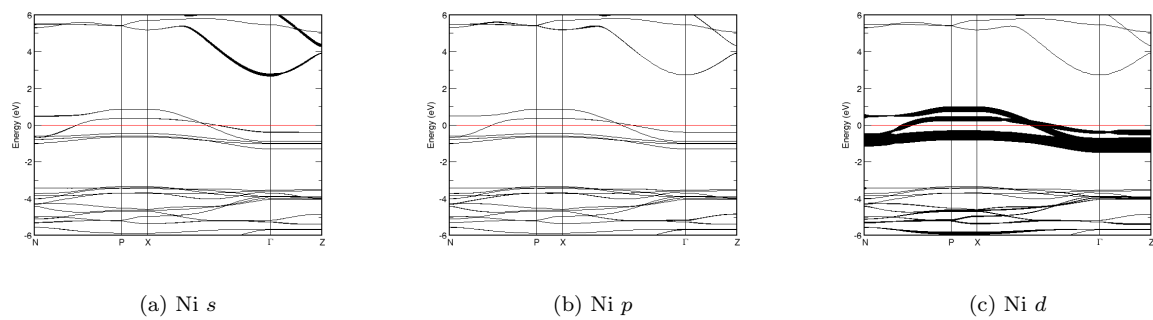FIG. 363: Fat band representation of Ni in  $\text{Rb}_2(\text{NiF}_4)$ 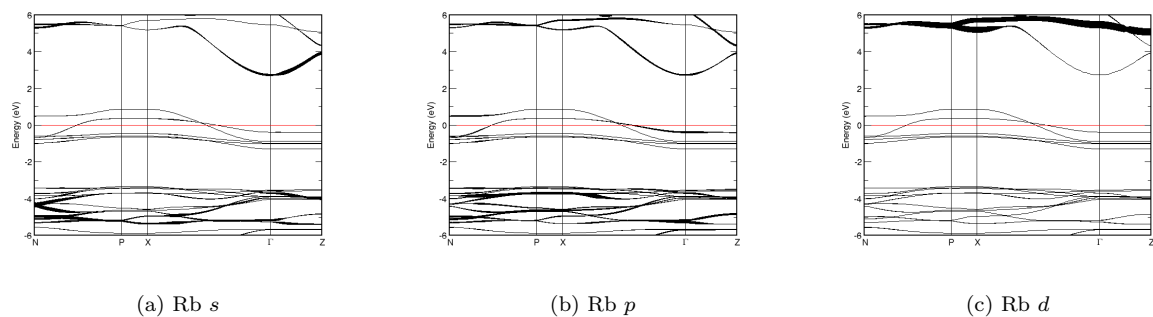FIG. 364: Fat band representation of Rb in  $\text{Rb}_2(\text{NiF}_4)$



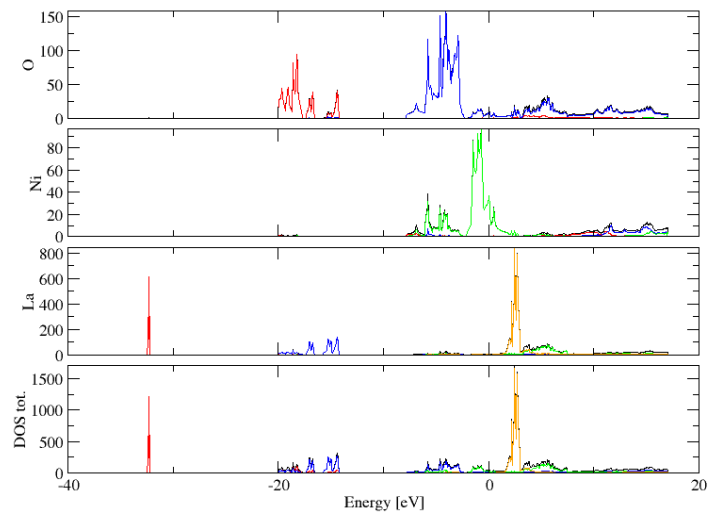

FIG. 365: (Color online) PDOS of  $\text{La}_2(\text{NiO}_4)$  (ICSD #1179). The  $s$ -,  $p$ - and  $d$ -projected states are in red, blue and green, respectively.  $\text{La}_2(\text{NiO}_4)$  crystallizes in space group  $I 4/m m m$  (#139), in a tetragonal body-centred structure.

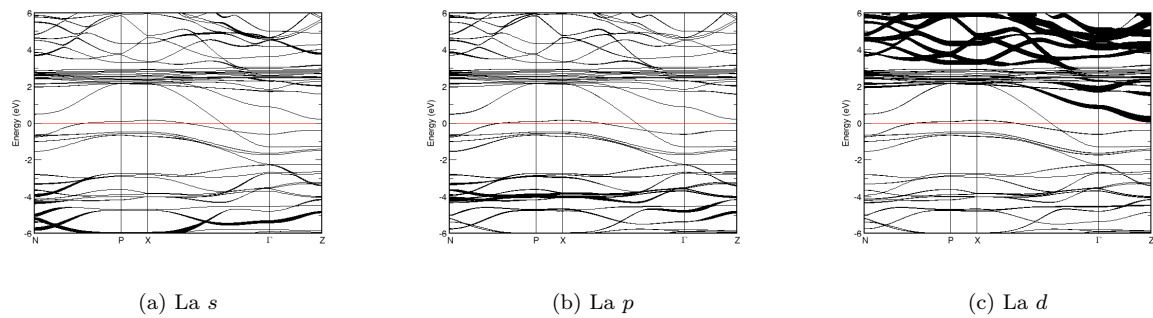

FIG. 366: Fat band representation of La in  $\text{La}_2(\text{NiO}_4)$

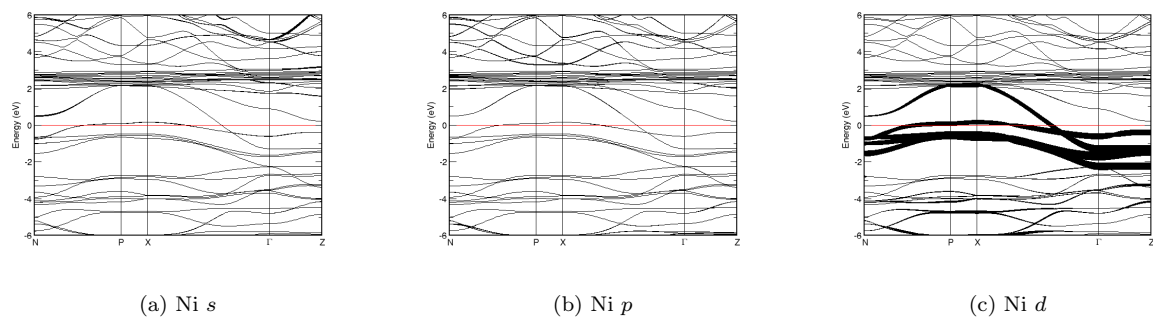

FIG. 367: Fat band representation of Ni in  $\text{La}_2(\text{NiO}_4)$

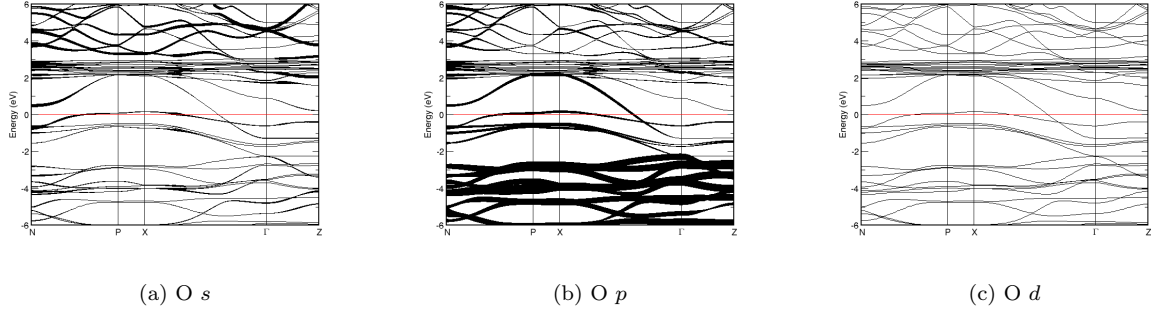

FIG. 368: Fat band representation of O in  $\text{La}_2(\text{NiO}_4)$

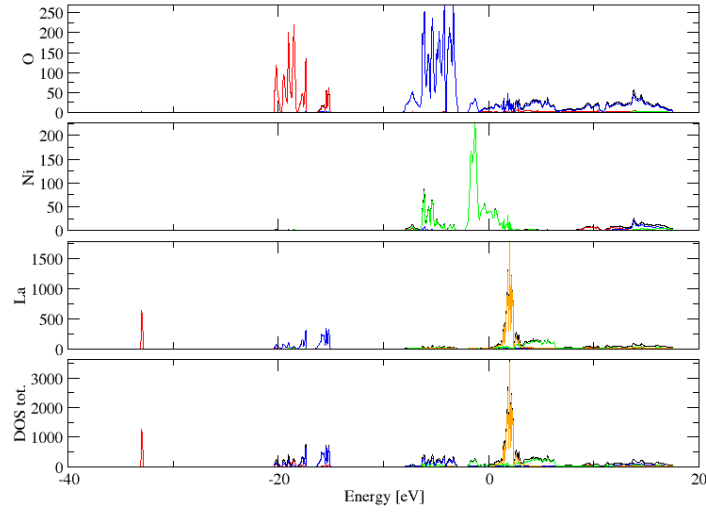

FIG. 369: (Color online) PDOS of  $\text{La}_2(\text{NiO}_4)$  (ICSD #33536). The  $s$ -,  $p$ - and  $d$ -projected states are in red, blue and green, respectively.  $\text{La}_2(\text{NiO}_4)$  crystallizes in space group  $I 4/m m m$  (#139), in a tetragonal body-centred structure.

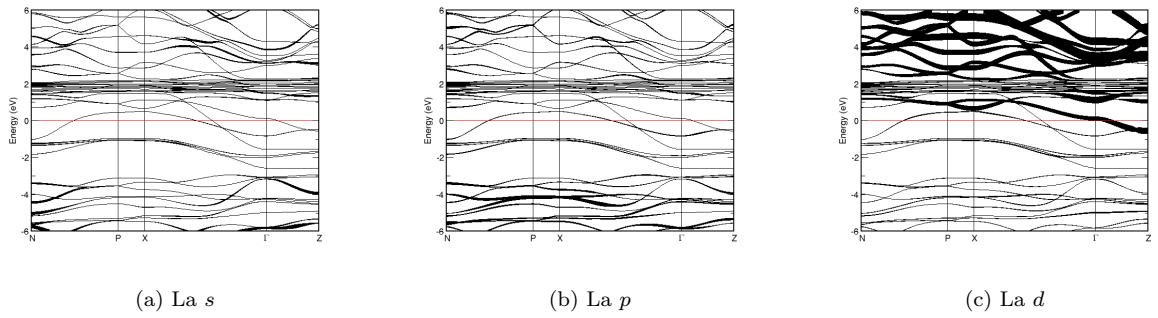

FIG. 370: Fat band representation of La in  $\text{La}_2(\text{NiO}_4)$

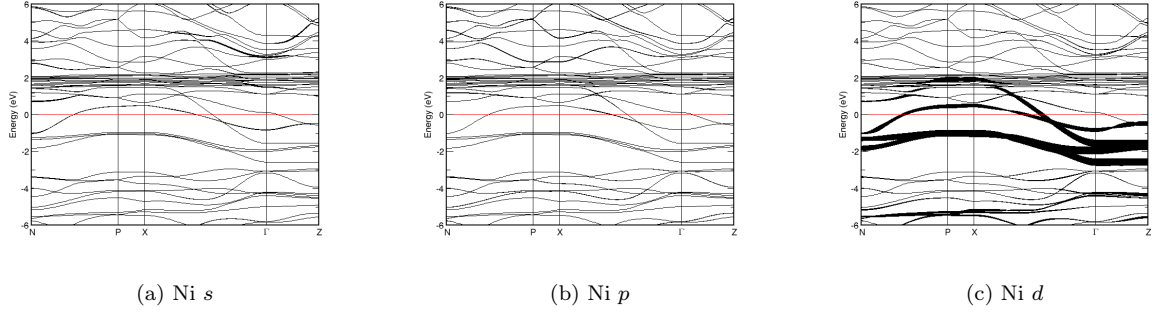FIG. 371: Fat band representation of Ni in  $\text{La}_2(\text{NiO}_4)$ 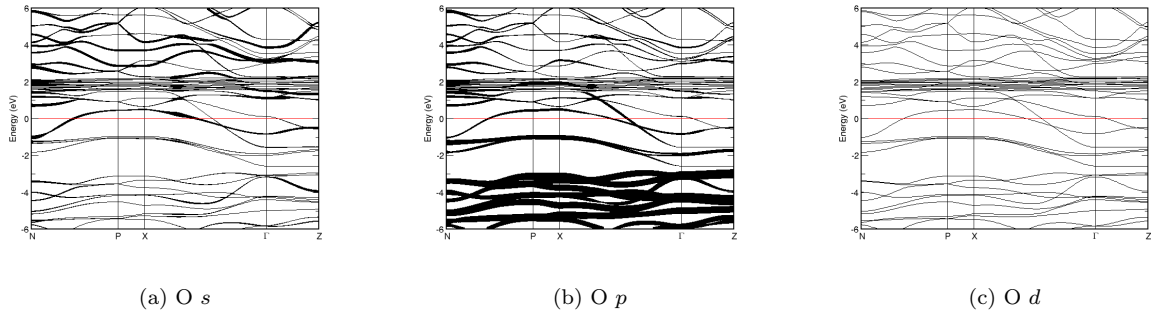FIG. 372: Fat band representation of O in  $\text{La}_2(\text{NiO}_4)$ 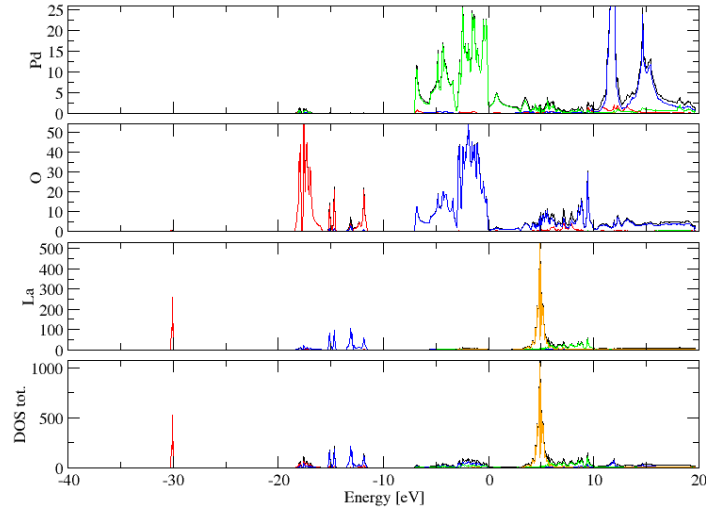FIG. 373: (Color online) PDOS of  $\text{La}_2\text{PdO}_4$  (ICSD #40262). The  $s$ -,  $p$ - and  $d$ -projected states are in red, blue and green, respectively.  $\text{La}_2\text{PdO}_4$  crystallizes in space group  $I 4/m m m$  (#139), in a tetragonal body-centred structure.

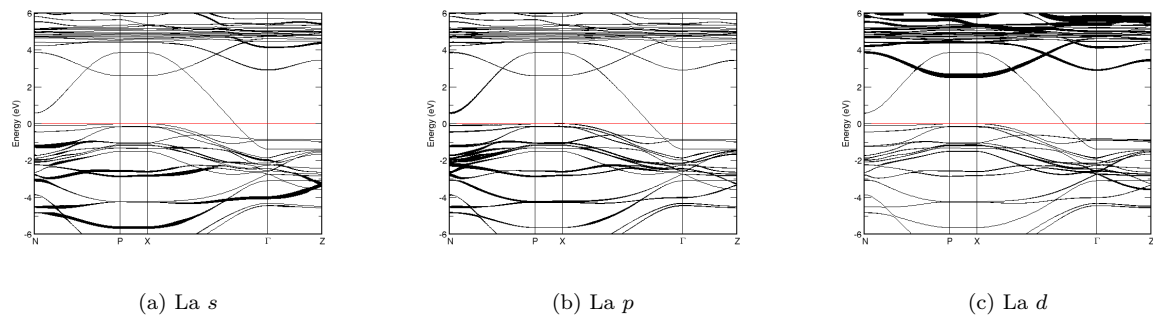FIG. 374: Fat band representation of La in  $\text{La}_2\text{PdO}_4$ 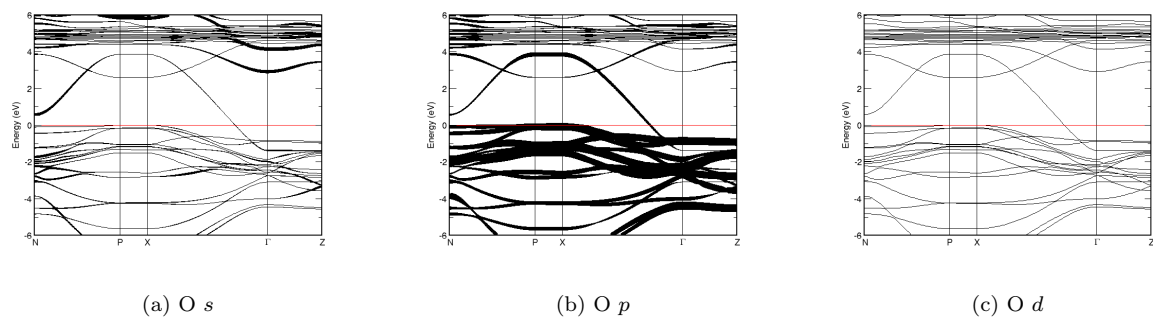FIG. 375: Fat band representation of O in  $\text{La}_2\text{PdO}_4$ 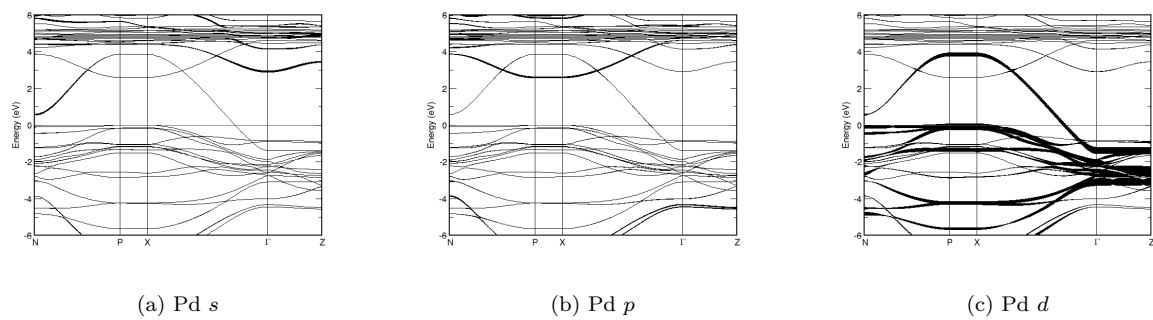FIG. 376: Fat band representation of Pd in  $\text{La}_2\text{PdO}_4$

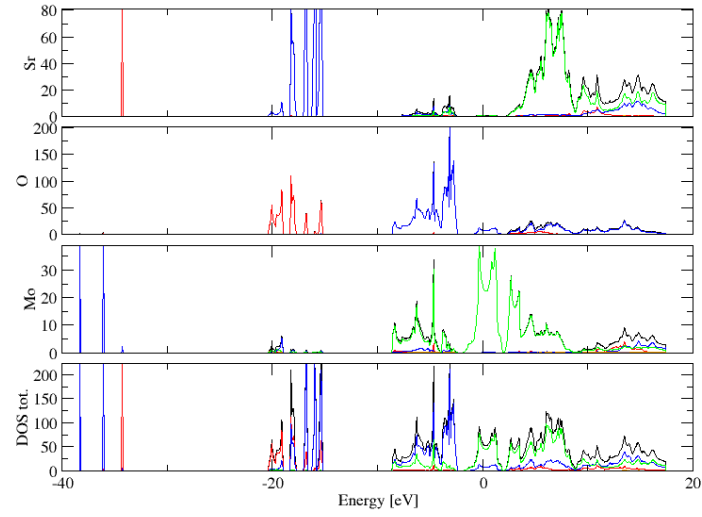

FIG. 377: (Color online) PDOS of  $\text{Sr}_2(\text{MoO}_4)$  (ICSD #152123). The  $s$ -,  $p$ - and  $d$ -projected states are in red, blue and green, respectively.  $\text{Sr}_2(\text{MoO}_4)$  crystallizes in space group  $I 4/m m m$  (#139), in a tetragonal body-centred structure.

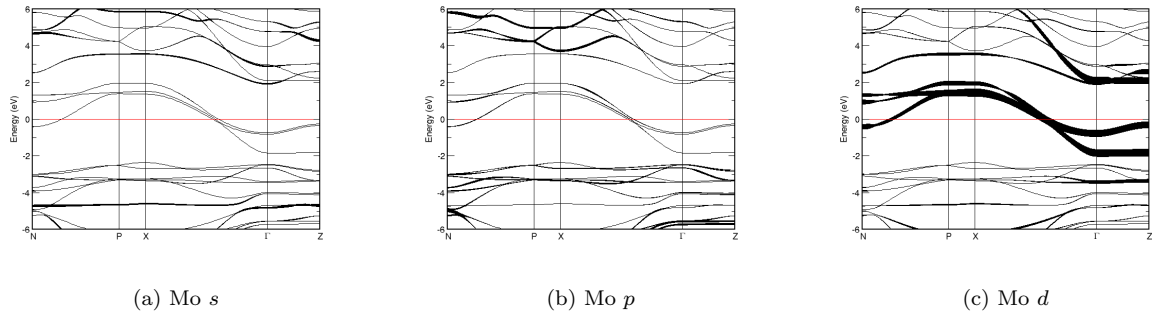

FIG. 378: Fat band representation of Mo in  $\text{Sr}_2(\text{MoO}_4)$

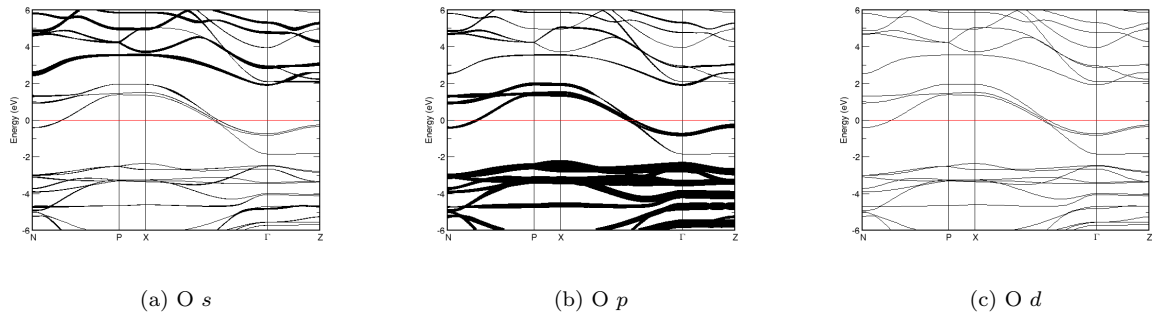

FIG. 379: Fat band representation of O in  $\text{Sr}_2(\text{MoO}_4)$

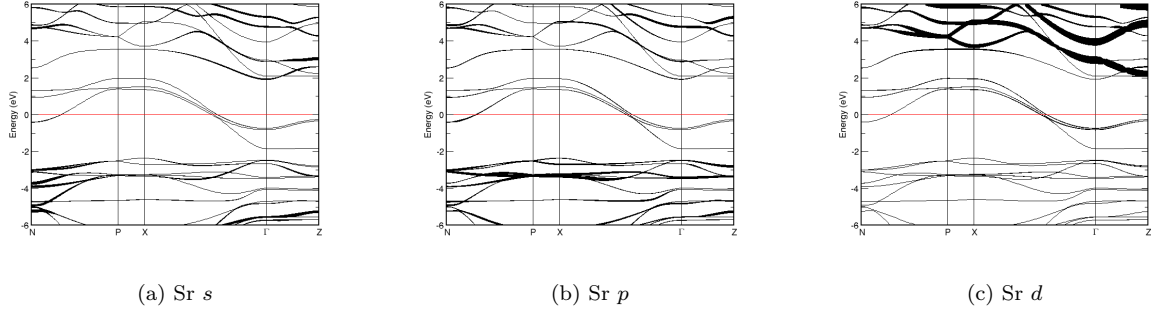

FIG. 380: Fat band representation of Sr in  $\text{Sr}_2(\text{MoO}_4)$

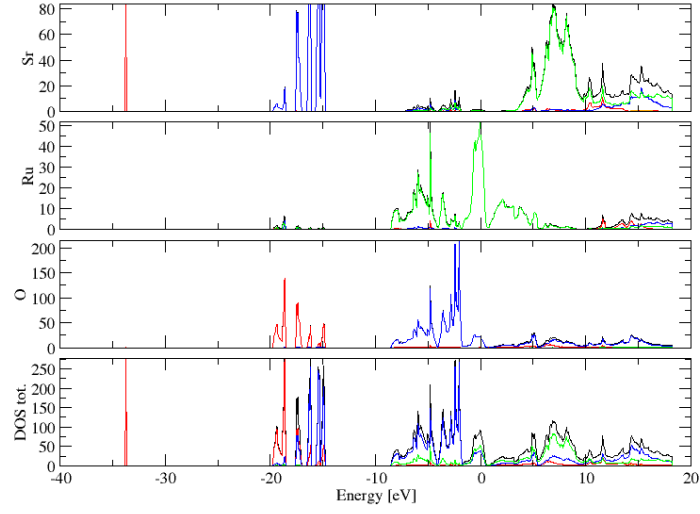

FIG. 381: (Color online) PDOS of  $\text{Sr}_2(\text{RuO}_4)$  (ICSD #157401). The *s*-, *p*- and *d*-projected states are in red, blue and green, respectively.  $\text{Sr}_2(\text{RuO}_4)$  crystallizes in space group  $I 4/m m m$  (#139), in a tetragonal body-centred structure.

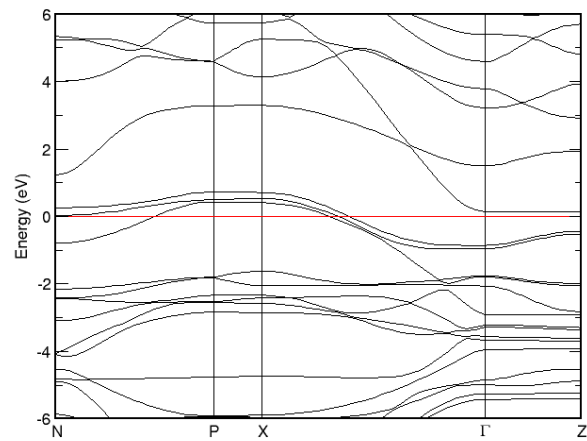(a)  $E$  vs.  $k$ FIG. 382: Band structure of  $\text{Sr}_2(\text{RuO}_4)$ 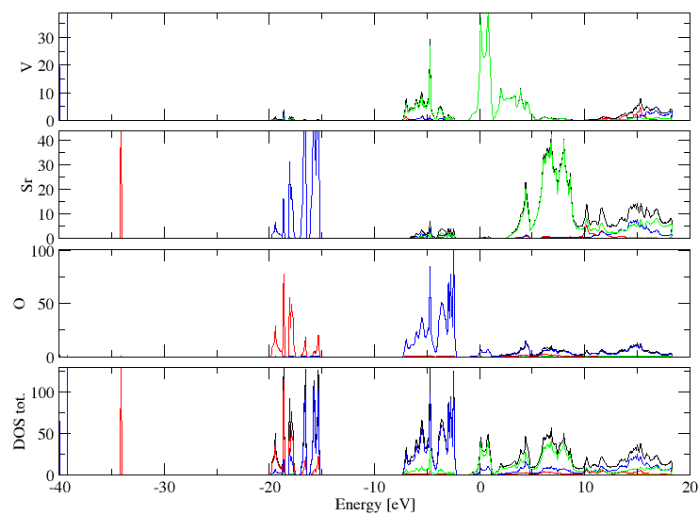

FIG. 383: (Color online) PDOS of  $\text{Sr}_2\text{VO}_4$  (ICSD #72219). The  $s$ -,  $p$ - and  $d$ -projected states are in red, blue and green, respectively.  $\text{Sr}_2\text{VO}_4$  crystallizes in space group  $I 4/m m m$  (#139), in a tetragonal body-centred structure.

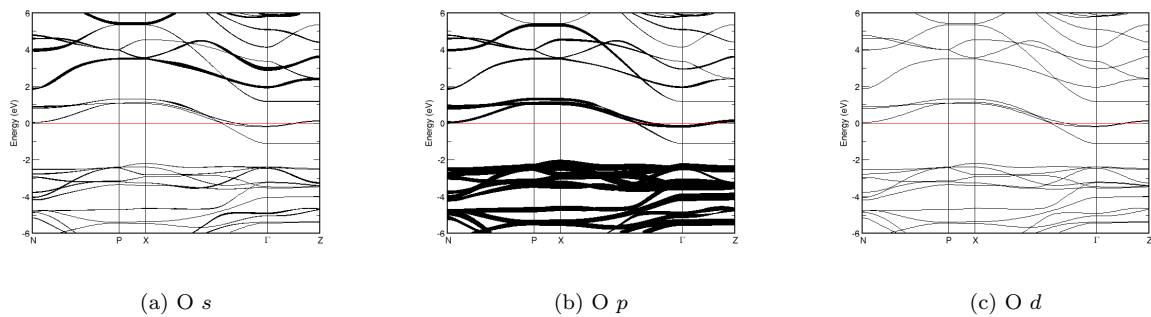(a) O  $s$ (b) O  $p$ (c) O  $d$ FIG. 384: Fat band representation of O in  $\text{Sr}_2\text{VO}_4$

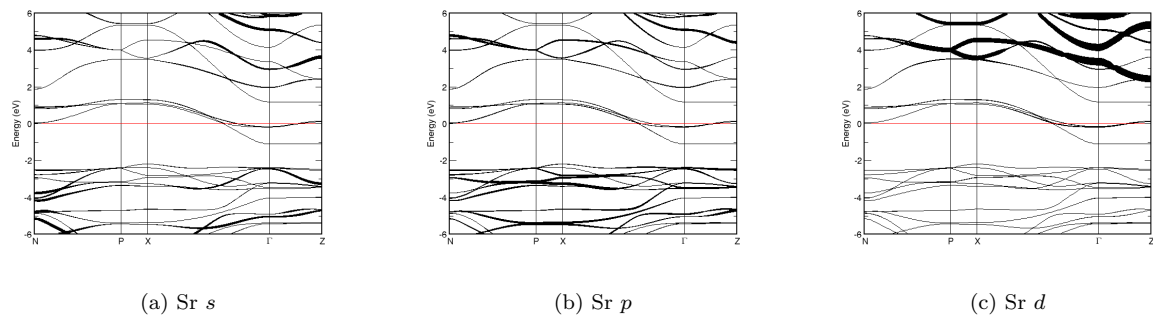FIG. 385: Fat band representation of Sr in  $\text{Sr}_2\text{VO}_4$ 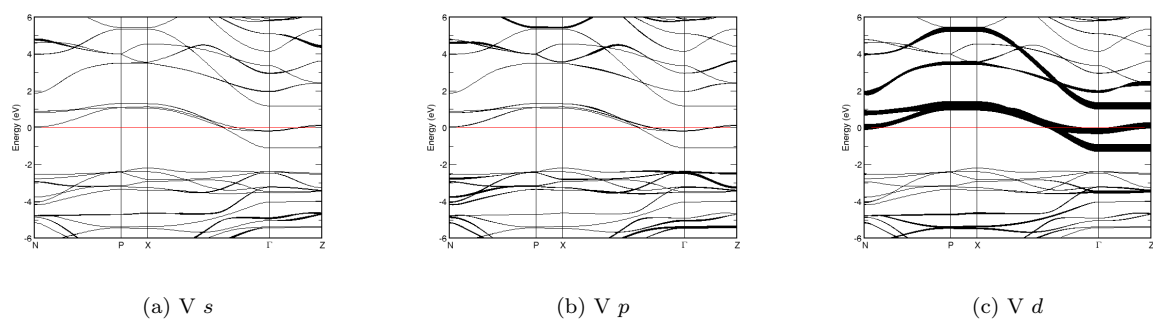FIG. 386: Fat band representation of V in  $\text{Sr}_2\text{VO}_4$ 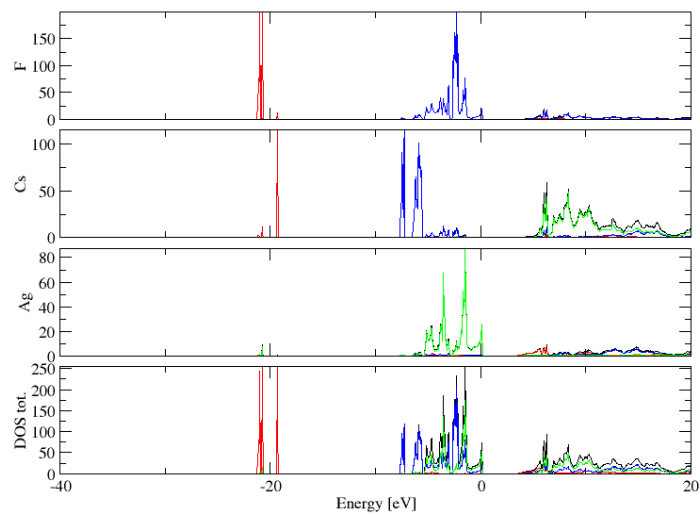FIG. 387: (Color online) PDOS of  $\text{Cs}_2\text{AgF}_4$  (ICSD #16254). The *s*-, *p*- and *d*-projected states are in red, blue and green, respectively.  $\text{Cs}_2\text{AgF}_4$  crystallizes in space group  $I 4/m m m$  (#139), in a tetragonal body-centred structure.



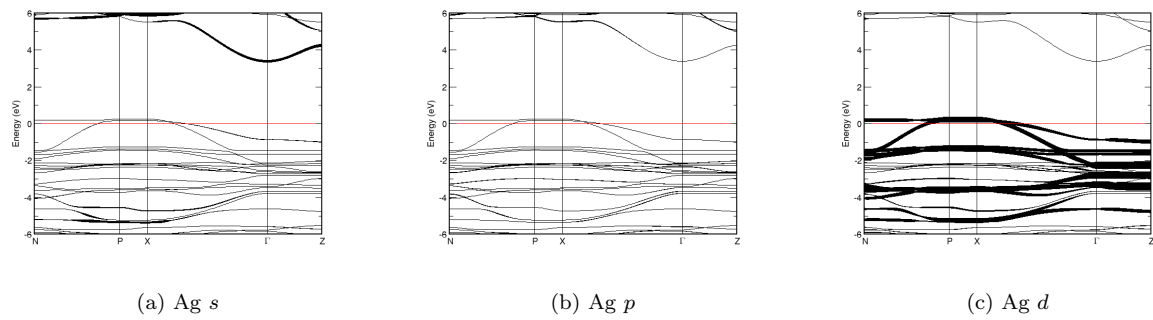FIG. 388: Fat band representation of Ag in  $\text{Cs}_2\text{AgF}_4$ 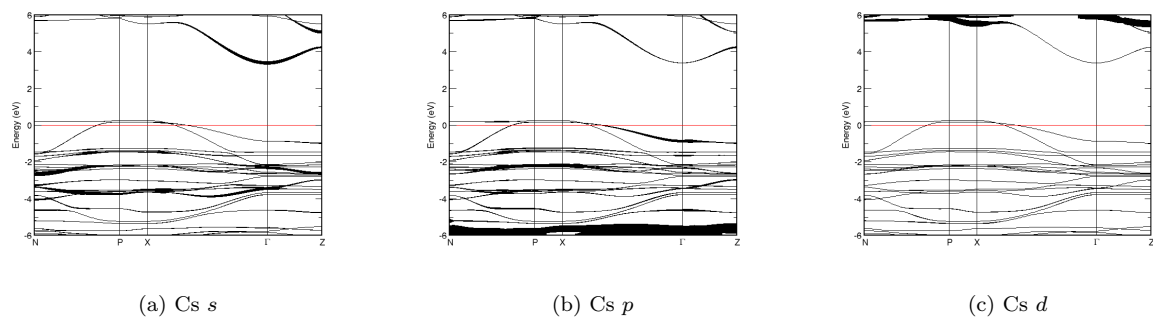FIG. 389: Fat band representation of Cs in  $\text{Cs}_2\text{AgF}_4$ 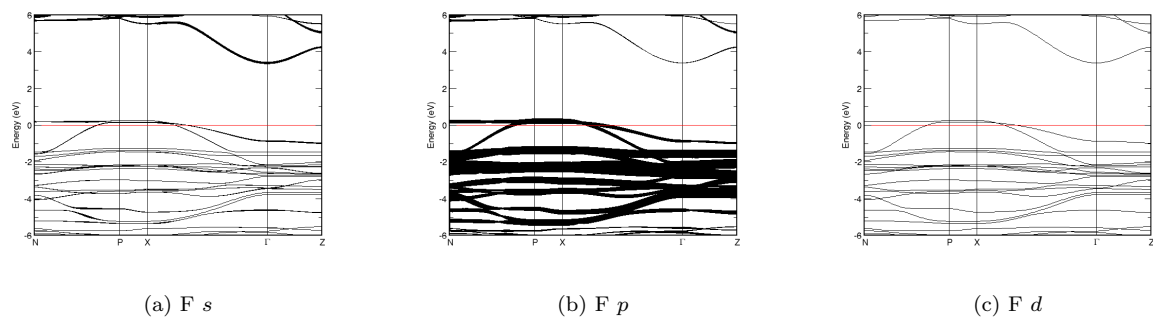FIG. 390: Fat band representation of F in  $\text{Cs}_2\text{AgF}_4$

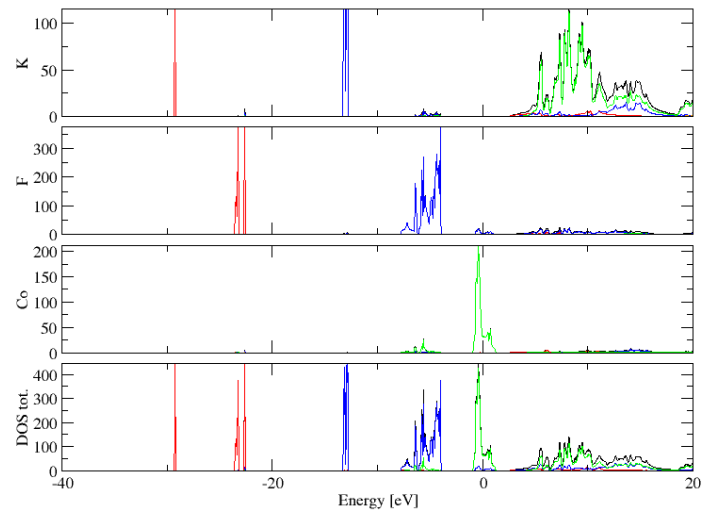

FIG. 391: (Color online) PDOS of  $\text{K}_2\text{CoF}_4$  (ICSD #33522). The  $s$ -,  $p$ - and  $d$ -projected states are in red, blue and green, respectively.  $\text{K}_2\text{CoF}_4$  crystallizes in space group  $I 4/m m m$  (#139), in a tetragonal body-centred structure.

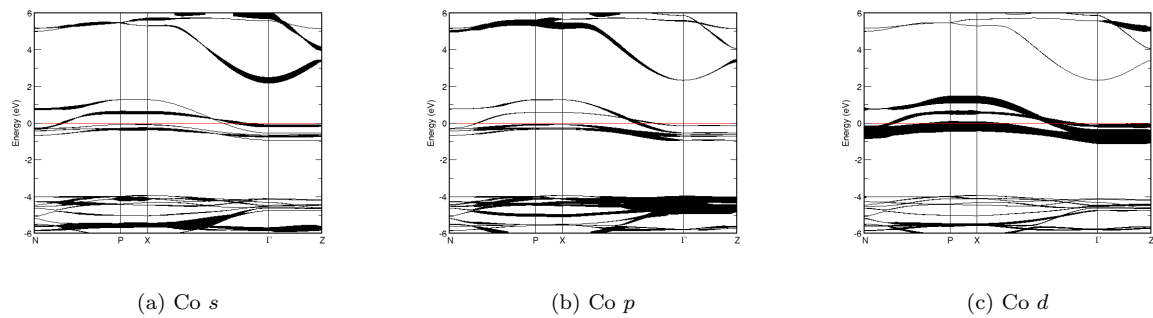

FIG. 392: Fat band representation of Co in  $\text{K}_2\text{CoF}_4$

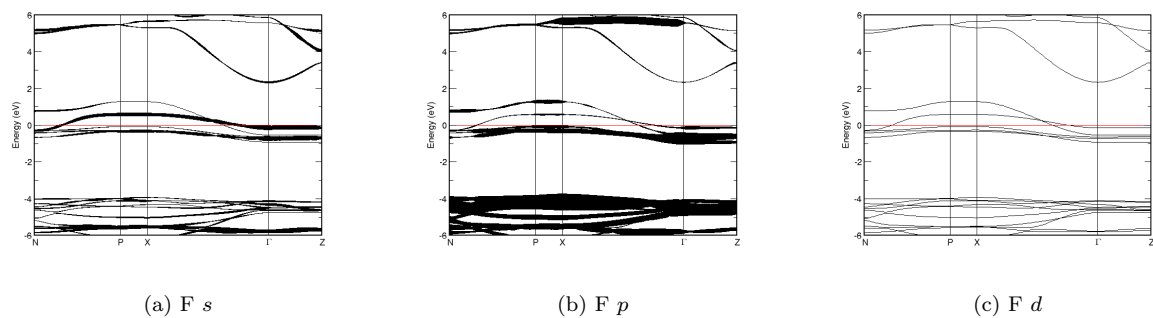

FIG. 393: Fat band representation of F in  $\text{K}_2\text{CoF}_4$

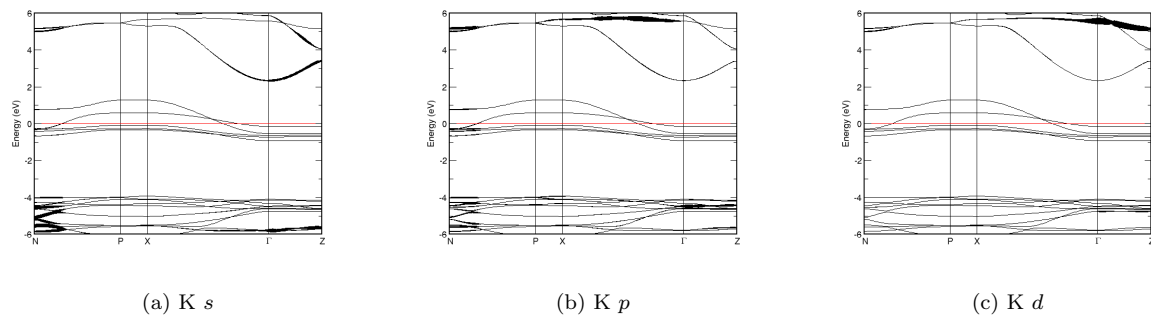FIG. 394: Fat band representation of K in  $K_2CoF_4$ 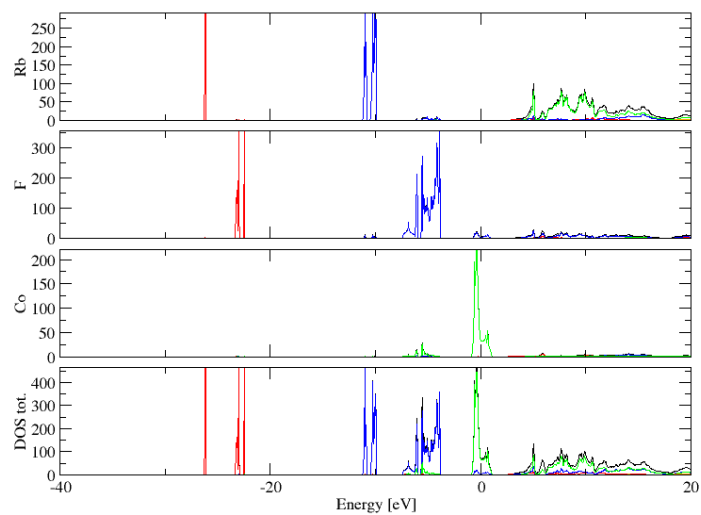FIG. 395: (Color online) PDOS of  $Rb_2CoF_4$  (ICSD #69683). The  $s$ -,  $p$ - and  $d$ -projected states are in red, blue and green, respectively.  $Rb_2CoF_4$  crystallizes in space group  $I 4/m m m$  (#139), in a tetragonal body-centred structure.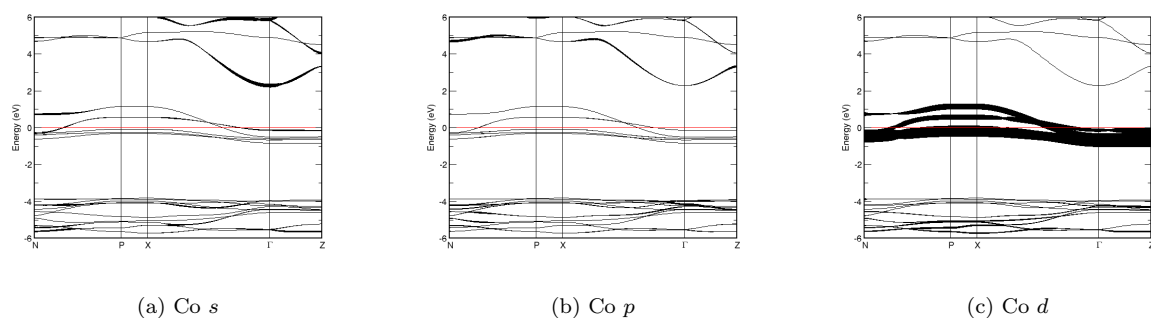FIG. 396: Fat band representation of Co in  $Rb_2CoF_4$

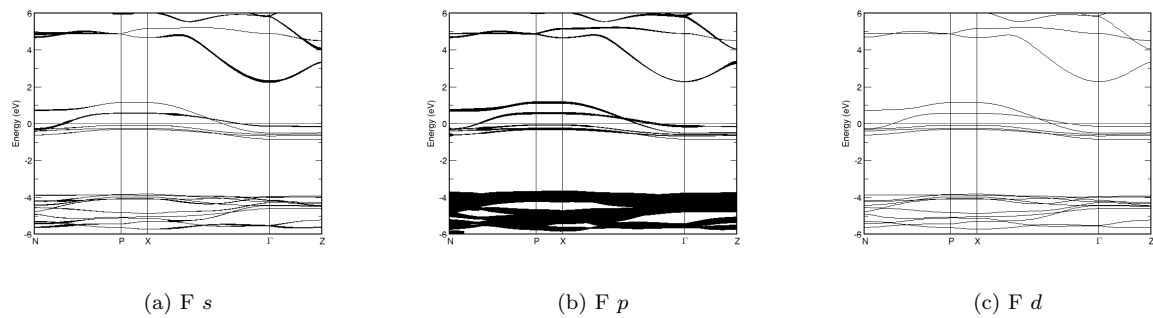FIG. 397: Fat band representation of F in  $\text{Rb}_2\text{CoF}_4$ 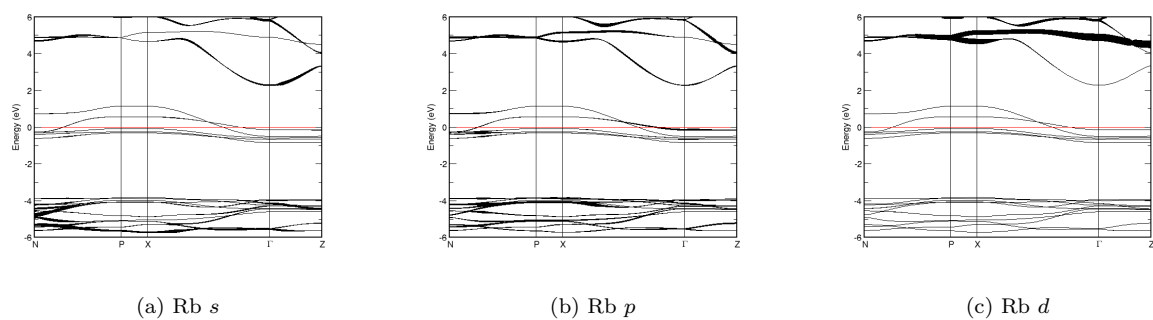FIG. 398: Fat band representation of Rb in  $\text{Rb}_2\text{CoF}_4$ 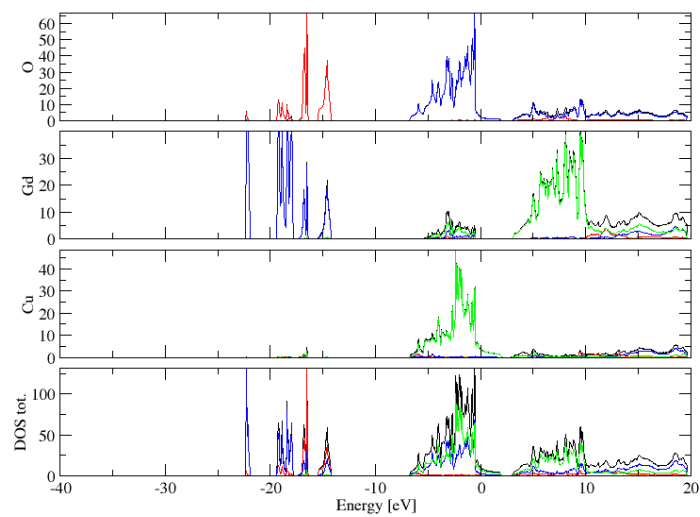

FIG. 399: (Color online) PDOS of  $\text{Gd}_2(\text{CuO}_4)$  (ICSD #41844). The *s*-, *p*- and *d*-projected states are in red, blue and green, respectively.  $\text{Gd}_2(\text{CuO}_4)$  crystallizes in space group  $I 4/m m m$  (#139), in a tetragonal body-centred structure.

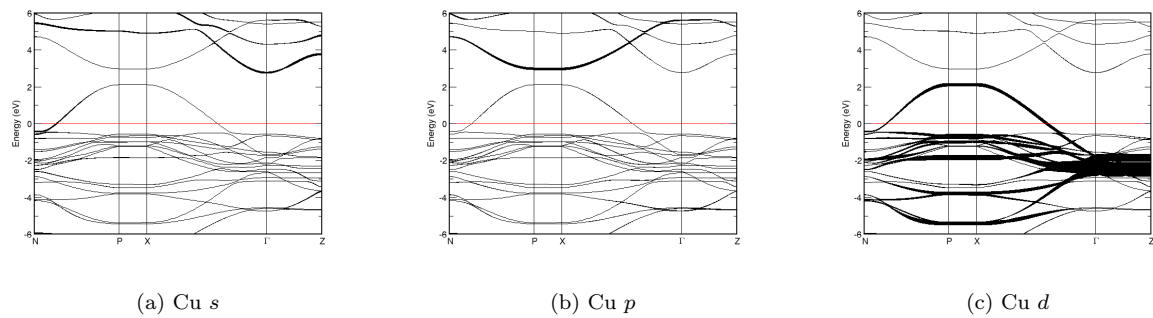FIG. 400: Fat band representation of Cu in  $\text{Gd}_2(\text{CuO}_4)$ 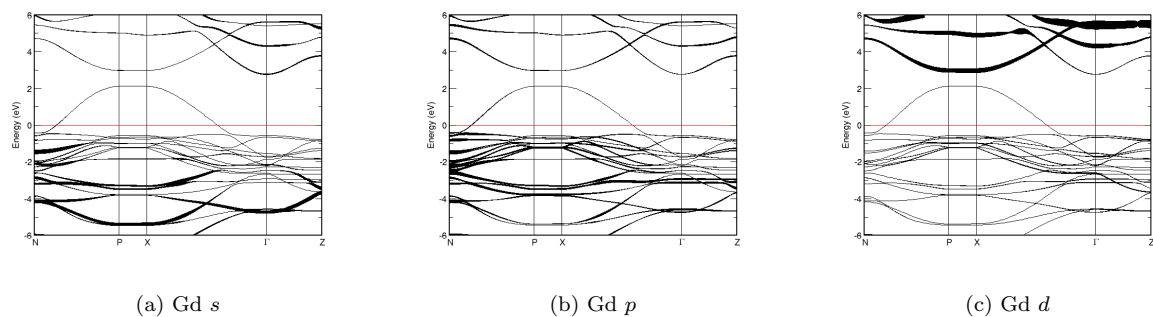FIG. 401: Fat band representation of Gd in  $\text{Gd}_2(\text{CuO}_4)$ 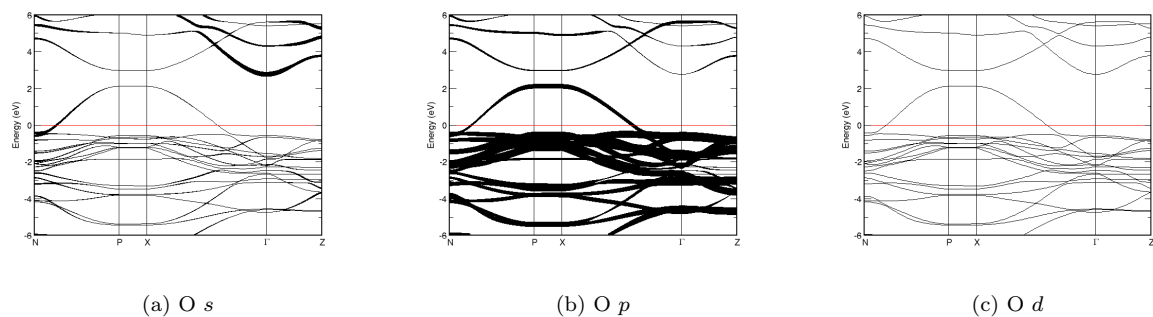FIG. 402: Fat band representation of O in  $\text{Gd}_2(\text{CuO}_4)$

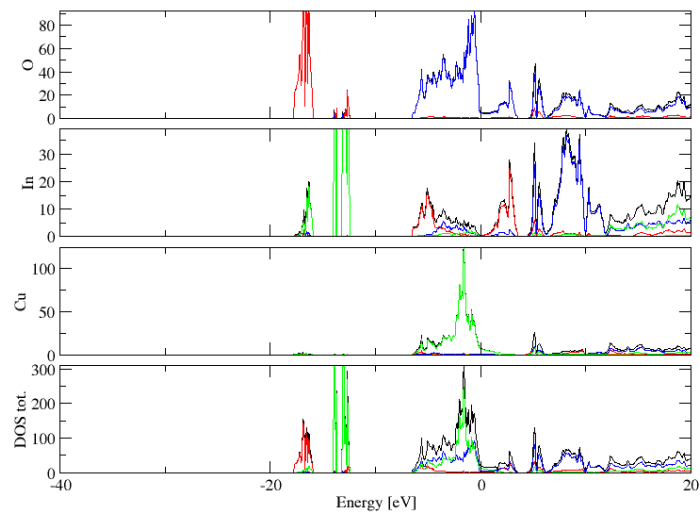

FIG. 403: (Color online) PDOS of  $\text{In}_2\text{CuO}_4$  (ICSD #39475). The  $s$ -,  $p$ - and  $d$ -projected states are in red, blue and green, respectively.  $\text{In}_2\text{CuO}_4$  crystallizes in space group  $I 4/m m m$  (#139), in a tetragonal body-centred structure.

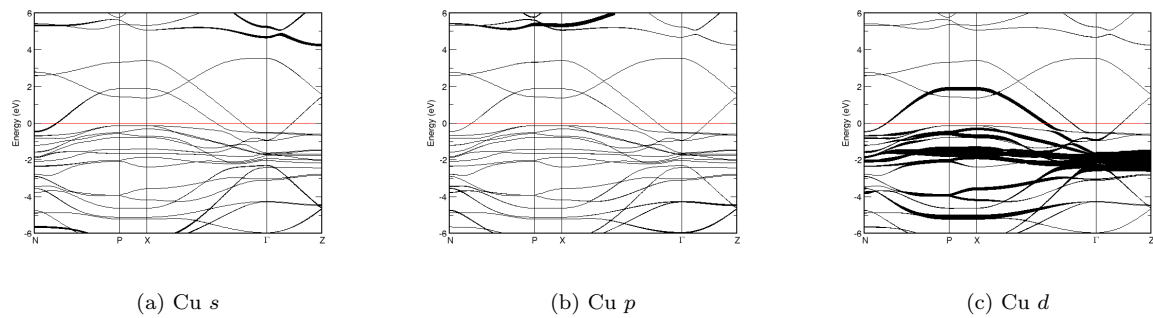

FIG. 404: Fat band representation of Cu in  $\text{In}_2\text{CuO}_4$

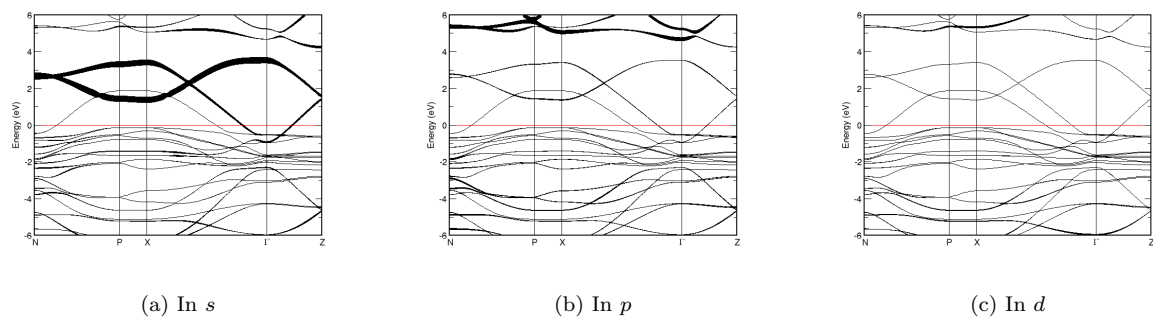

FIG. 405: Fat band representation of In in  $\text{In}_2\text{CuO}_4$

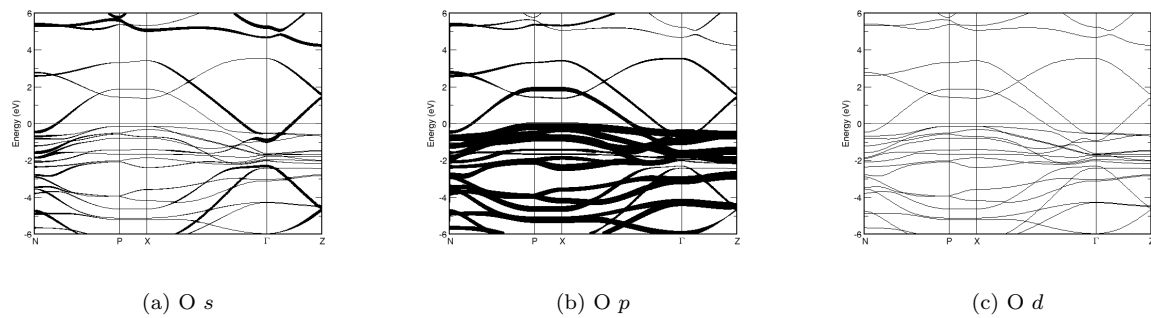FIG. 406: Fat band representation of O in  $\text{In}_2\text{CuO}_4$ 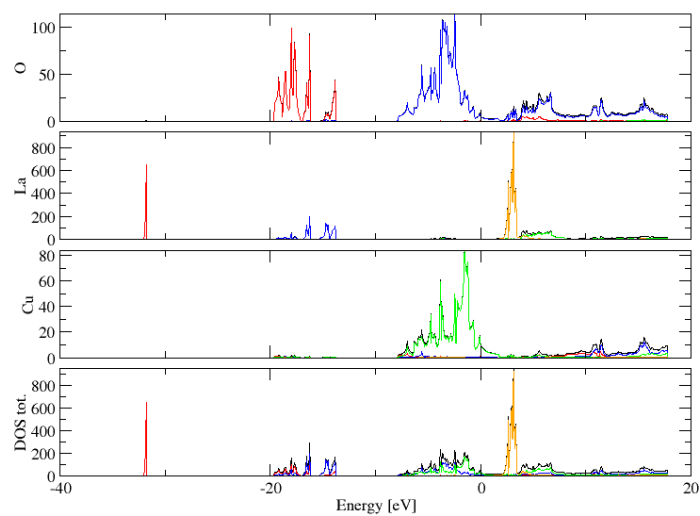FIG. 407: (Color online) PDOS of  $\text{La}_2(\text{CuO}_4)$  (ICSD #41643). The *s*-, *p*- and *d*-projected states are in red, blue and green, respectively.  $\text{La}_2(\text{CuO}_4)$  crystallizes in space group  $I 4/m m m$  (#139), in a tetragonal body-centred structure.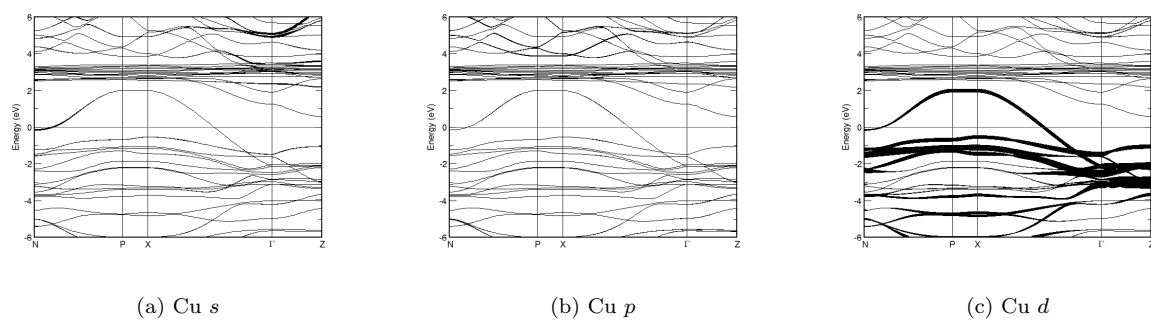FIG. 408: Fat band representation of Cu in  $\text{La}_2(\text{CuO}_4)$

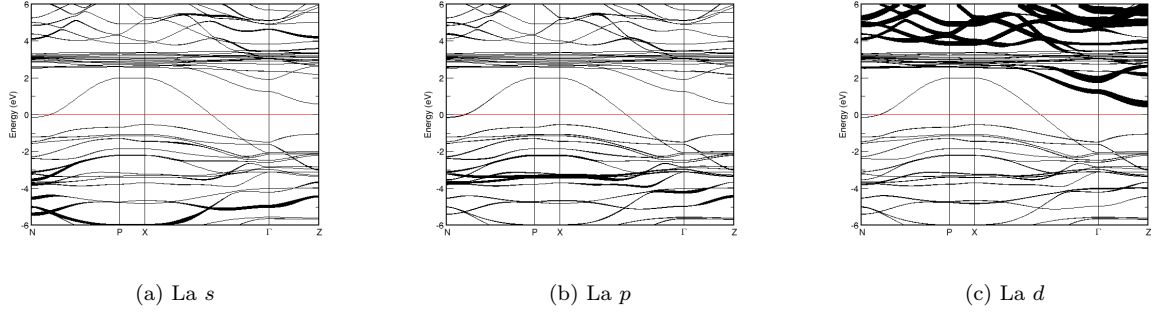FIG. 409: Fat band representation of La in  $\text{La}_2(\text{CuO}_4)$ 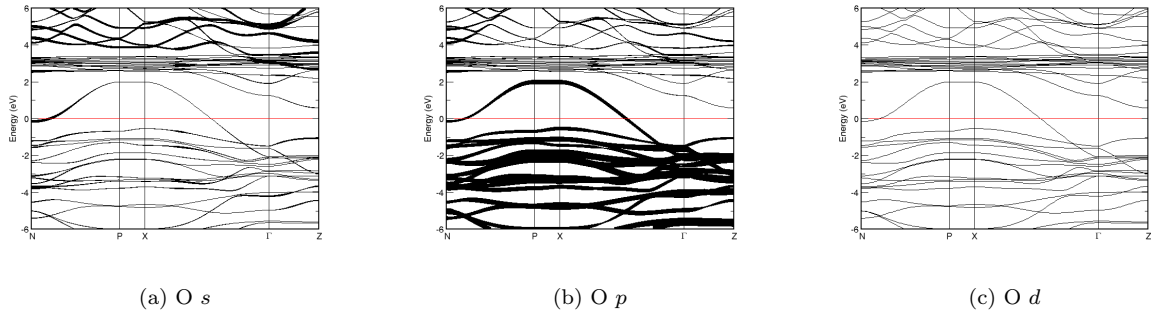FIG. 410: Fat band representation of O in  $\text{La}_2(\text{CuO}_4)$ 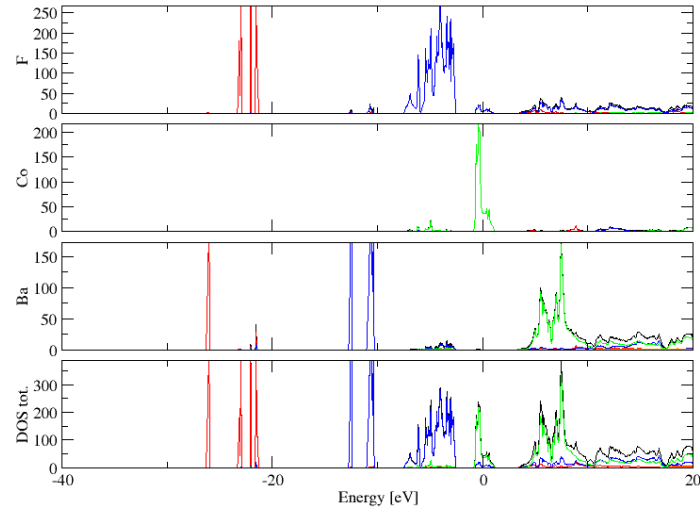FIG. 411: (Color online) PDOS of  $\text{Ba}_2\text{CoF}_6$  (ICSD #21057). The *s*-, *p*- and *d*-projected states are in red, blue and green, respectively.  $\text{Ba}_2\text{CoF}_6$  crystallizes in space group  $I 4/m m m$  (#139), in a tetragonal body-centred structure.



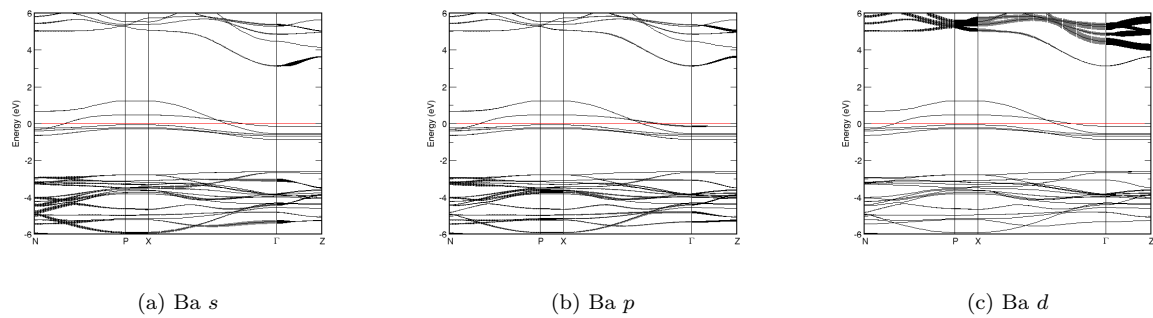FIG. 412: Fat band representation of Ba in  $\text{Ba}_2\text{CoF}_6$ 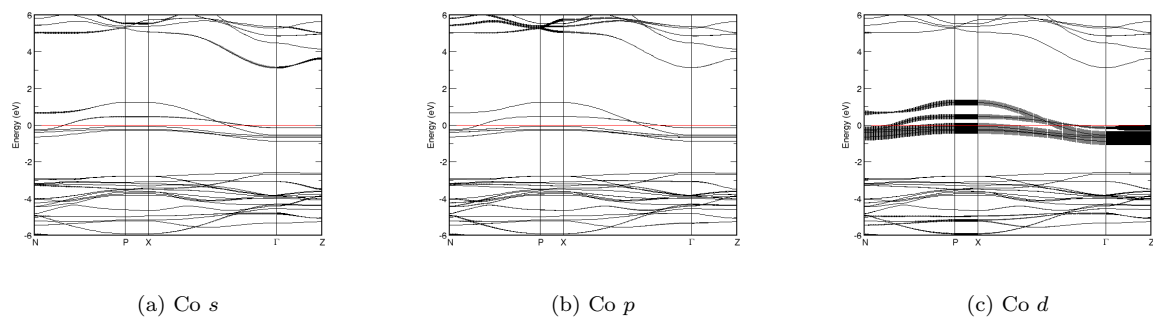FIG. 413: Fat band representation of Co in  $\text{Ba}_2\text{CoF}_6$ 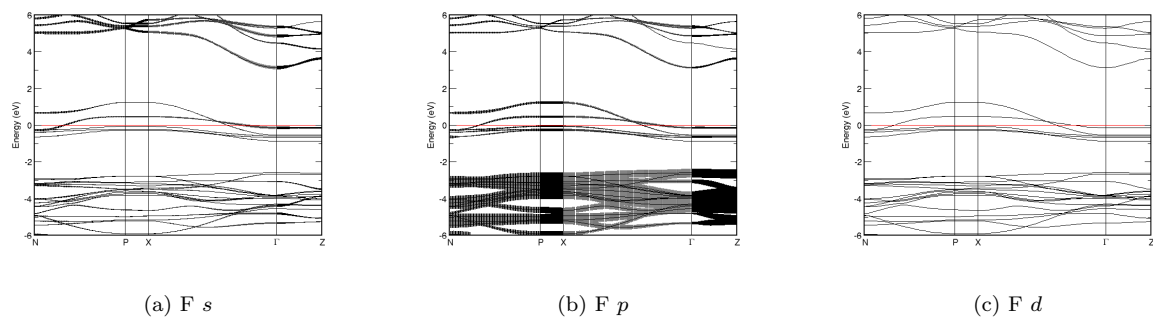FIG. 414: Fat band representation of F in  $\text{Ba}_2\text{CoF}_6$

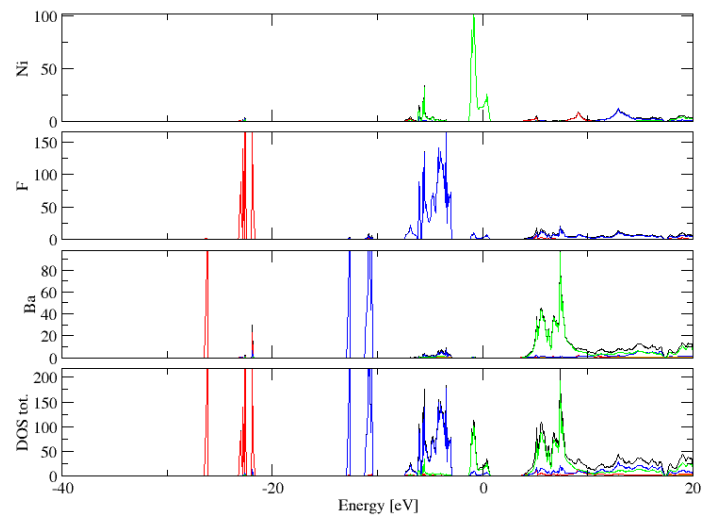

FIG. 415: (Color online) PDOS of  $\text{Ba}_2\text{NiF}_6$  (ICSD #21056). The  $s$ -,  $p$ - and  $d$ -projected states are in red, blue and green, respectively.  $\text{Ba}_2\text{NiF}_6$  crystallizes in space group  $I 4/m m m$  (#139), in a tetragonal body-centred structure.

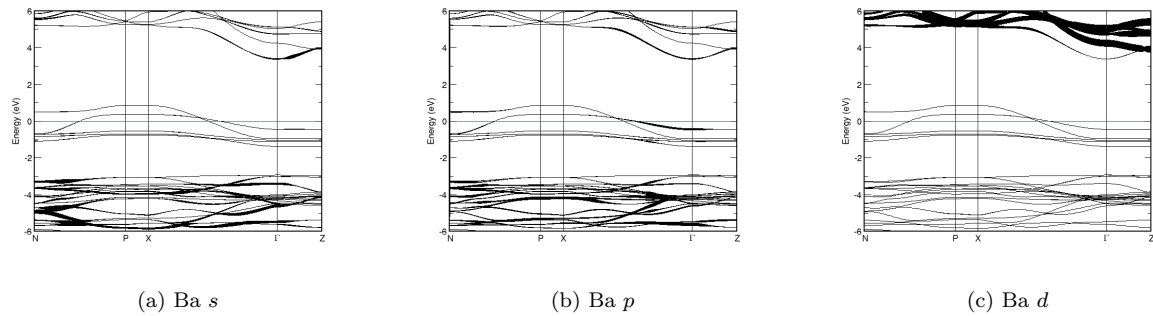

FIG. 416: Fat band representation of Ba in  $\text{Ba}_2\text{NiF}_6$

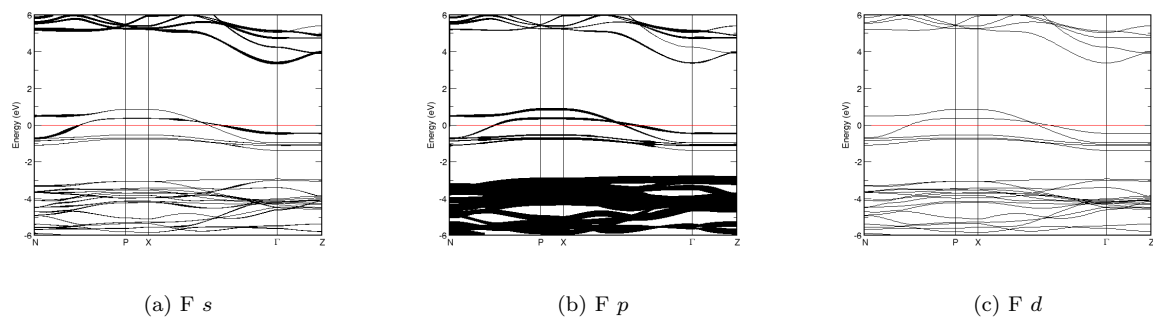

FIG. 417: Fat band representation of F in  $\text{Ba}_2\text{NiF}_6$

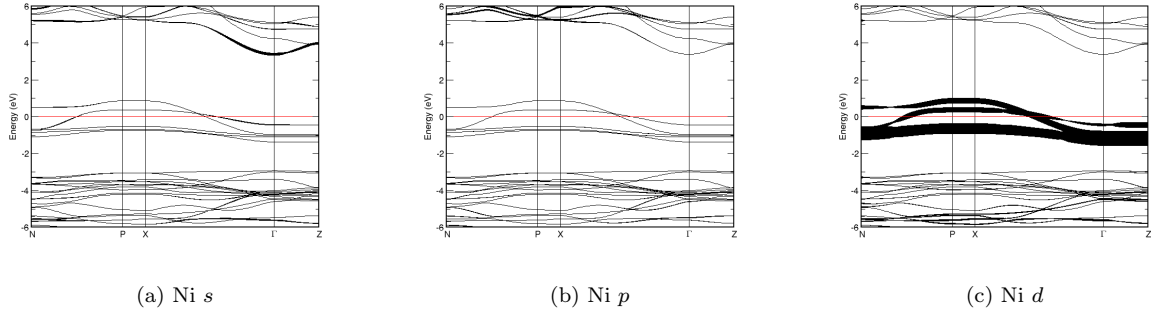FIG. 418: Fat band representation of Ni in  $\text{Ba}_2\text{NiF}_6$ 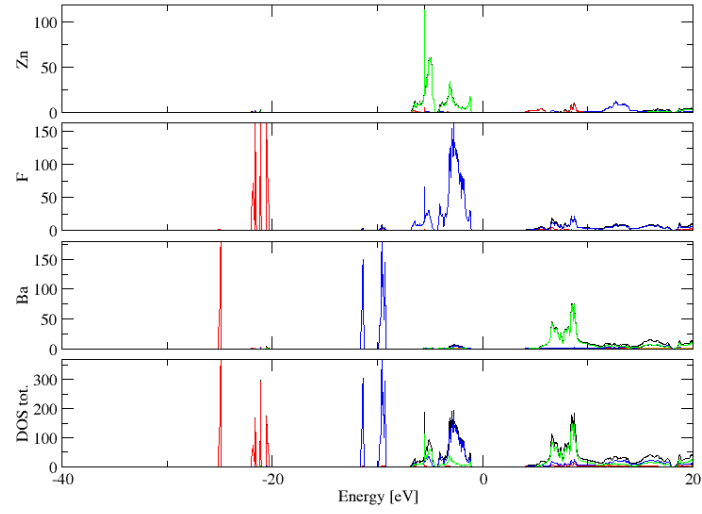FIG. 419: (Color online) PDOS of  $\text{Ba}_2(\text{ZnF}_6)$  (ICSD #21054). The  $s$ -,  $p$ - and  $d$ -projected states are in red, blue and green, respectively.  $\text{Ba}_2(\text{ZnF}_6)$  crystallizes in space group  $I 4/m m m$  (#139), in a tetragonal body-centred structure.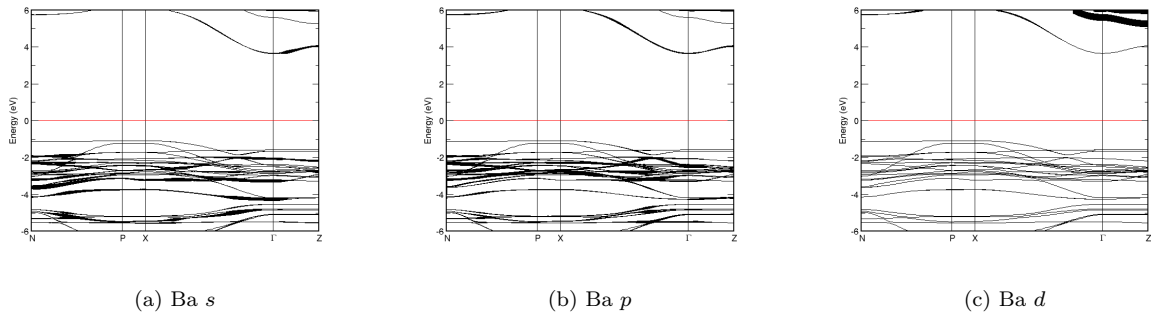FIG. 420: Fat band representation of Ba in  $\text{Ba}_2(\text{ZnF}_6)$

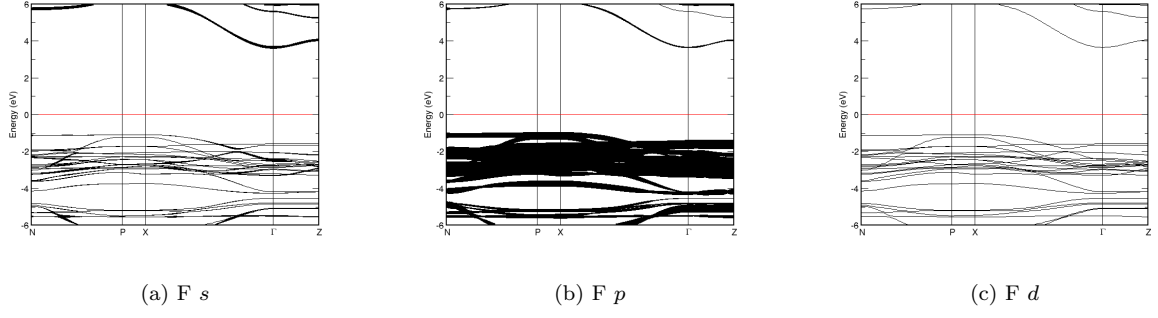FIG. 421: Fat band representation of F in  $\text{Ba}_2(\text{ZnF}_6)$ 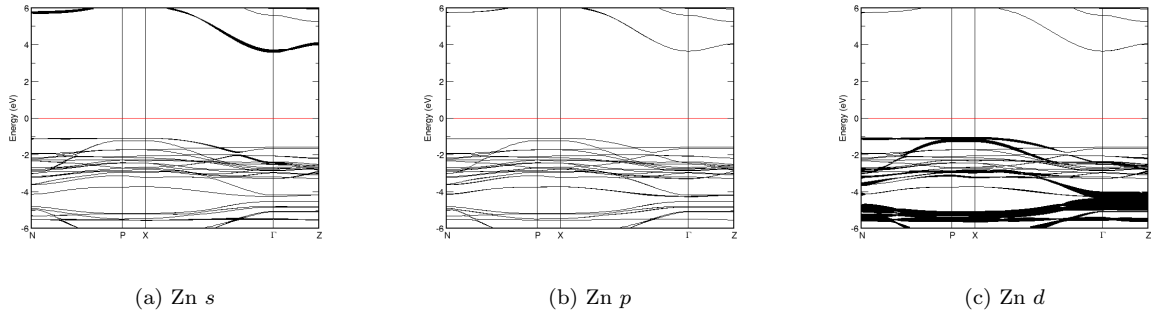FIG. 422: Fat band representation of Zn in  $\text{Ba}_2(\text{ZnF}_6)$ 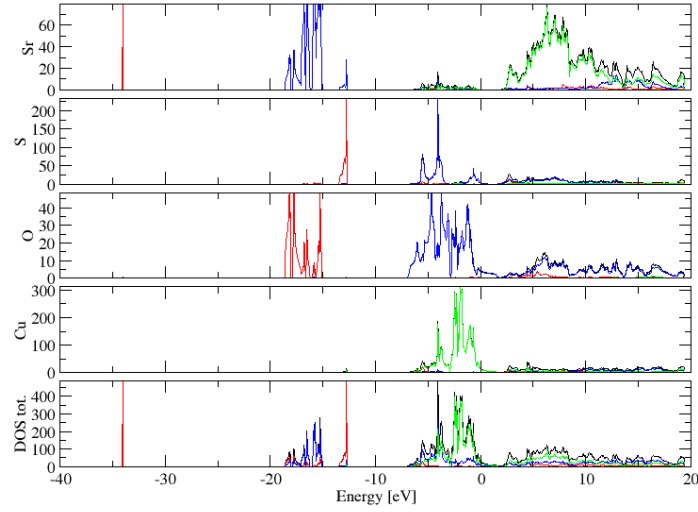

FIG. 423: (Color online) PDOS of  $(\text{Cu}_2\text{S}_2)(\text{Sr}_2\text{CuO}_2)$  (ICSD #88423). The *s*-, *p*- and *d*-projected states are in red, blue and green, respectively.  $(\text{Cu}_2\text{S}_2)(\text{Sr}_2\text{CuO}_2)$  crystallizes in space group  $I 4/m m m$  (#139), in a tetragonal body-centred structure.

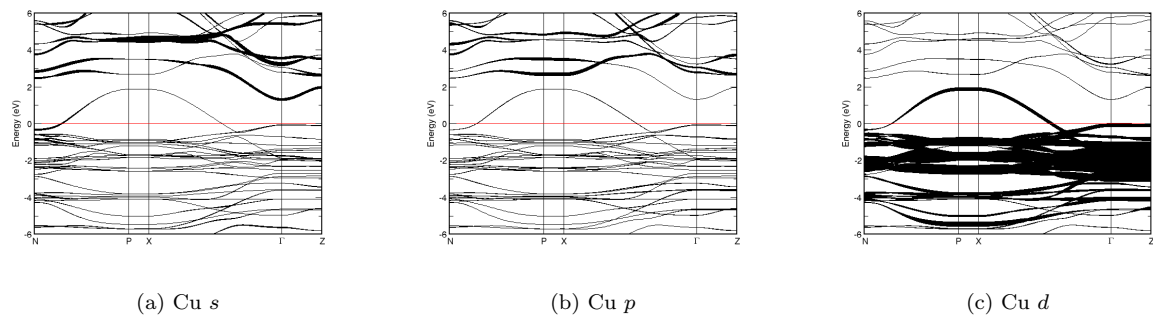FIG. 424: Fat band representation of Cu in  $(\text{Cu}_2\text{S}_2)(\text{Sr}_2\text{CuO}_2)$ 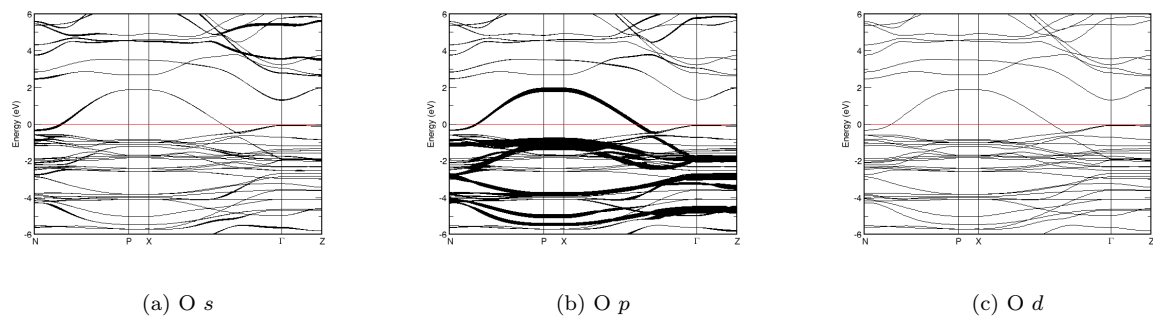FIG. 425: Fat band representation of O in  $(\text{Cu}_2\text{S}_2)(\text{Sr}_2\text{CuO}_2)$ 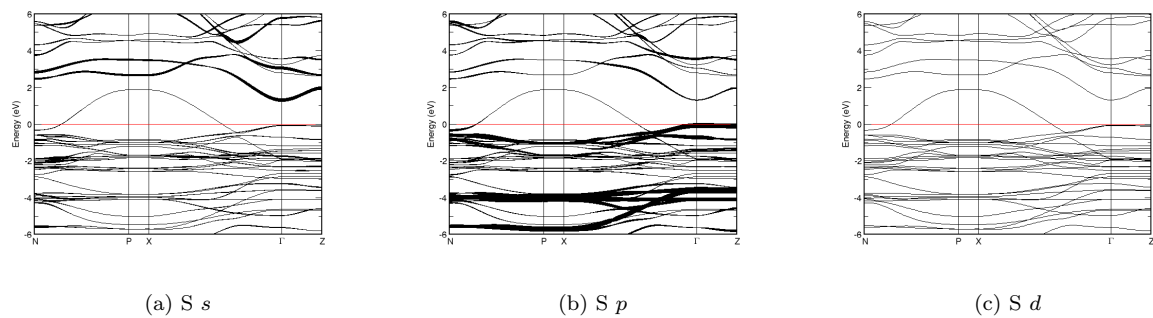FIG. 426: Fat band representation of S in  $(\text{Cu}_2\text{S}_2)(\text{Sr}_2\text{CuO}_2)$ 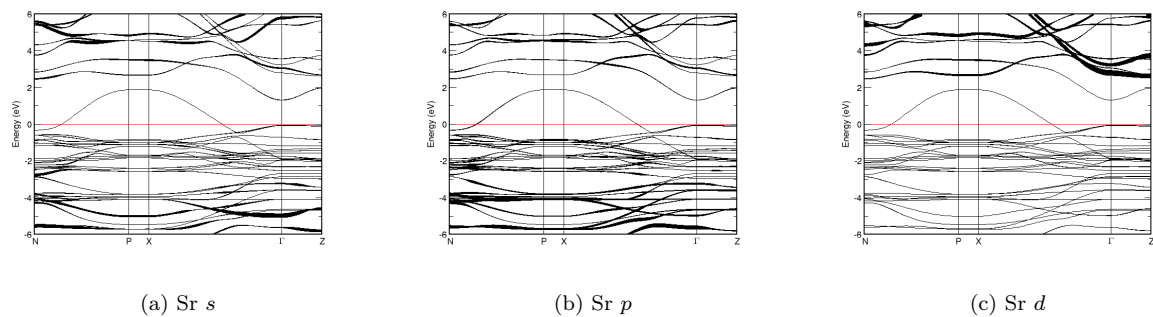FIG. 427: Fat band representation of Sr in  $(\text{Cu}_2\text{S}_2)(\text{Sr}_2\text{CuO}_2)$

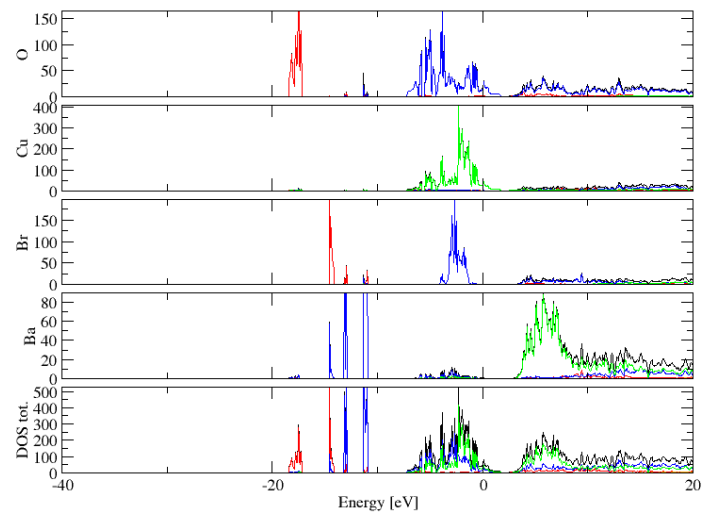

FIG. 428: (Color online) PDOS of  $\text{Ba}_2\text{Cu}_3\text{O}_4\text{Br}_2$  (ICSD #36128). The  $s$ -,  $p$ - and  $d$ -projected states are in red, blue and green, respectively.  $\text{Ba}_2\text{Cu}_3\text{O}_4\text{Br}_2$  crystallizes in space group I  $4/m\ m\ m$  (#139), in a tetragonal body-centred structure.

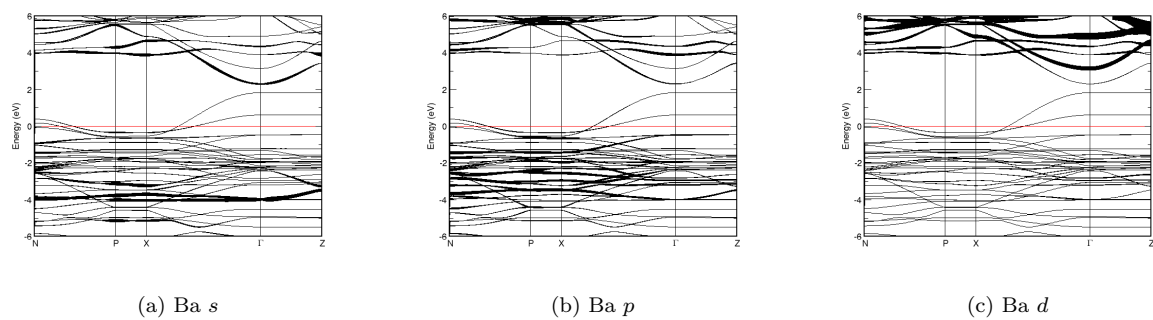

FIG. 429: Fat band representation of Ba in  $\text{Ba}_2\text{Cu}_3\text{O}_4\text{Br}_2$

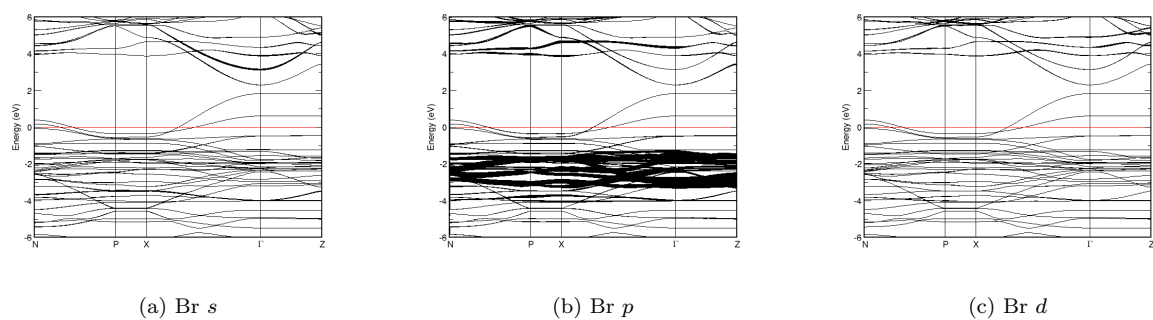

FIG. 430: Fat band representation of Br in  $\text{Ba}_2\text{Cu}_3\text{O}_4\text{Br}_2$

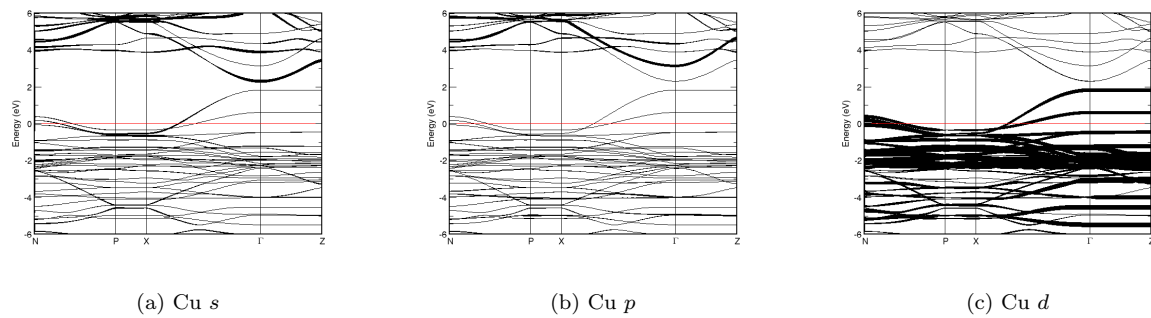FIG. 431: Fat band representation of Cu in  $\text{Ba}_2\text{Cu}_3\text{O}_4\text{Br}_2$ 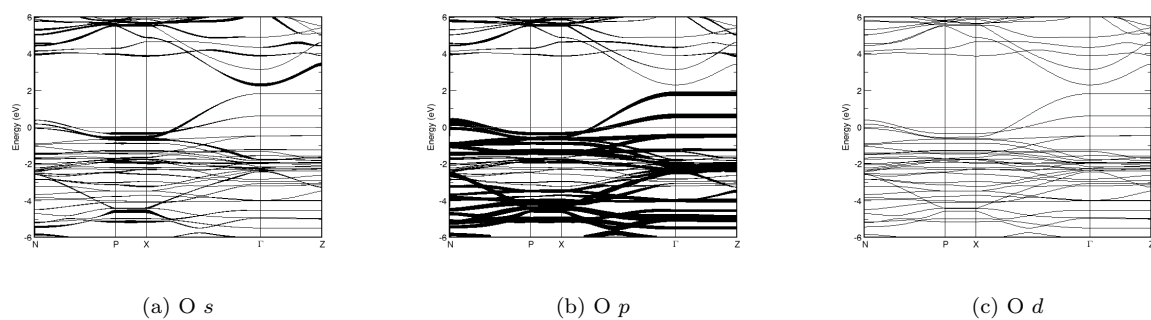FIG. 432: Fat band representation of O in  $\text{Ba}_2\text{Cu}_3\text{O}_4\text{Br}_2$ 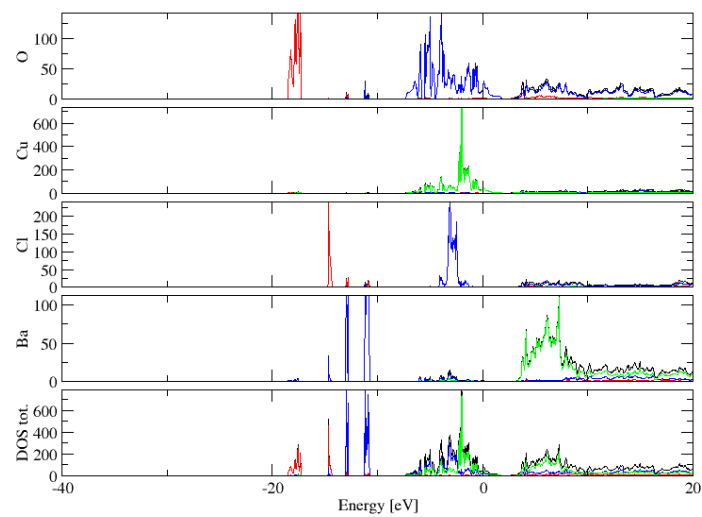

FIG. 433: (Color online) PDOS of  $\text{Ba}_2\text{Cu}_3\text{O}_4\text{Cl}_2$  (ICSD #355). The  $s$ -,  $p$ - and  $d$ -projected states are in red, blue and green, respectively.  $\text{Ba}_2\text{Cu}_3\text{O}_4\text{Cl}_2$  crystallizes in space group  $I 4/m m m$  (#139), in a tetragonal body-centred structure.

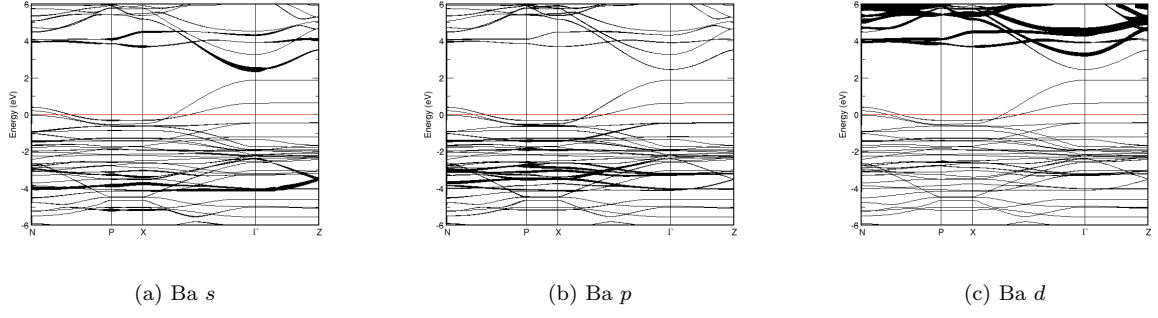FIG. 434: Fat band representation of Ba in  $\text{Ba}_2\text{Cu}_3\text{O}_4\text{Cl}_2$ 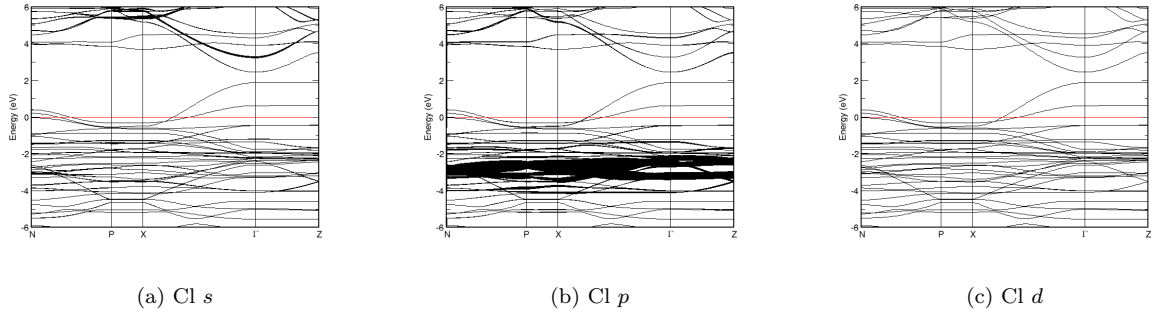FIG. 435: Fat band representation of Cl in  $\text{Ba}_2\text{Cu}_3\text{O}_4\text{Cl}_2$ 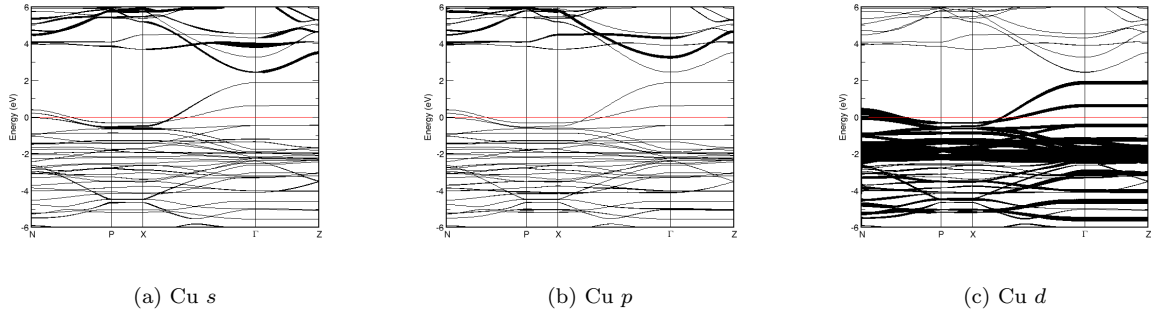FIG. 436: Fat band representation of Cu in  $\text{Ba}_2\text{Cu}_3\text{O}_4\text{Cl}_2$ 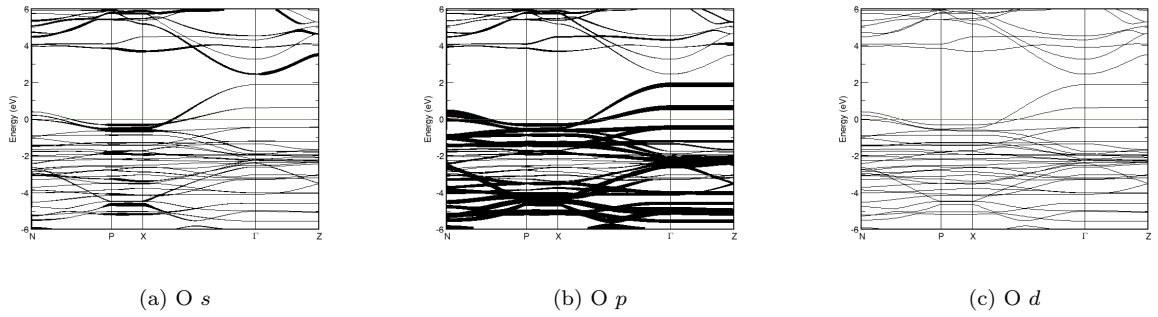FIG. 437: Fat band representation of O in  $\text{Ba}_2\text{Cu}_3\text{O}_4\text{Cl}_2$



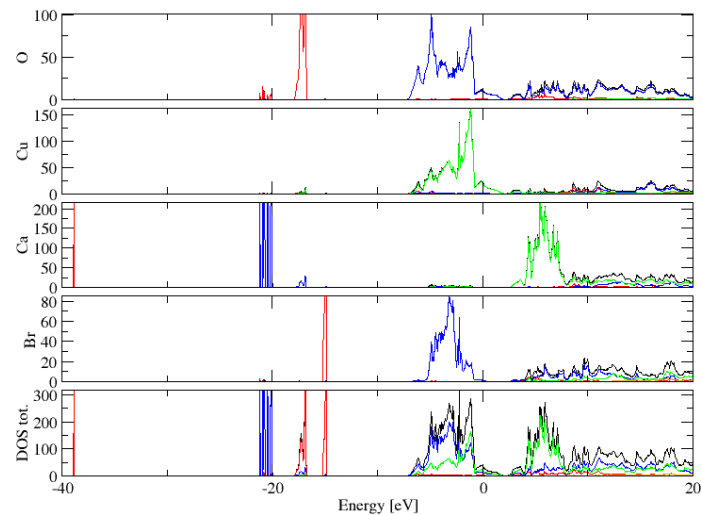

FIG. 438: (Color online) PDOS of  $\text{Ca}_3\text{Cu}_2\text{O}_4\text{Br}_2$  (ICSD #69182). The  $s$ -,  $p$ - and  $d$ -projected states are in red, blue and green, respectively.  $\text{Ca}_3\text{Cu}_2\text{O}_4\text{Br}_2$  crystallizes in space group  $I 4/m m m$  (#139), in a tetragonal body-centred structure.

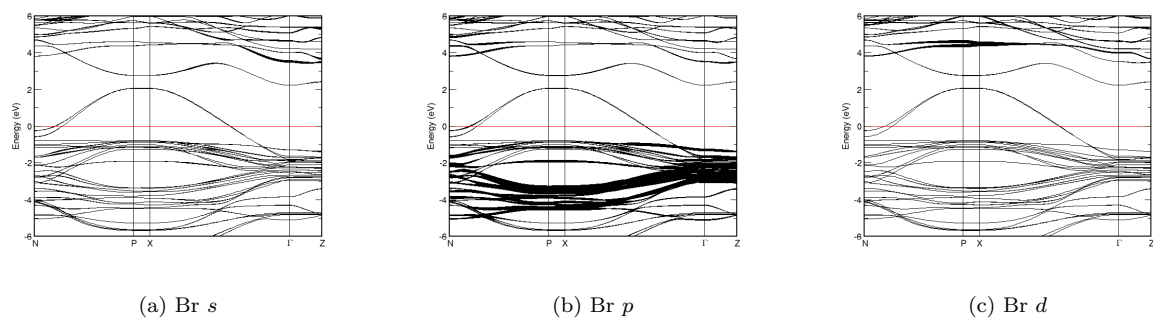

FIG. 439: Fat band representation of Br in  $\text{Ca}_3\text{Cu}_2\text{O}_4\text{Br}_2$

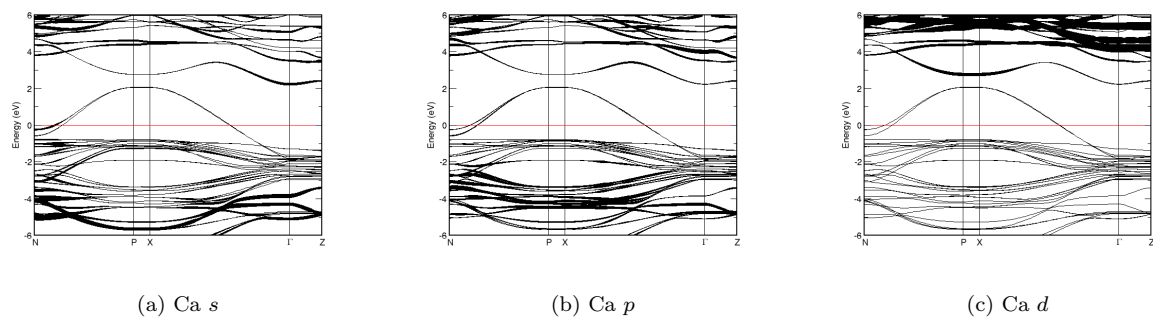

FIG. 440: Fat band representation of Ca in  $\text{Ca}_3\text{Cu}_2\text{O}_4\text{Br}_2$

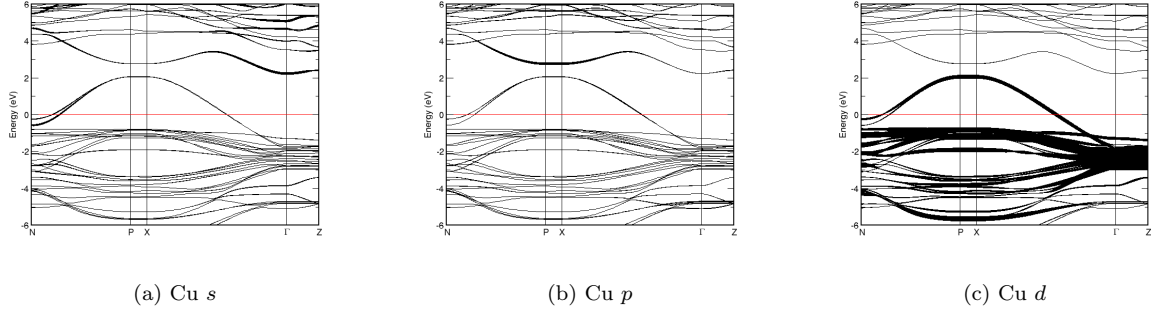FIG. 441: Fat band representation of Cu in  $\text{Ca}_3\text{Cu}_2\text{O}_4\text{Br}_2$ 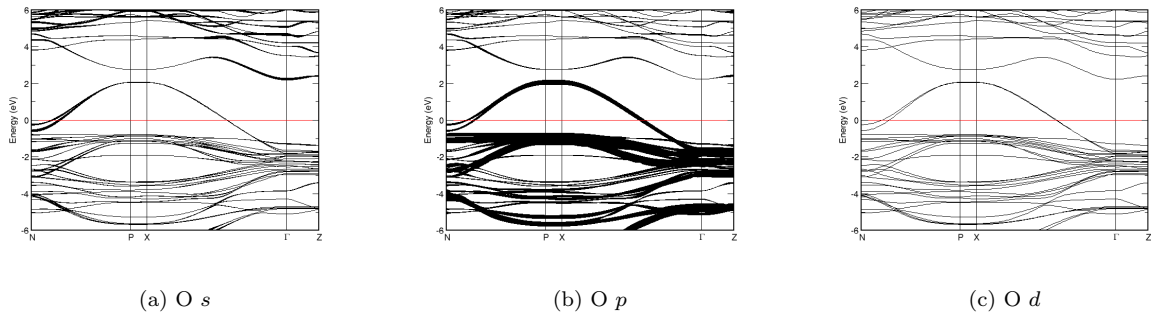FIG. 442: Fat band representation of O in  $\text{Ca}_3\text{Cu}_2\text{O}_4\text{Br}_2$ 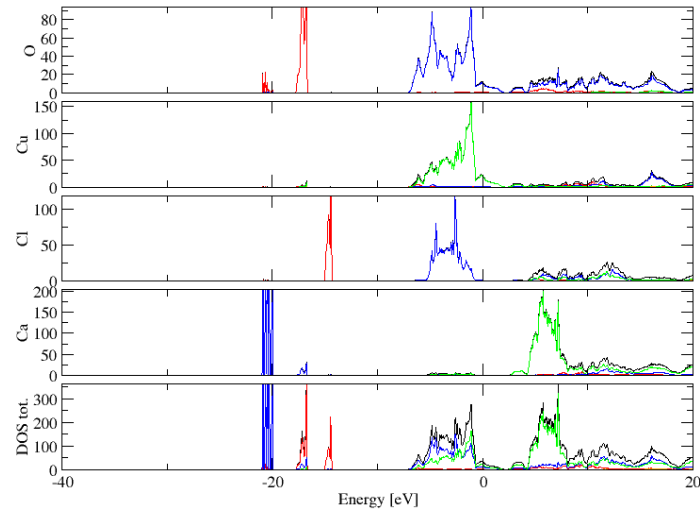

FIG. 443: (Color online) PDOS of  $\text{Ca}_3\text{Cu}_2\text{O}_4\text{Cl}_2$  (ICSD #69181). The *s*-, *p*- and *d*-projected states are in red, blue and green, respectively.  $\text{Ca}_3\text{Cu}_2\text{O}_4\text{Cl}_2$  crystallizes in space group  $I 4/m m m$  (#139), in a tetragonal body-centred structure.

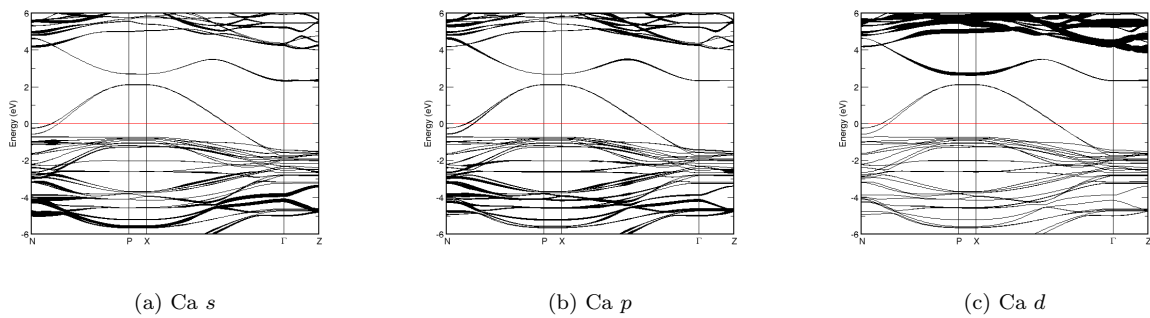FIG. 444: Fat band representation of Ca in  $\text{Ca}_3\text{Cu}_2\text{O}_4\text{Cl}_2$ 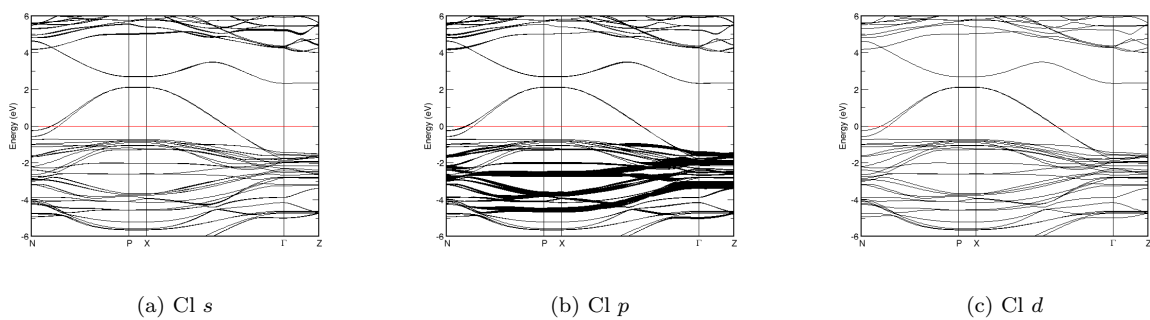FIG. 445: Fat band representation of Cl in  $\text{Ca}_3\text{Cu}_2\text{O}_4\text{Cl}_2$ 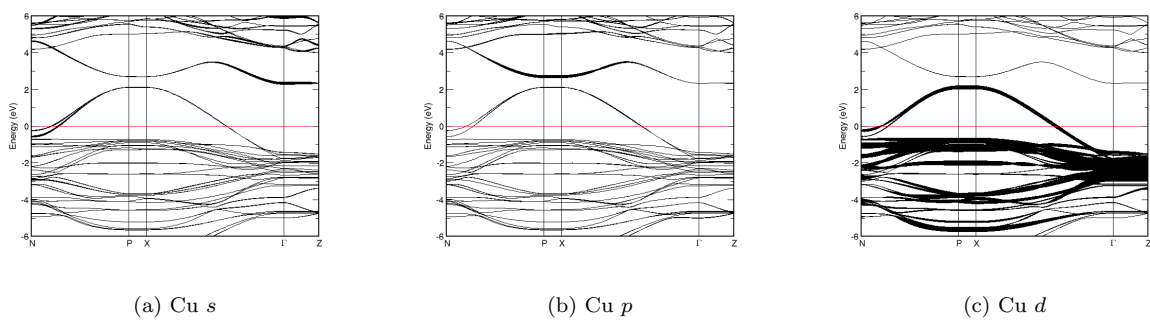FIG. 446: Fat band representation of Cu in  $\text{Ca}_3\text{Cu}_2\text{O}_4\text{Cl}_2$ 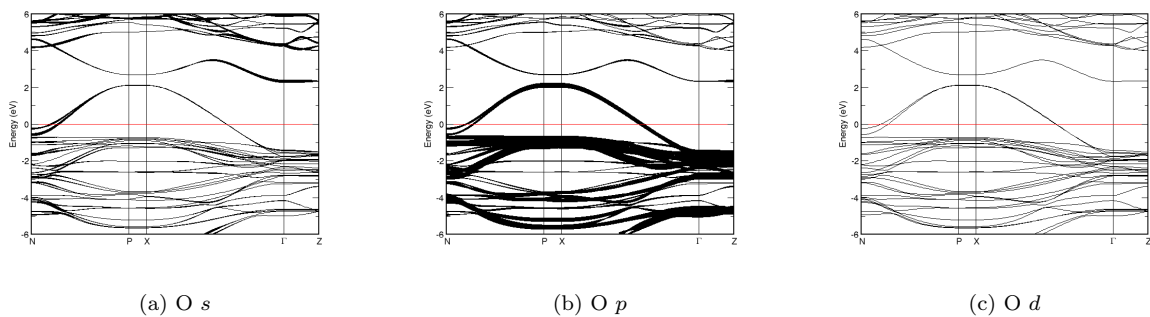FIG. 447: Fat band representation of O in  $\text{Ca}_3\text{Cu}_2\text{O}_4\text{Cl}_2$

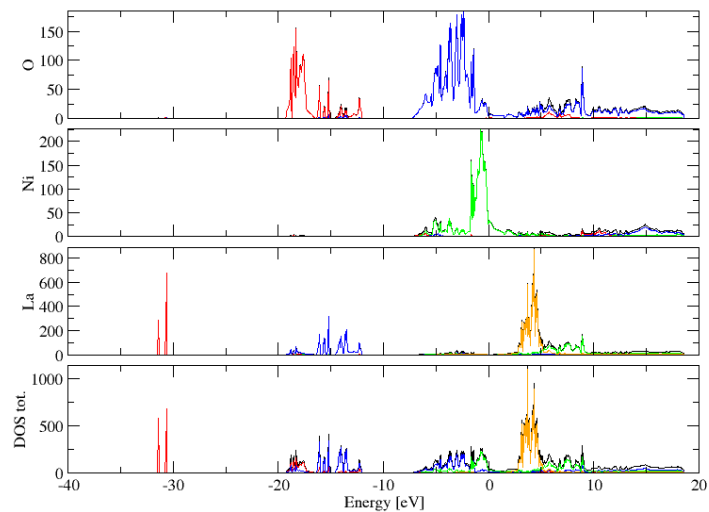

FIG. 448: (Color online) PDOS of  $\text{La}_3\text{Ni}_2\text{O}_6$  (ICSD #249209). The  $s$ -,  $p$ - and  $d$ -projected states are in red, blue and green, respectively.  $\text{La}_3\text{Ni}_2\text{O}_6$  crystallizes in space group  $I 4/m m m$  (#139), in a tetragonal body-centred structure.

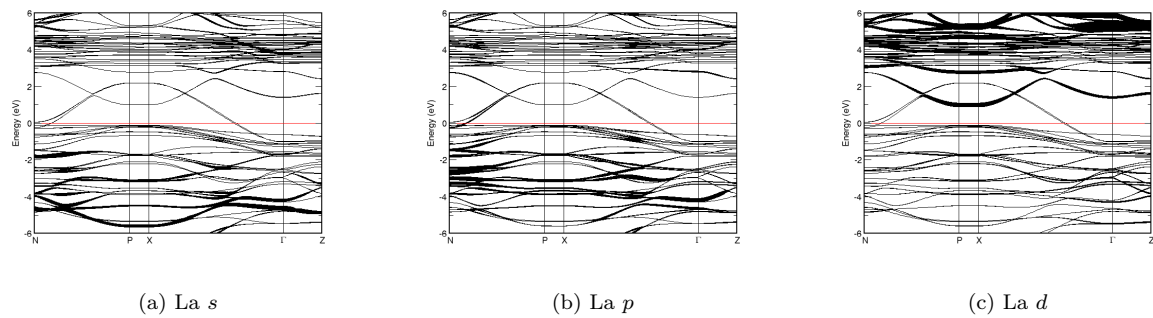

FIG. 449: Fat band representation of La in  $\text{La}_3\text{Ni}_2\text{O}_6$

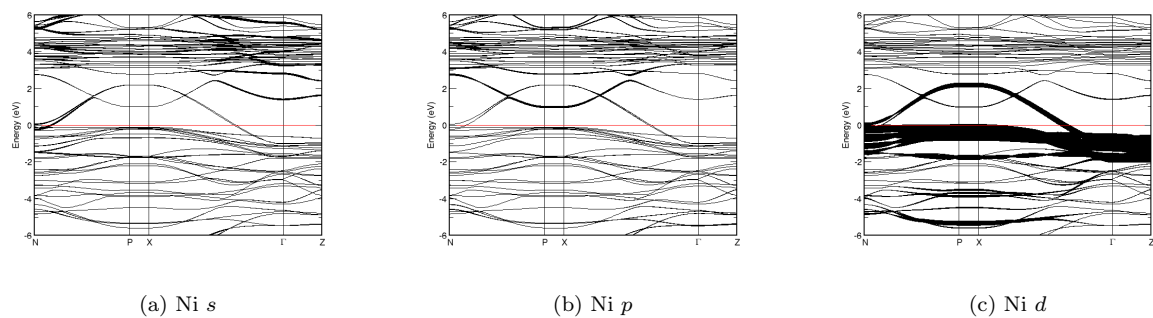

FIG. 450: Fat band representation of Ni in  $\text{La}_3\text{Ni}_2\text{O}_6$

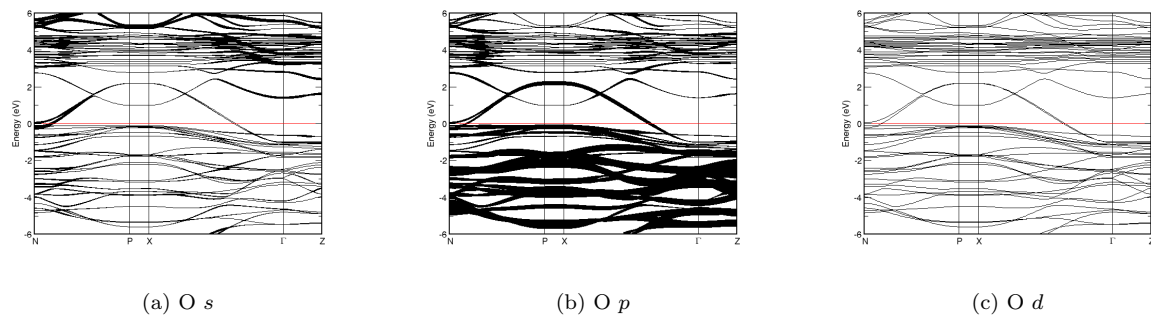FIG. 451: Fat band representation of O in  $\text{La}_3\text{Ni}_2\text{O}_6$ 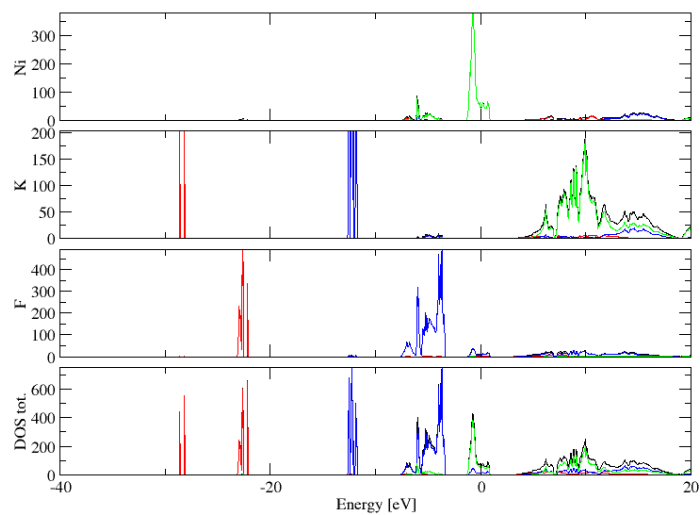FIG. 452: (Color online) PDOS of  $\text{K}_3\text{Ni}_2\text{F}_7$  (ICSD #33523). The *s*-, *p*- and *d*-projected states are in red, blue and green, respectively.  $\text{K}_3\text{Ni}_2\text{F}_7$  crystallizes in space group  $I 4/m m m$  (#139), in a tetragonal body-centred structure.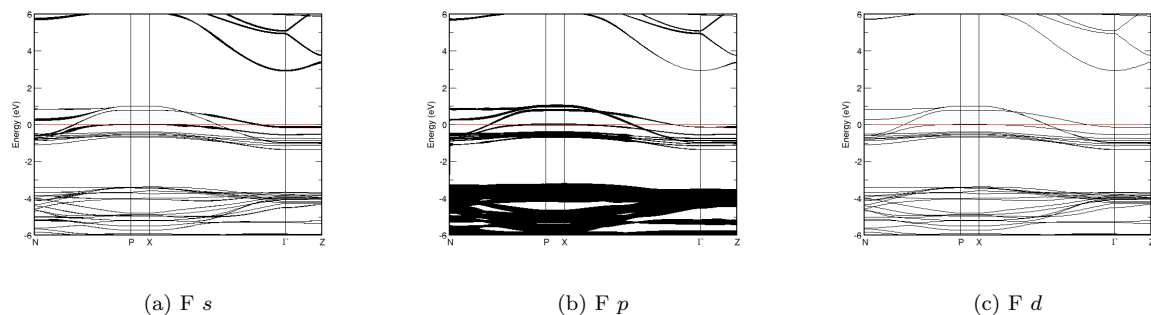FIG. 453: Fat band representation of F in  $\text{K}_3\text{Ni}_2\text{F}_7$

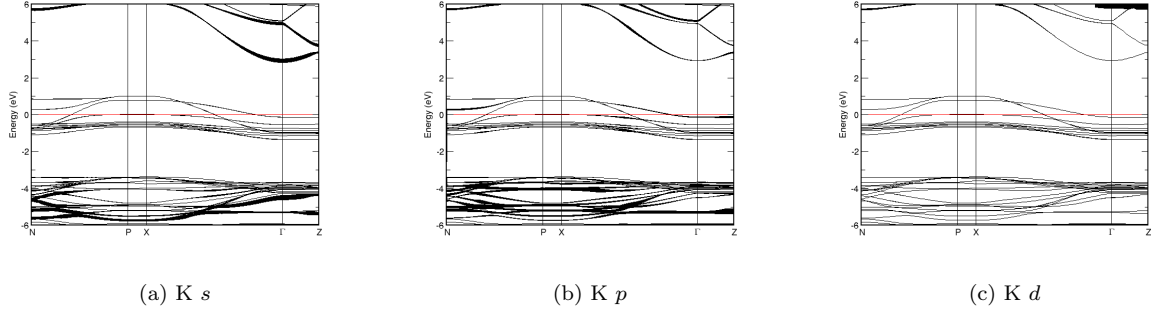FIG. 454: Fat band representation of K in  $K_3Ni_2F_7$ 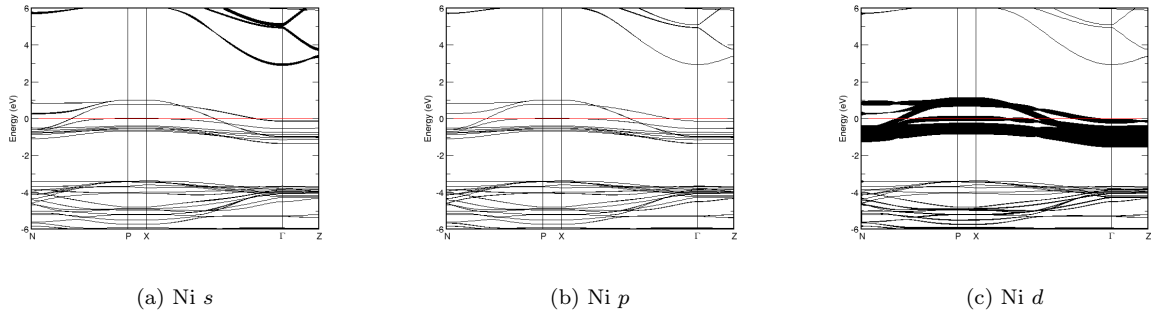FIG. 455: Fat band representation of Ni in  $K_3Ni_2F_7$ 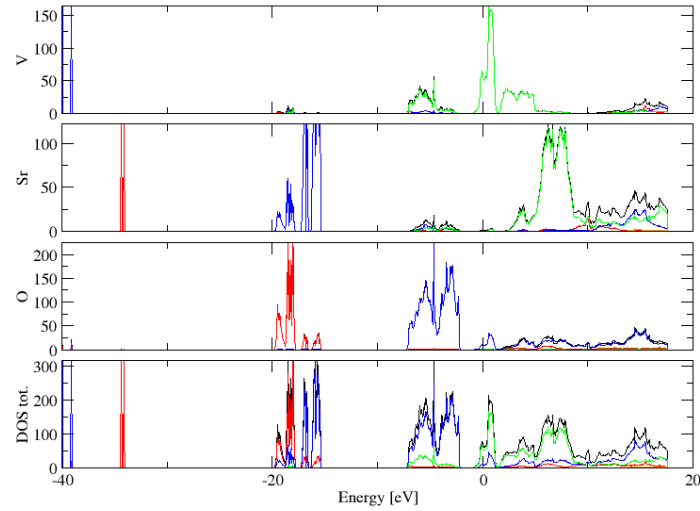FIG. 456: (Color online) PDOS of  $Sr_3V_2O_7$  (ICSD #71320). The *s*-, *p*- and *d*-projected states are in red, blue and green, respectively.  $Sr_3V_2O_7$  crystallizes in space group  $I 4/m m m$  (#139), in a tetragonal body-centred structure.

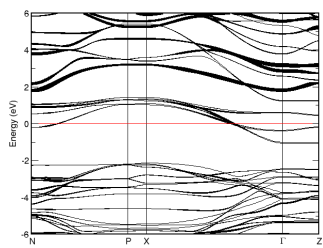(a) O *s*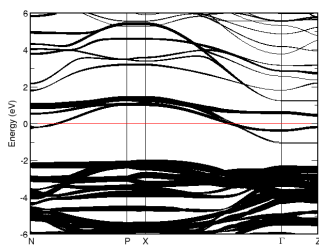(b) O *p*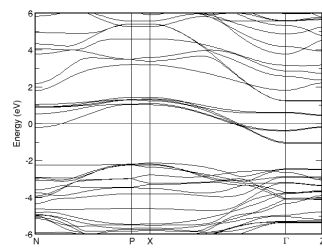(c) O *d*FIG. 457: Fat band representation of O in  $\text{Sr}_3\text{V}_2\text{O}_7$ 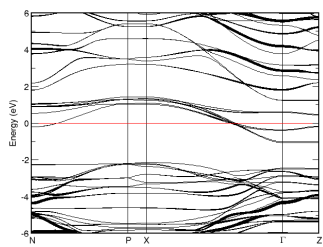(a) Sr *s*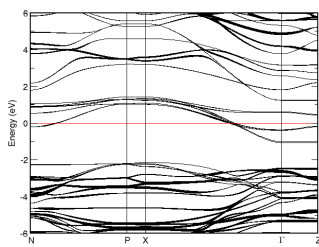(b) Sr *p*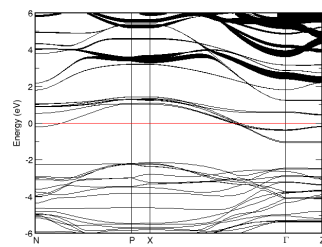(c) Sr *d*FIG. 458: Fat band representation of Sr in  $\text{Sr}_3\text{V}_2\text{O}_7$ 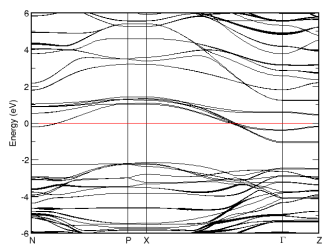(a) V *s*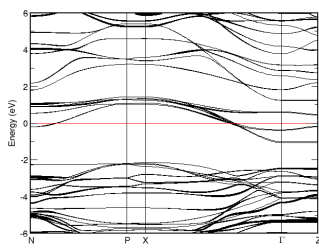(b) V *p*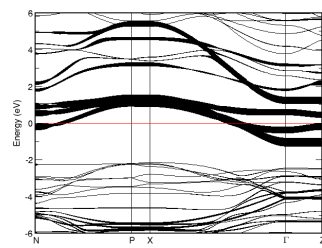(c) V *d*FIG. 459: Fat band representation of V in  $\text{Sr}_3\text{V}_2\text{O}_7$

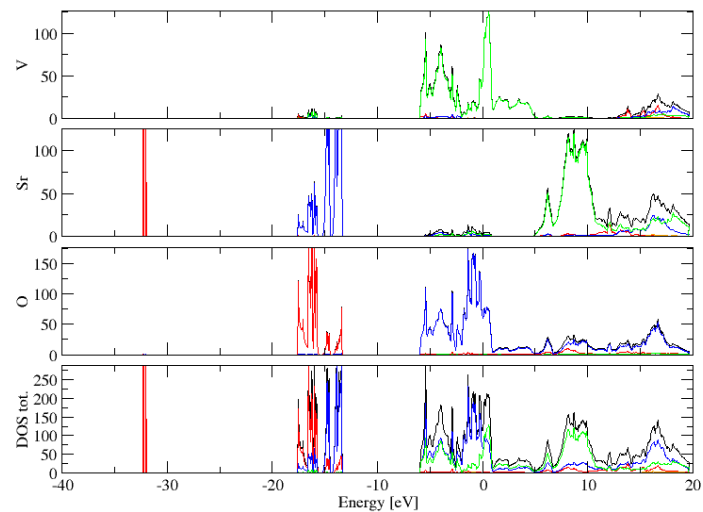

FIG. 460: (Color online) PDOS of  $\text{Sr}_3(\text{V}_2\text{O}_7)$  (ICSD #71451). The  $s$ -,  $p$ - and  $d$ -projected states are in red, blue and green, respectively.  $\text{Sr}_3(\text{V}_2\text{O}_7)$  crystallizes in space group  $I 4/m m m$  (#139), in a tetragonal body-centred structure.

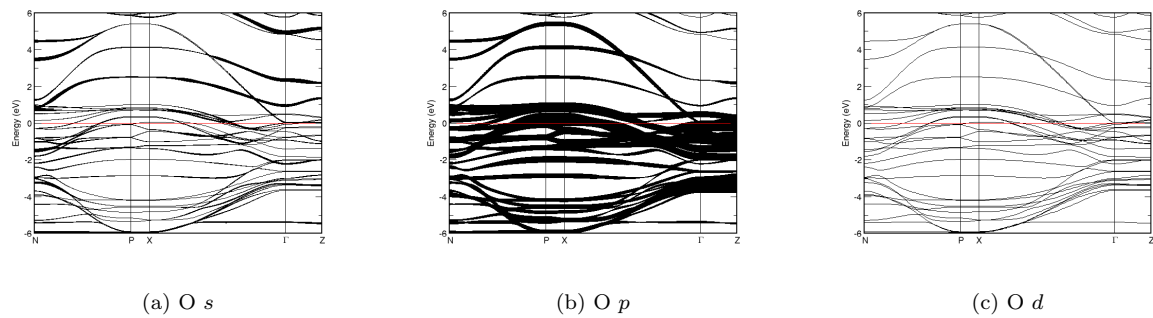

FIG. 461: Fat band representation of O in  $\text{Sr}_3(\text{V}_2\text{O}_7)$

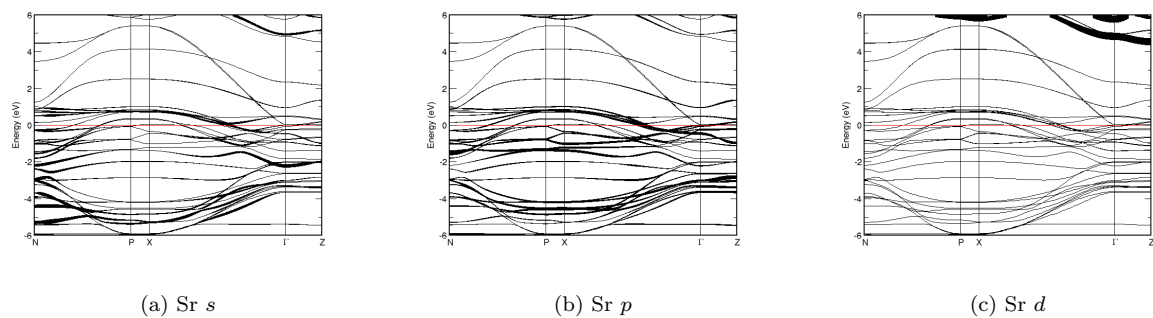

FIG. 462: Fat band representation of Sr in  $\text{Sr}_3(\text{V}_2\text{O}_7)$



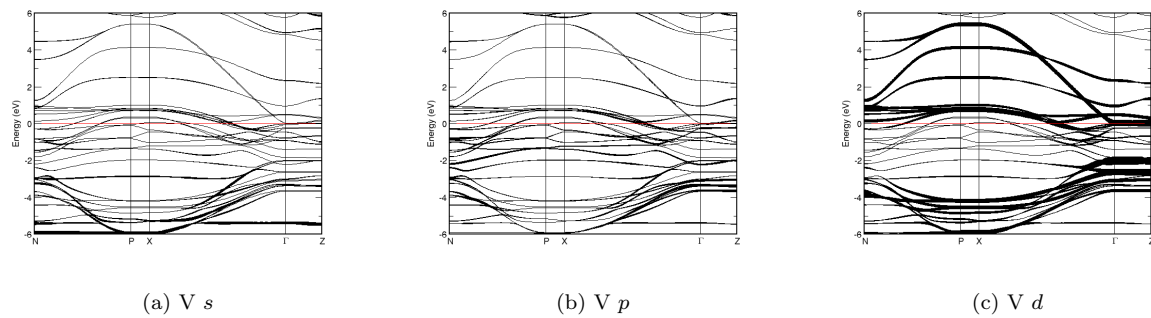FIG. 463: Fat band representation of V in  $\text{Sr}_3(\text{V}_2\text{O}_7)$ 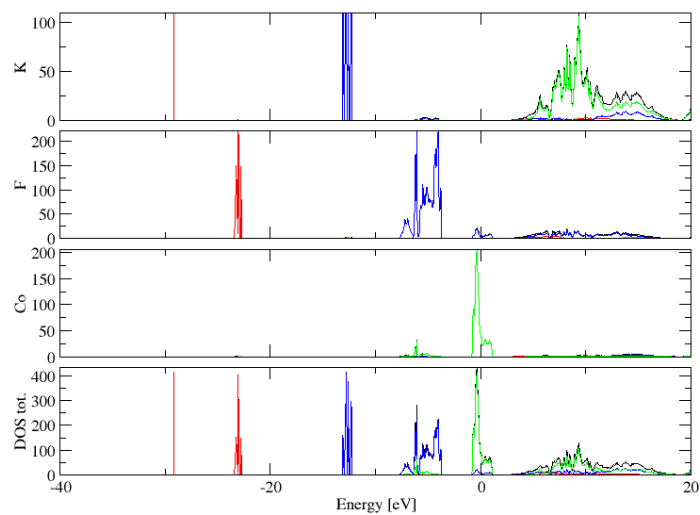FIG. 464: (Color online) PDOS of  $\text{K}_3\text{Co}_2\text{F}_7$  (ICSD #33524). The  $s$ -,  $p$ - and  $d$ -projected states are in red, blue and green, respectively.  $\text{K}_3\text{Co}_2\text{F}_7$  crystallizes in space group  $I 4/m m m$  (#139), in a tetragonal body-centred structure.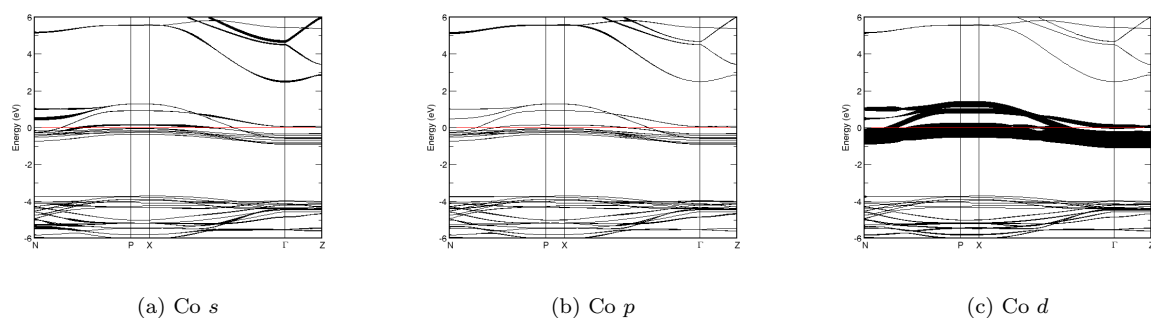FIG. 465: Fat band representation of Co in  $\text{K}_3\text{Co}_2\text{F}_7$

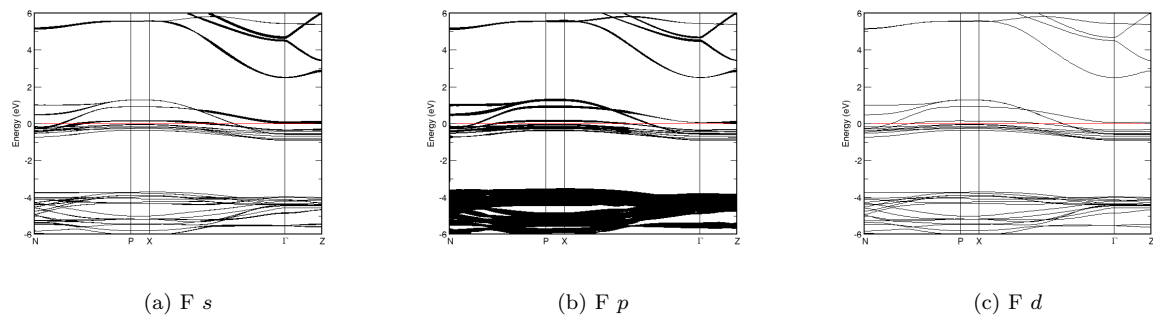FIG. 466: Fat band representation of F in  $K_3Co_2F_7$ 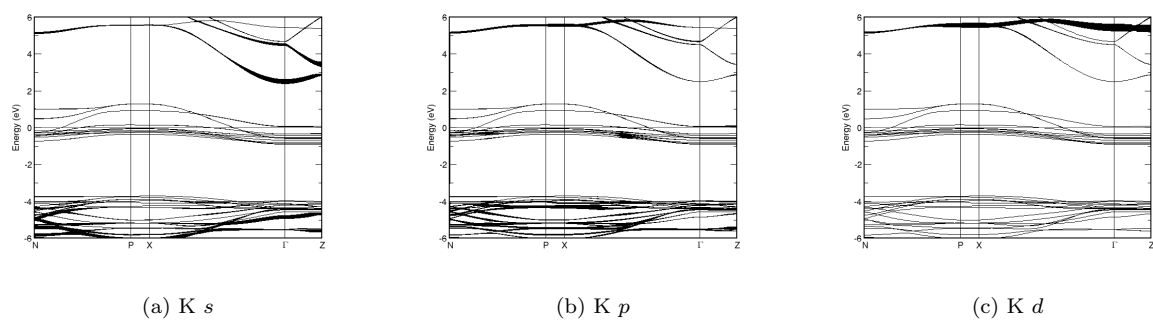FIG. 467: Fat band representation of K in  $K_3Co_2F_7$ 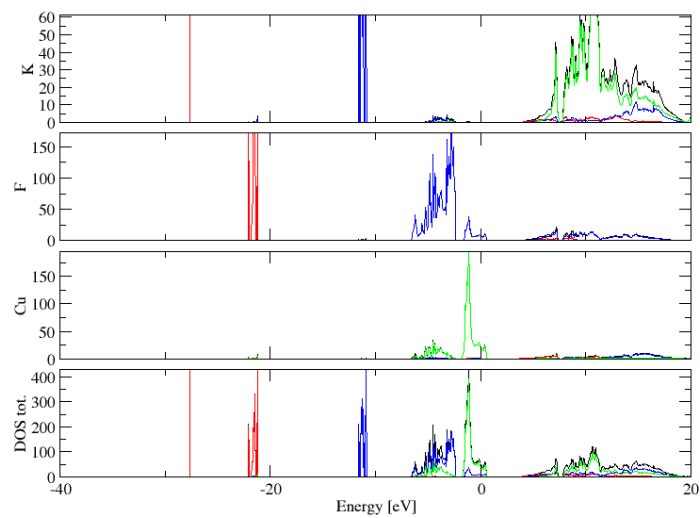FIG. 468: (Color online) PDOS of  $K_3Cu_2F_7$  (ICSD #15373). The *s*-, *p*- and *d*-projected states are in red, blue and green, respectively.  $K_3Cu_2F_7$  crystallizes in space group  $I 4/m m m$  (#139), in a tetragonal body-centred structure.

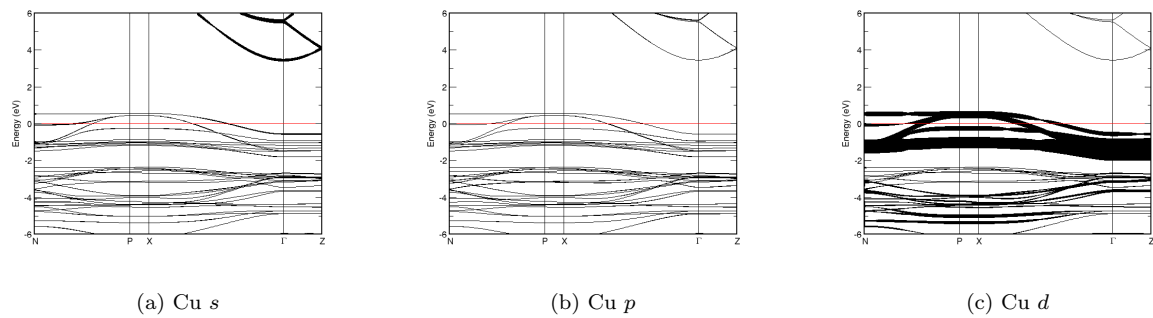FIG. 469: Fat band representation of Cu in  $K_3Cu_2F_7$ 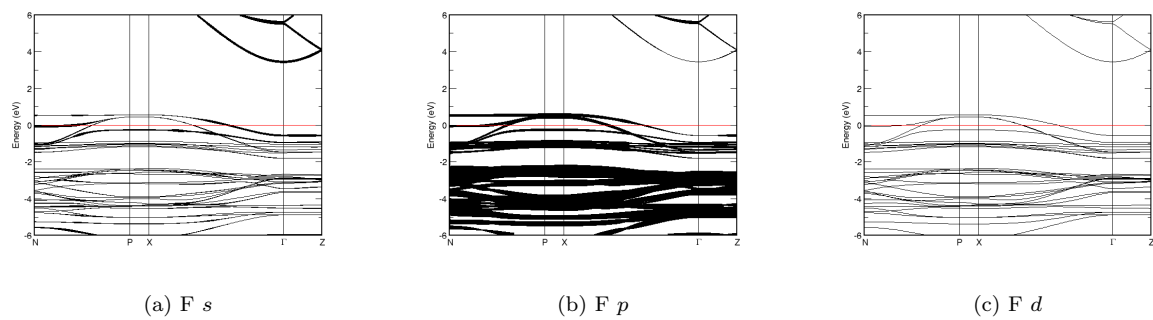FIG. 470: Fat band representation of F in  $K_3Cu_2F_7$ 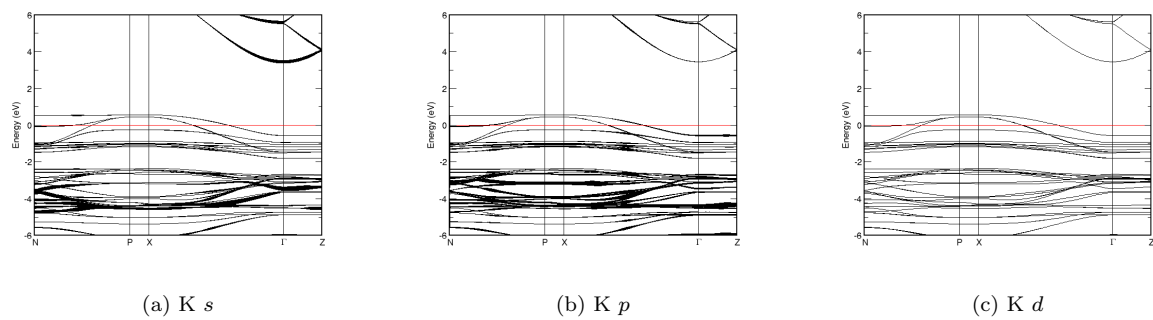FIG. 471: Fat band representation of K in  $K_3Cu_2F_7$

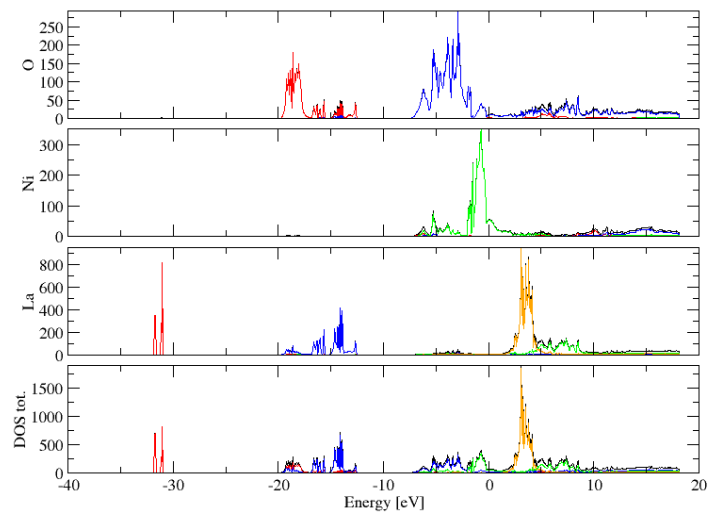

FIG. 472: (Color online) PDOS of  $\text{La}_4\text{Ni}_3\text{O}_8$  (ICSD #173372). The  $s$ -,  $p$ - and  $d$ -projected states are in red, blue and green, respectively.  $\text{La}_4\text{Ni}_3\text{O}_8$  crystallizes in space group I  $4/m\ m\ m$  (#139), in a tetragonal body-centred structure.

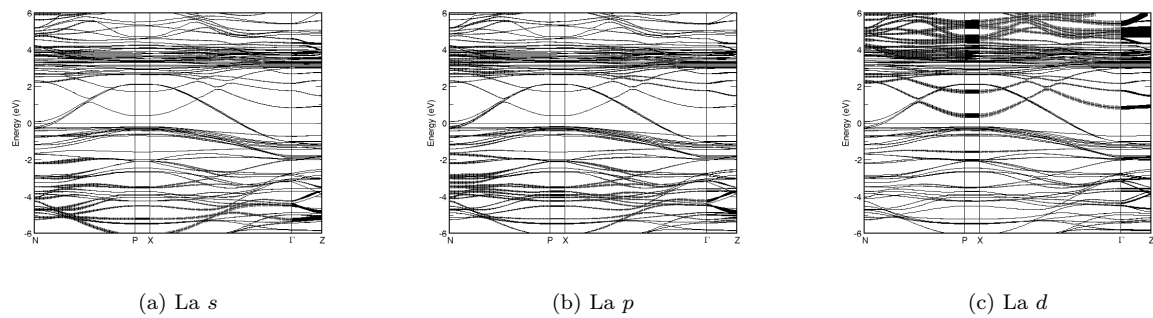

FIG. 473: Fat band representation of La in  $\text{La}_4\text{Ni}_3\text{O}_8$

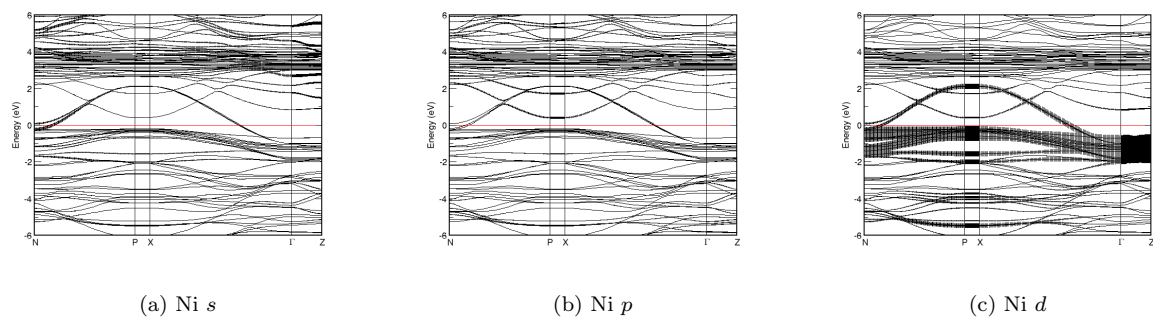

FIG. 474: Fat band representation of Ni in  $\text{La}_4\text{Ni}_3\text{O}_8$

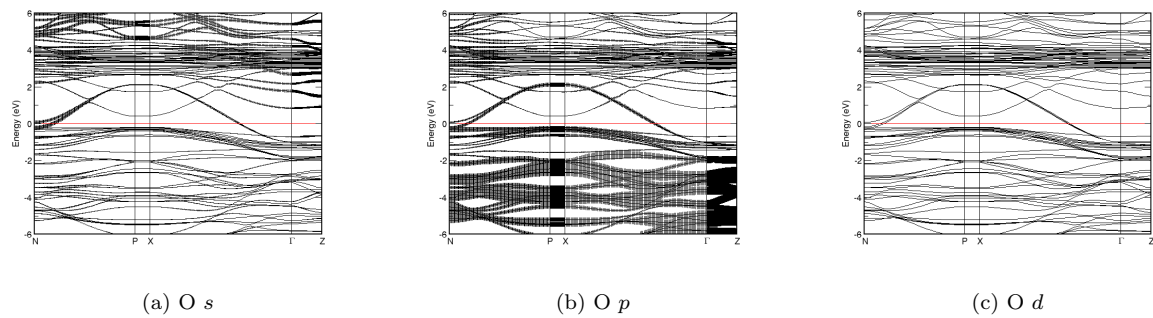FIG. 475: Fat band representation of O in  $\text{La}_4\text{Ni}_3\text{O}_8$ 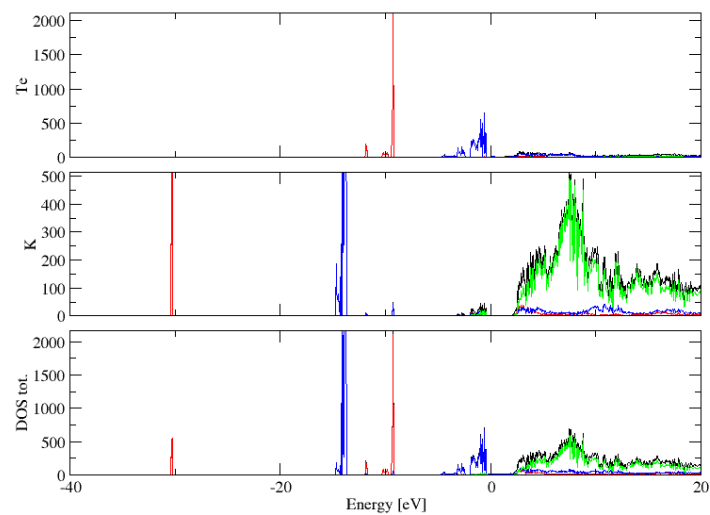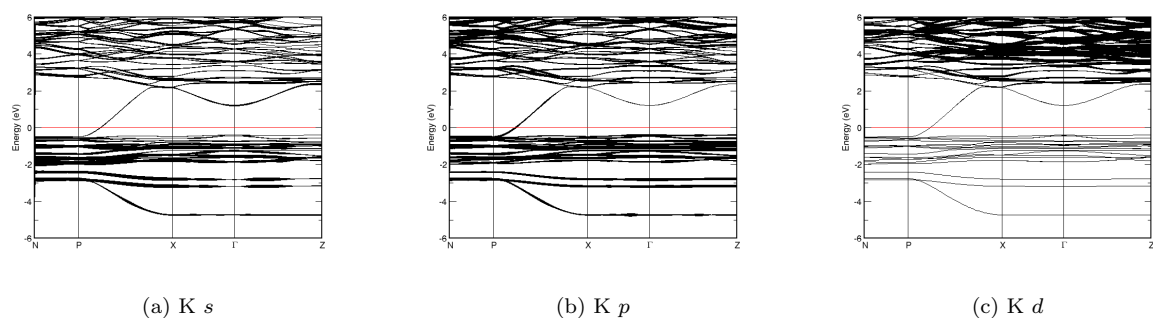FIG. 477: Fat band representation of K in  $\text{K}_5\text{Te}_3$

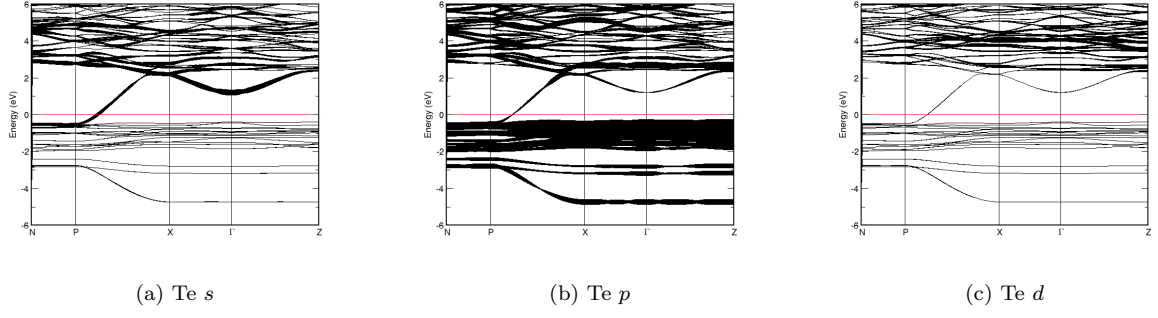FIG. 478: Fat band representation of Te in  $K_5Te_3$ 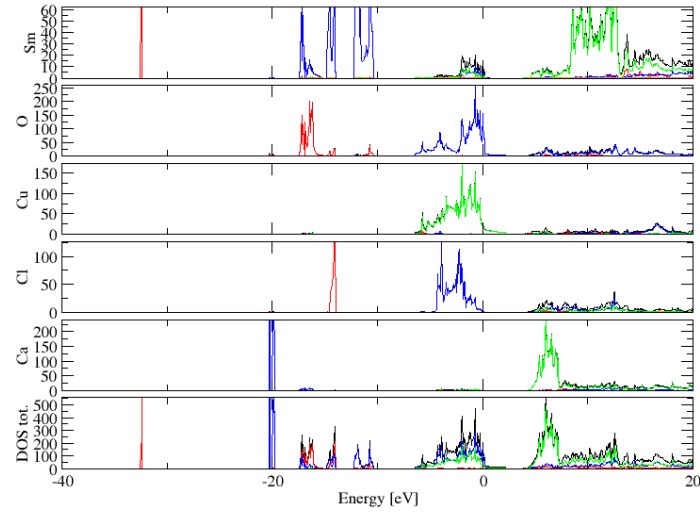FIG. 479: (Color online) PDOS of  $CaSmCuO_3Cl$  (ICSD #86428). The *s*-, *p*- and *d*-projected states are in red, blue and green, respectively.  $CaSmCuO_3Cl$  crystallizes in space group  $P 4/n m m Z$  (#129), in a tetragonal primitive structure.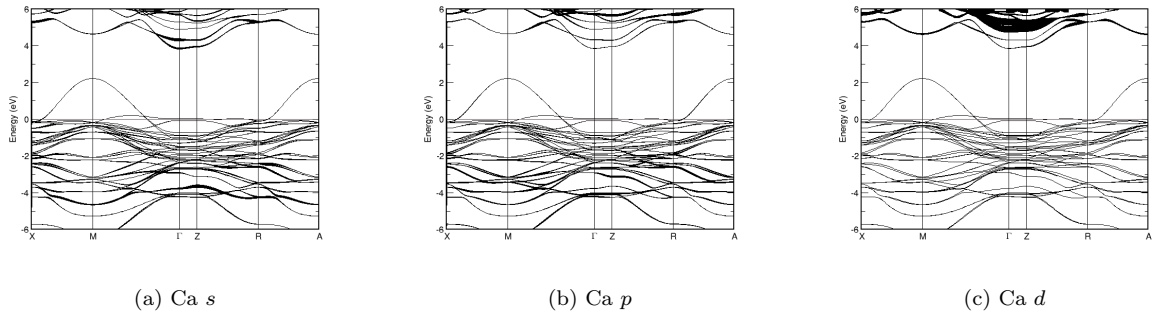FIG. 480: Fat band representation of Ca in  $CaSmCuO_3Cl$

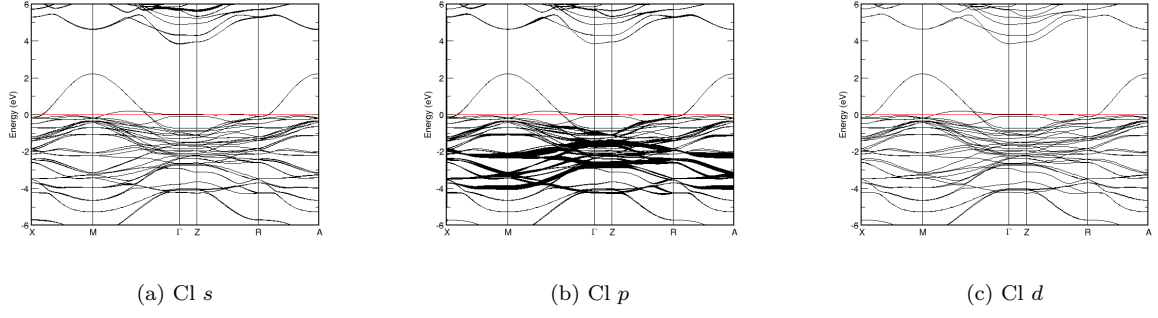FIG. 481: Fat band representation of Cl in  $\text{CaSmCuO}_3\text{Cl}$ 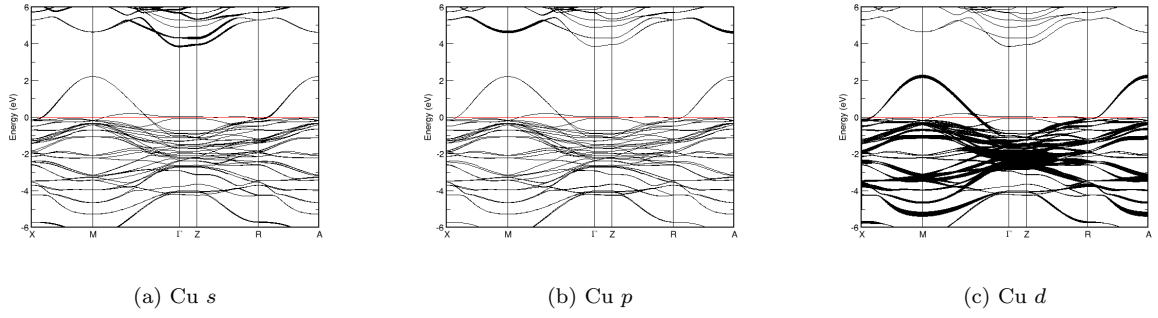FIG. 482: Fat band representation of Cu in  $\text{CaSmCuO}_3\text{Cl}$ 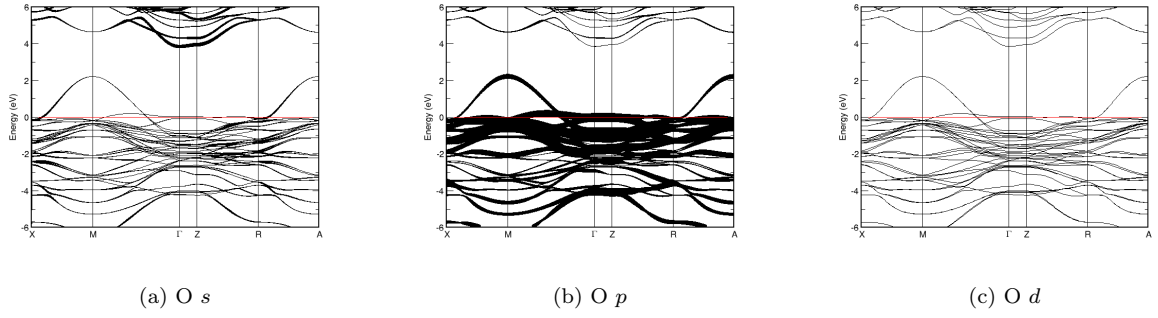FIG. 483: Fat band representation of O in  $\text{CaSmCuO}_3\text{Cl}$ 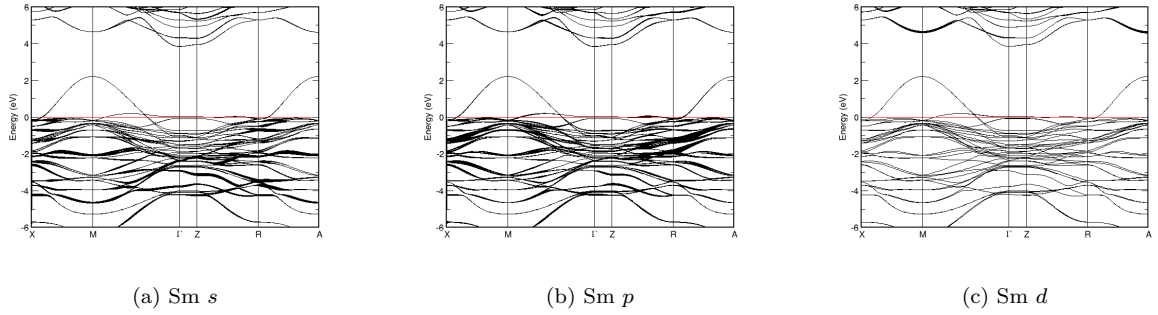FIG. 484: Fat band representation of Sm in  $\text{CaSmCuO}_3\text{Cl}$

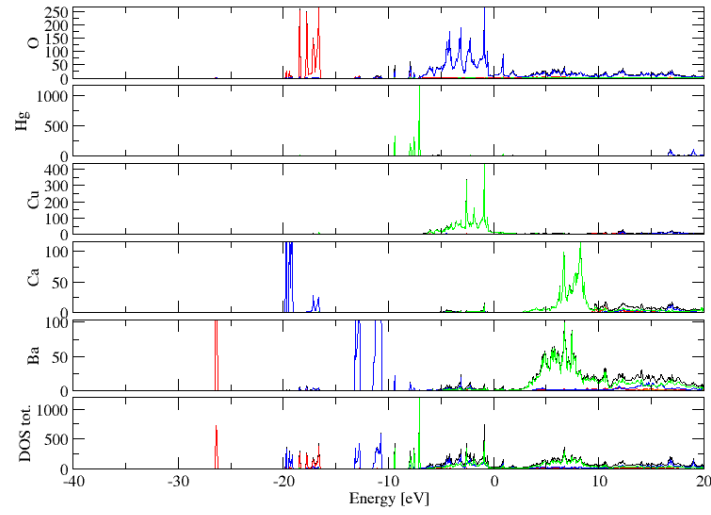

FIG. 485: (Color online) PDOS of  $\text{HgBa}_2\text{CaCu}_2\text{O}_6$  (ICSD #75725). The  $s$ -,  $p$ - and  $d$ -projected states are in red, blue and green, respectively.  $\text{HgBa}_2\text{CaCu}_2\text{O}_6$  crystallizes in space group  $P 4/m m m$  (#123), in a tetragonal primitive structure.

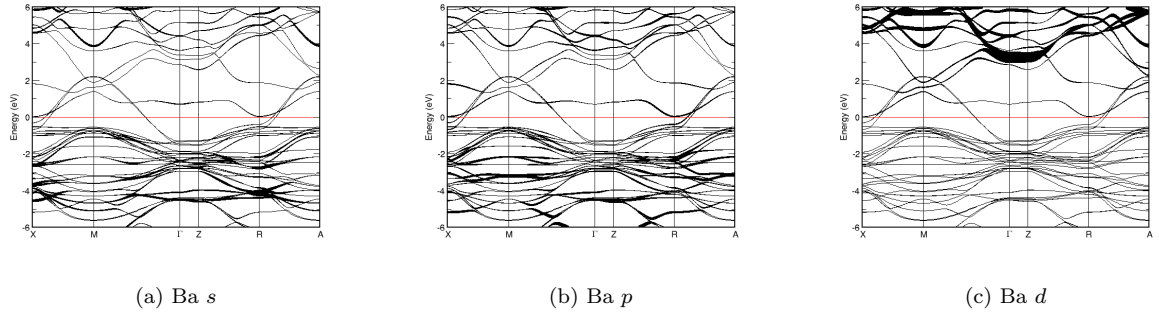

FIG. 486: Fat band representation of Ba in  $\text{HgBa}_2\text{CaCu}_2\text{O}_6$

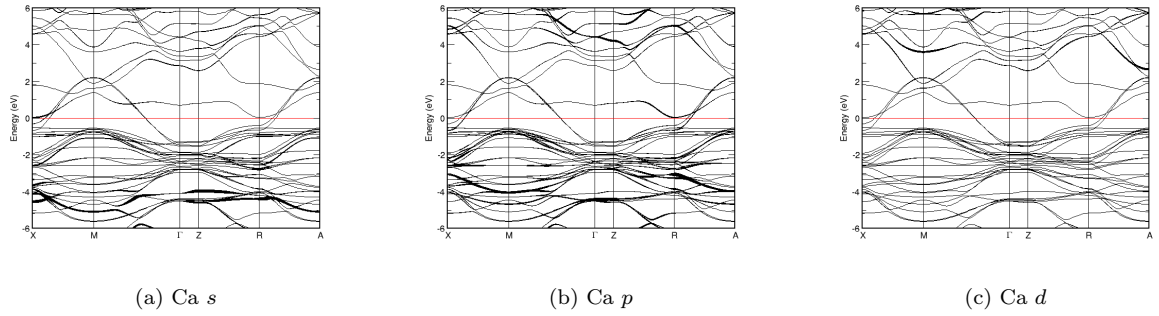

FIG. 487: Fat band representation of Ca in  $\text{HgBa}_2\text{CaCu}_2\text{O}_6$



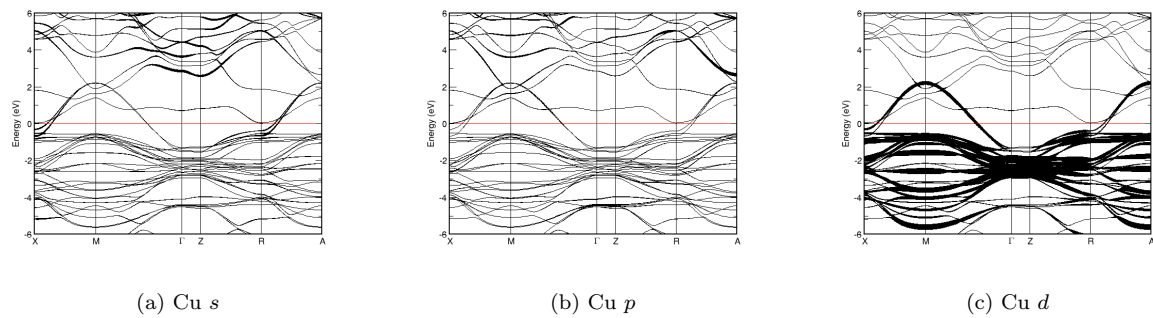FIG. 488: Fat band representation of Cu in  $\text{HgBa}_2\text{CaCu}_2\text{O}_6$ 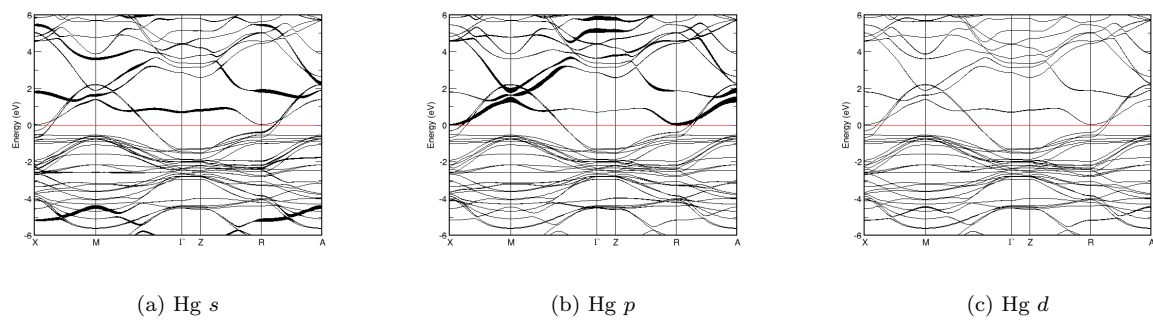FIG. 489: Fat band representation of Hg in  $\text{HgBa}_2\text{CaCu}_2\text{O}_6$ 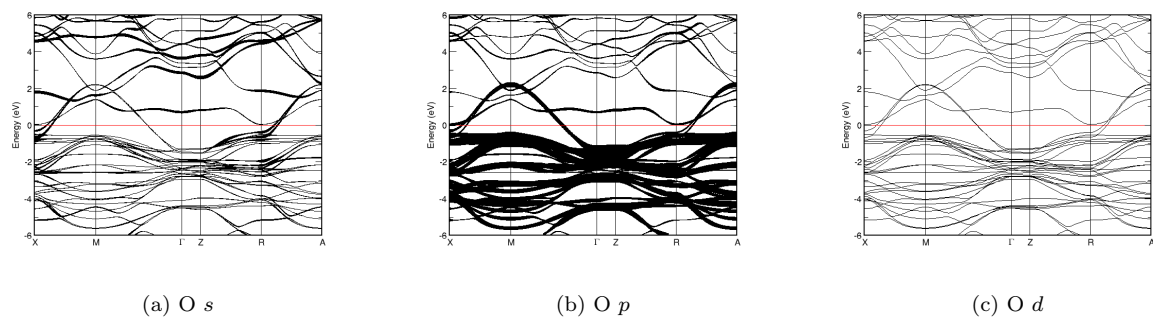FIG. 490: Fat band representation of O in  $\text{HgBa}_2\text{CaCu}_2\text{O}_6$

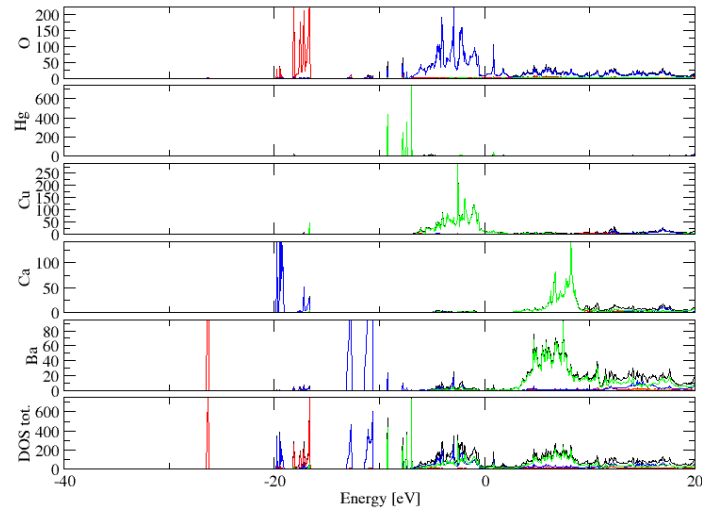

FIG. 491: (Color online) PDOS of  $\text{HgBa}_2\text{CaCu}_2\text{O}_6$  (ICSD #83087). The  $s$ -,  $p$ - and  $d$ -projected states are in red, blue and green, respectively.  $\text{HgBa}_2\text{CaCu}_2\text{O}_6$  crystallizes in space group  $P 4/m m m$  (#123), in a tetragonal primitive structure.

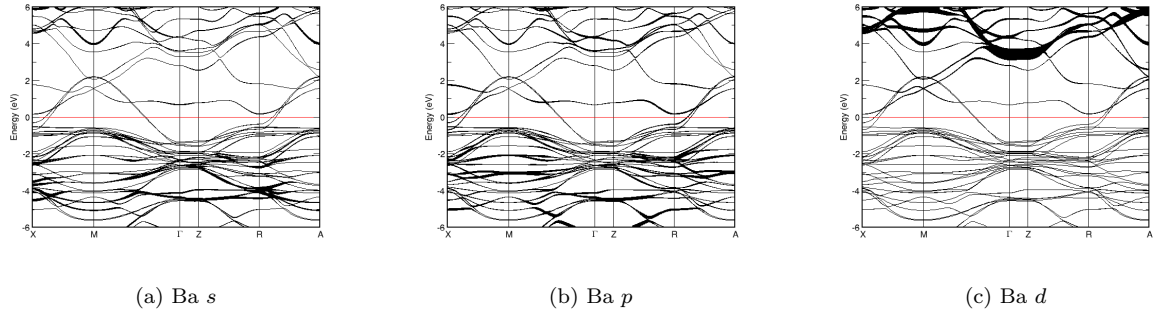

FIG. 492: Fat band representation of Ba in  $\text{HgBa}_2\text{CaCu}_2\text{O}_6$

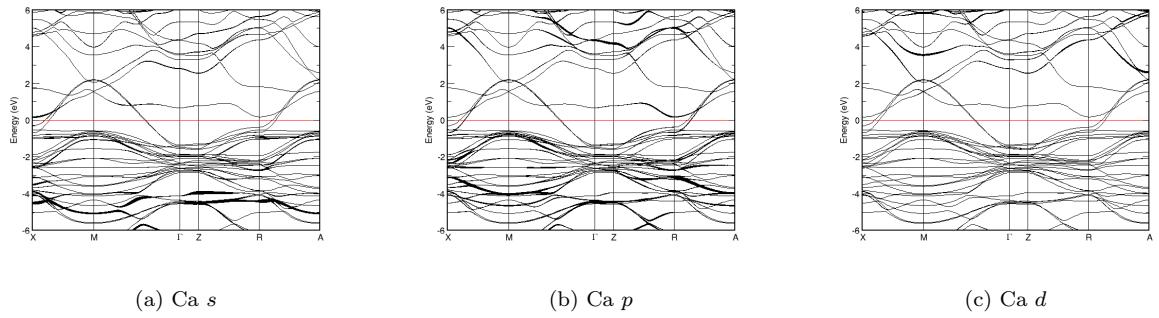

FIG. 493: Fat band representation of Ca in  $\text{HgBa}_2\text{CaCu}_2\text{O}_6$

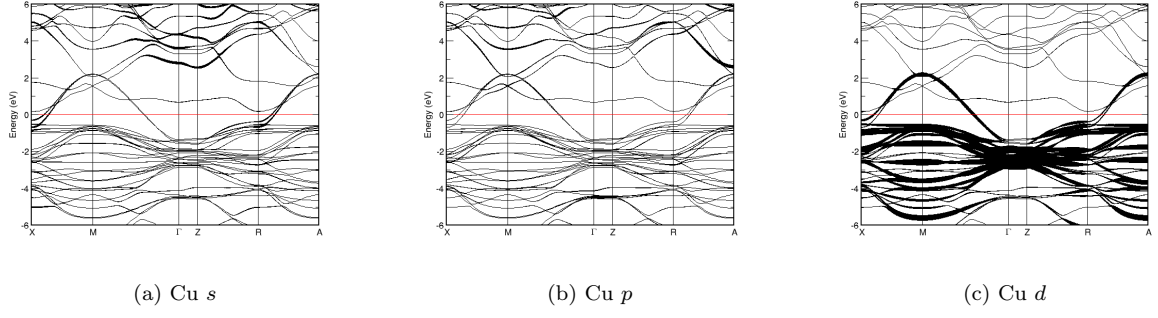FIG. 494: Fat band representation of Cu in  $\text{HgBa}_2\text{CaCu}_2\text{O}_6$ 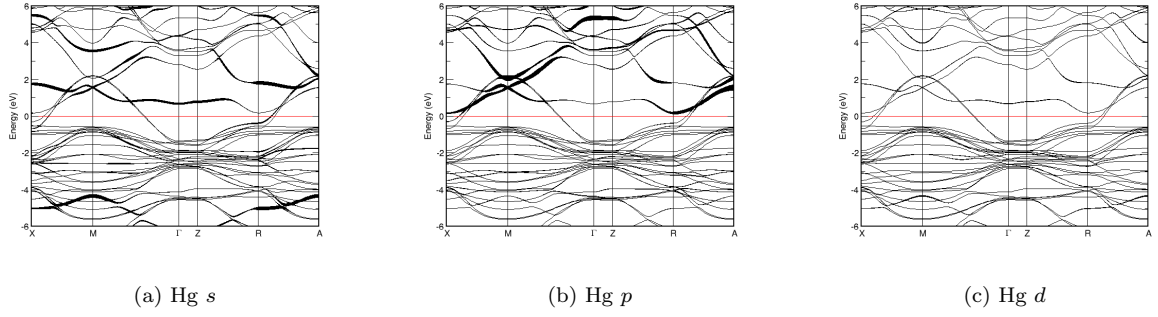FIG. 495: Fat band representation of Hg in  $\text{HgBa}_2\text{CaCu}_2\text{O}_6$ 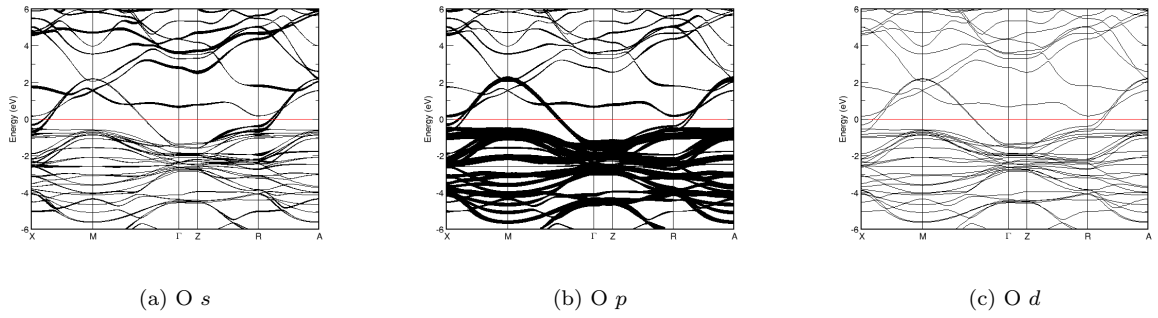FIG. 496: Fat band representation of O in  $\text{HgBa}_2\text{CaCu}_2\text{O}_6$

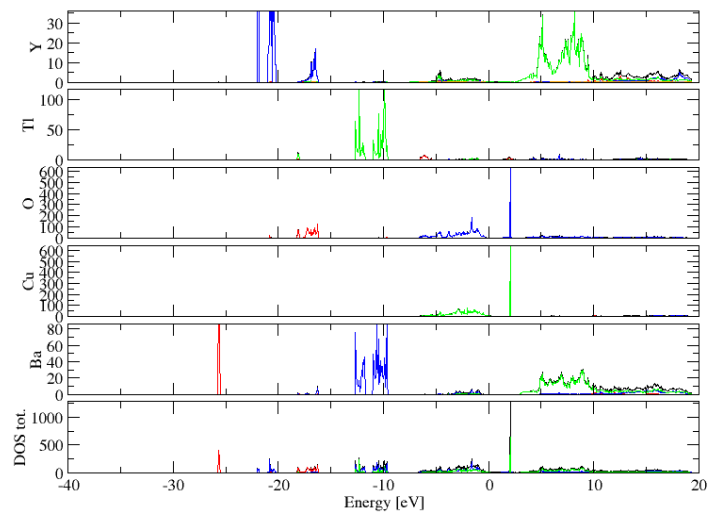

FIG. 497: (Color online) PDOS of  $\text{TiYBa}_2\text{Cu}_2\text{O}_7$  (ICSD #74163). The  $s$ -,  $p$ - and  $d$ -projected states are in red, blue and green, respectively.  $\text{TiYBa}_2\text{Cu}_2\text{O}_7$  crystallizes in space group  $P 4/m m m$  (#123), in a tetragonal primitive structure.

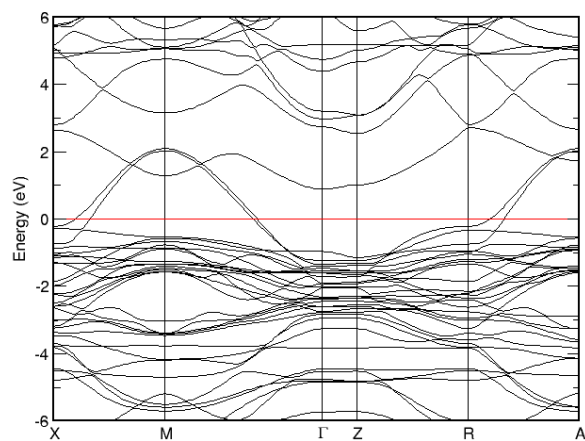

(a)  $E$  vs.  $k$

FIG. 498: Band structure of  $\text{TiYBa}_2\text{Cu}_2\text{O}_7$

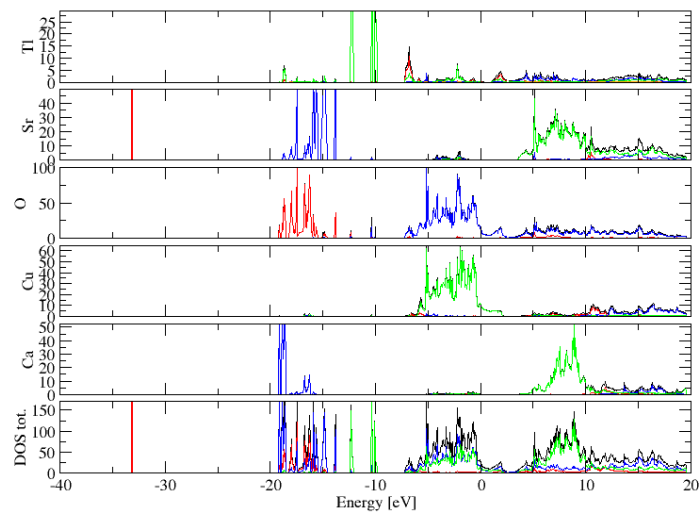

FIG. 499: (Color online) PDOS of  $\text{TlCaSr}_2\text{Cu}_2\text{O}_7$  (ICSD #74165). The  $s$ -,  $p$ - and  $d$ -projected states are in red, blue and green, respectively.  $\text{TlCaSr}_2\text{Cu}_2\text{O}_7$  crystallizes in space group  $P 4/m m m$  (#123), in a tetragonal primitive structure.

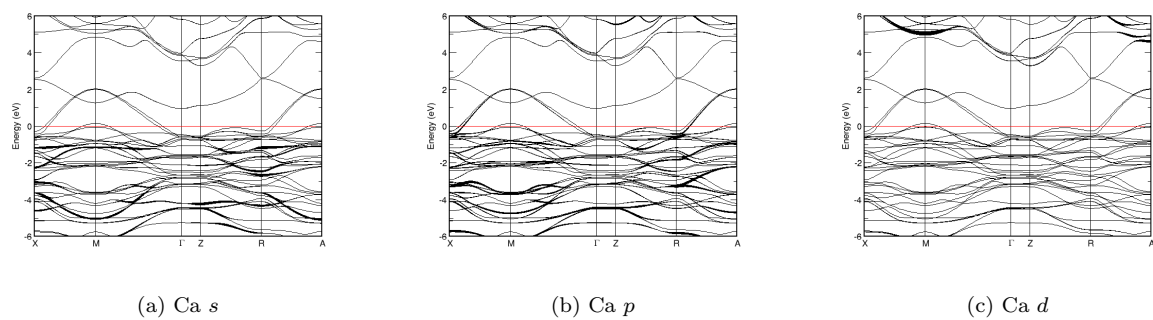

FIG. 500: Fat band representation of Ca in  $\text{TlCaSr}_2\text{Cu}_2\text{O}_7$

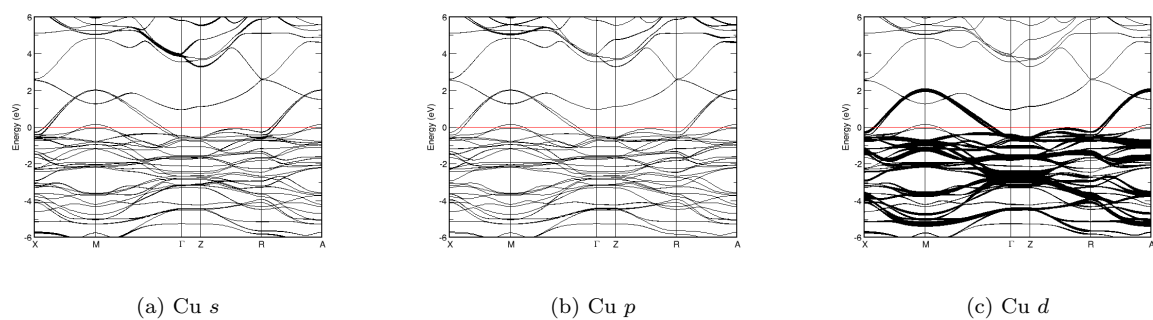

FIG. 501: Fat band representation of Cu in  $\text{TlCaSr}_2\text{Cu}_2\text{O}_7$

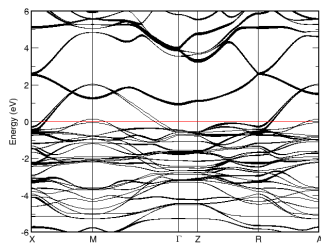(a) O *s*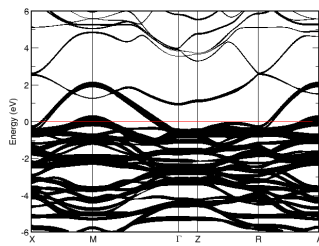(b) O *p*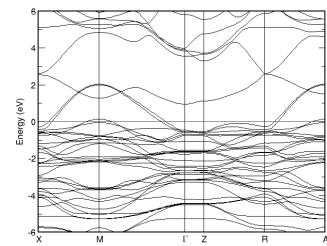(c) O *d*FIG. 502: Fat band representation of O in  $\text{TlCaSr}_2\text{Cu}_2\text{O}_7$ 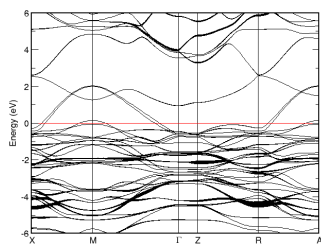(a) Sr *s*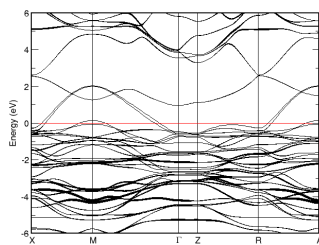(b) Sr *p*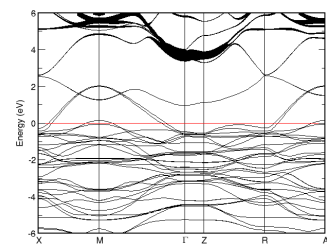(c) Sr *d*FIG. 503: Fat band representation of Sr in  $\text{TlCaSr}_2\text{Cu}_2\text{O}_7$ 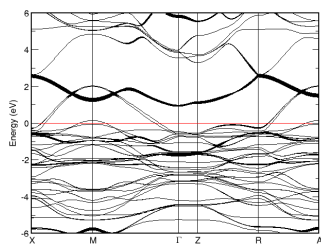(a) Tl *s*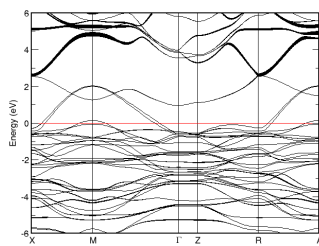(b) Tl *p*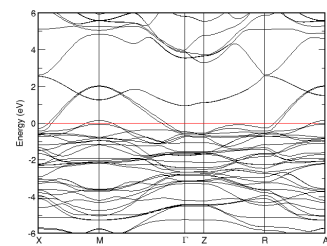(c) Tl *d*FIG. 504: Fat band representation of Tl in  $\text{TlCaSr}_2\text{Cu}_2\text{O}_7$

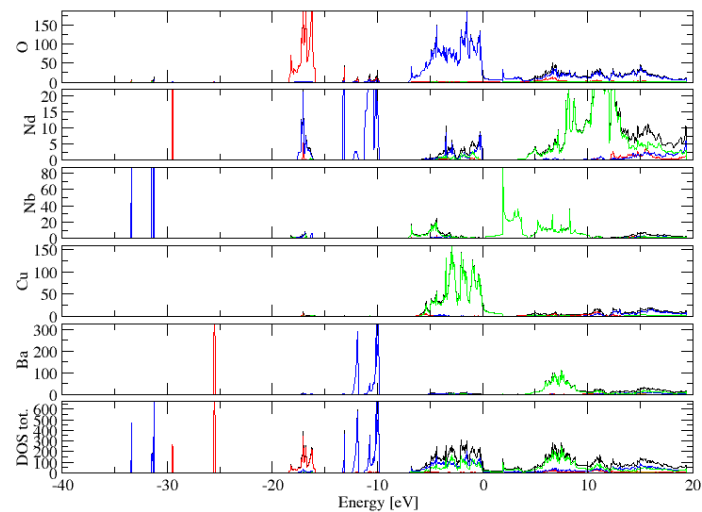

FIG. 505: (Color online) PDOS of  $\text{NdBa}_2\text{Cu}_2\text{NbO}_8$  (ICSD #44255). The  $s$ -,  $p$ - and  $d$ -projected states are in red, blue and green, respectively.  $\text{NdBa}_2\text{Cu}_2\text{NbO}_8$  crystallizes in space group  $P 4/m m m$  (#123), in a tetragonal primitive structure.

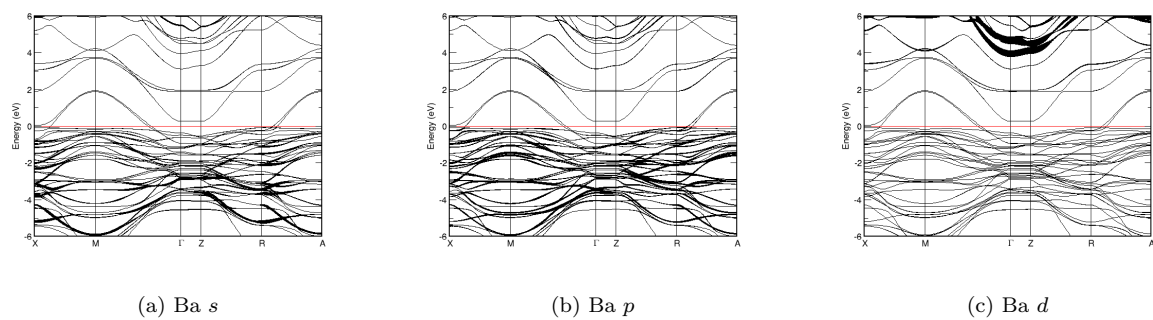

FIG. 506: Fat band representation of Ba in  $\text{NdBa}_2\text{Cu}_2\text{NbO}_8$

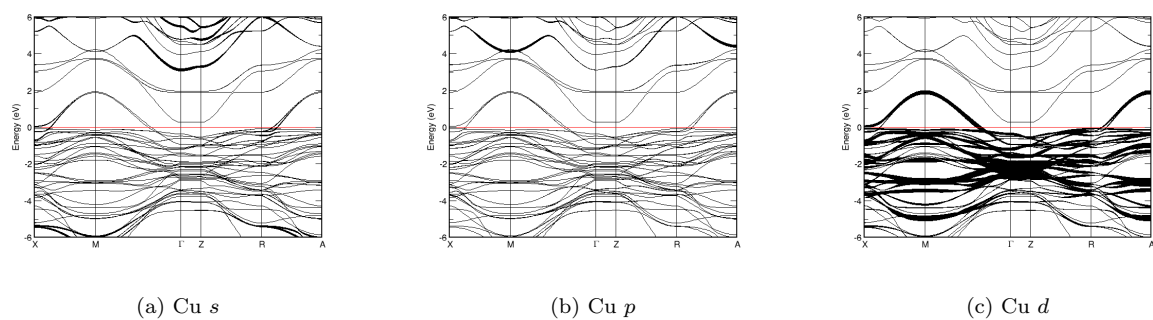

FIG. 507: Fat band representation of Cu in  $\text{NdBa}_2\text{Cu}_2\text{NbO}_8$

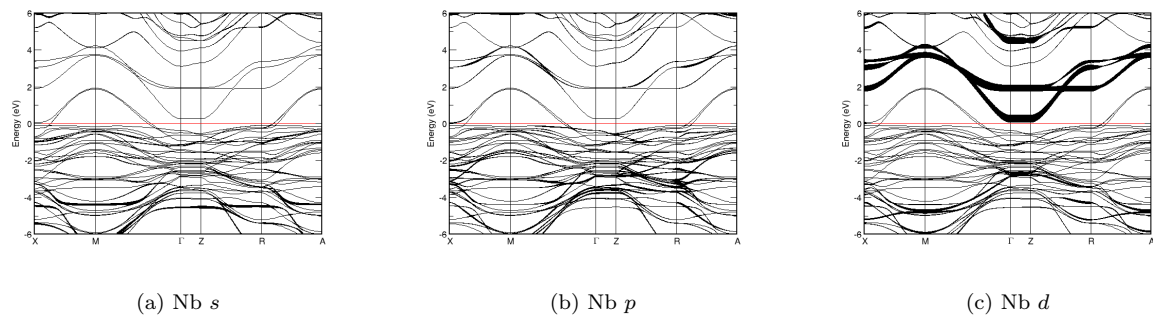FIG. 508: Fat band representation of Nb in  $\text{NdBa}_2\text{Cu}_2\text{NbO}_8$ 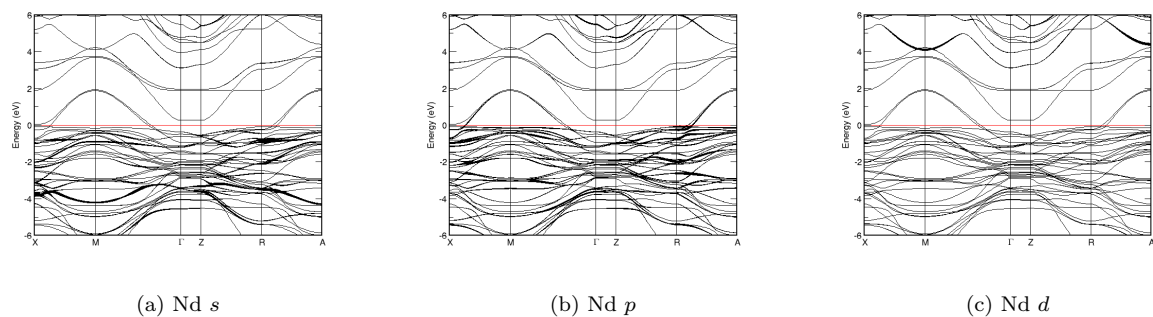FIG. 509: Fat band representation of Nd in  $\text{NdBa}_2\text{Cu}_2\text{NbO}_8$ 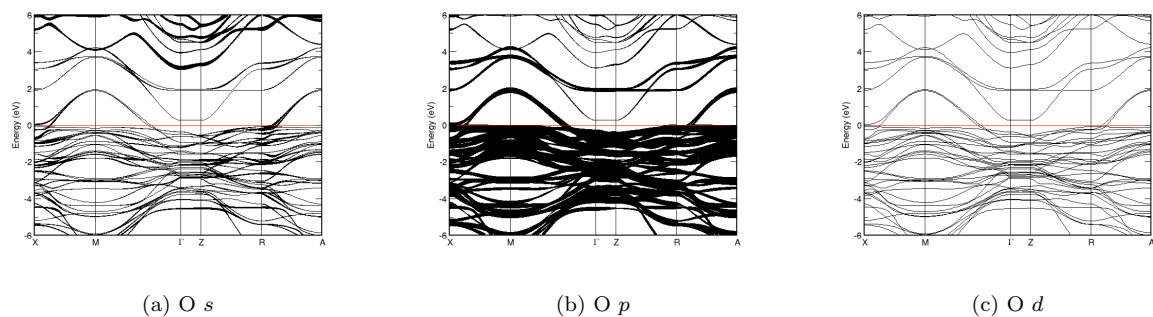FIG. 510: Fat band representation of O in  $\text{NdBa}_2\text{Cu}_2\text{NbO}_8$



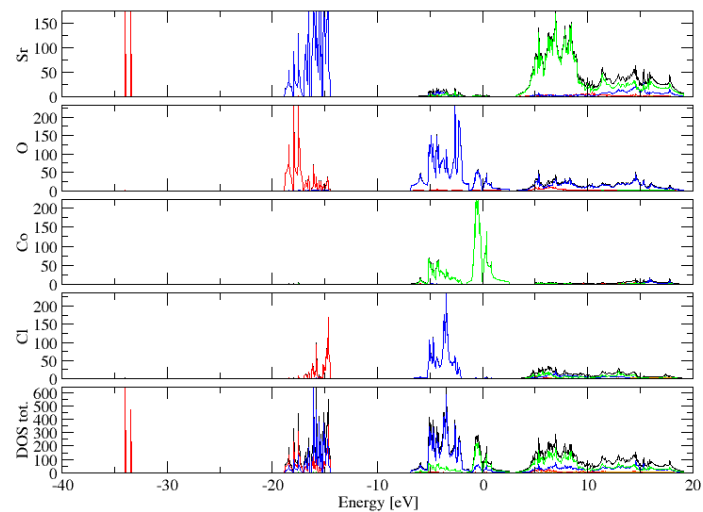

FIG. 511: (Color online) PDOS of  $\text{Sr}_2\text{CoO}_3\text{Cl}$  (ICSD #91750). The  $s$ -,  $p$ - and  $d$ -projected states are in red, blue and green, respectively.  $\text{Sr}_2\text{CoO}_3\text{Cl}$  crystallizes in space group  $P 4/n m m Z$  (#129), in a tetragonal primitive structure.

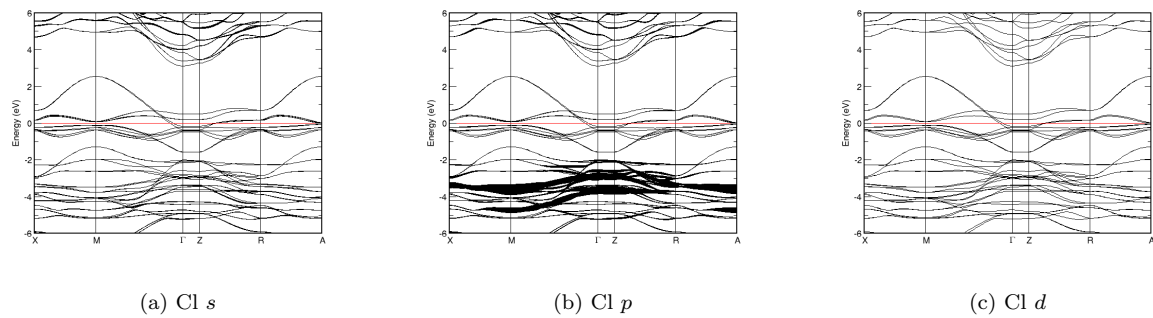

FIG. 512: Fat band representation of Cl in  $\text{Sr}_2\text{CoO}_3\text{Cl}$

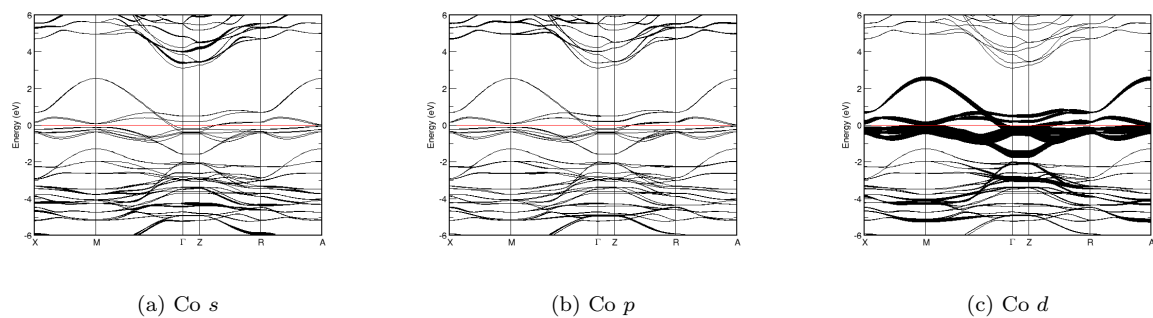

FIG. 513: Fat band representation of Co in  $\text{Sr}_2\text{CoO}_3\text{Cl}$

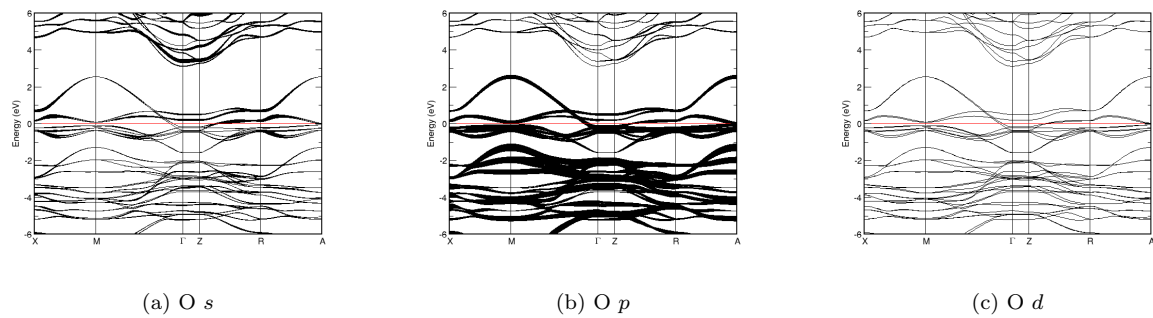FIG. 514: Fat band representation of O in  $\text{Sr}_2\text{CoO}_3\text{Cl}$ 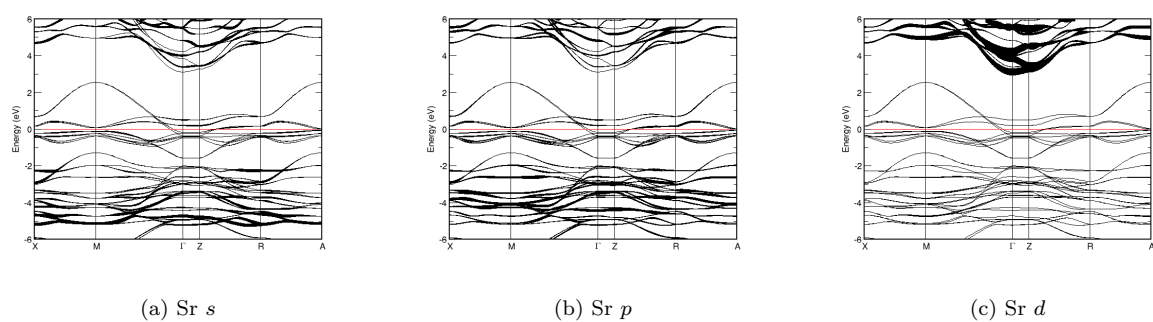FIG. 515: Fat band representation of Sr in  $\text{Sr}_2\text{CoO}_3\text{Cl}$ 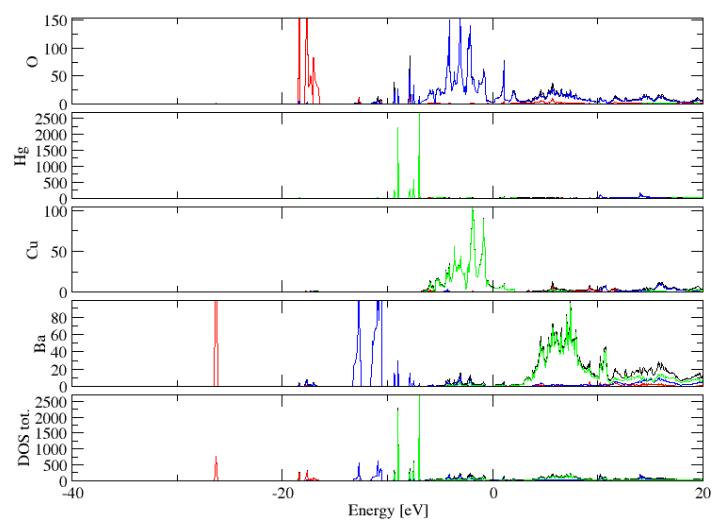

FIG. 516: (Color online) PDOS of  $\text{HgBa}_2\text{CuO}_4$  (ICSD #75720). The *s*-, *p*- and *d*-projected states are in red, blue and green, respectively.  $\text{HgBa}_2\text{CuO}_4$  crystallizes in space group  $P 4/m m m$  (#123), in a tetragonal primitive structure.

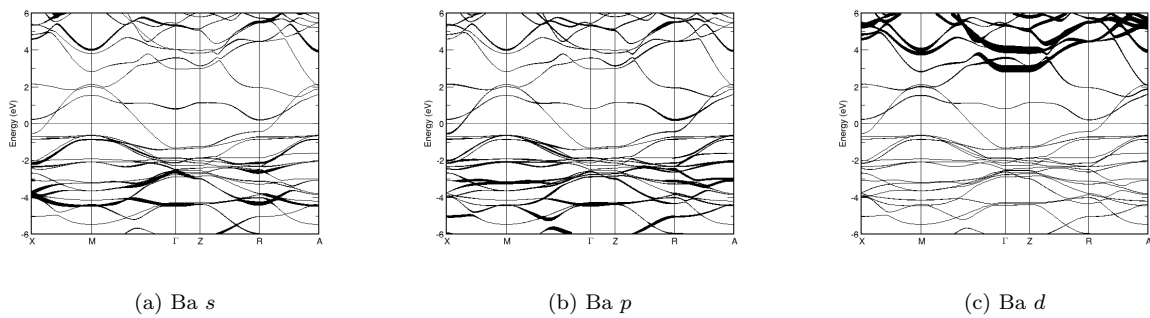FIG. 517: Fat band representation of Ba in  $\text{HgBa}_2\text{CuO}_4$ 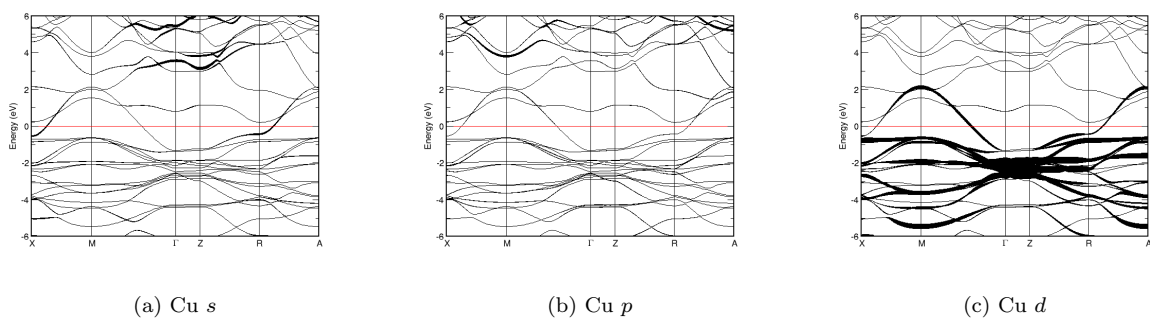FIG. 518: Fat band representation of Cu in  $\text{HgBa}_2\text{CuO}_4$ 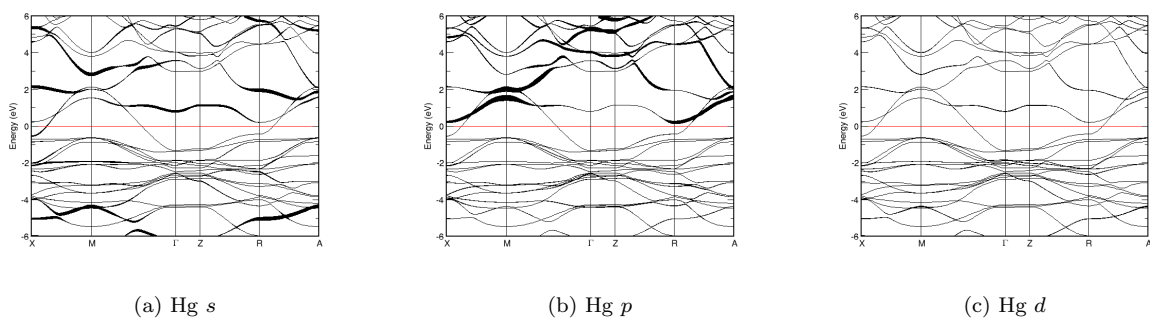FIG. 519: Fat band representation of Hg in  $\text{HgBa}_2\text{CuO}_4$ 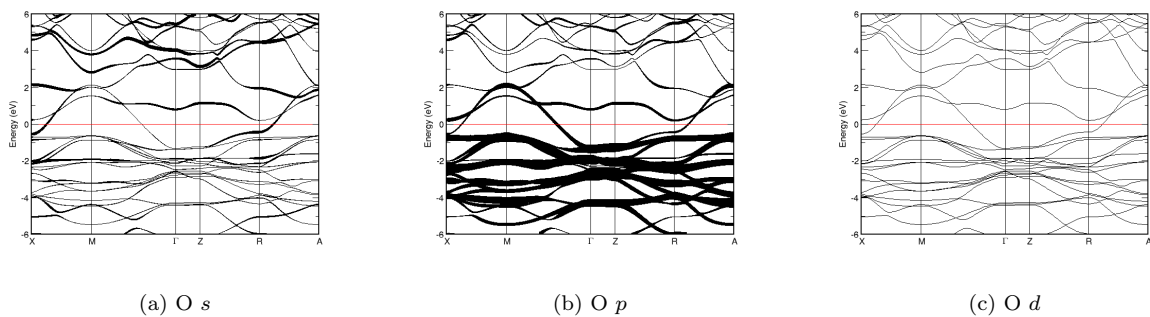FIG. 520: Fat band representation of O in  $\text{HgBa}_2\text{CuO}_4$

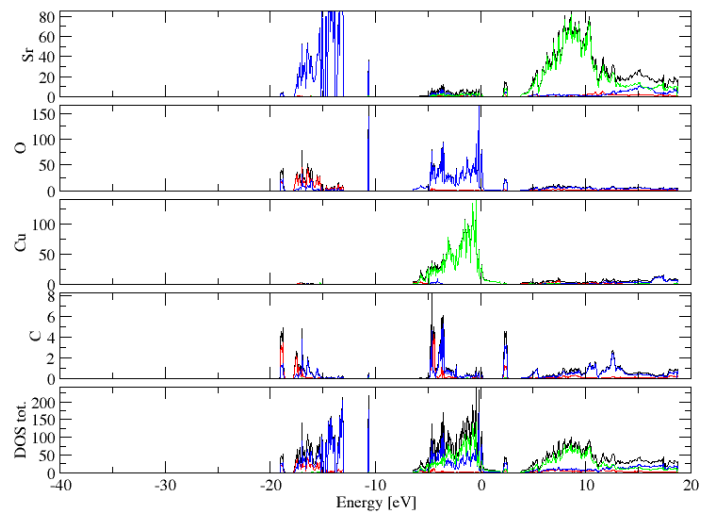

FIG. 521: (Color online) PDOS of  $\text{Sr}_2\text{CuO}_2(\text{CO}_3)$  (ICSD #83096). The  $s$ -,  $p$ - and  $d$ -projected states are in red, blue and green, respectively.  $\text{Sr}_2\text{CuO}_2(\text{CO}_3)$  crystallizes in space group P 4 21 2 (#90), in a tetragonal primitive structure.

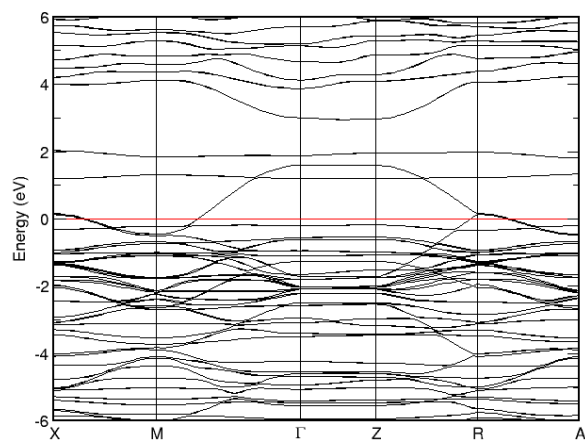

(a) E vs. k

FIG. 522: Band structure of  $\text{Sr}_2\text{CuO}_2(\text{CO}_3)$

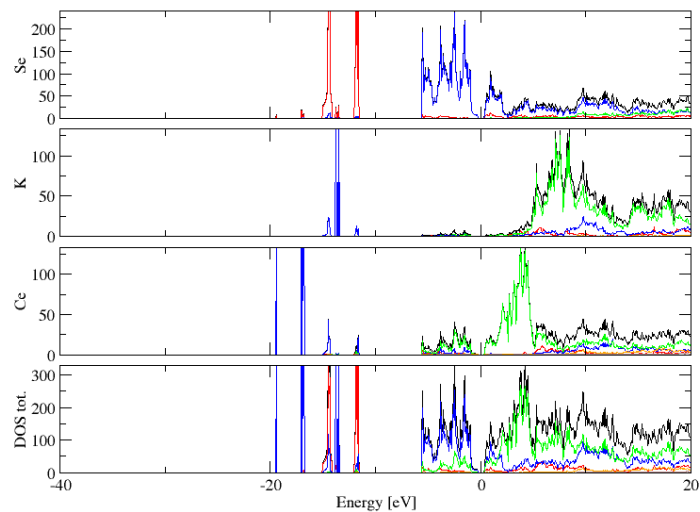

FIG. 523: (Color online) PDOS of  $\text{KCeSe}_4$  (ICSD #67656). The  $s$ -,  $p$ - and  $d$ -projected states are in red, blue and green, respectively.  $\text{KCeSe}_4$  crystallizes in space group  $P 4/n b m Z$  (#125), in a tetragonal primitive structure.

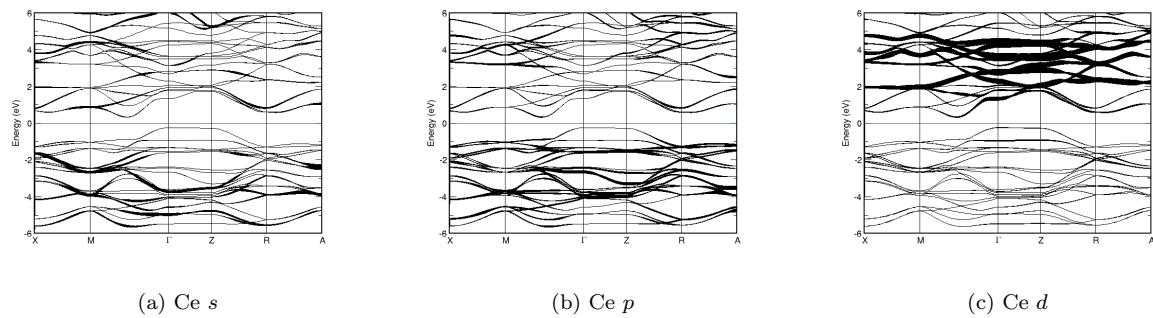

FIG. 524: Fat band representation of Ce in  $\text{KCeSe}_4$

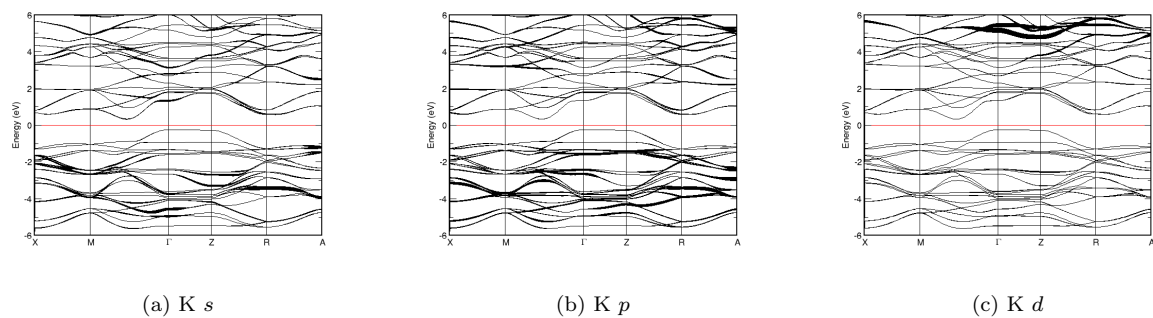

FIG. 525: Fat band representation of K in  $\text{KCeSe}_4$

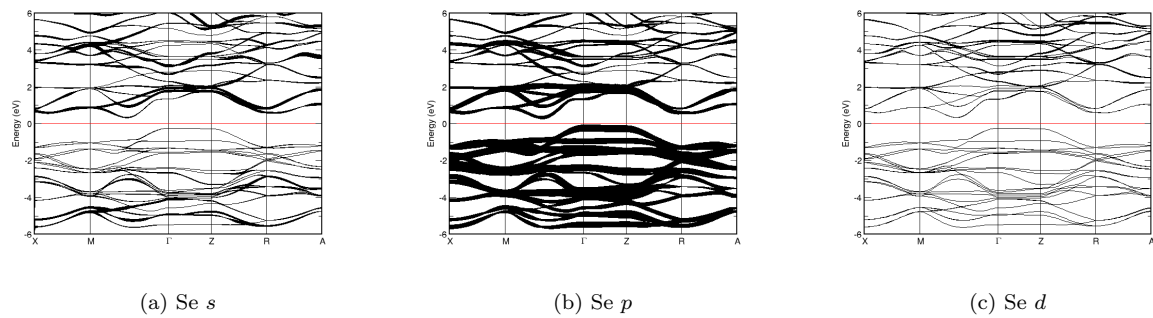FIG. 526: Fat band representation of Se in  $\text{KCeSe}_4$ 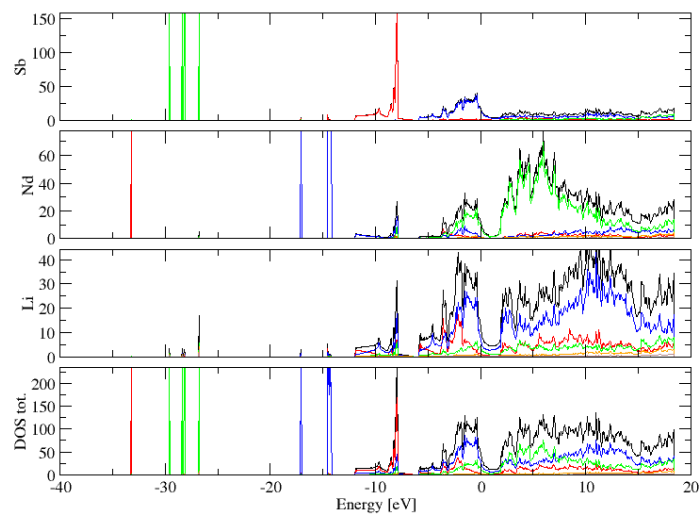FIG. 527: (Color online) PDOS of  $\text{NdLi}_2\text{Sb}_2$  (ICSD #36020). The  $s$ -,  $p$ - and  $d$ -projected states are in red, blue and green, respectively.  $\text{NdLi}_2\text{Sb}_2$  crystallizes in space group  $P 4/n m m Z$  (#129), in a tetragonal primitive structure.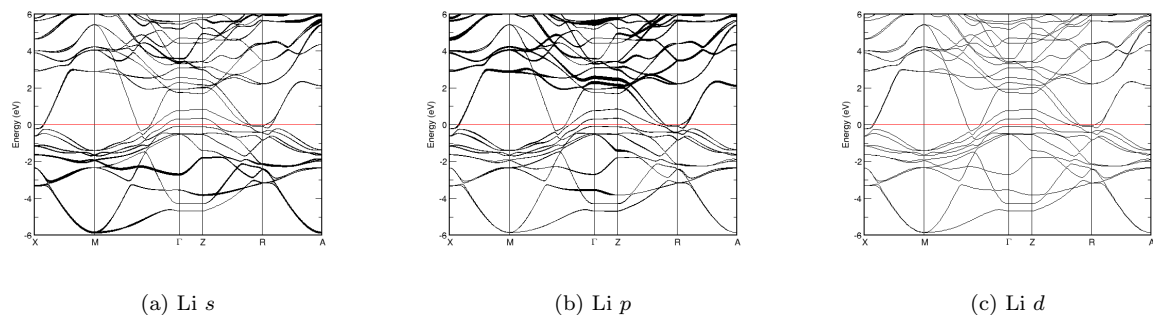FIG. 528: Fat band representation of Li in  $\text{NdLi}_2\text{Sb}_2$

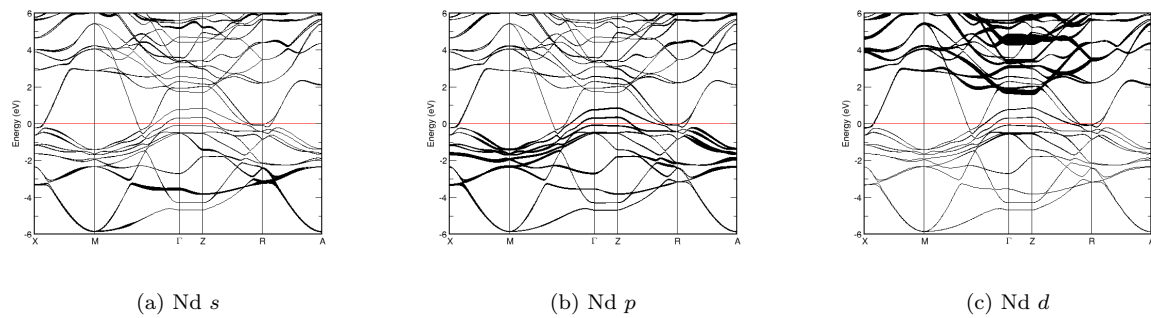FIG. 529: Fat band representation of Nd in  $\text{NdLi}_2\text{Sb}_2$ 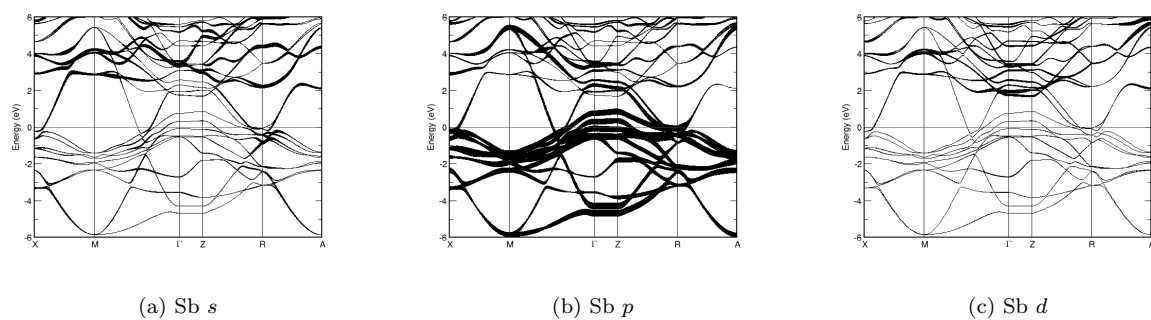FIG. 530: Fat band representation of Sb in  $\text{NdLi}_2\text{Sb}_2$ 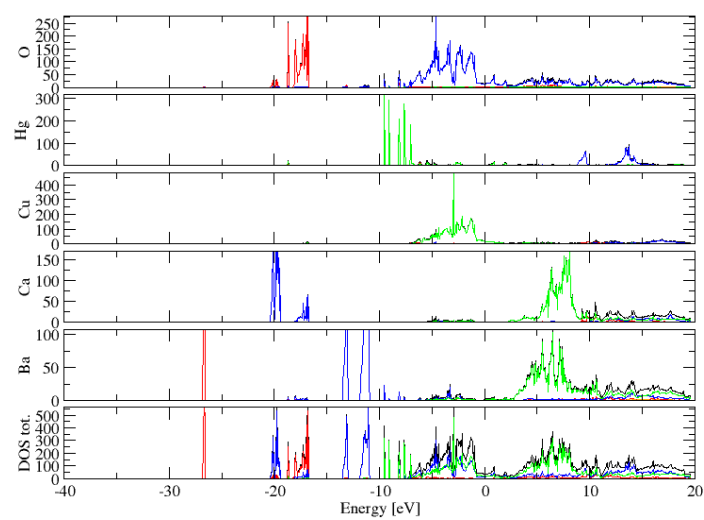FIG. 531: (Color online) PDOS of  $\text{HgBa}_2\text{Ca}_2\text{Cu}_3\text{O}_8$  (ICSD #75730). The  $s$ -,  $p$ - and  $d$ -projected states are in red, blue and green, respectively.  $\text{HgBa}_2\text{Ca}_2\text{Cu}_3\text{O}_8$  crystallizes in space group  $P 4/m m m$  (#123), in a tetragonal primitive structure.

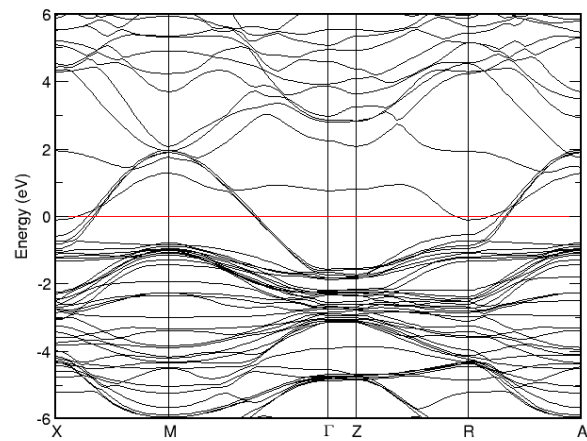(a)  $E$  vs.  $k$ FIG. 532: Band structure of  $\text{HgBa}_2\text{Ca}_2\text{Cu}_3\text{O}_8$ 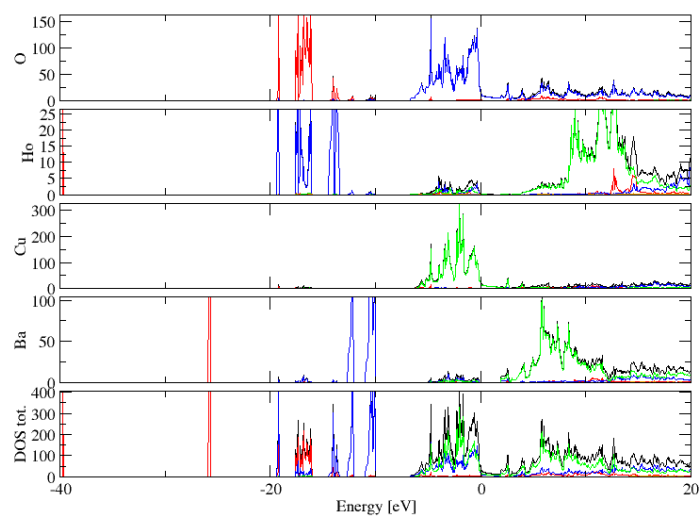

FIG. 533: (Color online) PDOS of  $\text{HoBa}_2\text{Cu}_3\text{O}_6$  (ICSD #68047). The  $s$ -,  $p$ - and  $d$ -projected states are in red, blue and green, respectively.  $\text{HoBa}_2\text{Cu}_3\text{O}_6$  crystallizes in space group  $P 4/m m m$  (#123), in a tetragonal primitive structure.



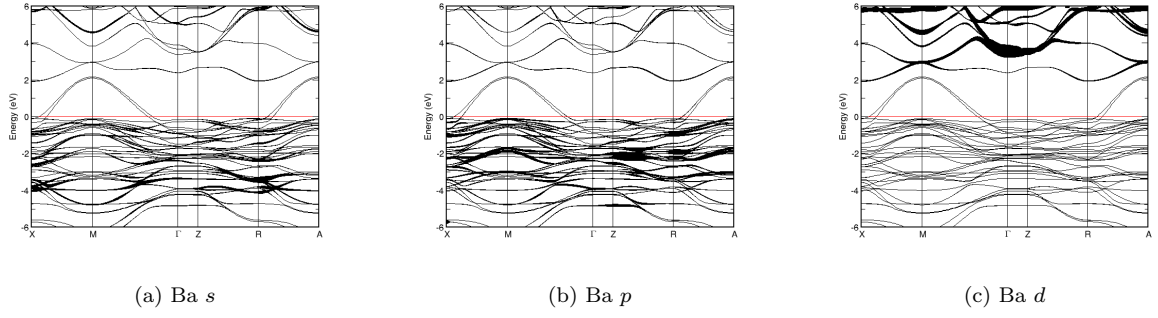FIG. 534: Fat band representation of Ba in  $\text{HoBa}_2\text{Cu}_3\text{O}_6$ 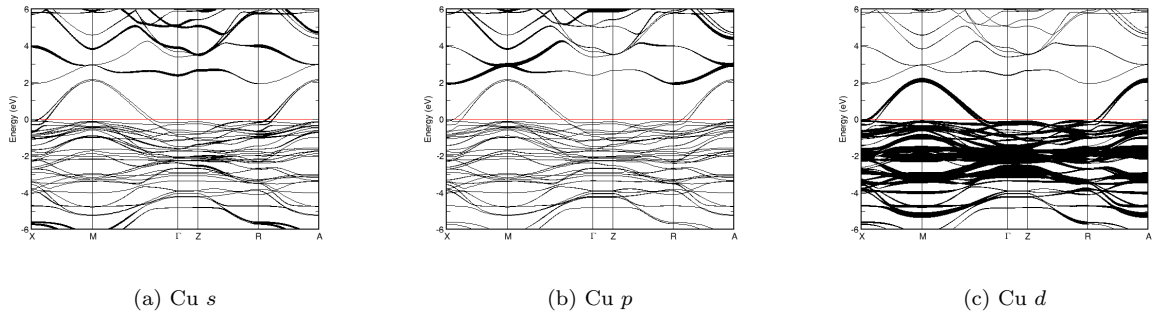FIG. 535: Fat band representation of Cu in  $\text{HoBa}_2\text{Cu}_3\text{O}_6$ 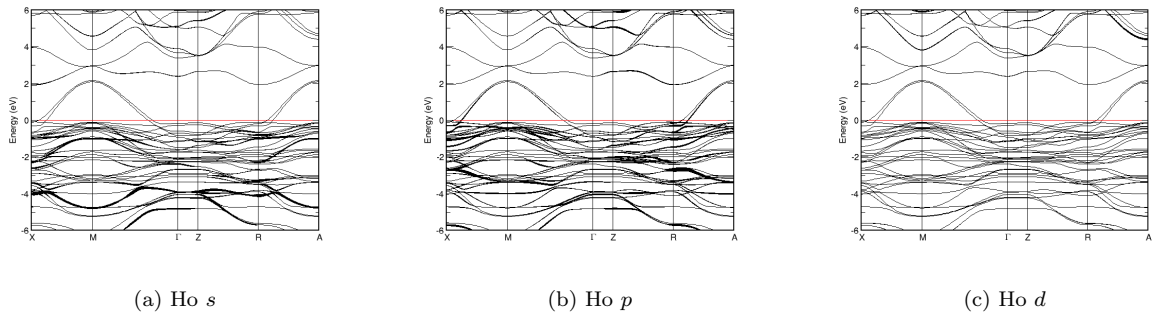FIG. 536: Fat band representation of Ho in  $\text{HoBa}_2\text{Cu}_3\text{O}_6$ 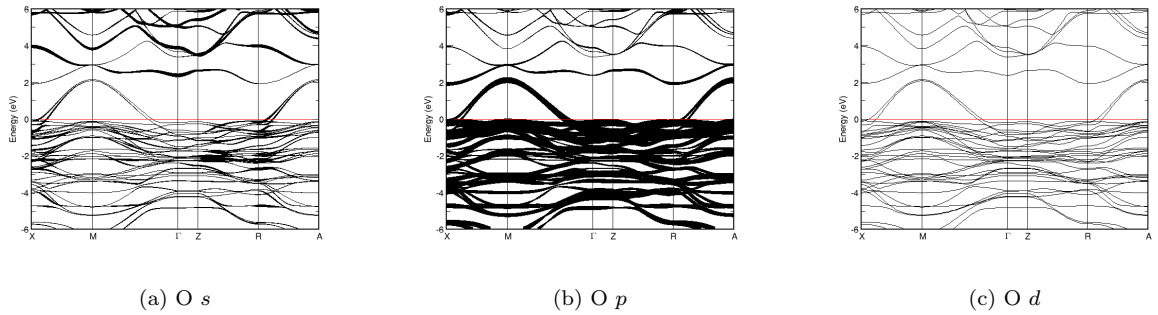FIG. 537: Fat band representation of O in  $\text{HoBa}_2\text{Cu}_3\text{O}_6$

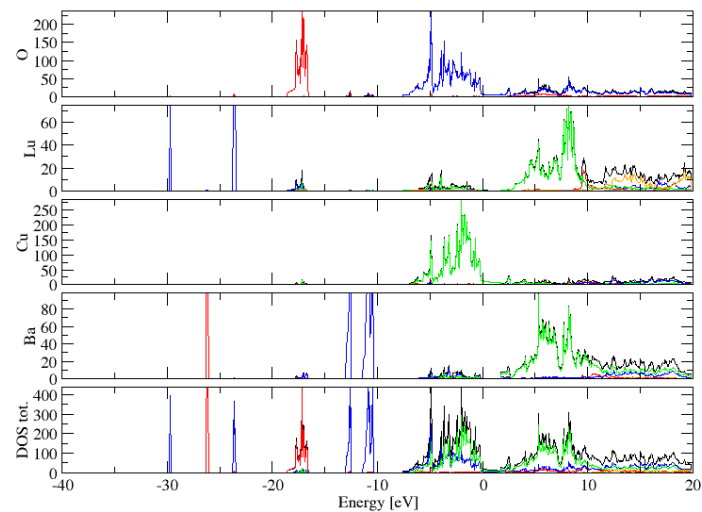

FIG. 538: (Color online) PDOS of  $\text{LuBa}_2\text{Cu}_3\text{O}_6$  (ICSD #98113). The  $s$ -,  $p$ - and  $d$ -projected states are in red, blue and green, respectively.  $\text{LuBa}_2\text{Cu}_3\text{O}_6$  crystallizes in space group  $P 4/m m m$  (#123), in a tetragonal primitive structure.

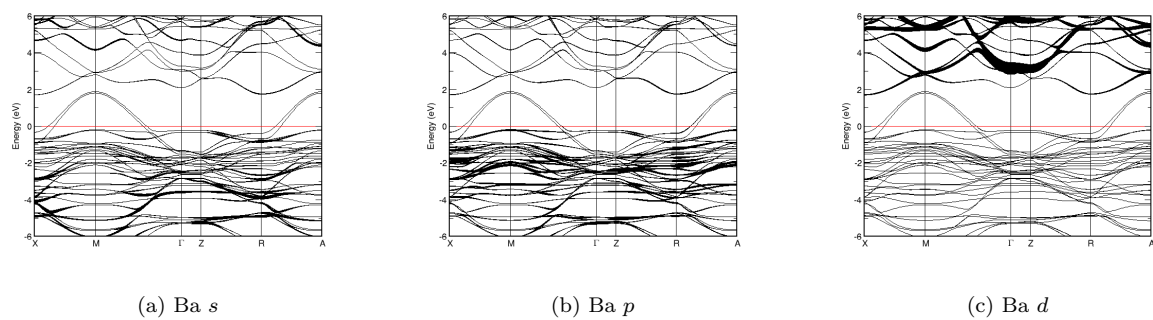

FIG. 539: Fat band representation of Ba in  $\text{LuBa}_2\text{Cu}_3\text{O}_6$

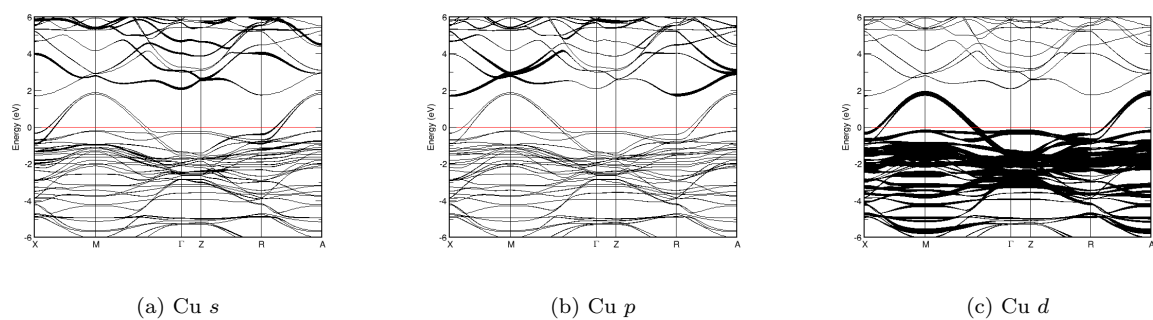

FIG. 540: Fat band representation of Cu in  $\text{LuBa}_2\text{Cu}_3\text{O}_6$

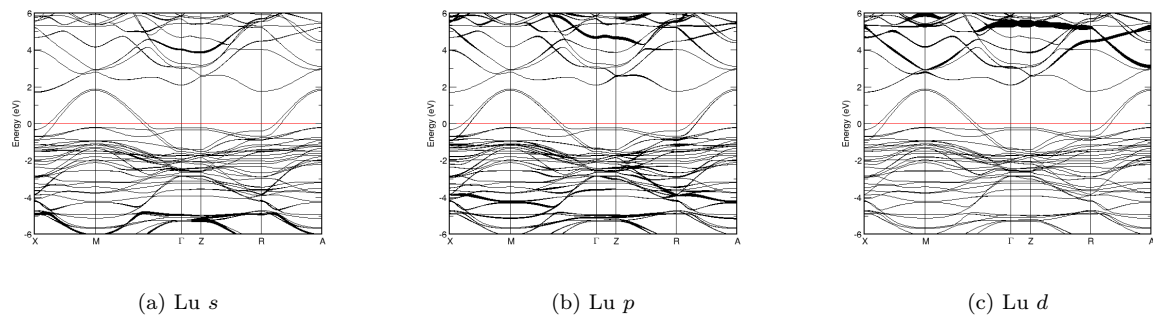FIG. 541: Fat band representation of Lu in  $\text{LuBa}_2\text{Cu}_3\text{O}_6$ 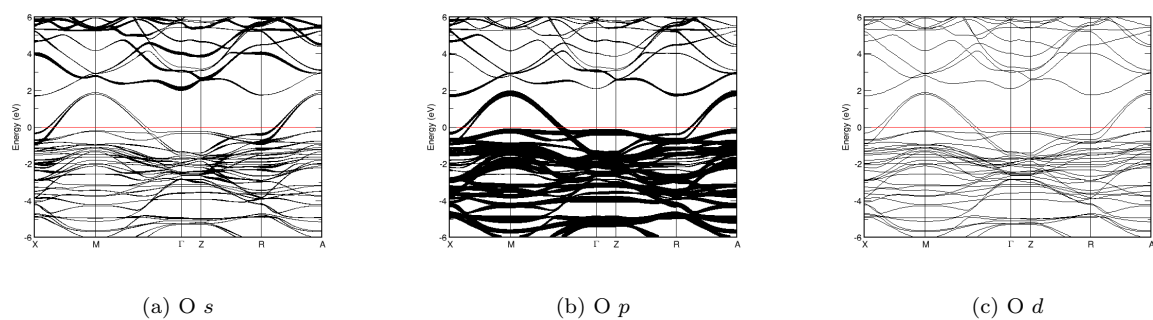FIG. 542: Fat band representation of O in  $\text{LuBa}_2\text{Cu}_3\text{O}_6$ 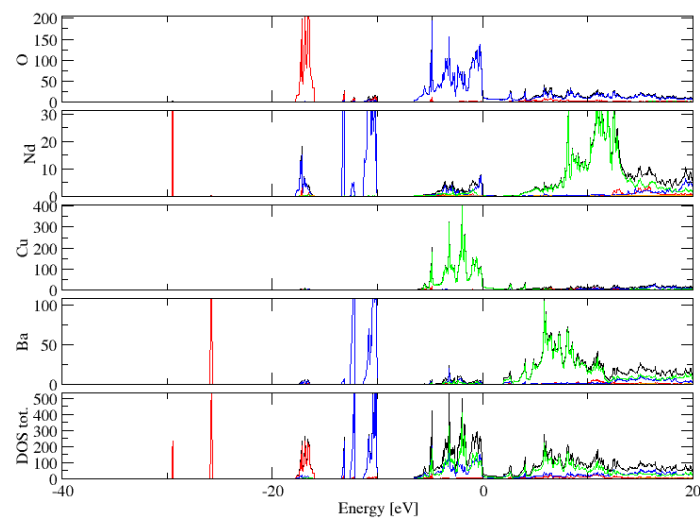

FIG. 543: (Color online) PDOS of  $\text{NdBa}_2\text{Cu}_3\text{O}_6$  (ICSD #83074). The *s*-, *p*- and *d*-projected states are in red, blue and green, respectively.  $\text{NdBa}_2\text{Cu}_3\text{O}_6$  crystallizes in space group  $P 4/m m m$  (#123), in a tetragonal primitive structure.

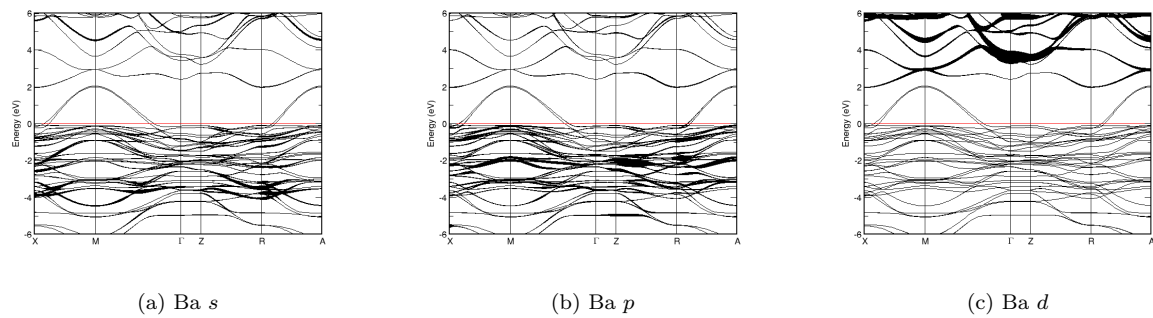FIG. 544: Fat band representation of Ba in NdBa<sub>2</sub>Cu<sub>3</sub>O<sub>6</sub>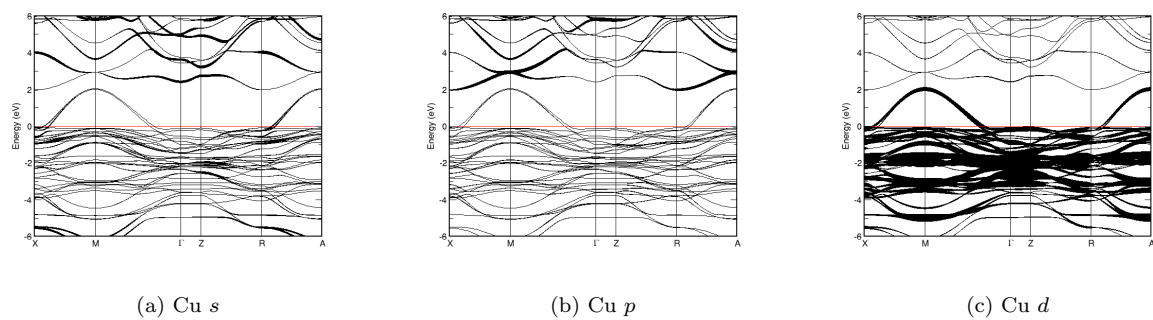FIG. 545: Fat band representation of Cu in NdBa<sub>2</sub>Cu<sub>3</sub>O<sub>6</sub>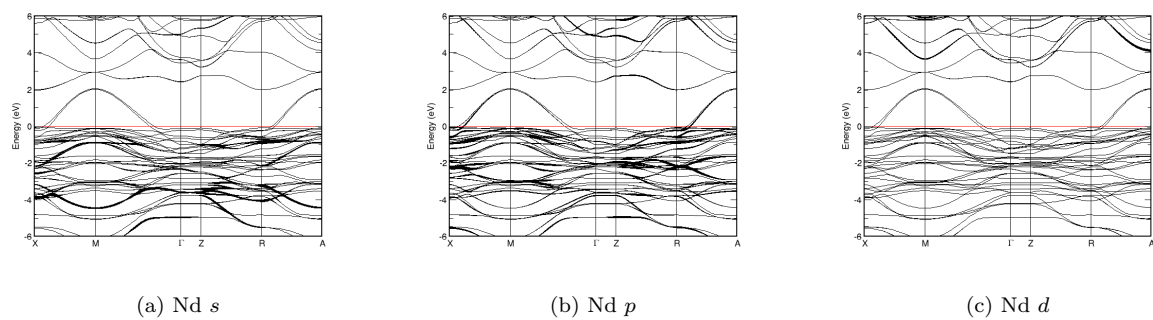FIG. 546: Fat band representation of Nd in NdBa<sub>2</sub>Cu<sub>3</sub>O<sub>6</sub>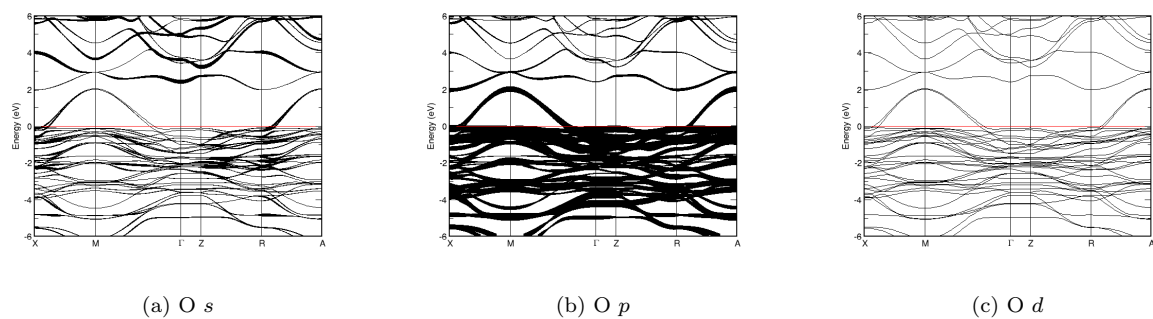FIG. 547: Fat band representation of O in NdBa<sub>2</sub>Cu<sub>3</sub>O<sub>6</sub>

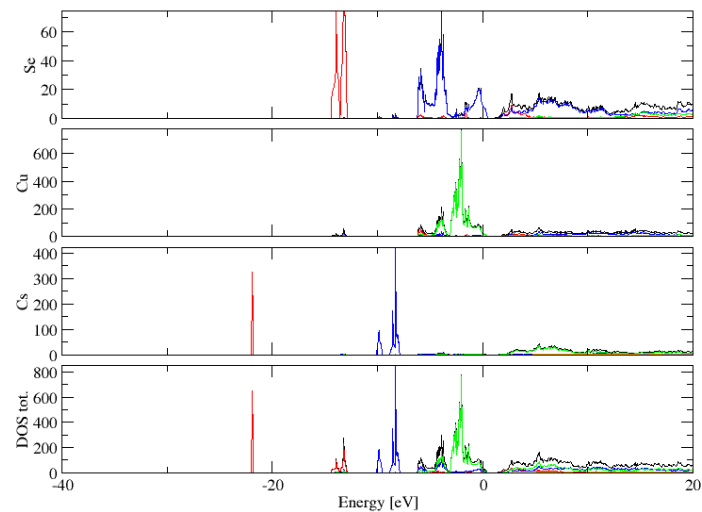

FIG. 548: (Color online) PDOS of  $\text{Cs}(\text{Cu}_4\text{Se}_3)$  (ICSD #75196). The  $s$ -,  $p$ - and  $d$ -projected states are in red, blue and green, respectively.  $\text{Cs}(\text{Cu}_4\text{Se}_3)$  crystallizes in space group  $P 4/m m m$  (#123), in a tetragonal primitive structure.

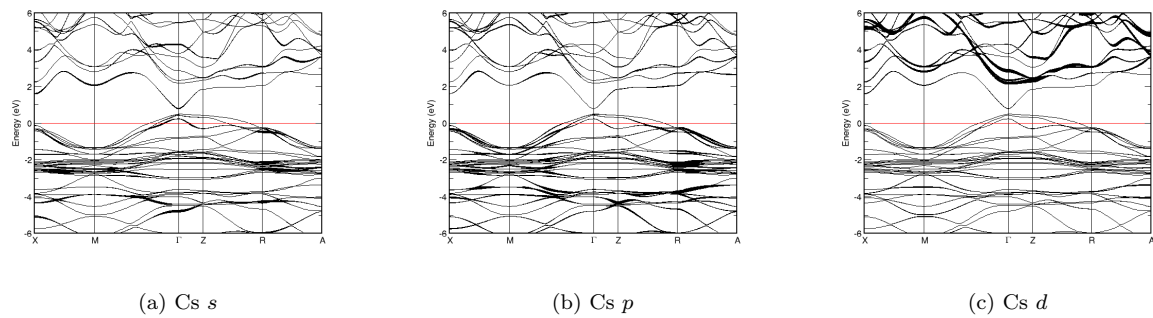

FIG. 549: Fat band representation of Cs in  $\text{Cs}(\text{Cu}_4\text{Se}_3)$

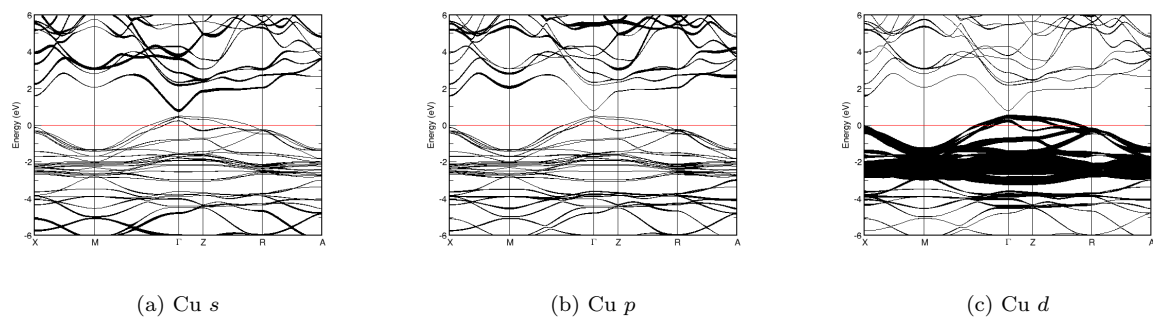

FIG. 550: Fat band representation of Cu in  $\text{Cs}(\text{Cu}_4\text{Se}_3)$

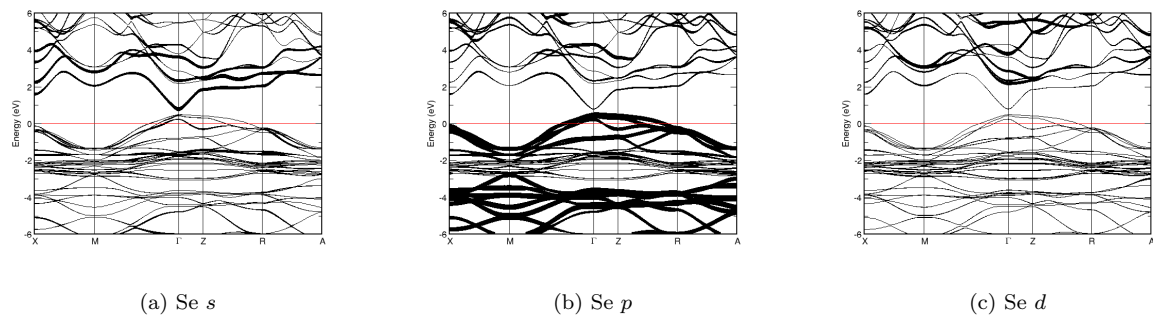FIG. 551: Fat band representation of Se in Cs(Cu<sub>4</sub>Se<sub>3</sub>)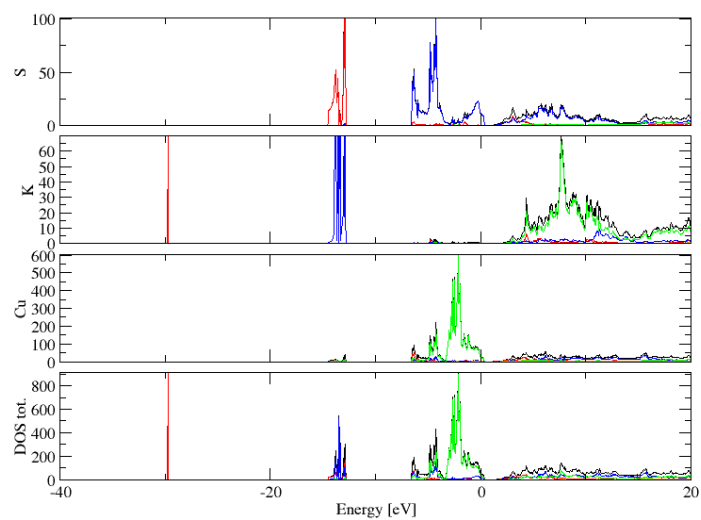FIG. 552: (Color online) PDOS of KCu<sub>4</sub>S<sub>3</sub> (ICSD #23336). The *s*-, *p*- and *d*-projected states are in red, blue and green, respectively. KCu<sub>4</sub>S<sub>3</sub> crystallizes in space group P 4/m m m (#123), in a tetragonal primitive structure.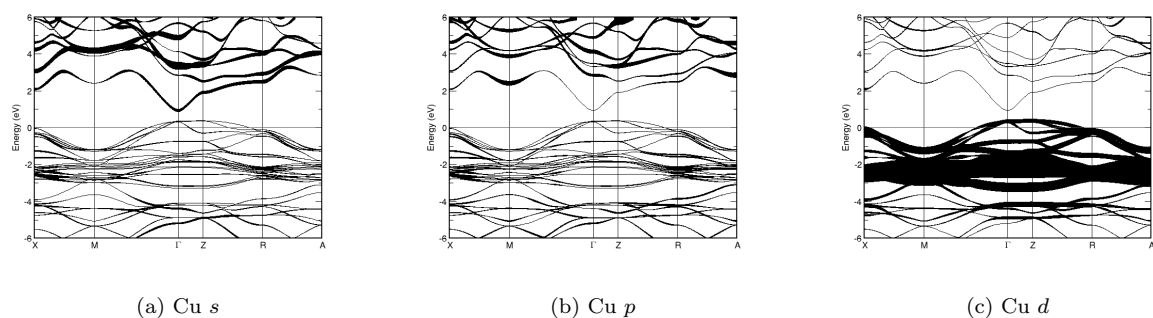FIG. 553: Fat band representation of Cu in KCu<sub>4</sub>S<sub>3</sub>

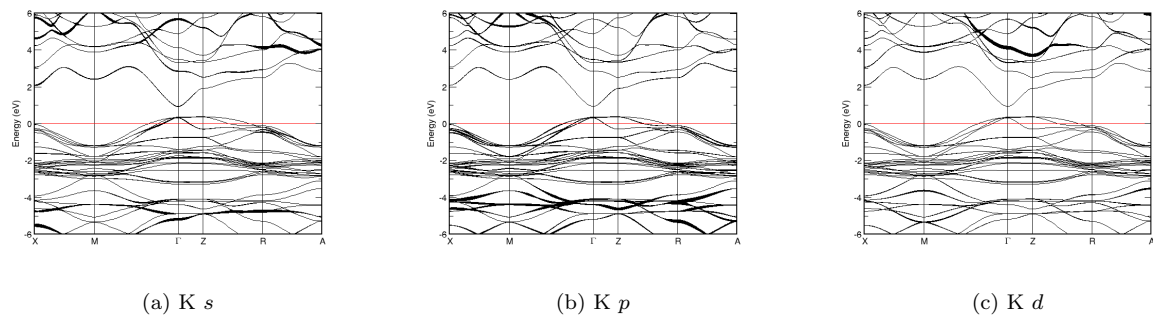FIG. 554: Fat band representation of K in  $\text{KCu}_4\text{S}_3$ 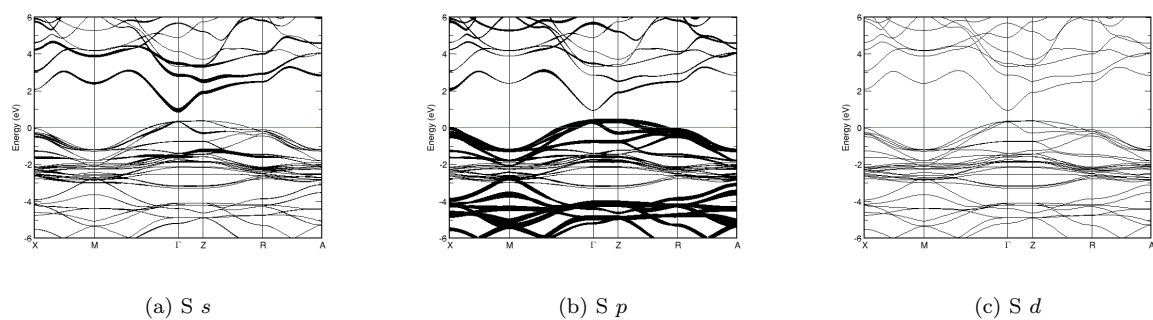FIG. 555: Fat band representation of S in  $\text{KCu}_4\text{S}_3$ 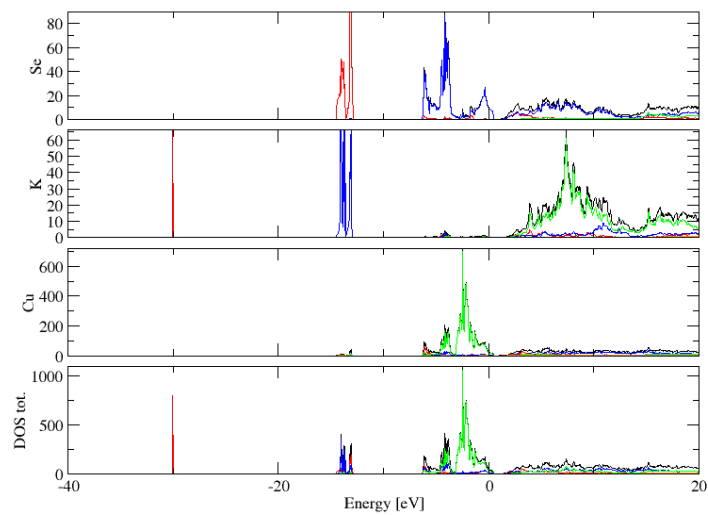FIG. 556: (Color online) PDOS of  $\text{KCu}_4\text{Se}_3$  (ICSD #280072). The *s*-, *p*- and *d*-projected states are in red, blue and green, respectively.  $\text{KCu}_4\text{Se}_3$  crystallizes in space group  $P 4/m m m$  (#123), in a tetragonal primitive structure.

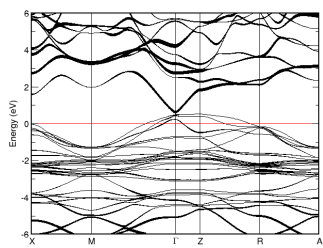(a) Cu *s*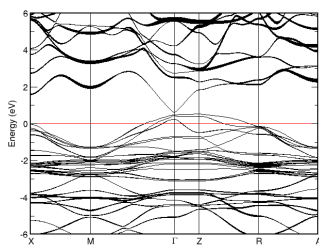(b) Cu *p*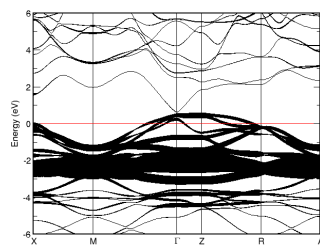(c) Cu *d*FIG. 557: Fat band representation of Cu in  $\text{KCu}_4\text{Se}_3$ 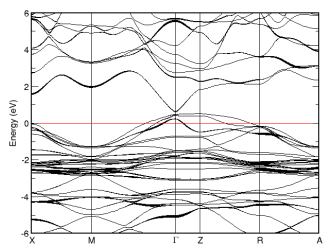(a) K *s*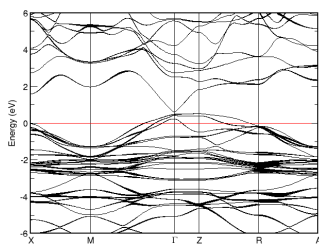(b) K *p*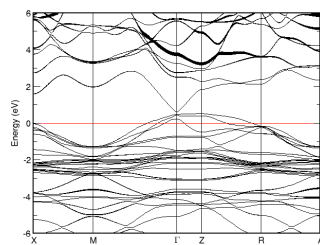(c) K *d*FIG. 558: Fat band representation of K in  $\text{KCu}_4\text{Se}_3$ 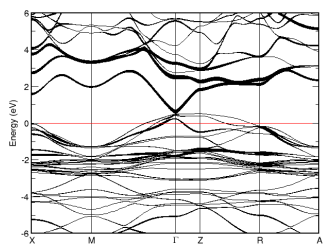(a) Se *s*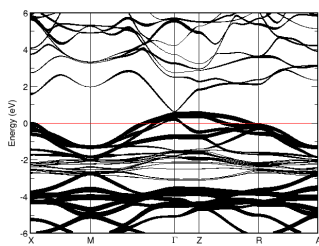(b) Se *p*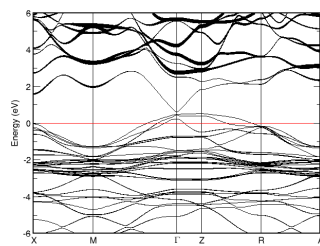(c) Se *d*FIG. 559: Fat band representation of Se in  $\text{KCu}_4\text{Se}_3$
